# Supplementary material for: Floccinaucinihilipilification: Semisimple extensions of the Standard Model gauge algebra
Source: arXiv:2104.14555 ancillary file (2022-06-17)
Supplement: Supplementary file 1 [file Supplementary_File.pdf]

# Floccinaucinihilipilification: Supplementary file

B C Allanach*
*DAMTP, University of Cambridge, Wilberforce Road, Cambridge, CB3 0WA, United Kingdom*

Ben Gripaios† and Joseph Tooby-Smith‡
*Cavendish Laboratory, University of Cambridge, J.J. Thomson Avenue, Cambridge, CB3 0HE, United Kingdom*

Algebras corresponding to: 1 generation can be found in § A, 2 generations in § B, maximal algebras with 3 generations in § C, minimal algebras with 3 generations in § D, and algebras with 3 generations, which are neither maximal nor minimal in § E.

## A. 1 generation algebras

**1 generation subalgebra** 1
Algebra: $\mathfrak{so}(10)$
$(\mathbf{16}),\ (0,0,0,0,1) \mapsto (D,E,L,N,Q,U)$
Projection matrix for $\alpha$:

$$\begin{pmatrix} 0 & 0 & 1 & 0 & 0 \\ 0 & 0 & 0 & 0 & 1 \\ 1 & 0 & 0 & 0 & 0 \\ 3 & 6 & 4 & 0 & 2 \end{pmatrix}$$

**1 generation subalgebra** 2
Algebra: $\mathfrak{su}(5)$
$(\overline{\mathbf{5}}),\ (0,0,0,1) \mapsto (D,L)$
$(\mathbf{10}),\ (0,1,0,0) \mapsto (E,Q,U)$
$(\mathbf{1}),\ (0,0,0,0) \mapsto (N)$
Projection matrix for $\alpha$:

$$\begin{pmatrix} 0 & 0 & 1 & 0 \\ 0 & 0 & 0 & 1 \\ 1 & 0 & 0 & 0 \\ 3 & 6 & 4 & 2 \end{pmatrix}$$

**1 generation subalgebra** 3
Algebra: $\mathfrak{su}(4) \oplus \mathfrak{su}(2) \oplus \mathfrak{su}(2)$
$(\overline{\mathbf{4}},\mathbf{2},\mathbf{1}),\ (0,0,1,1,0) \mapsto (L,Q)$
$(\mathbf{4},\mathbf{1},\mathbf{2}),\ (1,0,0,0,1) \mapsto (D,E,N,U)$
Projection matrix for $\alpha$:

$$\begin{pmatrix} 0 & 1 & 0 & 0 & 0 \\ 1 & 0 & 0 & 0 & 0 \\ 0 & 0 & 0 & 1 & 0 \\ -1 & -2 & -3 & 0 & 3 \end{pmatrix}$$

## B. 2 generation algebras

**2 generation subalgebra** 1
Algebra: $\mathfrak{so}(10)$

---

*Electronic address: B.C.Allanach@damtp.cam.ac.uk
†Electronic address: gripaios@hep.phy.cam.ac.uk
‡Electronic address: jss85@cam.ac.uk

$(\mathbf{16}),\ (0,0,0,0,1) \mapsto (D,E,L,N,Q,U)$
$(\mathbf{16}),\ (0,0,0,0,1) \mapsto (D,E,L,N,Q,U)$
Projection matrix for $\alpha$:

$$\begin{pmatrix} 0 & 0 & 1 & 0 & 0 \\ 0 & 0 & 0 & 0 & 1 \\ 1 & 0 & 0 & 0 & 0 \\ 3 & 6 & 4 & 0 & 2 \end{pmatrix}$$

**2 generation subalgebra** 2
Algebra: $\mathfrak{su}(5)$
$(\overline{\mathbf{5}}),\ (0,0,0,1) \mapsto (D,L)$
$(\overline{\mathbf{5}}),\ (0,0,0,1) \mapsto (D,L)$
$(\mathbf{10}),\ (0,1,0,0) \mapsto (E,Q,U)$
$(\mathbf{10}),\ (0,1,0,0) \mapsto (E,Q,U)$
$(\mathbf{1}),\ (0,0,0,0) \mapsto (N)$
$(\mathbf{1}),\ (0,0,0,0) \mapsto (N)$
Projection matrix for $\alpha$:

$$\begin{pmatrix} 0 & 0 & 1 & 0 \\ 0 & 0 & 0 & 1 \\ 1 & 0 & 0 & 0 \\ 3 & 6 & 4 & 2 \end{pmatrix}$$

**2 generation subalgebra** 3
Algebra: $\mathfrak{so}(10) \oplus \mathfrak{so}(10)$
$(\mathbf{16},\mathbf{1}),\ (0,0,0,0,1,0,0,0,0,0) \mapsto (D,E,L,N,Q,U)$
$(\mathbf{1},\mathbf{16}),\ (0,0,0,0,0,0,0,0,0,1) \mapsto (D,E,L,N,Q,U)$
Projection matrix for $\alpha$:

$$\begin{pmatrix} 0 & 0 & 1 & 0 & 0 & 0 & 0 & 1 & 0 & 0 \\ 0 & 0 & 0 & 0 & 1 & 0 & 0 & 0 & 0 & 1 \\ 1 & 0 & 0 & 0 & 0 & 1 & 0 & 0 & 0 & 0 \\ 3 & 6 & 4 & 0 & 2 & 3 & 6 & 4 & 0 & 2 \end{pmatrix}$$

**2 generation subalgebra** 4
Algebra: $\mathfrak{so}(10) \oplus \mathfrak{su}(2)$
$(\mathbf{16},\mathbf{2}),\ (0,0,0,0,1,1) \mapsto (D,D,E,E,L,L,N,N,Q,Q,U,U)$
Projection matrix for $\alpha$:

$$\begin{pmatrix} 0 & 0 & 1 & 0 & 0 & 0 \\ 0 & 0 & 0 & 0 & 1 & 0 \\ 1 & 0 & 0 & 0 & 0 & 0 \\ 3 & 6 & 4 & 0 & 2 & 0 \end{pmatrix}$$

**2 generation subalgebra** 5
Algebra: $\mathfrak{su}(5) \oplus \mathfrak{so}(10)$
$(\overline{\mathbf{5}},\mathbf{1}),\ (0,0,0,1,0,0,0,0,0) \mapsto (D,L)$
$(\mathbf{10},\mathbf{1}),\ (0,1,0,0,0,0,0,0,0) \mapsto (E,Q,U)$
$(\mathbf{1},\mathbf{16}),\ (0,0,0,0,0,0,0,0,1) \mapsto (D,E,L,N,Q,U)$
$(\mathbf{1},\mathbf{1}),\ (0,0,0,0,0,0,0,0,0) \mapsto (N)$
Projection matrix for $\alpha$:

$$\begin{pmatrix} 0 & 0 & 1 & 0 & 0 & 0 & 1 & 0 & 0 \\ 0 & 0 & 0 & 1 & 0 & 0 & 0 & 0 & 1 \\ 1 & 0 & 0 & 0 & 1 & 0 & 0 & 0 & 0 \\ 3 & 6 & 4 & 2 & 3 & 6 & 4 & 0 & 2 \end{pmatrix}$$

**2 generation subalgebra** 6
Algebra: $\mathfrak{su}(5) \oplus \mathfrak{su}(2)$

$(\overline{\mathbf{5}},\mathbf{2}),\ (0,0,0,1,1)\mapsto(D,D,L,L)$
$(\mathbf{10},\mathbf{2}),\ (0,1,0,0,1)\mapsto(E,E,Q,Q,U,U)$
$(\mathbf{1},\mathbf{1}),\ (0,0,0,0,0)\mapsto(N)$
$(\mathbf{1},\mathbf{1}),\ (0,0,0,0,0)\mapsto(N)$
Projection matrix for $\alpha$:

$$\begin{pmatrix}0&0&1&0&0\\0&0&0&1&0\\1&0&0&0&0\\3&6&4&2&0\end{pmatrix}$$

**2 generation subalgebra** 7
Algebra: $\mathfrak{su}(5)\oplus\mathfrak{su}(2)$
$(\overline{\mathbf{5}},\mathbf{1}),\ (0,0,0,1,0)\mapsto(D,L)$
$(\overline{\mathbf{5}},\mathbf{1}),\ (0,0,0,1,0)\mapsto(D,L)$
$(\mathbf{10},\mathbf{2}),\ (0,1,0,0,1)\mapsto(E,E,Q,Q,U,U)$
$(\mathbf{1},\mathbf{1}),\ (0,0,0,0,0)\mapsto(N)$
$(\mathbf{1},\mathbf{1}),\ (0,0,0,0,0)\mapsto(N)$
Projection matrix for $\alpha$:

$$\begin{pmatrix}0&0&1&0&0\\0&0&0&1&0\\1&0&0&0&0\\3&6&4&2&0\end{pmatrix}$$

**2 generation subalgebra** 8
Algebra: $\mathfrak{su}(5)\oplus\mathfrak{su}(2)$
$(\overline{\mathbf{5}},\mathbf{2}),\ (0,0,0,1,1)\mapsto(D,D,L,L)$
$(\mathbf{10},\mathbf{2}),\ (0,1,0,0,1)\mapsto(E,E,Q,Q,U,U)$
$(\mathbf{1},\mathbf{2}),\ (0,0,0,0,1)\mapsto(N,N)$
Projection matrix for $\alpha$:

$$\begin{pmatrix}0&0&1&0&0\\0&0&0&1&0\\1&0&0&0&0\\3&6&4&2&0\end{pmatrix}$$

**2 generation subalgebra** 9
Algebra: $\mathfrak{su}(5)\oplus\mathfrak{su}(2)$
$(\mathbf{10},\mathbf{1}),\ (0,1,0,0,0)\mapsto(E,Q,U)$
$(\mathbf{10},\mathbf{1}),\ (0,1,0,0,0)\mapsto(E,Q,U)$
$(\overline{\mathbf{5}},\mathbf{2}),\ (0,0,0,1,1)\mapsto(D,D,L,L)$
$(\mathbf{1},\mathbf{1}),\ (0,0,0,0,0)\mapsto(N)$
$(\mathbf{1},\mathbf{1}),\ (0,0,0,0,0)\mapsto(N)$
Projection matrix for $\alpha$:

$$\begin{pmatrix}0&0&1&0&0\\0&0&0&1&0\\1&0&0&0&0\\3&6&4&2&0\end{pmatrix}$$

**2 generation subalgebra** 10
Algebra: $\mathfrak{su}(5)\oplus\mathfrak{su}(2)$
$(\overline{\mathbf{5}},\mathbf{1}),\ (0,0,0,1,0)\mapsto(D,L)$
$(\overline{\mathbf{5}},\mathbf{1}),\ (0,0,0,1,0)\mapsto(D,L)$
$(\mathbf{10},\mathbf{2}),\ (0,1,0,0,1)\mapsto(E,E,Q,Q,U,U)$
$(\mathbf{1},\mathbf{2}),\ (0,0,0,0,1)\mapsto(N,N)$
Projection matrix for $\alpha$:

$$\begin{pmatrix}0&0&1&0&0\\0&0&0&1&0\\1&0&0&0&0\\3&6&4&2&0\end{pmatrix}$$

**2 generation subalgebra** 11
Algebra: $\mathfrak{su}(5) \oplus \mathfrak{su}(2)$
$(\mathbf{10}, \mathbf{1}),\ (0,1,0,0,0) \mapsto (E, Q, U)$
$(\mathbf{10}, \mathbf{1}),\ (0,1,0,0,0) \mapsto (E, Q, U)$
$(\overline{\mathbf{5}}, \mathbf{2}),\ (0,0,0,1,1) \mapsto (D, D, L, L)$
$(\mathbf{1}, \mathbf{2}),\ (0,0,0,0,1) \mapsto (N, N)$
Projection matrix for $\alpha$:

$$\begin{pmatrix} 0 & 0 & 1 & 0 & 0 \\ 0 & 0 & 0 & 1 & 0 \\ 1 & 0 & 0 & 0 & 0 \\ 3 & 6 & 4 & 2 & 0 \end{pmatrix}$$

**2 generation subalgebra** 12
Algebra: $\mathfrak{su}(5) \oplus \mathfrak{su}(2)$
$(\overline{\mathbf{5}}, \mathbf{1}),\ (0,0,0,1,0) \mapsto (D, L)$
$(\overline{\mathbf{5}}, \mathbf{1}),\ (0,0,0,1,0) \mapsto (D, L)$
$(\mathbf{10}, \mathbf{1}),\ (0,1,0,0,0) \mapsto (E, Q, U)$
$(\mathbf{10}, \mathbf{1}),\ (0,1,0,0,0) \mapsto (E, Q, U)$
$(\mathbf{1}, \mathbf{2}),\ (0,0,0,0,1) \mapsto (N, N)$
Projection matrix for $\alpha$:

$$\begin{pmatrix} 0 & 0 & 1 & 0 & 0 \\ 0 & 0 & 0 & 1 & 0 \\ 1 & 0 & 0 & 0 & 0 \\ 3 & 6 & 4 & 2 & 0 \end{pmatrix}$$

**2 generation subalgebra** 13
Algebra: $\mathfrak{su}(5) \oplus \mathfrak{su}(5)$
$(\overline{\mathbf{5}}, \mathbf{1}),\ (0,0,0,1,0,0,0,0) \mapsto (D, L)$
$(\mathbf{10}, \mathbf{1}),\ (0,1,0,0,0,0,0,0) \mapsto (E, Q, U)$
$(\mathbf{1}, \overline{\mathbf{5}}),\ (0,0,0,0,0,0,0,1) \mapsto (D, L)$
$(\mathbf{1}, \mathbf{10}),\ (0,0,0,0,0,1,0,0) \mapsto (E, Q, U)$
$(\mathbf{1}, \mathbf{1}),\ (0,0,0,0,0,0,0,0) \mapsto (N)$
$(\mathbf{1}, \mathbf{1}),\ (0,0,0,0,0,0,0,0) \mapsto (N)$
Projection matrix for $\alpha$:

$$\begin{pmatrix} 0 & 0 & 1 & 0 & 0 & 0 & 1 & 0 \\ 0 & 0 & 0 & 1 & 0 & 0 & 0 & 1 \\ 1 & 0 & 0 & 0 & 1 & 0 & 0 & 0 \\ 3 & 6 & 4 & 2 & 3 & 6 & 4 & 2 \end{pmatrix}$$

**2 generation subalgebra** 14
Algebra: $\mathfrak{su}(4) \oplus \mathfrak{sp}(4) \oplus \mathfrak{sp}(4)$
$(\overline{\mathbf{4}}, \mathbf{4}, \mathbf{1}),\ (0,0,1,1,0,0,0) \mapsto (L, L, Q, Q)$
$(\mathbf{4}, \mathbf{1}, \mathbf{4}),\ (1,0,0,0,0,1,0) \mapsto (D, D, E, E, N, N, U, U)$
Projection matrix for $\alpha$:

$$\begin{pmatrix} 0 & 1 & 0 & 0 & 0 & 0 & 0 \\ 1 & 0 & 0 & 0 & 0 & 0 & 0 \\ 0 & 0 & 0 & 1 & 2 & 0 & 0 \\ -1 & -2 & -3 & 0 & 0 & 3 & 0 \end{pmatrix}$$

**2 generation subalgebra** 15
Algebra: $\mathfrak{su}(4) \oplus \mathfrak{sp}(4) \oplus \mathfrak{su}(2)$
$(\overline{\mathbf{4}}, \mathbf{4}, \mathbf{1}),\ (0,0,1,1,0,0) \mapsto (L, L, Q, Q)$
$(\mathbf{4}, \mathbf{1}, \mathbf{2}),\ (1,0,0,0,0,1) \mapsto (D, E, N, U)$
$(\mathbf{4}, \mathbf{1}, \mathbf{2}),\ (1,0,0,0,0,1) \mapsto (D, E, N, U)$

Projection matrix for $\alpha$:

$$\begin{pmatrix} 0 & 1 & 0 & 0 & 0 & 0 \\ 1 & 0 & 0 & 0 & 0 & 0 \\ 0 & 0 & 0 & 1 & 2 & 0 \\ -1 & -2 & -3 & 0 & 0 & 3 \end{pmatrix}$$

**2 generation subalgebra** 16
Algebra: $\mathfrak{su}(4) \oplus \mathfrak{sp}(4) \oplus \mathfrak{su}(2)$
$(\overline{\mathbf{4}}, \mathbf{4}, \mathbf{1})$, $(0,0,1,1,0,0) \mapsto (D, D, E, E, N, N, U, U)$
$(\mathbf{4}, \mathbf{1}, \mathbf{2})$, $(1,0,0,0,0,1) \mapsto (L, Q)$
$(\mathbf{4}, \mathbf{1}, \mathbf{2})$, $(1,0,0,0,0,1) \mapsto (L, Q)$
Projection matrix for $\alpha$:

$$\begin{pmatrix} 1 & 0 & 0 & 0 & 0 & 0 \\ 0 & 1 & 0 & 0 & 0 & 0 \\ 0 & 0 & 0 & 0 & 0 & 1 \\ 1 & 2 & 3 & 3 & 0 & 0 \end{pmatrix}$$

**2 generation subalgebra** 17
Algebra: $\mathfrak{su}(4) \oplus \mathfrak{su}(2) \oplus \mathfrak{su}(2)$
$(\overline{\mathbf{4}}, \mathbf{2}, \mathbf{1})$, $(0,0,1,1,0) \mapsto (L, Q)$
$(\overline{\mathbf{4}}, \mathbf{2}, \mathbf{1})$, $(0,0,1,1,0) \mapsto (L, Q)$
$(\mathbf{4}, \mathbf{1}, \mathbf{2})$, $(1,0,0,0,1) \mapsto (D, E, N, U)$
$(\mathbf{4}, \mathbf{1}, \mathbf{2})$, $(1,0,0,0,1) \mapsto (D, E, N, U)$
Projection matrix for $\alpha$:

$$\begin{pmatrix} 0 & 1 & 0 & 0 & 0 \\ 1 & 0 & 0 & 0 & 0 \\ 0 & 0 & 0 & 1 & 0 \\ -1 & -2 & -3 & 0 & 3 \end{pmatrix}$$

**2 generation subalgebra** 18
Algebra: $\mathfrak{su}(5) \oplus \mathfrak{su}(2) \oplus \mathfrak{su}(2)$
$(\overline{\mathbf{5}}, \mathbf{2}, \mathbf{1})$, $(0,0,0,1,1,0) \mapsto (D, D, L, L)$
$(\mathbf{10}, \mathbf{1}, \mathbf{2})$, $(0,1,0,0,0,1) \mapsto (E, E, Q, Q, U, U)$
$(\mathbf{1}, \mathbf{1}, \mathbf{1})$, $(0,0,0,0,0,0) \mapsto (N)$
$(\mathbf{1}, \mathbf{1}, \mathbf{1})$, $(0,0,0,0,0,0) \mapsto (N)$
Projection matrix for $\alpha$:

$$\begin{pmatrix} 0 & 0 & 1 & 0 & 0 & 0 \\ 0 & 0 & 0 & 1 & 0 & 0 \\ 1 & 0 & 0 & 0 & 0 & 0 \\ 3 & 6 & 4 & 2 & 0 & 0 \end{pmatrix}$$

**2 generation subalgebra** 19
Algebra: $\mathfrak{su}(5) \oplus \mathfrak{su}(2) \oplus \mathfrak{su}(2)$
$(\overline{\mathbf{5}}, \mathbf{2}, \mathbf{1})$, $(0,0,0,1,1,0) \mapsto (D, D, L, L)$
$(\mathbf{10}, \mathbf{1}, \mathbf{2})$, $(0,1,0,0,0,1) \mapsto (E, E, Q, Q, U, U)$
$(\mathbf{1}, \mathbf{1}, \mathbf{2})$, $(0,0,0,0,0,1) \mapsto (N, N)$
Projection matrix for $\alpha$:

$$\begin{pmatrix} 0 & 0 & 1 & 0 & 0 & 0 \\ 0 & 0 & 0 & 1 & 0 & 0 \\ 1 & 0 & 0 & 0 & 0 & 0 \\ 3 & 6 & 4 & 2 & 0 & 0 \end{pmatrix}$$

**2 generation subalgebra** 20
Algebra: $\mathfrak{su}(5) \oplus \mathfrak{su}(2) \oplus \mathfrak{su}(2)$
$(\overline{\mathbf{5}}, \mathbf{2}, \mathbf{1})$, $(0,0,0,1,1,0) \mapsto (D, D, L, L)$

$(\mathbf{10},\mathbf{1},\mathbf{2})$, $(0,1,0,0,0,1) \mapsto (E,E,Q,Q,U,U)$
$(\mathbf{1},\mathbf{2},\mathbf{1})$, $(0,0,0,0,1,0) \mapsto (N,N)$
Projection matrix for $\alpha$:

$$\begin{pmatrix} 0 & 0 & 1 & 0 & 0 & 0 \\ 0 & 0 & 0 & 1 & 0 & 0 \\ 1 & 0 & 0 & 0 & 0 & 0 \\ 3 & 6 & 4 & 2 & 0 & 0 \end{pmatrix}$$

**2 generation subalgebra** 21
Algebra: $\mathfrak{su}(5) \oplus \mathfrak{su}(2) \oplus \mathfrak{su}(2)$
$(\overline{\mathbf{5}},\mathbf{2},\mathbf{1})$, $(0,0,0,1,1,0) \mapsto (D,D,L,L)$
$(\mathbf{10},\mathbf{2},\mathbf{1})$, $(0,1,0,0,1,0) \mapsto (E,E,Q,Q,U,U)$
$(\mathbf{1},\mathbf{1},\mathbf{2})$, $(0,0,0,0,0,1) \mapsto (N,N)$
Projection matrix for $\alpha$:

$$\begin{pmatrix} 0 & 0 & 1 & 0 & 0 & 0 \\ 0 & 0 & 0 & 1 & 0 & 0 \\ 1 & 0 & 0 & 0 & 0 & 0 \\ 3 & 6 & 4 & 2 & 0 & 0 \end{pmatrix}$$

**2 generation subalgebra** 22
Algebra: $\mathfrak{su}(5) \oplus \mathfrak{su}(2) \oplus \mathfrak{su}(2)$
$(\overline{\mathbf{5}},\mathbf{1},\mathbf{1})$, $(0,0,0,1,0,0) \mapsto (D,L)$
$(\overline{\mathbf{5}},\mathbf{1},\mathbf{1})$, $(0,0,0,1,0,0) \mapsto (D,L)$
$(\mathbf{10},\mathbf{2},\mathbf{1})$, $(0,1,0,0,1,0) \mapsto (E,E,Q,Q,U,U)$
$(\mathbf{1},\mathbf{1},\mathbf{2})$, $(0,0,0,0,0,1) \mapsto (N,N)$
Projection matrix for $\alpha$:

$$\begin{pmatrix} 0 & 0 & 1 & 0 & 0 & 0 \\ 0 & 0 & 0 & 1 & 0 & 0 \\ 1 & 0 & 0 & 0 & 0 & 0 \\ 3 & 6 & 4 & 2 & 0 & 0 \end{pmatrix}$$

**2 generation subalgebra** 23
Algebra: $\mathfrak{su}(5) \oplus \mathfrak{su}(2) \oplus \mathfrak{su}(2)$
$(\mathbf{10},\mathbf{1},\mathbf{1})$, $(0,1,0,0,0,0) \mapsto (E,Q,U)$
$(\mathbf{10},\mathbf{1},\mathbf{1})$, $(0,1,0,0,0,0) \mapsto (E,Q,U)$
$(\overline{\mathbf{5}},\mathbf{2},\mathbf{1})$, $(0,0,0,1,1,0) \mapsto (D,D,L,L)$
$(\mathbf{1},\mathbf{1},\mathbf{2})$, $(0,0,0,0,0,1) \mapsto (N,N)$
Projection matrix for $\alpha$:

$$\begin{pmatrix} 0 & 0 & 1 & 0 & 0 & 0 \\ 0 & 0 & 0 & 1 & 0 & 0 \\ 1 & 0 & 0 & 0 & 0 & 0 \\ 3 & 6 & 4 & 2 & 0 & 0 \end{pmatrix}$$

**2 generation subalgebra** 24
Algebra: $\mathfrak{su}(5) \oplus \mathfrak{su}(5) \oplus \mathfrak{su}(2)$
$(\overline{\mathbf{5}},\mathbf{1},\mathbf{1})$, $(0,0,0,1,0,0,0,0,0) \mapsto (D,L)$
$(\mathbf{10},\mathbf{1},\mathbf{1})$, $(0,1,0,0,0,0,0,0,0) \mapsto (E,Q,U)$
$(\mathbf{1},\overline{\mathbf{5}},\mathbf{1})$, $(0,0,0,0,0,0,0,1,0) \mapsto (D,L)$
$(\mathbf{1},\mathbf{10},\mathbf{1})$, $(0,0,0,0,0,1,0,0,0) \mapsto (E,Q,U)$
$(\mathbf{1},\mathbf{1},\mathbf{2})$, $(0,0,0,0,0,0,0,0,1) \mapsto (N,N)$
Projection matrix for $\alpha$:

$$\begin{pmatrix} 0 & 0 & 1 & 0 & 0 & 0 & 1 & 0 & 0 \\ 0 & 0 & 0 & 1 & 0 & 0 & 0 & 1 & 0 \\ 1 & 0 & 0 & 0 & 1 & 0 & 0 & 0 & 0 \\ 3 & 6 & 4 & 2 & 3 & 6 & 4 & 2 & 0 \end{pmatrix}$$

**2 generation subalgebra** 25
Algebra: $\mathfrak{su}(8) \oplus \mathfrak{su}(2) \oplus \mathfrak{su}(2)$
$(\overline{\mathbf{8}}, \mathbf{2}, \mathbf{1})$, $(0,0,0,0,0,0,1,1,0) \mapsto (L,L,Q,Q)$
$(\mathbf{8}, \mathbf{1}, \mathbf{2})$, $(1,0,0,0,0,0,0,0,1) \mapsto (D,D,E,E,N,N,U,U)$
Projection matrix for $\alpha$:

$$\begin{pmatrix} 0 & 1 & 0 & 0 & 1 & 0 & 0 & 0 & 0 \\ 1 & 0 & 0 & 1 & 0 & 0 & 0 & 0 & 0 \\ 0 & 0 & 0 & 0 & 0 & 0 & 0 & 1 & 0 \\ -1 & -2 & -3 & -4 & -5 & -6 & -3 & 0 & 3 \end{pmatrix}$$

**2 generation subalgebra** 26
Algebra: $\mathfrak{su}(4) \oplus \mathfrak{so}(10) \oplus \mathfrak{su}(2) \oplus \mathfrak{su}(2)$
$(\mathbf{1}, \mathbf{16}, \mathbf{1}, \mathbf{1})$, $(0,0,0,0,0,0,0,1,0,0) \mapsto (D,E,L,N,Q,U)$
$(\overline{\mathbf{4}}, \mathbf{1}, \mathbf{2}, \mathbf{1})$, $(0,0,1,0,0,0,0,0,1,0) \mapsto (L,Q)$
$(\mathbf{4}, \mathbf{1}, \mathbf{1}, \mathbf{2})$, $(1,0,0,0,0,0,0,0,0,1) \mapsto (D,E,N,U)$
Projection matrix for $\alpha$:

$$\begin{pmatrix} 0 & 1 & 0 & 0 & 0 & 1 & 0 & 0 & 0 & 0 \\ 1 & 0 & 0 & 0 & 0 & 0 & 0 & 1 & 0 & 0 \\ 0 & 0 & 0 & 1 & 0 & 0 & 0 & 0 & 1 & 0 \\ -1 & -2 & -3 & 3 & 6 & 4 & 0 & 2 & 0 & 3 \end{pmatrix}$$

**2 generation subalgebra** 27
Algebra: $\mathfrak{su}(4) \oplus \mathfrak{sp}(4) \oplus \mathfrak{su}(2) \oplus \mathfrak{su}(2)$
$(\overline{\mathbf{4}}, \mathbf{4}, \mathbf{1}, \mathbf{1})$, $(0,0,1,1,0,0,0) \mapsto (L,L,Q,Q)$
$(\mathbf{4}, \mathbf{1}, \mathbf{2}, \mathbf{2})$, $(1,0,0,0,0,1,1) \mapsto (D,D,E,E,N,N,U,U)$
Projection matrix for $\alpha$:

$$\begin{pmatrix} 0 & 1 & 0 & 0 & 0 & 0 & 0 \\ 1 & 0 & 0 & 0 & 0 & 0 & 0 \\ 0 & 0 & 0 & 1 & 2 & 0 & 0 \\ -1 & -2 & -3 & 0 & 0 & 3 & 0 \end{pmatrix}$$

**2 generation subalgebra** 28
Algebra: $\mathfrak{su}(4) \oplus \mathfrak{sp}(4) \oplus \mathfrak{su}(2) \oplus \mathfrak{su}(2)$
$(\overline{\mathbf{4}}, \mathbf{4}, \mathbf{1}, \mathbf{1})$, $(0,0,1,1,0,0,0) \mapsto (D,D,E,E,N,N,U,U)$
$(\mathbf{4}, \mathbf{1}, \mathbf{2}, \mathbf{2})$, $(1,0,0,0,0,1,1) \mapsto (L,L,Q,Q)$
Projection matrix for $\alpha$:

$$\begin{pmatrix} 1 & 0 & 0 & 0 & 0 & 0 & 0 \\ 0 & 1 & 0 & 0 & 0 & 0 & 0 \\ 0 & 0 & 0 & 0 & 0 & 1 & 0 \\ 1 & 2 & 3 & 3 & 0 & 0 & 0 \end{pmatrix}$$

**2 generation subalgebra** 29
Algebra: $\mathfrak{su}(4) \oplus \mathfrak{sp}(4) \oplus \mathfrak{su}(2) \oplus \mathfrak{su}(2)$
$(\overline{\mathbf{4}}, \mathbf{4}, \mathbf{1}, \mathbf{1})$, $(0,0,1,1,0,0,0) \mapsto (L,L,Q,Q)$
$(\mathbf{4}, \mathbf{1}, \mathbf{2}, \mathbf{1})$, $(1,0,0,0,0,1,0) \mapsto (D,E,N,U)$
$(\mathbf{4}, \mathbf{1}, \mathbf{1}, \mathbf{2})$, $(1,0,0,0,0,0,1) \mapsto (D,E,N,U)$
Projection matrix for $\alpha$:

$$\begin{pmatrix} 0 & 1 & 0 & 0 & 0 & 0 & 0 \\ 1 & 0 & 0 & 0 & 0 & 0 & 0 \\ 0 & 0 & 0 & 1 & 2 & 0 & 0 \\ -1 & -2 & -3 & 0 & 0 & 3 & 3 \end{pmatrix}$$

**2 generation subalgebra** 30
Algebra: $\mathfrak{su}(4) \oplus \mathfrak{sp}(4) \oplus \mathfrak{su}(2) \oplus \mathfrak{su}(2)$
$(\overline{\mathbf{4}}, \mathbf{4}, \mathbf{1}, \mathbf{1})$, $(0,0,1,1,0,0,0) \mapsto (D,D,E,E,N,N,U,U)$

$(\mathbf{4},\mathbf{1},\mathbf{2},\mathbf{1})$, $(1,0,0,0,0,1,0) \mapsto (L,Q)$
$(\mathbf{4},\mathbf{1},\mathbf{1},\mathbf{2})$, $(1,0,0,0,0,0,1) \mapsto (L,Q)$
Projection matrix for $\alpha$:

$$\begin{pmatrix} 1 & 0 & 0 & 0 & 0 & 0 & 0 \\ 0 & 1 & 0 & 0 & 0 & 0 & 0 \\ 0 & 0 & 0 & 0 & 0 & 1 & 1 \\ 1 & 2 & 3 & 3 & 0 & 0 & 0 \end{pmatrix}$$

**2 generation subalgebra** 31
Algebra: $\mathfrak{su}(4) \oplus \mathfrak{su}(2) \oplus \mathfrak{su}(2) \oplus \mathfrak{su}(2)$
$(\mathbf{4},\mathbf{2},\mathbf{2},\mathbf{1})$, $(1,0,0,1,1,0) \mapsto (L,L,Q,Q)$
$(\overline{\mathbf{4}},\mathbf{2},\mathbf{1},\mathbf{2})$, $(0,0,1,1,0,1) \mapsto (D,D,E,E,N,N,U,U)$
Projection matrix for $\alpha$:

$$\begin{pmatrix} 1 & 0 & 0 & 0 & 0 & 0 \\ 0 & 1 & 0 & 0 & 0 & 0 \\ 0 & 0 & 0 & 0 & 1 & 0 \\ 1 & 2 & 3 & 0 & 0 & 3 \end{pmatrix}$$

**2 generation subalgebra** 32
Algebra: $\mathfrak{su}(4) \oplus \mathfrak{su}(2) \oplus \mathfrak{su}(2) \oplus \mathfrak{su}(2)$
$(\mathbf{4},\mathbf{2},\mathbf{2},\mathbf{1})$, $(1,0,0,1,1,0) \mapsto (D,D,E,E,N,N,U,U)$
$(\overline{\mathbf{4}},\mathbf{1},\mathbf{1},\mathbf{2})$, $(0,0,1,0,0,1) \mapsto (L,Q)$
$(\overline{\mathbf{4}},\mathbf{1},\mathbf{1},\mathbf{2})$, $(0,0,1,0,0,1) \mapsto (L,Q)$
Projection matrix for $\alpha$:

$$\begin{pmatrix} 0 & 1 & 0 & 0 & 0 & 0 \\ 1 & 0 & 0 & 0 & 0 & 0 \\ 0 & 0 & 0 & 0 & 0 & 1 \\ -1 & -2 & -3 & 3 & 0 & 0 \end{pmatrix}$$

**2 generation subalgebra** 33
Algebra: $\mathfrak{su}(4) \oplus \mathfrak{su}(2) \oplus \mathfrak{su}(2) \oplus \mathfrak{su}(2)$
$(\mathbf{4},\mathbf{2},\mathbf{2},\mathbf{1})$, $(1,0,0,1,1,0) \mapsto (L,L,Q,Q)$
$(\overline{\mathbf{4}},\mathbf{1},\mathbf{1},\mathbf{2})$, $(0,0,1,0,0,1) \mapsto (D,E,N,U)$
$(\overline{\mathbf{4}},\mathbf{1},\mathbf{1},\mathbf{2})$, $(0,0,1,0,0,1) \mapsto (D,E,N,U)$
Projection matrix for $\alpha$:

$$\begin{pmatrix} 1 & 0 & 0 & 0 & 0 & 0 \\ 0 & 1 & 0 & 0 & 0 & 0 \\ 0 & 0 & 0 & 1 & 0 & 0 \\ 1 & 2 & 3 & 0 & 0 & 3 \end{pmatrix}$$

**2 generation subalgebra** 34
Algebra: $\mathfrak{su}(4) \oplus \mathfrak{su}(2) \oplus \mathfrak{su}(2) \oplus \mathfrak{su}(2)$
$(\overline{\mathbf{4}},\mathbf{2},\mathbf{1},\mathbf{1})$, $(0,0,1,1,0,0) \mapsto (L,Q)$
$(\overline{\mathbf{4}},\mathbf{2},\mathbf{1},\mathbf{1})$, $(0,0,1,1,0,0) \mapsto (L,Q)$
$(\mathbf{4},\mathbf{1},\mathbf{2},\mathbf{1})$, $(1,0,0,0,1,0) \mapsto (D,E,N,U)$
$(\mathbf{4},\mathbf{1},\mathbf{1},\mathbf{2})$, $(1,0,0,0,0,1) \mapsto (D,E,N,U)$
Projection matrix for $\alpha$:

$$\begin{pmatrix} 0 & 1 & 0 & 0 & 0 & 0 \\ 1 & 0 & 0 & 0 & 0 & 0 \\ 0 & 0 & 0 & 1 & 0 & 0 \\ -1 & -2 & -3 & 0 & 3 & 3 \end{pmatrix}$$

**2 generation subalgebra** 35
Algebra: $\mathfrak{su}(4) \oplus \mathfrak{su}(2) \oplus \mathfrak{su}(2) \oplus \mathfrak{su}(2)$
$(\overline{\mathbf{4}},\mathbf{2},\mathbf{1},\mathbf{1})$, $(0,0,1,1,0,0) \mapsto (D,E,N,U)$

$(\overline{\mathbf{4}}, \mathbf{2}, \mathbf{1}, \mathbf{1})$, $(0,0,1,1,0,0) \mapsto (D,E,N,U)$
$(\mathbf{4}, \mathbf{1}, \mathbf{2}, \mathbf{1})$, $(1,0,0,0,1,0) \mapsto (L,Q)$
$(\mathbf{4}, \mathbf{1}, \mathbf{1}, \mathbf{2})$, $(1,0,0,0,0,1) \mapsto (L,Q)$
Projection matrix for $\alpha$:

$$\begin{pmatrix} 1 & 0 & 0 & 0 & 0 & 0 \\ 0 & 1 & 0 & 0 & 0 & 0 \\ 0 & 0 & 0 & 0 & 1 & 1 \\ 1 & 2 & 3 & 3 & 0 & 0 \end{pmatrix}$$

**2 generation subalgebra** 36
Algebra: $\mathfrak{su}(4) \oplus \mathfrak{su}(4) \oplus \mathfrak{su}(2) \oplus \mathfrak{su}(2)$
$(\overline{\mathbf{4}}, \mathbf{1}, \mathbf{2}, \mathbf{1})$, $(0,0,1,0,0,0,1,0) \mapsto (L,Q)$
$(\mathbf{1}, \overline{\mathbf{4}}, \mathbf{2}, \mathbf{1})$, $(0,0,0,0,0,1,1,0) \mapsto (L,Q)$
$(\mathbf{4}, \mathbf{1}, \mathbf{1}, \mathbf{2})$, $(1,0,0,0,0,0,0,1) \mapsto (D,E,N,U)$
$(\mathbf{1}, \mathbf{4}, \mathbf{1}, \mathbf{2})$, $(0,0,0,1,0,0,0,1) \mapsto (D,E,N,U)$
Projection matrix for $\alpha$:

$$\begin{pmatrix} 0 & 1 & 0 & 0 & 1 & 0 & 0 & 0 \\ 1 & 0 & 0 & 1 & 0 & 0 & 0 & 0 \\ 0 & 0 & 0 & 0 & 0 & 0 & 1 & 0 \\ -1 & -2 & -3 & -1 & -2 & -3 & 0 & 3 \end{pmatrix}$$

**2 generation subalgebra** 37
Algebra: $\mathfrak{su}(4) \oplus \mathfrak{su}(5) \oplus \mathfrak{su}(2) \oplus \mathfrak{su}(2)$
$(\mathbf{1}, \overline{\mathbf{5}}, \mathbf{1}, \mathbf{1})$, $(0,0,0,0,0,0,1,0,0) \mapsto (D,L)$
$(\mathbf{1}, \mathbf{10}, \mathbf{1}, \mathbf{1})$, $(0,0,0,0,1,0,0,0,0) \mapsto (E,Q,U)$
$(\overline{\mathbf{4}}, \mathbf{1}, \mathbf{2}, \mathbf{1})$, $(0,0,1,0,0,0,0,1,0) \mapsto (L,Q)$
$(\mathbf{4}, \mathbf{1}, \mathbf{1}, \mathbf{2})$, $(1,0,0,0,0,0,0,0,1) \mapsto (D,E,N,U)$
$(\mathbf{1}, \mathbf{1}, \mathbf{1}, \mathbf{1})$, $(0,0,0,0,0,0,0,0,0) \mapsto (N)$
Projection matrix for $\alpha$:

$$\begin{pmatrix} 0 & 1 & 0 & 0 & 0 & 1 & 0 & 0 & 0 \\ 1 & 0 & 0 & 0 & 0 & 0 & 1 & 0 & 0 \\ 0 & 0 & 0 & 1 & 0 & 0 & 0 & 1 & 0 \\ -1 & -2 & -3 & 3 & 6 & 4 & 2 & 0 & 3 \end{pmatrix}$$

**2 generation subalgebra** 38
Algebra: $\mathfrak{su}(5) \oplus \mathfrak{su}(2) \oplus \mathfrak{su}(2) \oplus \mathfrak{su}(2)$
$(\overline{\mathbf{5}}, \mathbf{2}, \mathbf{1}, \mathbf{1})$, $(0,0,0,1,1,0,0) \mapsto (D,D,L,L)$
$(\mathbf{10}, \mathbf{1}, \mathbf{2}, \mathbf{1})$, $(0,1,0,0,0,1,0) \mapsto (E,E,Q,Q,U,U)$
$(\mathbf{1}, \mathbf{1}, \mathbf{1}, \mathbf{2})$, $(0,0,0,0,0,0,1) \mapsto (N,N)$
Projection matrix for $\alpha$:

$$\begin{pmatrix} 0 & 0 & 1 & 0 & 0 & 0 & 0 \\ 0 & 0 & 0 & 1 & 0 & 0 & 0 \\ 1 & 0 & 0 & 0 & 0 & 0 & 0 \\ 3 & 6 & 4 & 2 & 0 & 0 & 0 \end{pmatrix}$$

**2 generation subalgebra** 39
Algebra: $\mathfrak{su}(4) \oplus \mathfrak{su}(2) \oplus \mathfrak{su}(2) \oplus \mathfrak{su}(2) \oplus \mathfrak{su}(2)$
$(\mathbf{4}, \mathbf{2}, \mathbf{2}, \mathbf{1}, \mathbf{1})$, $(1,0,0,1,1,0,0) \mapsto (L,L,Q,Q)$
$(\overline{\mathbf{4}}, \mathbf{1}, \mathbf{1}, \mathbf{2}, \mathbf{2})$, $(0,0,1,0,0,1,1) \mapsto (D,D,E,E,N,N,U,U)$
Projection matrix for $\alpha$:

$$\begin{pmatrix} 1 & 0 & 0 & 0 & 0 & 0 & 0 \\ 0 & 1 & 0 & 0 & 0 & 0 & 0 \\ 0 & 0 & 0 & 1 & 0 & 0 & 0 \\ 1 & 2 & 3 & 0 & 0 & 3 & 0 \end{pmatrix}$$

**2 generation subalgebra** 40
Algebra: $\mathfrak{su}(4) \oplus \mathfrak{su}(2) \oplus \mathfrak{su}(2) \oplus \mathfrak{su}(2) \oplus \mathfrak{su}(2)$

$(\mathbf{4},\mathbf{2},\mathbf{2},\mathbf{1},\mathbf{1}),\ (1,0,0,1,1,0,0) \mapsto (D,D,E,E,N,N,U,U)$
$(\bar{\mathbf{4}},\mathbf{1},\mathbf{1},\mathbf{2},\mathbf{1}),\ (0,0,1,0,0,1,0) \mapsto (L,Q)$
$(\bar{\mathbf{4}},\mathbf{1},\mathbf{1},\mathbf{1},\mathbf{2}),\ (0,0,1,0,0,0,1) \mapsto (L,Q)$
Projection matrix for $\alpha$:

$$\begin{pmatrix} 0 & 1 & 0 & 0 & 0 & 0 & 0 \\ 1 & 0 & 0 & 0 & 0 & 0 & 0 \\ 0 & 0 & 0 & 0 & 0 & 1 & 1 \\ -1 & -2 & -3 & 3 & 0 & 0 & 0 \end{pmatrix}$$

**2 generation subalgebra** 41
Algebra: $\mathfrak{su}(4) \oplus \mathfrak{su}(2) \oplus \mathfrak{su}(2) \oplus \mathfrak{su}(2) \oplus \mathfrak{su}(2)$
$(\mathbf{4},\mathbf{2},\mathbf{2},\mathbf{1},\mathbf{1}),\ (1,0,0,1,1,0,0) \mapsto (L,L,Q,Q)$
$(\bar{\mathbf{4}},\mathbf{1},\mathbf{1},\mathbf{2},\mathbf{1}),\ (0,0,1,0,0,1,0) \mapsto (D,E,N,U)$
$(\bar{\mathbf{4}},\mathbf{1},\mathbf{1},\mathbf{1},\mathbf{2}),\ (0,0,1,0,0,0,1) \mapsto (D,E,N,U)$
Projection matrix for $\alpha$:

$$\begin{pmatrix} 1 & 0 & 0 & 0 & 0 & 0 & 0 \\ 0 & 1 & 0 & 0 & 0 & 0 & 0 \\ 0 & 0 & 0 & 1 & 0 & 0 & 0 \\ 1 & 2 & 3 & 0 & 0 & 3 & 3 \end{pmatrix}$$

**2 generation subalgebra** 42
Algebra: $\mathfrak{su}(4) \oplus \mathfrak{su}(2) \oplus \mathfrak{su}(2) \oplus \mathfrak{su}(2) \oplus \mathfrak{su}(2)$
$(\bar{\mathbf{4}},\mathbf{2},\mathbf{1},\mathbf{1},\mathbf{1}),\ (0,0,1,1,0,0,0) \mapsto (L,Q)$
$(\bar{\mathbf{4}},\mathbf{1},\mathbf{2},\mathbf{1},\mathbf{1}),\ (0,0,1,0,1,0,0) \mapsto (L,Q)$
$(\mathbf{4},\mathbf{1},\mathbf{1},\mathbf{2},\mathbf{1}),\ (1,0,0,0,0,1,0) \mapsto (D,E,N,U)$
$(\mathbf{4},\mathbf{1},\mathbf{1},\mathbf{1},\mathbf{2}),\ (1,0,0,0,0,0,1) \mapsto (D,E,N,U)$
Projection matrix for $\alpha$:

$$\begin{pmatrix} 0 & 1 & 0 & 0 & 0 & 0 & 0 \\ 1 & 0 & 0 & 0 & 0 & 0 & 0 \\ 0 & 0 & 0 & 1 & 1 & 0 & 0 \\ -1 & -2 & -3 & 0 & 0 & 3 & 3 \end{pmatrix}$$

**2 generation subalgebra** 43
Algebra: $\mathfrak{su}(4) \oplus \mathfrak{su}(4) \oplus \mathfrak{su}(2) \oplus \mathfrak{su}(2) \oplus \mathfrak{su}(2)$
$(\bar{\mathbf{4}},\mathbf{1},\mathbf{2},\mathbf{1},\mathbf{1}),\ (0,0,1,0,0,0,1,0,0) \mapsto (L,Q)$
$(\mathbf{1},\bar{\mathbf{4}},\mathbf{2},\mathbf{1},\mathbf{1}),\ (0,0,0,0,0,1,1,0,0) \mapsto (L,Q)$
$(\mathbf{4},\mathbf{1},\mathbf{1},\mathbf{2},\mathbf{1}),\ (1,0,0,0,0,0,0,1,0) \mapsto (D,E,N,U)$
$(\mathbf{1},\mathbf{4},\mathbf{1},\mathbf{1},\mathbf{2}),\ (0,0,0,1,0,0,0,0,1) \mapsto (D,E,N,U)$
Projection matrix for $\alpha$:

$$\begin{pmatrix} 0 & 1 & 0 & 0 & 1 & 0 & 0 & 0 & 0 \\ 1 & 0 & 0 & 1 & 0 & 0 & 0 & 0 & 0 \\ 0 & 0 & 0 & 0 & 0 & 0 & 1 & 0 & 0 \\ -1 & -2 & -3 & -1 & -2 & -3 & 0 & 3 & 3 \end{pmatrix}$$

**2 generation subalgebra** 44
Algebra: $\mathfrak{su}(4) \oplus \mathfrak{su}(4) \oplus \mathfrak{su}(2) \oplus \mathfrak{su}(2) \oplus \mathfrak{su}(2)$
$(\bar{\mathbf{4}},\mathbf{1},\mathbf{2},\mathbf{1},\mathbf{1}),\ (0,0,1,0,0,0,1,0,0) \mapsto (D,E,N,U)$
$(\mathbf{1},\bar{\mathbf{4}},\mathbf{2},\mathbf{1},\mathbf{1}),\ (0,0,0,0,0,1,1,0,0) \mapsto (D,E,N,U)$
$(\mathbf{4},\mathbf{1},\mathbf{1},\mathbf{2},\mathbf{1}),\ (1,0,0,0,0,0,0,1,0) \mapsto (L,Q)$
$(\mathbf{1},\mathbf{4},\mathbf{1},\mathbf{1},\mathbf{2}),\ (0,0,0,1,0,0,0,0,1) \mapsto (L,Q)$
Projection matrix for $\alpha$:

$$\begin{pmatrix} 1 & 0 & 0 & 1 & 0 & 0 & 0 & 0 & 0 \\ 0 & 1 & 0 & 0 & 1 & 0 & 0 & 0 & 0 \\ 0 & 0 & 0 & 0 & 0 & 0 & 0 & 1 & 1 \\ 1 & 2 & 3 & 1 & 2 & 3 & 3 & 0 & 0 \end{pmatrix}$$

**2 generation subalgebra** 45
Algebra: $\mathfrak{su}(4) \oplus \mathfrak{su}(4) \oplus \mathfrak{su}(2) \oplus \mathfrak{su}(2) \oplus \mathfrak{su}(2) \oplus \mathfrak{su}(2)$
$(\overline{\mathbf{4}}, \mathbf{1}, \mathbf{2}, \mathbf{1}, \mathbf{1}, \mathbf{1})$, $(0,0,1,0,0,0,1,0,0,0) \mapsto (L, Q)$
$(\mathbf{4}, \mathbf{1}, \mathbf{1}, \mathbf{2}, \mathbf{1}, \mathbf{1})$, $(1,0,0,0,0,0,0,1,0,0) \mapsto (D, E, N, U)$
$(\mathbf{1}, \overline{\mathbf{4}}, \mathbf{1}, \mathbf{1}, \mathbf{2}, \mathbf{1})$, $(0,0,0,0,0,1,0,0,1,0) \mapsto (L, Q)$
$(\mathbf{1}, \mathbf{4}, \mathbf{1}, \mathbf{1}, \mathbf{1}, \mathbf{2})$, $(0,0,0,1,0,0,0,0,0,1) \mapsto (D, E, N, U)$
Projection matrix for $\alpha$:

$$\begin{pmatrix} 0 & 1 & 0 & 0 & 1 & 0 & 0 & 0 & 0 & 0 \\ 1 & 0 & 0 & 1 & 0 & 0 & 0 & 0 & 0 & 0 \\ 0 & 0 & 0 & 0 & 0 & 0 & 1 & 0 & 1 & 0 \\ -1 & -2 & -3 & -1 & -2 & -3 & 0 & 3 & 0 & 3 \end{pmatrix}$$

## C. 3 generation maximal algebras

**3 generation subalgebra** 1
Algebra: $\mathfrak{so}(10) \oplus \mathfrak{su}(2)$
$(\mathbf{16}, \mathbf{3})$, $(0,0,0,0,1,2) \mapsto (D, D, D, E, E, E, L, L, L, N, N, N, Q, Q, Q, U, U, U)$
Projection matrix for $\alpha$:

$$\begin{pmatrix} 0 & 0 & 1 & 0 & 0 & 0 \\ 0 & 0 & 0 & 0 & 1 & 0 \\ 1 & 0 & 0 & 0 & 0 & 0 \\ 3 & 6 & 4 & 0 & 2 & 0 \end{pmatrix}$$

**3 generation subalgebra** 2
Algebra: $\mathfrak{so}(10) \oplus \mathfrak{so}(10) \oplus \mathfrak{so}(10)$
$(\mathbf{16}, \mathbf{1}, \mathbf{1})$, $(0,0,0,0,1,0,0,0,0,0,0,0,0,0,0) \mapsto (D, E, L, N, Q, U)$
$(\mathbf{1}, \mathbf{16}, \mathbf{1})$, $(0,0,0,0,0,0,0,0,0,1,0,0,0,0,0) \mapsto (D, E, L, N, Q, U)$
$(\mathbf{1}, \mathbf{1}, \mathbf{16})$, $(0,0,0,0,0,0,0,0,0,0,0,0,0,0,1) \mapsto (D, E, L, N, Q, U)$
Projection matrix for $\alpha$:

$$\begin{pmatrix} 0 & 0 & 1 & 0 & 0 & 0 & 0 & 1 & 0 & 0 & 0 & 0 & 1 & 0 & 0 \\ 0 & 0 & 0 & 0 & 1 & 0 & 0 & 0 & 0 & 1 & 0 & 0 & 0 & 0 & 1 \\ 1 & 0 & 0 & 0 & 0 & 1 & 0 & 0 & 0 & 0 & 1 & 0 & 0 & 0 & 0 \\ 3 & 6 & 4 & 0 & 2 & 3 & 6 & 4 & 0 & 2 & 3 & 6 & 4 & 0 & 2 \end{pmatrix}$$

**3 generation subalgebra** 3
Algebra: $\mathfrak{so}(10) \oplus \mathfrak{so}(10) \oplus \mathfrak{su}(2)$
$(\mathbf{16}, \mathbf{1}, \mathbf{1})$, $(0,0,0,0,1,0,0,0,0,0,0) \mapsto (D, E, L, N, Q, U)$
$(\mathbf{1}, \mathbf{16}, \mathbf{2})$, $(0,0,0,0,0,0,0,0,0,1,1) \mapsto (D, D, E, E, L, L, N, N, Q, Q, U, U)$
Projection matrix for $\alpha$:

$$\begin{pmatrix} 0 & 0 & 1 & 0 & 0 & 0 & 0 & 1 & 0 & 0 & 0 \\ 0 & 0 & 0 & 0 & 1 & 0 & 0 & 0 & 0 & 1 & 0 \\ 1 & 0 & 0 & 0 & 0 & 1 & 0 & 0 & 0 & 0 & 0 \\ 3 & 6 & 4 & 0 & 2 & 3 & 6 & 4 & 0 & 2 & 0 \end{pmatrix}$$

**3 generation subalgebra** 4
Algebra: $\mathfrak{su}(4) \oplus \mathfrak{sp}(6) \oplus \mathfrak{sp}(6)$
$(\overline{\mathbf{4}}, \mathbf{6}, \mathbf{1})$, $(0,0,1,1,0,0,0,0,0) \mapsto (L, L, L, Q, Q, Q)$
$(\mathbf{4}, \mathbf{1}, \mathbf{6})$, $(1,0,0,0,0,0,1,0,0) \mapsto (D, D, D, E, E, E, N, N, N, U, U, U)$
Projection matrix for $\alpha$:

$$\begin{pmatrix} 0 & 1 & 0 & 0 & 0 & 0 & 0 & 0 & 0 \\ 1 & 0 & 0 & 0 & 0 & 0 & 0 & 0 & 0 \\ 0 & 0 & 0 & 1 & 2 & 3 & 0 & 0 & 0 \\ -1 & -2 & -3 & 0 & 0 & 0 & 3 & 0 & -3 \end{pmatrix}$$

**3 generation subalgebra** 5
Algebra: $\mathfrak{su}(4) \oplus \mathfrak{su}(4) \oplus \mathfrak{sp}(6)$
$(\overline{\mathbf{4}}, \mathbf{6}, \mathbf{1})$, $(0,0,1,0,1,0,0,0,0) \mapsto (D,D,D,E,E,E,N,N,N,U,U,U)$
$(\mathbf{4}, \mathbf{1}, \mathbf{6})$, $(1,0,0,0,0,0,1,0,0) \mapsto (L,L,L,Q,Q,Q)$
Projection matrix for $\alpha$:

$$\begin{pmatrix} 1 & 0 & 0 & 0 & 0 & 0 & 0 & 0 & 0 \\ 0 & 1 & 0 & 0 & 0 & 0 & 0 & 0 & 0 \\ 0 & 0 & 0 & 0 & 0 & 0 & 1 & 2 & 3 \\ 1 & 2 & 3 & \frac{9}{2} & 3 & \frac{3}{2} & 0 & 0 & 0 \end{pmatrix}$$

**3 generation subalgebra** 6
Algebra: $\mathfrak{su}(12) \oplus \mathfrak{su}(2) \oplus \mathfrak{su}(2)$
$(\overline{\mathbf{12}}, \mathbf{2}, \mathbf{1})$, $(0,0,0,0,0,0,0,0,0,0,1,1,0) \mapsto (L,L,L,Q,Q,Q)$
$(\mathbf{12}, \mathbf{1}, \mathbf{2})$, $(1,0,0,0,0,0,0,0,0,0,0,0,1) \mapsto (D,D,D,E,E,E,N,N,N,U,U,U)$
Projection matrix for $\alpha$:

$$\begin{pmatrix} 0 & 1 & 0 & 0 & 1 & 0 & 0 & 1 & 0 & 0 & 0 & 0 & 0 \\ 1 & 0 & 0 & 1 & 0 & 0 & 1 & 0 & 0 & 0 & 0 & 0 & 0 \\ 0 & 0 & 0 & 0 & 0 & 0 & 0 & 0 & 0 & 0 & 0 & 1 & 0 \\ -1 & -2 & -3 & -4 & -5 & -6 & -7 & -8 & -9 & -6 & -3 & 0 & 3 \end{pmatrix}$$

**3 generation subalgebra** 7
Algebra: $\mathfrak{su}(4) \oplus \mathfrak{sp}(4) \oplus \mathfrak{sp}(4) \oplus \mathfrak{so}(10)$
$(\overline{\mathbf{4}}, \mathbf{4}, \mathbf{1}, \mathbf{1})$, $(0,0,1,1,0,0,0,0,0,0,0,0,0) \mapsto (L,L,Q,Q)$
$(\mathbf{4}, \mathbf{1}, \mathbf{4}, \mathbf{1})$, $(1,0,0,0,0,1,0,0,0,0,0,0,0) \mapsto (D,D,E,E,N,N,U,U)$
$(\mathbf{1}, \mathbf{1}, \mathbf{1}, \mathbf{16})$, $(0,0,0,0,0,0,0,0,0,0,0,0,1) \mapsto (D,E,L,N,Q,U)$
Projection matrix for $\alpha$:

$$\begin{pmatrix} 0 & 1 & 0 & 0 & 0 & 0 & 0 & 0 & 0 & 1 & 0 & 0 \\ 1 & 0 & 0 & 0 & 0 & 0 & 0 & 0 & 0 & 0 & 0 & 1 \\ 0 & 0 & 0 & 1 & 2 & 0 & 0 & 1 & 0 & 0 & 0 & 0 \\ -1 & -2 & -3 & 0 & 0 & 3 & 0 & 3 & 6 & 4 & 0 & 2 \end{pmatrix}$$

**3 generation subalgebra** 8
Algebra: $\mathfrak{su}(5) \oplus \mathfrak{su}(2) \oplus \mathfrak{su}(2) \oplus \mathfrak{su}(2)$
$(\overline{\mathbf{5}}, \mathbf{3}, \mathbf{1}, \mathbf{1})$, $(0,0,0,1,2,0,0) \mapsto (D,D,D,L,L,L)$
$(\mathbf{10}, \mathbf{1}, \mathbf{3}, \mathbf{1})$, $(0,1,0,0,0,2,0) \mapsto (E,E,E,Q,Q,Q,U,U,U)$
$(\mathbf{1}, \mathbf{1}, \mathbf{1}, \mathbf{2})$, $(0,0,0,0,0,0,1) \mapsto (N,N)$
$(\mathbf{1}, \mathbf{1}, \mathbf{1}, \mathbf{1})$, $(0,0,0,0,0,0,0) \mapsto (N)$
Projection matrix for $\alpha$:

$$\begin{pmatrix} 0 & 0 & 1 & 0 & 0 & 0 & 0 \\ 0 & 0 & 0 & 1 & 0 & 0 & 0 \\ 1 & 0 & 0 & 0 & 0 & 0 & 0 \\ 3 & 6 & 4 & 2 & 0 & 0 & 0 \end{pmatrix}$$

**3 generation subalgebra** 9
Algebra: $\mathfrak{su}(5) \oplus \mathfrak{su}(2) \oplus \mathfrak{su}(2) \oplus \mathfrak{su}(2)$
$(\overline{\mathbf{5}}, \mathbf{3}, \mathbf{1}, \mathbf{1})$, $(0,0,0,1,2,0,0) \mapsto (D,D,D,L,L,L)$
$(\mathbf{10}, \mathbf{1}, \mathbf{3}, \mathbf{1})$, $(0,1,0,0,0,2,0) \mapsto (E,E,E,Q,Q,Q,U,U,U)$
$(\mathbf{1}, \mathbf{1}, \mathbf{1}, \mathbf{3})$, $(0,0,0,0,0,0,2) \mapsto (N,N,N)$
Projection matrix for $\alpha$:

$$\begin{pmatrix} 0 & 0 & 1 & 0 & 0 & 0 & 0 \\ 0 & 0 & 0 & 1 & 0 & 0 & 0 \\ 1 & 0 & 0 & 0 & 0 & 0 & 0 \\ 3 & 6 & 4 & 2 & 0 & 0 & 0 \end{pmatrix}$$

**3 generation subalgebra** 10
Algebra: $\mathfrak{su}(5) \oplus \mathfrak{su}(2) \oplus \mathfrak{su}(2) \oplus \mathfrak{su}(2)$

$(\overline{\mathbf{5}}, \mathbf{1}, \mathbf{1}, \mathbf{1})$, $(0,0,0,1,0,0,0) \mapsto (D, L)$
$(\overline{\mathbf{5}}, \mathbf{2}, \mathbf{1}, \mathbf{1})$, $(0,0,0,1,1,0,0) \mapsto (D, D, L, L)$
$(\mathbf{10}, \mathbf{1}, \mathbf{3}, \mathbf{1})$, $(0,1,0,0,0,2,0) \mapsto (E, E, E, Q, Q, Q, U, U, U)$
$(\mathbf{1}, \mathbf{1}, \mathbf{1}, \mathbf{2})$, $(0,0,0,0,0,0,1) \mapsto (N, N)$
$(\mathbf{1}, \mathbf{1}, \mathbf{1}, \mathbf{1})$, $(0,0,0,0,0,0,0) \mapsto (N)$
Projection matrix for $\alpha$:

$$\begin{pmatrix} 0 & 0 & 1 & 0 & 0 & 0 & 0 \\ 0 & 0 & 0 & 1 & 0 & 0 & 0 \\ 1 & 0 & 0 & 0 & 0 & 0 & 0 \\ 3 & 6 & 4 & 2 & 0 & 0 & 0 \end{pmatrix}$$

**3 generation subalgebra** 11
Algebra: $\mathfrak{su}(5) \oplus \mathfrak{su}(2) \oplus \mathfrak{su}(2) \oplus \mathfrak{su}(2)$
$(\overline{\mathbf{5}}, \mathbf{1}, \mathbf{1}, \mathbf{1})$, $(0,0,0,1,0,0,0) \mapsto (D, L)$
$(\overline{\mathbf{5}}, \mathbf{2}, \mathbf{1}, \mathbf{1})$, $(0,0,0,1,1,0,0) \mapsto (D, D, L, L)$
$(\mathbf{10}, \mathbf{1}, \mathbf{3}, \mathbf{1})$, $(0,1,0,0,0,2,0) \mapsto (E, E, E, Q, Q, Q, U, U, U)$
$(\mathbf{1}, \mathbf{1}, \mathbf{1}, \mathbf{3})$, $(0,0,0,0,0,0,2) \mapsto (N, N, N)$
Projection matrix for $\alpha$:

$$\begin{pmatrix} 0 & 0 & 1 & 0 & 0 & 0 & 0 \\ 0 & 0 & 0 & 1 & 0 & 0 & 0 \\ 1 & 0 & 0 & 0 & 0 & 0 & 0 \\ 3 & 6 & 4 & 2 & 0 & 0 & 0 \end{pmatrix}$$

**3 generation subalgebra** 12
Algebra: $\mathfrak{su}(5) \oplus \mathfrak{su}(2) \oplus \mathfrak{su}(2) \oplus \mathfrak{su}(2)$
$(\mathbf{10}, \mathbf{1}, \mathbf{1}, \mathbf{1})$, $(0,1,0,0,0,0,0) \mapsto (E, Q, U)$
$(\overline{\mathbf{5}}, \mathbf{3}, \mathbf{1}, \mathbf{1})$, $(0,0,0,1,2,0,0) \mapsto (D, D, D, L, L, L)$
$(\mathbf{10}, \mathbf{1}, \mathbf{2}, \mathbf{1})$, $(0,1,0,0,0,1,0) \mapsto (E, E, Q, Q, U, U)$
$(\mathbf{1}, \mathbf{1}, \mathbf{1}, \mathbf{2})$, $(0,0,0,0,0,0,1) \mapsto (N, N)$
$(\mathbf{1}, \mathbf{1}, \mathbf{1}, \mathbf{1})$, $(0,0,0,0,0,0,0) \mapsto (N)$
Projection matrix for $\alpha$:

$$\begin{pmatrix} 0 & 0 & 1 & 0 & 0 & 0 & 0 \\ 0 & 0 & 0 & 1 & 0 & 0 & 0 \\ 1 & 0 & 0 & 0 & 0 & 0 & 0 \\ 3 & 6 & 4 & 2 & 0 & 0 & 0 \end{pmatrix}$$

**3 generation subalgebra** 13
Algebra: $\mathfrak{su}(5) \oplus \mathfrak{su}(2) \oplus \mathfrak{su}(2) \oplus \mathfrak{su}(2)$
$(\mathbf{10}, \mathbf{1}, \mathbf{1}, \mathbf{1})$, $(0,1,0,0,0,0,0) \mapsto (E, Q, U)$
$(\overline{\mathbf{5}}, \mathbf{3}, \mathbf{1}, \mathbf{1})$, $(0,0,0,1,2,0,0) \mapsto (D, D, D, L, L, L)$
$(\mathbf{10}, \mathbf{1}, \mathbf{2}, \mathbf{1})$, $(0,1,0,0,0,1,0) \mapsto (E, E, Q, Q, U, U)$
$(\mathbf{1}, \mathbf{1}, \mathbf{1}, \mathbf{3})$, $(0,0,0,0,0,0,2) \mapsto (N, N, N)$
Projection matrix for $\alpha$:

$$\begin{pmatrix} 0 & 0 & 1 & 0 & 0 & 0 & 0 \\ 0 & 0 & 0 & 1 & 0 & 0 & 0 \\ 1 & 0 & 0 & 0 & 0 & 0 & 0 \\ 3 & 6 & 4 & 2 & 0 & 0 & 0 \end{pmatrix}$$

**3 generation subalgebra** 14
Algebra: $\mathfrak{su}(5) \oplus \mathfrak{su}(5) \oplus \mathfrak{so}(10) \oplus \mathfrak{su}(2)$
$(\overline{\mathbf{5}}, \mathbf{1}, \mathbf{1}, \mathbf{1})$, $(0,0,0,1,0,0,0,0,0,0,0,0,0,0) \mapsto (D, L)$
$(\mathbf{10}, \mathbf{1}, \mathbf{1}, \mathbf{1})$, $(0,1,0,0,0,0,0,0,0,0,0,0,0,0) \mapsto (E, Q, U)$
$(\mathbf{1}, \overline{\mathbf{5}}, \mathbf{1}, \mathbf{1})$, $(0,0,0,0,0,0,0,1,0,0,0,0,0,0) \mapsto (D, L)$
$(\mathbf{1}, \mathbf{10}, \mathbf{1}, \mathbf{1})$, $(0,0,0,0,0,1,0,0,0,0,0,0,0,0) \mapsto (E, Q, U)$
$(\mathbf{1}, \mathbf{1}, \mathbf{16}, \mathbf{1})$, $(0,0,0,0,0,0,0,0,0,0,0,0,1,0) \mapsto (D, E, L, N, Q, U)$

$(\mathbf{1},\mathbf{1},\mathbf{1},\mathbf{2})$, $(0,0,0,0,0,0,0,0,0,0,0,0,0,1) \mapsto (N,N)$
Projection matrix for $\alpha$:

$$\begin{pmatrix} 0 & 0 & 1 & 0 & 0 & 0 & 1 & 0 & 0 & 0 & 1 & 0 & 0 & 0 \\ 0 & 0 & 0 & 1 & 0 & 0 & 0 & 1 & 0 & 0 & 0 & 0 & 1 & 0 \\ 1 & 0 & 0 & 0 & 1 & 0 & 0 & 0 & 1 & 0 & 0 & 0 & 0 & 0 \\ 3 & 6 & 4 & 2 & 3 & 6 & 4 & 2 & 3 & 6 & 4 & 0 & 2 & 0 \end{pmatrix}$$

**3 generation subalgebra** 15
Algebra: $\mathfrak{su}(5) \oplus \mathfrak{su}(5) \oplus \mathfrak{su}(5) \oplus \mathfrak{su}(2)$
$(\overline{\mathbf{5}},\mathbf{1},\mathbf{1},\mathbf{1})$, $(0,0,0,1,0,0,0,0,0,0,0,0,0) \mapsto (D,L)$
$(\mathbf{10},\mathbf{1},\mathbf{1},\mathbf{1})$, $(0,1,0,0,0,0,0,0,0,0,0,0,0) \mapsto (E,Q,U)$
$(\mathbf{1},\overline{\mathbf{5}},\mathbf{1},\mathbf{1})$, $(0,0,0,0,0,0,0,1,0,0,0,0,0) \mapsto (D,L)$
$(\mathbf{1},\mathbf{10},\mathbf{1},\mathbf{1})$, $(0,0,0,0,0,1,0,0,0,0,0,0,0) \mapsto (E,Q,U)$
$(\mathbf{1},\mathbf{1},\overline{\mathbf{5}},\mathbf{1})$, $(0,0,0,0,0,0,0,0,0,0,0,1,0) \mapsto (D,L)$
$(\mathbf{1},\mathbf{1},\mathbf{10},\mathbf{1})$, $(0,0,0,0,0,0,0,0,0,1,0,0,0) \mapsto (E,Q,U)$
$(\mathbf{1},\mathbf{1},\mathbf{1},\mathbf{3})$, $(0,0,0,0,0,0,0,0,0,0,0,0,2) \mapsto (N,N,N)$
Projection matrix for $\alpha$:

$$\begin{pmatrix} 0 & 0 & 1 & 0 & 0 & 0 & 1 & 0 & 0 & 0 & 1 & 0 & 0 \\ 0 & 0 & 0 & 1 & 0 & 0 & 0 & 1 & 0 & 0 & 0 & 1 & 0 \\ 1 & 0 & 0 & 0 & 1 & 0 & 0 & 0 & 1 & 0 & 0 & 0 & 0 \\ 3 & 6 & 4 & 2 & 3 & 6 & 4 & 2 & 3 & 6 & 4 & 2 & 0 \end{pmatrix}$$

**3 generation subalgebra** 16
Algebra: $\mathfrak{su}(8) \oplus \mathfrak{so}(10) \oplus \mathfrak{su}(2) \oplus \mathfrak{su}(2)$
$(\mathbf{1},\mathbf{16},\mathbf{1},\mathbf{1})$, $(0,0,0,0,0,0,0,0,0,0,0,1,0,0) \mapsto (D,E,L,N,Q,U)$
$(\overline{\mathbf{8}},\mathbf{1},\mathbf{2},\mathbf{1})$, $(0,0,0,0,0,0,1,0,0,0,0,0,1,0) \mapsto (L,L,Q,Q)$
$(\mathbf{8},\mathbf{1},\mathbf{1},\mathbf{2})$, $(1,0,0,0,0,0,0,0,0,0,0,0,0,1) \mapsto (D,D,E,E,N,N,U,U)$
Projection matrix for $\alpha$:

$$\begin{pmatrix} 0 & 1 & 0 & 0 & 1 & 0 & 0 & 0 & 0 & 1 & 0 & 0 & 0 & 0 \\ 1 & 0 & 0 & 1 & 0 & 0 & 0 & 0 & 0 & 0 & 0 & 1 & 0 & 0 \\ 0 & 0 & 0 & 0 & 0 & 0 & 0 & 1 & 0 & 0 & 0 & 0 & 1 & 0 \\ -1 & -2 & -3 & -4 & -5 & -6 & -3 & 3 & 6 & 4 & 0 & 2 & 0 & 3 \end{pmatrix}$$

**3 generation subalgebra** 17
Algebra: $\mathfrak{su}(4) \oplus \mathfrak{sp}(4) \oplus \mathfrak{so}(10) \oplus \mathfrak{su}(2) \oplus \mathfrak{su}(2)$
$(\overline{\mathbf{4}},\mathbf{4},\mathbf{1},\mathbf{1},\mathbf{1})$, $(0,0,1,1,0,0,0,0,0,0,0,0) \mapsto (L,L,Q,Q)$
$(\mathbf{1},\mathbf{1},\mathbf{16},\mathbf{1},\mathbf{1})$, $(0,0,0,0,0,0,0,0,0,1,0,0) \mapsto (D,E,L,N,Q,U)$
$(\mathbf{4},\mathbf{1},\mathbf{1},\mathbf{2},\mathbf{2})$, $(1,0,0,0,0,0,0,0,0,0,1,1) \mapsto (D,D,E,E,N,N,U,U)$
Projection matrix for $\alpha$:

$$\begin{pmatrix} 0 & 1 & 0 & 0 & 0 & 0 & 0 & 1 & 0 & 0 & 0 & 0 \\ 1 & 0 & 0 & 0 & 0 & 0 & 0 & 0 & 0 & 1 & 0 & 0 \\ 0 & 0 & 0 & 1 & 2 & 1 & 0 & 0 & 0 & 0 & 0 & 0 \\ -1 & -2 & -3 & 0 & 0 & 3 & 6 & 4 & 0 & 2 & 3 & 0 \end{pmatrix}$$

**3 generation subalgebra** 18
Algebra: $\mathfrak{su}(4) \oplus \mathfrak{sp}(4) \oplus \mathfrak{so}(10) \oplus \mathfrak{su}(2) \oplus \mathfrak{su}(2)$
$(\overline{\mathbf{4}},\mathbf{4},\mathbf{1},\mathbf{1},\mathbf{1})$, $(0,0,1,1,0,0,0,0,0,0,0,0) \mapsto (D,D,E,E,N,N,U,U)$
$(\mathbf{1},\mathbf{1},\mathbf{16},\mathbf{1},\mathbf{1})$, $(0,0,0,0,0,0,0,0,0,1,0,0) \mapsto (D,E,L,N,Q,U)$
$(\mathbf{4},\mathbf{1},\mathbf{1},\mathbf{2},\mathbf{2})$, $(1,0,0,0,0,0,0,0,0,0,1,1) \mapsto (L,L,Q,Q)$
Projection matrix for $\alpha$:

$$\begin{pmatrix} 1 & 0 & 0 & 0 & 0 & 0 & 0 & 1 & 0 & 0 & 0 & 0 \\ 0 & 1 & 0 & 0 & 0 & 0 & 0 & 0 & 0 & 1 & 0 & 0 \\ 0 & 0 & 0 & 0 & 0 & 1 & 0 & 0 & 0 & 0 & 1 & 0 \\ 1 & 2 & 3 & 3 & 0 & 3 & 6 & 4 & 0 & 2 & 0 & 0 \end{pmatrix}$$

**3 generation subalgebra** 19
Algebra: $\mathfrak{su}(4) \oplus \mathfrak{sp}(6) \oplus \mathfrak{su}(2) \oplus \mathfrak{su}(2) \oplus \mathfrak{su}(2)$

$(\bar{\mathbf{4}}, \mathbf{6}, \mathbf{1}, \mathbf{1}, \mathbf{1})$, $(0,0,1,1,0,0,0,0,0) \mapsto (L,L,L,Q,Q,Q)$
$(\mathbf{4}, \mathbf{1}, \mathbf{2}, \mathbf{2}, \mathbf{1})$, $(1,0,0,0,0,0,1,1,0) \mapsto (D,D,E,E,N,N,U,U)$
$(\mathbf{4}, \mathbf{1}, \mathbf{1}, \mathbf{1}, \mathbf{2})$, $(1,0,0,0,0,0,0,0,1) \mapsto (D,E,N,U)$
Projection matrix for $\alpha$:

$$\begin{pmatrix} 0 & 1 & 0 & 0 & 0 & 0 & 0 & 0 & 0 \\ 1 & 0 & 0 & 0 & 0 & 0 & 0 & 0 & 0 \\ 0 & 0 & 0 & 1 & 2 & 3 & 0 & 0 & 0 \\ -1 & -2 & -3 & 0 & 0 & 0 & 3 & 0 & 3 \end{pmatrix}$$

**3 generation subalgebra** 20
Algebra: $\mathfrak{su}(4) \oplus \mathfrak{sp}(6) \oplus \mathfrak{su}(2) \oplus \mathfrak{su}(2) \oplus \mathfrak{su}(2)$
$(\bar{\mathbf{4}}, \mathbf{6}, \mathbf{1}, \mathbf{1}, \mathbf{1})$, $(0,0,1,1,0,0,0,0,0) \mapsto (D,D,D,E,E,E,N,N,N,U,U,U)$
$(\mathbf{4}, \mathbf{1}, \mathbf{2}, \mathbf{2}, \mathbf{1})$, $(1,0,0,0,0,0,1,1,0) \mapsto (L,L,Q,Q)$
$(\mathbf{4}, \mathbf{1}, \mathbf{1}, \mathbf{1}, \mathbf{2})$, $(1,0,0,0,0,0,0,0,1) \mapsto (L,Q)$
Projection matrix for $\alpha$:

$$\begin{pmatrix} 1 & 0 & 0 & 0 & 0 & 0 & 0 & 0 & 0 \\ 0 & 1 & 0 & 0 & 0 & 0 & 0 & 0 & 0 \\ 0 & 0 & 0 & 0 & 0 & 0 & 1 & 0 & 1 \\ 1 & 2 & 3 & 3 & 0 & -3 & 0 & 0 & 0 \end{pmatrix}$$

**3 generation subalgebra** 21
Algebra: $\mathfrak{su}(4) \oplus \mathfrak{su}(4) \oplus \mathfrak{su}(2) \oplus \mathfrak{su}(2) \oplus \mathfrak{su}(2)$
$(\bar{\mathbf{4}}, \mathbf{6}, \mathbf{1}, \mathbf{1}, \mathbf{1})$, $(0,0,1,0,1,0,0,0,0) \mapsto (D,D,D,E,E,E,N,N,N,U,U,U)$
$(\mathbf{4}, \mathbf{1}, \mathbf{2}, \mathbf{2}, \mathbf{1})$, $(1,0,0,0,0,0,1,1,0) \mapsto (L,L,Q,Q)$
$(\mathbf{4}, \mathbf{1}, \mathbf{1}, \mathbf{1}, \mathbf{2})$, $(1,0,0,0,0,0,0,0,1) \mapsto (L,Q)$
Projection matrix for $\alpha$:

$$\begin{pmatrix} 1 & 0 & 0 & 0 & 0 & 0 & 0 & 0 & 0 \\ 0 & 1 & 0 & 0 & 0 & 0 & 0 & 0 & 0 \\ 0 & 0 & 0 & 0 & 0 & 0 & 1 & 0 & 1 \\ 1 & 2 & 3 & \frac{9}{2} & 3 & \frac{3}{2} & 0 & 0 & 0 \end{pmatrix}$$

**3 generation subalgebra** 22
Algebra: $\mathfrak{su}(4) \oplus \mathfrak{su}(5) \oplus \mathfrak{su}(5) \oplus \mathfrak{su}(2) \oplus \mathfrak{su}(2)$
$(\mathbf{1}, \bar{\mathbf{5}}, \mathbf{1}, \mathbf{1}, \mathbf{1})$, $(0,0,0,0,0,0,1,0,0,0,0,0,0) \mapsto (D,L)$
$(\mathbf{1}, \mathbf{10}, \mathbf{1}, \mathbf{1}, \mathbf{1})$, $(0,0,0,0,1,0,0,0,0,0,0,0,0) \mapsto (E,Q,U)$
$(\mathbf{1}, \mathbf{1}, \bar{\mathbf{5}}, \mathbf{1}, \mathbf{1})$, $(0,0,0,0,0,0,0,0,0,0,1,0,0) \mapsto (D,L)$
$(\mathbf{1}, \mathbf{1}, \mathbf{10}, \mathbf{1}, \mathbf{1})$, $(0,0,0,0,0,0,0,0,1,0,0,0,0) \mapsto (E,Q,U)$
$(\bar{\mathbf{4}}, \mathbf{1}, \mathbf{1}, \mathbf{2}, \mathbf{1})$, $(0,0,1,0,0,0,0,0,0,0,0,1,0) \mapsto (L,Q)$
$(\mathbf{4}, \mathbf{1}, \mathbf{1}, \mathbf{1}, \mathbf{2})$, $(1,0,0,0,0,0,0,0,0,0,0,0,1) \mapsto (D,E,N,U)$
$(\mathbf{1}, \mathbf{1}, \mathbf{1}, \mathbf{1}, \mathbf{2})$, $(0,0,0,0,0,0,0,0,0,0,0,0,1) \mapsto (N,N)$
Projection matrix for $\alpha$:

$$\begin{pmatrix} 0 & 1 & 0 & 0 & 0 & 1 & 0 & 0 & 0 & 1 & 0 & 0 & 0 \\ 1 & 0 & 0 & 0 & 0 & 0 & 1 & 0 & 0 & 0 & 1 & 0 & 0 \\ 0 & 0 & 0 & 1 & 0 & 0 & 0 & 1 & 0 & 0 & 0 & 1 & 0 \\ -1 & -2 & -3 & 3 & 6 & 4 & 2 & 3 & 6 & 4 & 2 & 0 & 3 \end{pmatrix}$$

**3 generation subalgebra** 23
Algebra: $\mathfrak{su}(4) \oplus \mathfrak{su}(5) \oplus \mathfrak{su}(5) \oplus \mathfrak{su}(2) \oplus \mathfrak{su}(2)$
$(\mathbf{1}, \bar{\mathbf{5}}, \mathbf{1}, \mathbf{1}, \mathbf{1})$, $(0,0,0,0,0,0,1,0,0,0,0,0,0) \mapsto (D,L)$
$(\mathbf{1}, \mathbf{10}, \mathbf{1}, \mathbf{1}, \mathbf{1})$, $(0,0,0,0,1,0,0,0,0,0,0,0,0) \mapsto (E,Q,U)$
$(\mathbf{1}, \mathbf{1}, \bar{\mathbf{5}}, \mathbf{1}, \mathbf{1})$, $(0,0,0,0,0,0,0,0,0,0,1,0,0) \mapsto (D,L)$
$(\mathbf{1}, \mathbf{1}, \mathbf{10}, \mathbf{1}, \mathbf{1})$, $(0,0,0,0,0,0,0,0,1,0,0,0,0) \mapsto (E,Q,U)$
$(\bar{\mathbf{4}}, \mathbf{1}, \mathbf{1}, \mathbf{2}, \mathbf{1})$, $(0,0,1,0,0,0,0,0,0,0,0,1,0) \mapsto (L,Q)$
$(\mathbf{4}, \mathbf{1}, \mathbf{1}, \mathbf{1}, \mathbf{2})$, $(1,0,0,0,0,0,0,0,0,0,0,0,1) \mapsto (D,E,N,U)$
$(\mathbf{1}, \mathbf{1}, \mathbf{1}, \mathbf{2}, \mathbf{1})$, $(0,0,0,0,0,0,0,0,0,0,0,1,0) \mapsto (N,N)$

Projection matrix for $\alpha$:

$$\begin{pmatrix} 0 & 1 & 0 & 0 & 0 & 1 & 0 & 0 & 0 & 1 & 0 & 0 & 0 \\ 1 & 0 & 0 & 0 & 0 & 0 & 1 & 0 & 0 & 0 & 1 & 0 & 0 \\ 0 & 0 & 0 & 1 & 0 & 0 & 0 & 1 & 0 & 0 & 0 & 1 & 0 \\ -1 & -2 & -3 & 3 & 6 & 4 & 2 & 3 & 6 & 4 & 2 & 0 & 3 \end{pmatrix}$$

**3 generation subalgebra** 24
Algebra: $\mathfrak{su}(5) \oplus \mathfrak{so}(10) \oplus \mathfrak{su}(2) \oplus \mathfrak{su}(2) \oplus \mathfrak{su}(2)$
$(\mathbf{1}, \mathbf{16}, \mathbf{1}, \mathbf{1}, \mathbf{1})$, $(0,0,0,0,0,0,0,0,1,0,0,0) \mapsto (D, E, L, N, Q, U)$
$(\overline{\mathbf{5}}, \mathbf{1}, \mathbf{2}, \mathbf{1}, \mathbf{1})$, $(0,0,0,1,0,0,0,0,0,1,0,0) \mapsto (D, D, L, L)$
$(\mathbf{10}, \mathbf{1}, \mathbf{1}, \mathbf{2}, \mathbf{1})$, $(0,1,0,0,0,0,0,0,0,0,1,0) \mapsto (E, E, Q, Q, U, U)$
$(\mathbf{1}, \mathbf{1}, \mathbf{1}, \mathbf{1}, \mathbf{2})$, $(0,0,0,0,0,0,0,0,0,0,0,1) \mapsto (N, N)$
Projection matrix for $\alpha$:

$$\begin{pmatrix} 0 & 0 & 1 & 0 & 0 & 0 & 1 & 0 & 0 & 0 & 0 & 0 \\ 0 & 0 & 0 & 1 & 0 & 0 & 0 & 0 & 1 & 0 & 0 & 0 \\ 1 & 0 & 0 & 0 & 1 & 0 & 0 & 0 & 0 & 0 & 0 & 0 \\ 3 & 6 & 4 & 2 & 3 & 6 & 4 & 0 & 2 & 0 & 0 & 0 \end{pmatrix}$$

**3 generation subalgebra** 25
Algebra: $\mathfrak{su}(5) \oplus \mathfrak{su}(5) \oplus \mathfrak{su}(2) \oplus \mathfrak{su}(2) \oplus \mathfrak{su}(2)$
$(\mathbf{1}, \overline{\mathbf{5}}, \mathbf{1}, \mathbf{1}, \mathbf{1})$, $(0,0,0,0,0,0,0,1,0,0,0) \mapsto (D, L)$
$(\mathbf{1}, \mathbf{10}, \mathbf{1}, \mathbf{1}, \mathbf{1})$, $(0,0,0,0,0,1,0,0,0,0,0) \mapsto (E, Q, U)$
$(\overline{\mathbf{5}}, \mathbf{1}, \mathbf{2}, \mathbf{1}, \mathbf{1})$, $(0,0,0,1,0,0,0,0,1,0,0) \mapsto (D, D, L, L)$
$(\mathbf{10}, \mathbf{1}, \mathbf{1}, \mathbf{2}, \mathbf{1})$, $(0,1,0,0,0,0,0,0,0,1,0) \mapsto (E, E, Q, Q, U, U)$
$(\mathbf{1}, \mathbf{1}, \mathbf{1}, \mathbf{1}, \mathbf{2})$, $(0,0,0,0,0,0,0,0,0,0,1) \mapsto (N, N)$
$(\mathbf{1}, \mathbf{1}, \mathbf{1}, \mathbf{1}, \mathbf{1})$, $(0,0,0,0,0,0,0,0,0,0,0) \mapsto (N)$
Projection matrix for $\alpha$:

$$\begin{pmatrix} 0 & 0 & 1 & 0 & 0 & 0 & 1 & 0 & 0 & 0 & 0 \\ 0 & 0 & 0 & 1 & 0 & 0 & 0 & 1 & 0 & 0 & 0 \\ 1 & 0 & 0 & 0 & 1 & 0 & 0 & 0 & 0 & 0 & 0 \\ 3 & 6 & 4 & 2 & 3 & 6 & 4 & 2 & 0 & 0 & 0 \end{pmatrix}$$

**3 generation subalgebra** 26
Algebra: $\mathfrak{su}(5) \oplus \mathfrak{su}(5) \oplus \mathfrak{su}(2) \oplus \mathfrak{su}(2) \oplus \mathfrak{su}(2)$
$(\mathbf{1}, \overline{\mathbf{5}}, \mathbf{1}, \mathbf{1}, \mathbf{1})$, $(0,0,0,0,0,0,0,1,0,0,0) \mapsto (D, L)$
$(\mathbf{1}, \mathbf{10}, \mathbf{1}, \mathbf{1}, \mathbf{1})$, $(0,0,0,0,0,1,0,0,0,0,0) \mapsto (E, Q, U)$
$(\overline{\mathbf{5}}, \mathbf{1}, \mathbf{2}, \mathbf{1}, \mathbf{1})$, $(0,0,0,1,0,0,0,0,1,0,0) \mapsto (D, D, L, L)$
$(\mathbf{10}, \mathbf{1}, \mathbf{1}, \mathbf{2}, \mathbf{1})$, $(0,1,0,0,0,0,0,0,0,1,0) \mapsto (E, E, Q, Q, U, U)$
$(\mathbf{1}, \mathbf{1}, \mathbf{1}, \mathbf{1}, \mathbf{3})$, $(0,0,0,0,0,0,0,0,0,0,2) \mapsto (N, N, N)$
Projection matrix for $\alpha$:

$$\begin{pmatrix} 0 & 0 & 1 & 0 & 0 & 0 & 1 & 0 & 0 & 0 & 0 \\ 0 & 0 & 0 & 1 & 0 & 0 & 0 & 1 & 0 & 0 & 0 \\ 1 & 0 & 0 & 0 & 1 & 0 & 0 & 0 & 0 & 0 & 0 \\ 3 & 6 & 4 & 2 & 3 & 6 & 4 & 2 & 0 & 0 & 0 \end{pmatrix}$$

**3 generation subalgebra** 27
Algebra: $\mathfrak{su}(4) \oplus \mathfrak{so}(10) \oplus \mathfrak{su}(2) \oplus \mathfrak{su}(2) \oplus \mathfrak{su}(2) \oplus \mathfrak{su}(2)$
$(\mathbf{1}, \mathbf{16}, \mathbf{1}, \mathbf{1}, \mathbf{1}, \mathbf{1})$, $(0,0,0,0,0,0,0,1,0,0,0,0) \mapsto (D, E, L, N, Q, U)$
$(\mathbf{4}, \mathbf{1}, \mathbf{2}, \mathbf{2}, \mathbf{1}, \mathbf{1})$, $(1,0,0,0,0,0,0,0,1,1,0,0) \mapsto (L, L, Q, Q)$
$(\overline{\mathbf{4}}, \mathbf{1}, \mathbf{1}, \mathbf{1}, \mathbf{2}, \mathbf{2})$, $(0,0,1,0,0,0,0,0,0,0,1,1) \mapsto (D, D, E, E, N, N, U, U)$
Projection matrix for $\alpha$:

$$\begin{pmatrix} 1 & 0 & 0 & 0 & 0 & 1 & 0 & 0 & 0 & 0 & 0 & 0 \\ 0 & 1 & 0 & 0 & 0 & 0 & 0 & 1 & 0 & 0 & 0 & 0 \\ 0 & 0 & 0 & 1 & 0 & 0 & 0 & 0 & 1 & 0 & 0 & 0 \\ 1 & 2 & 3 & 3 & 6 & 4 & 0 & 2 & 0 & 0 & 3 & 0 \end{pmatrix}$$

**3 generation subalgebra** 28
Algebra: $\mathfrak{su}(4) \oplus \mathfrak{su}(4) \oplus \mathfrak{sp}(4) \oplus \mathfrak{sp}(4) \oplus \mathfrak{su}(2) \oplus \mathfrak{su}(2)$
$(\overline{\mathbf{4}}, \mathbf{1}, \mathbf{4}, \mathbf{1}, \mathbf{1}, \mathbf{1}),\ (0,0,1,0,0,0,1,0,0,0,0,0) \mapsto (L, L, Q, Q)$
$(\mathbf{4}, \mathbf{1}, \mathbf{1}, \mathbf{4}, \mathbf{1}, \mathbf{1}),\ (1,0,0,0,0,0,0,0,1,0,0,0) \mapsto (D, D, E, E, N, N, U, U)$
$(\mathbf{1}, \overline{\mathbf{4}}, \mathbf{1}, \mathbf{1}, \mathbf{2}, \mathbf{1}),\ (0,0,0,0,0,1,0,0,0,0,1,0) \mapsto (L, Q)$
$(\mathbf{1}, \mathbf{4}, \mathbf{1}, \mathbf{1}, \mathbf{1}, \mathbf{2}),\ (0,0,0,1,0,0,0,0,0,0,0,1) \mapsto (D, E, N, U)$
Projection matrix for $\alpha$:

$$\begin{pmatrix} 0 & 1 & 0 & 0 & 1 & 0 & 0 & 0 & 0 & 0 & 0 & 0 \\ 1 & 0 & 0 & 1 & 0 & 0 & 0 & 0 & 0 & 0 & 0 & 0 \\ 0 & 0 & 0 & 0 & 0 & 0 & 1 & 2 & 0 & 0 & 1 & 0 \\ -1 & -2 & -3 & -1 & -2 & -3 & 0 & 0 & 3 & 0 & 0 & 3 \end{pmatrix}$$

**3 generation subalgebra** 29
Algebra: $\mathfrak{su}(4) \oplus \mathfrak{su}(5) \oplus \mathfrak{su}(2) \oplus \mathfrak{su}(2) \oplus \mathfrak{su}(2) \oplus \mathfrak{su}(2)$
$(\overline{\mathbf{4}}, \mathbf{1}, \mathbf{2}, \mathbf{1}, \mathbf{1}, \mathbf{1}),\ (0,0,1,0,0,0,0,1,0,0,0) \mapsto (L, Q)$
$(\mathbf{4}, \mathbf{1}, \mathbf{1}, \mathbf{2}, \mathbf{1}, \mathbf{1}),\ (1,0,0,0,0,0,0,0,1,0,0) \mapsto (D, E, N, U)$
$(\mathbf{1}, \overline{\mathbf{5}}, \mathbf{1}, \mathbf{1}, \mathbf{2}, \mathbf{1}),\ (0,0,0,0,0,0,1,0,0,1,0) \mapsto (D, D, L, L)$
$(\mathbf{1}, \mathbf{10}, \mathbf{1}, \mathbf{1}, \mathbf{1}, \mathbf{2}),\ (0,0,0,0,1,0,0,0,0,0,1) \mapsto (E, E, Q, Q, U, U)$
$(\mathbf{1}, \mathbf{1}, \mathbf{1}, \mathbf{2}, \mathbf{1}, \mathbf{1}),\ (0,0,0,0,0,0,0,0,1,0,0) \mapsto (N, N)$
Projection matrix for $\alpha$:

$$\begin{pmatrix} 0 & 1 & 0 & 0 & 0 & 1 & 0 & 0 & 0 & 0 & 0 \\ 1 & 0 & 0 & 0 & 0 & 0 & 1 & 0 & 0 & 0 & 0 \\ 0 & 0 & 0 & 1 & 0 & 0 & 0 & 1 & 0 & 0 & 0 \\ -1 & -2 & -3 & 3 & 6 & 4 & 2 & 0 & 3 & 0 & 0 \end{pmatrix}$$

**3 generation subalgebra** 30
Algebra: $\mathfrak{su}(4) \oplus \mathfrak{su}(5) \oplus \mathfrak{su}(2) \oplus \mathfrak{su}(2) \oplus \mathfrak{su}(2) \oplus \mathfrak{su}(2)$
$(\overline{\mathbf{4}}, \mathbf{1}, \mathbf{2}, \mathbf{1}, \mathbf{1}, \mathbf{1}),\ (0,0,1,0,0,0,0,1,0,0,0) \mapsto (L, Q)$
$(\mathbf{4}, \mathbf{1}, \mathbf{1}, \mathbf{2}, \mathbf{1}, \mathbf{1}),\ (1,0,0,0,0,0,0,0,1,0,0) \mapsto (D, E, N, U)$
$(\mathbf{1}, \overline{\mathbf{5}}, \mathbf{1}, \mathbf{1}, \mathbf{2}, \mathbf{1}),\ (0,0,0,0,0,0,1,0,0,1,0) \mapsto (D, D, L, L)$
$(\mathbf{1}, \mathbf{10}, \mathbf{1}, \mathbf{1}, \mathbf{1}, \mathbf{2}),\ (0,0,0,0,1,0,0,0,0,0,1) \mapsto (E, E, Q, Q, U, U)$
$(\mathbf{1}, \mathbf{1}, \mathbf{2}, \mathbf{1}, \mathbf{1}, \mathbf{1}),\ (0,0,0,0,0,0,0,1,0,0,0) \mapsto (N, N)$
Projection matrix for $\alpha$:

$$\begin{pmatrix} 0 & 1 & 0 & 0 & 0 & 1 & 0 & 0 & 0 & 0 & 0 \\ 1 & 0 & 0 & 0 & 0 & 0 & 1 & 0 & 0 & 0 & 0 \\ 0 & 0 & 0 & 1 & 0 & 0 & 0 & 1 & 0 & 0 & 0 \\ -1 & -2 & -3 & 3 & 6 & 4 & 2 & 0 & 3 & 0 & 0 \end{pmatrix}$$

## D. 3 generation minimal algebras

**3 generation subalgebra** 31
Algebra: $\mathfrak{su}(5)$
$(\overline{\mathbf{5}}),\ (0,0,0,1) \mapsto (D, L)$
$(\overline{\mathbf{5}}),\ (0,0,0,1) \mapsto (D, L)$
$(\overline{\mathbf{5}}),\ (0,0,0,1) \mapsto (D, L)$
$(\mathbf{10}),\ (0,1,0,0) \mapsto (E, Q, U)$
$(\mathbf{10}),\ (0,1,0,0) \mapsto (E, Q, U)$
$(\mathbf{10}),\ (0,1,0,0) \mapsto (E, Q, U)$
$(\mathbf{1}),\ (0,0,0,0) \mapsto (N)$
$(\mathbf{1}),\ (0,0,0,0) \mapsto (N)$
$(\mathbf{1}),\ (0,0,0,0) \mapsto (N)$
Projection matrix for $\alpha$:

$$\begin{pmatrix} 0 & 0 & 1 & 0 \\ 0 & 0 & 0 & 1 \\ 1 & 0 & 0 & 0 \\ 3 & 6 & 4 & 2 \end{pmatrix}$$

**3 generation subalgebra** 32
Algebra: $\mathfrak{su}(4) \oplus \mathfrak{su}(2) \oplus \mathfrak{su}(2)$
$(\overline{\mathbf{4}}, \mathbf{2}, \mathbf{1})$, $(0,0,1,1,0) \mapsto (L, Q)$
$(\overline{\mathbf{4}}, \mathbf{2}, \mathbf{1})$, $(0,0,1,1,0) \mapsto (L, Q)$
$(\overline{\mathbf{4}}, \mathbf{2}, \mathbf{1})$, $(0,0,1,1,0) \mapsto (L, Q)$
$(\mathbf{4}, \mathbf{1}, \mathbf{2})$, $(1,0,0,0,1) \mapsto (D, E, N, U)$
$(\mathbf{4}, \mathbf{1}, \mathbf{2})$, $(1,0,0,0,1) \mapsto (D, E, N, U)$
$(\mathbf{4}, \mathbf{1}, \mathbf{2})$, $(1,0,0,0,1) \mapsto (D, E, N, U)$
Projection matrix for $\alpha$:

$$\begin{pmatrix} 0 & 1 & 0 & 0 & 0 \\ 1 & 0 & 0 & 0 & 0 \\ 0 & 0 & 0 & 1 & 0 \\ -1 & -2 & -3 & 0 & 3 \end{pmatrix}$$

**3 generation subalgebra** 33
Algebra: $\mathfrak{su}(4) \oplus \mathfrak{su}(4) \oplus \mathfrak{su}(2)$
$(\overline{\mathbf{4}}, \mathbf{6}, \mathbf{1})$, $(0,0,1,0,1,0,0) \mapsto (D, D, D, E, E, E, N, N, N, U, U, U)$
$(\mathbf{4}, \mathbf{1}, \mathbf{2})$, $(1,0,0,0,0,0,1) \mapsto (L, Q)$
$(\mathbf{4}, \mathbf{1}, \mathbf{2})$, $(1,0,0,0,0,0,1) \mapsto (L, Q)$
$(\mathbf{4}, \mathbf{1}, \mathbf{2})$, $(1,0,0,0,0,0,1) \mapsto (L, Q)$
Projection matrix for $\alpha$:

$$\begin{pmatrix} 1 & 0 & 0 & 0 & 0 & 0 & 0 \\ 0 & 1 & 0 & 0 & 0 & 0 & 0 \\ 0 & 0 & 0 & 0 & 0 & 0 & 1 \\ 1 & 2 & 3 & \frac{9}{2} & 3 & \frac{3}{2} & 0 \end{pmatrix}$$

**3 generation subalgebra** 34
Algebra: $\mathfrak{su}(4) \oplus \mathfrak{su}(5) \oplus \mathfrak{su}(2) \oplus \mathfrak{su}(2)$
$(\mathbf{1}, \overline{\mathbf{5}}, \mathbf{1}, \mathbf{1})$, $(0,0,0,0,0,0,1,0,0) \mapsto (D, L)$
$(\mathbf{1}, \overline{\mathbf{5}}, \mathbf{1}, \mathbf{1})$, $(0,0,0,0,0,0,1,0,0) \mapsto (D, L)$
$(\mathbf{1}, \mathbf{10}, \mathbf{1}, \mathbf{1})$, $(0,0,0,0,1,0,0,0,0) \mapsto (E, Q, U)$
$(\mathbf{1}, \mathbf{10}, \mathbf{1}, \mathbf{1})$, $(0,0,0,0,1,0,0,0,0) \mapsto (E, Q, U)$
$(\overline{\mathbf{4}}, \mathbf{1}, \mathbf{2}, \mathbf{1})$, $(0,0,1,0,0,0,0,1,0) \mapsto (L, Q)$
$(\mathbf{4}, \mathbf{1}, \mathbf{1}, \mathbf{2})$, $(1,0,0,0,0,0,0,0,1) \mapsto (D, E, N, U)$
$(\mathbf{1}, \mathbf{1}, \mathbf{1}, \mathbf{1})$, $(0,0,0,0,0,0,0,0,0) \mapsto (N)$
$(\mathbf{1}, \mathbf{1}, \mathbf{1}, \mathbf{1})$, $(0,0,0,0,0,0,0,0,0) \mapsto (N)$
Projection matrix for $\alpha$:

$$\begin{pmatrix} 0 & 1 & 0 & 0 & 0 & 1 & 0 & 0 & 0 \\ 1 & 0 & 0 & 0 & 0 & 0 & 1 & 0 & 0 \\ 0 & 0 & 0 & 1 & 0 & 0 & 0 & 1 & 0 \\ -1 & -2 & -3 & 3 & 6 & 4 & 2 & 0 & 3 \end{pmatrix}$$

**3 generation subalgebra** 35
Algebra: $\mathfrak{su}(4) \oplus \mathfrak{su}(5) \oplus \mathfrak{su}(2) \oplus \mathfrak{su}(2)$
$(\mathbf{1}, \overline{\mathbf{5}}, \mathbf{1}, \mathbf{1})$, $(0,0,0,0,0,0,1,0,0) \mapsto (D, L)$
$(\mathbf{1}, \mathbf{10}, \mathbf{1}, \mathbf{1})$, $(0,0,0,0,1,0,0,0,0) \mapsto (E, Q, U)$
$(\overline{\mathbf{4}}, \mathbf{1}, \mathbf{2}, \mathbf{1})$, $(0,0,1,0,0,0,0,1,0) \mapsto (L, Q)$
$(\overline{\mathbf{4}}, \mathbf{1}, \mathbf{2}, \mathbf{1})$, $(0,0,1,0,0,0,0,1,0) \mapsto (L, Q)$
$(\mathbf{4}, \mathbf{1}, \mathbf{1}, \mathbf{2})$, $(1,0,0,0,0,0,0,0,1) \mapsto (D, E, N, U)$
$(\mathbf{4}, \mathbf{1}, \mathbf{1}, \mathbf{2})$, $(1,0,0,0,0,0,0,0,1) \mapsto (D, E, N, U)$
$(\mathbf{1}, \mathbf{1}, \mathbf{1}, \mathbf{1})$, $(0,0,0,0,0,0,0,0,0) \mapsto (N)$
Projection matrix for $\alpha$:

$$\begin{pmatrix} 0 & 1 & 0 & 0 & 0 & 1 & 0 & 0 & 0 \\ 1 & 0 & 0 & 0 & 0 & 0 & 1 & 0 & 0 \\ 0 & 0 & 0 & 1 & 0 & 0 & 0 & 1 & 0 \\ -1 & -2 & -3 & 3 & 6 & 4 & 2 & 0 & 3 \end{pmatrix}$$

**3 generation subalgebra** 36
Algebra: $\mathfrak{su}(4) \oplus \mathfrak{su}(5) \oplus \mathfrak{su}(2) \oplus \mathfrak{su}(2)$
$(\mathbf{1}, \overline{\mathbf{5}}, \mathbf{1}, \mathbf{1}),\ (0,0,0,0,0,0,1,0,0) \mapsto (D, L)$
$(\mathbf{1}, \overline{\mathbf{5}}, \mathbf{1}, \mathbf{1}),\ (0,0,0,0,0,0,1,0,0) \mapsto (D, L)$
$(\mathbf{1}, \mathbf{10}, \mathbf{1}, \mathbf{1}),\ (0,0,0,0,1,0,0,0,0) \mapsto (E, Q, U)$
$(\mathbf{1}, \mathbf{10}, \mathbf{1}, \mathbf{1}),\ (0,0,0,0,1,0,0,0,0) \mapsto (E, Q, U)$
$(\overline{\mathbf{4}}, \mathbf{1}, \mathbf{2}, \mathbf{1}),\ (0,0,1,0,0,0,0,1,0) \mapsto (L, Q)$
$(\mathbf{4}, \mathbf{1}, \mathbf{1}, \mathbf{2}),\ (1,0,0,0,0,0,0,0,1) \mapsto (D, E, N, U)$
$(\mathbf{1}, \mathbf{1}, \mathbf{1}, \mathbf{2}),\ (0,0,0,0,0,0,0,0,1) \mapsto (N, N)$
Projection matrix for $\alpha$:

$$\begin{pmatrix} 0 & 1 & 0 & 0 & 0 & 1 & 0 & 0 & 0 \\ 1 & 0 & 0 & 0 & 0 & 0 & 1 & 0 & 0 \\ 0 & 0 & 0 & 1 & 0 & 0 & 0 & 1 & 0 \\ -1 & -2 & -3 & 3 & 6 & 4 & 2 & 0 & 3 \end{pmatrix}$$

**3 generation subalgebra** 37
Algebra: $\mathfrak{su}(4) \oplus \mathfrak{su}(5) \oplus \mathfrak{su}(2) \oplus \mathfrak{su}(2)$
$(\mathbf{1}, \overline{\mathbf{5}}, \mathbf{1}, \mathbf{1}),\ (0,0,0,0,0,0,1,0,0) \mapsto (D, L)$
$(\mathbf{1}, \overline{\mathbf{5}}, \mathbf{1}, \mathbf{1}),\ (0,0,0,0,0,0,1,0,0) \mapsto (D, L)$
$(\mathbf{1}, \mathbf{10}, \mathbf{1}, \mathbf{1}),\ (0,0,0,0,1,0,0,0,0) \mapsto (E, Q, U)$
$(\mathbf{1}, \mathbf{10}, \mathbf{1}, \mathbf{1}),\ (0,0,0,0,1,0,0,0,0) \mapsto (E, Q, U)$
$(\overline{\mathbf{4}}, \mathbf{1}, \mathbf{2}, \mathbf{1}),\ (0,0,1,0,0,0,0,1,0) \mapsto (L, Q)$
$(\mathbf{4}, \mathbf{1}, \mathbf{1}, \mathbf{2}),\ (1,0,0,0,0,0,0,0,1) \mapsto (D, E, N, U)$
$(\mathbf{1}, \mathbf{1}, \mathbf{2}, \mathbf{1}),\ (0,0,0,0,0,0,0,1,0) \mapsto (N, N)$
Projection matrix for $\alpha$:

$$\begin{pmatrix} 0 & 1 & 0 & 0 & 0 & 1 & 0 & 0 & 0 \\ 1 & 0 & 0 & 0 & 0 & 0 & 1 & 0 & 0 \\ 0 & 0 & 0 & 1 & 0 & 0 & 0 & 1 & 0 \\ -1 & -2 & -3 & 3 & 6 & 4 & 2 & 0 & 3 \end{pmatrix}$$

**3 generation subalgebra** 38
Algebra: $\mathfrak{su}(4) \oplus \mathfrak{su}(4) \oplus \mathfrak{su}(4) \oplus \mathfrak{su}(2) \oplus \mathfrak{su}(2)$
$(\overline{\mathbf{4}}, \mathbf{1}, \mathbf{1}, \mathbf{2}, \mathbf{1}),\ (0,0,1,0,0,0,0,0,0,1,0) \mapsto (L, Q)$
$(\mathbf{1}, \overline{\mathbf{4}}, \mathbf{1}, \mathbf{2}, \mathbf{1}),\ (0,0,0,0,0,1,0,0,0,1,0) \mapsto (L, Q)$
$(\mathbf{1}, \mathbf{1}, \overline{\mathbf{4}}, \mathbf{2}, \mathbf{1}),\ (0,0,0,0,0,0,0,0,1,1,0) \mapsto (L, Q)$
$(\mathbf{4}, \mathbf{1}, \mathbf{1}, \mathbf{1}, \mathbf{2}),\ (1,0,0,0,0,0,0,0,0,0,1) \mapsto (D, E, N, U)$
$(\mathbf{1}, \mathbf{4}, \mathbf{1}, \mathbf{1}, \mathbf{2}),\ (0,0,0,1,0,0,0,0,0,0,1) \mapsto (D, E, N, U)$
$(\mathbf{1}, \mathbf{1}, \mathbf{4}, \mathbf{1}, \mathbf{2}),\ (0,0,0,0,0,0,1,0,0,0,1) \mapsto (D, E, N, U)$
Projection matrix for $\alpha$:

$$\begin{pmatrix} 0 & 1 & 0 & 0 & 1 & 0 & 0 & 1 & 0 & 0 & 0 \\ 1 & 0 & 0 & 1 & 0 & 0 & 1 & 0 & 0 & 0 & 0 \\ 0 & 0 & 0 & 0 & 0 & 0 & 0 & 0 & 0 & 1 & 0 \\ -1 & -2 & -3 & -1 & -2 & -3 & -1 & -2 & -3 & 0 & 3 \end{pmatrix}$$

### E. 3 generation non maximal nor minimal algebras

**3 generation subalgebra** 39
Algebra: $\mathfrak{so}(10)$
$(\mathbf{16}),\ (0,0,0,0,1) \mapsto (D, E, L, N, Q, U)$
$(\mathbf{16}),\ (0,0,0,0,1) \mapsto (D, E, L, N, Q, U)$
$(\mathbf{16}),\ (0,0,0,0,1) \mapsto (D, E, L, N, Q, U)$
Projection matrix for $\alpha$:

$$\begin{pmatrix} 0 & 0 & 1 & 0 & 0 \\ 0 & 0 & 0 & 0 & 1 \\ 1 & 0 & 0 & 0 & 0 \\ 3 & 6 & 4 & 0 & 2 \end{pmatrix}$$

**3 generation subalgebra** 40
Algebra: $\mathfrak{so}(10) \oplus \mathfrak{so}(10)$
$(\mathbf{16}, \mathbf{1}),\ (0,0,0,0,1,0,0,0,0,0) \mapsto (D, E, L, N, Q, U)$
$(\mathbf{1}, \mathbf{16}),\ (0,0,0,0,0,0,0,0,0,1) \mapsto (D, E, L, N, Q, U)$
$(\mathbf{1}, \mathbf{16}),\ (0,0,0,0,0,0,0,0,0,1) \mapsto (D, E, L, N, Q, U)$
Projection matrix for $\alpha$:

$$\begin{pmatrix} 0 & 0 & 1 & 0 & 0 & 0 & 0 & 1 & 0 & 0 \\ 0 & 0 & 0 & 0 & 1 & 0 & 0 & 0 & 0 & 1 \\ 1 & 0 & 0 & 0 & 0 & 1 & 0 & 0 & 0 & 0 \\ 3 & 6 & 4 & 0 & 2 & 3 & 6 & 4 & 0 & 2 \end{pmatrix}$$

**3 generation subalgebra** 41
Algebra: $\mathfrak{so}(10) \oplus \mathfrak{su}(2)$
$(\mathbf{16}, \mathbf{1}),\ (0,0,0,0,1,0) \mapsto (D, E, L, N, Q, U)$
$(\mathbf{16}, \mathbf{2}),\ (0,0,0,0,1,1) \mapsto (D, D, E, E, L, L, N, N, Q, Q, U, U)$
Projection matrix for $\alpha$:

$$\begin{pmatrix} 0 & 0 & 1 & 0 & 0 & 0 \\ 0 & 0 & 0 & 0 & 1 & 0 \\ 1 & 0 & 0 & 0 & 0 & 0 \\ 3 & 6 & 4 & 0 & 2 & 0 \end{pmatrix}$$

**3 generation subalgebra** 42
Algebra: $\mathfrak{su}(5) \oplus \mathfrak{so}(10)$
$(\overline{\mathbf{5}}, \mathbf{1}),\ (0,0,0,1,0,0,0,0,0) \mapsto (D, L)$
$(\mathbf{10}, \mathbf{1}),\ (0,1,0,0,0,0,0,0,0) \mapsto (E, Q, U)$
$(\mathbf{1}, \mathbf{16}),\ (0,0,0,0,0,0,0,0,1) \mapsto (D, E, L, N, Q, U)$
$(\mathbf{1}, \mathbf{16}),\ (0,0,0,0,0,0,0,0,1) \mapsto (D, E, L, N, Q, U)$
$(\mathbf{1}, \mathbf{1}),\ (0,0,0,0,0,0,0,0,0) \mapsto (N)$
Projection matrix for $\alpha$:

$$\begin{pmatrix} 0 & 0 & 1 & 0 & 0 & 0 & 1 & 0 & 0 \\ 0 & 0 & 0 & 1 & 0 & 0 & 0 & 0 & 1 \\ 1 & 0 & 0 & 0 & 1 & 0 & 0 & 0 & 0 \\ 3 & 6 & 4 & 2 & 3 & 6 & 4 & 0 & 2 \end{pmatrix}$$

**3 generation subalgebra** 43
Algebra: $\mathfrak{su}(5) \oplus \mathfrak{so}(10)$
$(\overline{\mathbf{5}}, \mathbf{1}),\ (0,0,0,1,0,0,0,0,0) \mapsto (D, L)$
$(\overline{\mathbf{5}}, \mathbf{1}),\ (0,0,0,1,0,0,0,0,0) \mapsto (D, L)$
$(\mathbf{10}, \mathbf{1}),\ (0,1,0,0,0,0,0,0,0) \mapsto (E, Q, U)$
$(\mathbf{10}, \mathbf{1}),\ (0,1,0,0,0,0,0,0,0) \mapsto (E, Q, U)$
$(\mathbf{1}, \mathbf{16}),\ (0,0,0,0,0,0,0,0,1) \mapsto (D, E, L, N, Q, U)$
$(\mathbf{1}, \mathbf{1}),\ (0,0,0,0,0,0,0,0,0) \mapsto (N)$
$(\mathbf{1}, \mathbf{1}),\ (0,0,0,0,0,0,0,0,0) \mapsto (N)$
Projection matrix for $\alpha$:

$$\begin{pmatrix} 0 & 0 & 1 & 0 & 0 & 0 & 1 & 0 & 0 \\ 0 & 0 & 0 & 1 & 0 & 0 & 0 & 0 & 1 \\ 1 & 0 & 0 & 0 & 1 & 0 & 0 & 0 & 0 \\ 3 & 6 & 4 & 2 & 3 & 6 & 4 & 0 & 2 \end{pmatrix}$$

**3 generation subalgebra** 44
Algebra: $\mathfrak{su}(5) \oplus \mathfrak{su}(2)$
$(\overline{\mathbf{5}}, \mathbf{3}),\ (0,0,0,1,2) \mapsto (D, D, D, L, L, L)$
$(\mathbf{10}, \mathbf{3}),\ (0,1,0,0,2) \mapsto (E, E, E, Q, Q, Q, U, U, U)$
$(\mathbf{1}, \mathbf{1}),\ (0,0,0,0,0) \mapsto (N)$
$(\mathbf{1}, \mathbf{1}),\ (0,0,0,0,0) \mapsto (N)$

$(\mathbf{1},\mathbf{1}),\ (0,0,0,0,0) \mapsto (N)$
Projection matrix for $\alpha$:

$$\begin{pmatrix} 0 & 0 & 1 & 0 & 0 \\ 0 & 0 & 0 & 1 & 0 \\ 1 & 0 & 0 & 0 & 0 \\ 3 & 6 & 4 & 2 & 0 \end{pmatrix}$$

**3 generation subalgebra** 45
Algebra: $\mathfrak{su}(5) \oplus \mathfrak{su}(2)$
$(\overline{\mathbf{5}},\mathbf{1}),\ (0,0,0,1,0) \mapsto (D,L)$
$(\overline{\mathbf{5}},\mathbf{2}),\ (0,0,0,1,1) \mapsto (D,D,L,L)$
$(\mathbf{10},\mathbf{3}),\ (0,1,0,0,2) \mapsto (E,E,E,Q,Q,Q,U,U,U)$
$(\mathbf{1},\mathbf{1}),\ (0,0,0,0,0) \mapsto (N)$
$(\mathbf{1},\mathbf{1}),\ (0,0,0,0,0) \mapsto (N)$
$(\mathbf{1},\mathbf{1}),\ (0,0,0,0,0) \mapsto (N)$
Projection matrix for $\alpha$:

$$\begin{pmatrix} 0 & 0 & 1 & 0 & 0 \\ 0 & 0 & 0 & 1 & 0 \\ 1 & 0 & 0 & 0 & 0 \\ 3 & 6 & 4 & 2 & 0 \end{pmatrix}$$

**3 generation subalgebra** 46
Algebra: $\mathfrak{su}(5) \oplus \mathfrak{su}(2)$
$(\overline{\mathbf{5}},\mathbf{3}),\ (0,0,0,1,2) \mapsto (D,D,D,L,L,L)$
$(\mathbf{10},\mathbf{3}),\ (0,1,0,0,2) \mapsto (E,E,E,Q,Q,Q,U,U,U)$
$(\mathbf{1},\mathbf{2}),\ (0,0,0,0,1) \mapsto (N,N)$
$(\mathbf{1},\mathbf{1}),\ (0,0,0,0,0) \mapsto (N)$
Projection matrix for $\alpha$:

$$\begin{pmatrix} 0 & 0 & 1 & 0 & 0 \\ 0 & 0 & 0 & 1 & 0 \\ 1 & 0 & 0 & 0 & 0 \\ 3 & 6 & 4 & 2 & 0 \end{pmatrix}$$

**3 generation subalgebra** 47
Algebra: $\mathfrak{su}(5) \oplus \mathfrak{su}(2)$
$(\overline{\mathbf{5}},\mathbf{3}),\ (0,0,0,1,2) \mapsto (D,D,D,L,L,L)$
$(\mathbf{10},\mathbf{3}),\ (0,1,0,0,2) \mapsto (E,E,E,Q,Q,Q,U,U,U)$
$(\mathbf{1},\mathbf{3}),\ (0,0,0,0,2) \mapsto (N,N,N)$
Projection matrix for $\alpha$:

$$\begin{pmatrix} 0 & 0 & 1 & 0 & 0 \\ 0 & 0 & 0 & 1 & 0 \\ 1 & 0 & 0 & 0 & 0 \\ 3 & 6 & 4 & 2 & 0 \end{pmatrix}$$

**3 generation subalgebra** 48
Algebra: $\mathfrak{su}(5) \oplus \mathfrak{su}(2)$
$(\mathbf{10},\mathbf{1}),\ (0,1,0,0,0) \mapsto (E,Q,U)$
$(\overline{\mathbf{5}},\mathbf{3}),\ (0,0,0,1,2) \mapsto (D,D,D,L,L,L)$
$(\mathbf{10},\mathbf{2}),\ (0,1,0,0,1) \mapsto (E,E,Q,Q,U,U)$
$(\mathbf{1},\mathbf{1}),\ (0,0,0,0,0) \mapsto (N)$
$(\mathbf{1},\mathbf{1}),\ (0,0,0,0,0) \mapsto (N)$
$(\mathbf{1},\mathbf{1}),\ (0,0,0,0,0) \mapsto (N)$
Projection matrix for $\alpha$:

$$\begin{pmatrix} 0 & 0 & 1 & 0 & 0 \\ 0 & 0 & 0 & 1 & 0 \\ 1 & 0 & 0 & 0 & 0 \\ 3 & 6 & 4 & 2 & 0 \end{pmatrix}$$

**3 generation subalgebra** 49
Algebra: $\mathfrak{su}(5) \oplus \mathfrak{su}(2)$
$(\overline{\mathbf{5}}, \mathbf{1}),\ (0,0,0,1,0) \mapsto (D, L)$
$(\overline{\mathbf{5}}, \mathbf{1}),\ (0,0,0,1,0) \mapsto (D, L)$
$(\overline{\mathbf{5}}, \mathbf{1}),\ (0,0,0,1,0) \mapsto (D, L)$
$(\mathbf{10}, \mathbf{3}),\ (0,1,0,0,2) \mapsto (E, E, E, Q, Q, Q, U, U, U)$
$(\mathbf{1}, \mathbf{1}),\ (0,0,0,0,0) \mapsto (N)$
$(\mathbf{1}, \mathbf{1}),\ (0,0,0,0,0) \mapsto (N)$
$(\mathbf{1}, \mathbf{1}),\ (0,0,0,0,0) \mapsto (N)$
Projection matrix for $\alpha$:

$$\begin{pmatrix} 0 & 0 & 1 & 0 & 0 \\ 0 & 0 & 0 & 1 & 0 \\ 1 & 0 & 0 & 0 & 0 \\ 3 & 6 & 4 & 2 & 0 \end{pmatrix}$$

**3 generation subalgebra** 50
Algebra: $\mathfrak{su}(5) \oplus \mathfrak{su}(2)$
$(\overline{\mathbf{5}}, \mathbf{1}),\ (0,0,0,1,0) \mapsto (D, L)$
$(\overline{\mathbf{5}}, \mathbf{2}),\ (0,0,0,1,1) \mapsto (D, D, L, L)$
$(\mathbf{10}, \mathbf{3}),\ (0,1,0,0,2) \mapsto (E, E, E, Q, Q, Q, U, U, U)$
$(\mathbf{1}, \mathbf{2}),\ (0,0,0,0,1) \mapsto (N, N)$
$(\mathbf{1}, \mathbf{1}),\ (0,0,0,0,0) \mapsto (N)$
Projection matrix for $\alpha$:

$$\begin{pmatrix} 0 & 0 & 1 & 0 & 0 \\ 0 & 0 & 0 & 1 & 0 \\ 1 & 0 & 0 & 0 & 0 \\ 3 & 6 & 4 & 2 & 0 \end{pmatrix}$$

**3 generation subalgebra** 51
Algebra: $\mathfrak{su}(5) \oplus \mathfrak{su}(2)$
$(\overline{\mathbf{5}}, \mathbf{1}),\ (0,0,0,1,0) \mapsto (D, L)$
$(\overline{\mathbf{5}}, \mathbf{2}),\ (0,0,0,1,1) \mapsto (D, D, L, L)$
$(\mathbf{10}, \mathbf{3}),\ (0,1,0,0,2) \mapsto (E, E, E, Q, Q, Q, U, U, U)$
$(\mathbf{1}, \mathbf{3}),\ (0,0,0,0,2) \mapsto (N, N, N)$
Projection matrix for $\alpha$:

$$\begin{pmatrix} 0 & 0 & 1 & 0 & 0 \\ 0 & 0 & 0 & 1 & 0 \\ 1 & 0 & 0 & 0 & 0 \\ 3 & 6 & 4 & 2 & 0 \end{pmatrix}$$

**3 generation subalgebra** 52
Algebra: $\mathfrak{su}(5) \oplus \mathfrak{su}(2)$
$(\overline{\mathbf{5}}, \mathbf{1}),\ (0,0,0,1,0) \mapsto (D, L)$
$(\mathbf{10}, \mathbf{1}),\ (0,1,0,0,0) \mapsto (E, Q, U)$
$(\overline{\mathbf{5}}, \mathbf{2}),\ (0,0,0,1,1) \mapsto (D, D, L, L)$
$(\mathbf{10}, \mathbf{2}),\ (0,1,0,0,1) \mapsto (E, E, Q, Q, U, U)$
$(\mathbf{1}, \mathbf{1}),\ (0,0,0,0,0) \mapsto (N)$
$(\mathbf{1}, \mathbf{1}),\ (0,0,0,0,0) \mapsto (N)$
$(\mathbf{1}, \mathbf{1}),\ (0,0,0,0,0) \mapsto (N)$
Projection matrix for $\alpha$:

$$\begin{pmatrix} 0 & 0 & 1 & 0 & 0 \\ 0 & 0 & 0 & 1 & 0 \\ 1 & 0 & 0 & 0 & 0 \\ 3 & 6 & 4 & 2 & 0 \end{pmatrix}$$

**3 generation subalgebra** 53
Algebra: $\mathfrak{su}(5) \oplus \mathfrak{su}(2)$

$(\mathbf{10}, \mathbf{1})$, $(0,1,0,0,0) \mapsto (E,Q,U)$
$(\bar{\mathbf{5}}, \mathbf{3})$, $(0,0,0,1,2) \mapsto (D,D,D,L,L,L)$
$(\mathbf{10}, \mathbf{2})$, $(0,1,0,0,1) \mapsto (E,E,Q,Q,U,U)$
$(\mathbf{1}, \mathbf{2})$, $(0,0,0,0,1) \mapsto (N,N)$
$(\mathbf{1}, \mathbf{1})$, $(0,0,0,0,0) \mapsto (N)$
Projection matrix for $\alpha$:

$$\begin{pmatrix} 0 & 0 & 1 & 0 & 0 \\ 0 & 0 & 0 & 1 & 0 \\ 1 & 0 & 0 & 0 & 0 \\ 3 & 6 & 4 & 2 & 0 \end{pmatrix}$$

**3 generation subalgebra** 54
Algebra: $\mathfrak{su}(5) \oplus \mathfrak{su}(2)$
$(\mathbf{10}, \mathbf{1})$, $(0,1,0,0,0) \mapsto (E,Q,U)$
$(\bar{\mathbf{5}}, \mathbf{3})$, $(0,0,0,1,2) \mapsto (D,D,D,L,L,L)$
$(\mathbf{10}, \mathbf{2})$, $(0,1,0,0,1) \mapsto (E,E,Q,Q,U,U)$
$(\mathbf{1}, \mathbf{3})$, $(0,0,0,0,2) \mapsto (N,N,N)$
Projection matrix for $\alpha$:

$$\begin{pmatrix} 0 & 0 & 1 & 0 & 0 \\ 0 & 0 & 0 & 1 & 0 \\ 1 & 0 & 0 & 0 & 0 \\ 3 & 6 & 4 & 2 & 0 \end{pmatrix}$$

**3 generation subalgebra** 55
Algebra: $\mathfrak{su}(5) \oplus \mathfrak{su}(2)$
$(\mathbf{10}, \mathbf{1})$, $(0,1,0,0,0) \mapsto (E,Q,U)$
$(\mathbf{10}, \mathbf{1})$, $(0,1,0,0,0) \mapsto (E,Q,U)$
$(\mathbf{10}, \mathbf{1})$, $(0,1,0,0,0) \mapsto (E,Q,U)$
$(\bar{\mathbf{5}}, \mathbf{3})$, $(0,0,0,1,2) \mapsto (D,D,D,L,L,L)$
$(\mathbf{1}, \mathbf{1})$, $(0,0,0,0,0) \mapsto (N)$
$(\mathbf{1}, \mathbf{1})$, $(0,0,0,0,0) \mapsto (N)$
$(\mathbf{1}, \mathbf{1})$, $(0,0,0,0,0) \mapsto (N)$
Projection matrix for $\alpha$:

$$\begin{pmatrix} 0 & 0 & 1 & 0 & 0 \\ 0 & 0 & 0 & 1 & 0 \\ 1 & 0 & 0 & 0 & 0 \\ 3 & 6 & 4 & 2 & 0 \end{pmatrix}$$

**3 generation subalgebra** 56
Algebra: $\mathfrak{su}(5) \oplus \mathfrak{su}(2)$
$(\bar{\mathbf{5}}, \mathbf{1})$, $(0,0,0,1,0) \mapsto (D,L)$
$(\bar{\mathbf{5}}, \mathbf{1})$, $(0,0,0,1,0) \mapsto (D,L)$
$(\bar{\mathbf{5}}, \mathbf{1})$, $(0,0,0,1,0) \mapsto (D,L)$
$(\mathbf{10}, \mathbf{1})$, $(0,1,0,0,0) \mapsto (E,Q,U)$
$(\mathbf{10}, \mathbf{2})$, $(0,1,0,0,1) \mapsto (E,E,Q,Q,U,U)$
$(\mathbf{1}, \mathbf{1})$, $(0,0,0,0,0) \mapsto (N)$
$(\mathbf{1}, \mathbf{1})$, $(0,0,0,0,0) \mapsto (N)$
$(\mathbf{1}, \mathbf{1})$, $(0,0,0,0,0) \mapsto (N)$
Projection matrix for $\alpha$:

$$\begin{pmatrix} 0 & 0 & 1 & 0 & 0 \\ 0 & 0 & 0 & 1 & 0 \\ 1 & 0 & 0 & 0 & 0 \\ 3 & 6 & 4 & 2 & 0 \end{pmatrix}$$

**3 generation subalgebra** 57
Algebra: $\mathfrak{su}(5) \oplus \mathfrak{su}(2)$

$(\bar{\mathbf{5}},\mathbf{1}),\ (0,0,0,1,0)\mapsto(D,L)$
$(\bar{\mathbf{5}},\mathbf{1}),\ (0,0,0,1,0)\mapsto(D,L)$
$(\bar{\mathbf{5}},\mathbf{1}),\ (0,0,0,1,0)\mapsto(D,L)$
$(\mathbf{10},\mathbf{3}),\ (0,1,0,0,2)\mapsto(E,E,E,Q,Q,Q,U,U,U)$
$(\mathbf{1},\mathbf{2}),\ (0,0,0,0,1)\mapsto(N,N)$
$(\mathbf{1},\mathbf{1}),\ (0,0,0,0,0)\mapsto(N)$
Projection matrix for $\alpha$:

$$\begin{pmatrix}0&0&1&0&0\\0&0&0&1&0\\1&0&0&0&0\\3&6&4&2&0\end{pmatrix}$$

**3 generation subalgebra** 58
Algebra: $\mathfrak{su}(5)\oplus\mathfrak{su}(2)$
$(\bar{\mathbf{5}},\mathbf{1}),\ (0,0,0,1,0)\mapsto(D,L)$
$(\bar{\mathbf{5}},\mathbf{1}),\ (0,0,0,1,0)\mapsto(D,L)$
$(\bar{\mathbf{5}},\mathbf{1}),\ (0,0,0,1,0)\mapsto(D,L)$
$(\mathbf{10},\mathbf{3}),\ (0,1,0,0,2)\mapsto(E,E,E,Q,Q,Q,U,U,U)$
$(\mathbf{1},\mathbf{3}),\ (0,0,0,0,2)\mapsto(N,N,N)$
Projection matrix for $\alpha$:

$$\begin{pmatrix}0&0&1&0&0\\0&0&0&1&0\\1&0&0&0&0\\3&6&4&2&0\end{pmatrix}$$

**3 generation subalgebra** 59
Algebra: $\mathfrak{su}(5)\oplus\mathfrak{su}(2)$
$(\bar{\mathbf{5}},\mathbf{1}),\ (0,0,0,1,0)\mapsto(D,L)$
$(\mathbf{10},\mathbf{1}),\ (0,1,0,0,0)\mapsto(E,Q,U)$
$(\bar{\mathbf{5}},\mathbf{2}),\ (0,0,0,1,1)\mapsto(D,D,L,L)$
$(\mathbf{10},\mathbf{2}),\ (0,1,0,0,1)\mapsto(E,E,Q,Q,U,U)$
$(\mathbf{1},\mathbf{2}),\ (0,0,0,0,1)\mapsto(N,N)$
$(\mathbf{1},\mathbf{1}),\ (0,0,0,0,0)\mapsto(N)$
Projection matrix for $\alpha$:

$$\begin{pmatrix}0&0&1&0&0\\0&0&0&1&0\\1&0&0&0&0\\3&6&4&2&0\end{pmatrix}$$

**3 generation subalgebra** 60
Algebra: $\mathfrak{su}(5)\oplus\mathfrak{su}(2)$
$(\bar{\mathbf{5}},\mathbf{1}),\ (0,0,0,1,0)\mapsto(D,L)$
$(\mathbf{10},\mathbf{1}),\ (0,1,0,0,0)\mapsto(E,Q,U)$
$(\bar{\mathbf{5}},\mathbf{2}),\ (0,0,0,1,1)\mapsto(D,D,L,L)$
$(\mathbf{10},\mathbf{2}),\ (0,1,0,0,1)\mapsto(E,E,Q,Q,U,U)$
$(\mathbf{1},\mathbf{3}),\ (0,0,0,0,2)\mapsto(N,N,N)$
Projection matrix for $\alpha$:

$$\begin{pmatrix}0&0&1&0&0\\0&0&0&1&0\\1&0&0&0&0\\3&6&4&2&0\end{pmatrix}$$

**3 generation subalgebra** 61
Algebra: $\mathfrak{su}(5)\oplus\mathfrak{su}(2)$
$(\bar{\mathbf{5}},\mathbf{1}),\ (0,0,0,1,0)\mapsto(D,L)$
$(\mathbf{10},\mathbf{1}),\ (0,1,0,0,0)\mapsto(E,Q,U)$

$(\mathbf{10},\mathbf{1}),\ (0,1,0,0,0) \mapsto (E,Q,U)$
$(\mathbf{10},\mathbf{1}),\ (0,1,0,0,0) \mapsto (E,Q,U)$
$(\overline{\mathbf{5}},\mathbf{2}),\ (0,0,0,1,1) \mapsto (D,D,L,L)$
$(\mathbf{1},\mathbf{1}),\ (0,0,0,0,0) \mapsto (N)$
$(\mathbf{1},\mathbf{1}),\ (0,0,0,0,0) \mapsto (N)$
$(\mathbf{1},\mathbf{1}),\ (0,0,0,0,0) \mapsto (N)$
Projection matrix for $\alpha$:

$$\begin{pmatrix}0&0&1&0&0\\0&0&0&1&0\\1&0&0&0&0\\3&6&4&2&0\end{pmatrix}$$

**3 generation subalgebra** 62
Algebra: $\mathfrak{su}(5)\oplus\mathfrak{su}(2)$
$(\mathbf{10},\mathbf{1}),\ (0,1,0,0,0) \mapsto (E,Q,U)$
$(\mathbf{10},\mathbf{1}),\ (0,1,0,0,0) \mapsto (E,Q,U)$
$(\mathbf{10},\mathbf{1}),\ (0,1,0,0,0) \mapsto (E,Q,U)$
$(\overline{\mathbf{5}},\mathbf{3}),\ (0,0,0,1,2) \mapsto (D,D,D,L,L,L)$
$(\mathbf{1},\mathbf{2}),\ (0,0,0,0,1) \mapsto (N,N)$
$(\mathbf{1},\mathbf{1}),\ (0,0,0,0,0) \mapsto (N)$
Projection matrix for $\alpha$:

$$\begin{pmatrix}0&0&1&0&0\\0&0&0&1&0\\1&0&0&0&0\\3&6&4&2&0\end{pmatrix}$$

**3 generation subalgebra** 63
Algebra: $\mathfrak{su}(5)\oplus\mathfrak{su}(2)$
$(\mathbf{10},\mathbf{1}),\ (0,1,0,0,0) \mapsto (E,Q,U)$
$(\mathbf{10},\mathbf{1}),\ (0,1,0,0,0) \mapsto (E,Q,U)$
$(\mathbf{10},\mathbf{1}),\ (0,1,0,0,0) \mapsto (E,Q,U)$
$(\overline{\mathbf{5}},\mathbf{3}),\ (0,0,0,1,2) \mapsto (D,D,D,L,L,L)$
$(\mathbf{1},\mathbf{3}),\ (0,0,0,0,2) \mapsto (N,N,N)$
Projection matrix for $\alpha$:

$$\begin{pmatrix}0&0&1&0&0\\0&0&0&1&0\\1&0&0&0&0\\3&6&4&2&0\end{pmatrix}$$

**3 generation subalgebra** 64
Algebra: $\mathfrak{su}(5)\oplus\mathfrak{su}(2)$
$(\overline{\mathbf{5}},\mathbf{1}),\ (0,0,0,1,0) \mapsto (D,L)$
$(\overline{\mathbf{5}},\mathbf{1}),\ (0,0,0,1,0) \mapsto (D,L)$
$(\overline{\mathbf{5}},\mathbf{1}),\ (0,0,0,1,0) \mapsto (D,L)$
$(\mathbf{10},\mathbf{1}),\ (0,1,0,0,0) \mapsto (E,Q,U)$
$(\mathbf{10},\mathbf{2}),\ (0,1,0,0,1) \mapsto (E,E,Q,Q,U,U)$
$(\mathbf{1},\mathbf{2}),\ (0,0,0,0,1) \mapsto (N,N)$
$(\mathbf{1},\mathbf{1}),\ (0,0,0,0,0) \mapsto (N)$
Projection matrix for $\alpha$:

$$\begin{pmatrix}0&0&1&0&0\\0&0&0&1&0\\1&0&0&0&0\\3&6&4&2&0\end{pmatrix}$$

**3 generation subalgebra** 65
Algebra: $\mathfrak{su}(5)\oplus\mathfrak{su}(2)$

$(\bar{\mathbf{5}}, \mathbf{1}),\ (0,0,0,1,0) \mapsto (D, L)$
$(\bar{\mathbf{5}}, \mathbf{1}),\ (0,0,0,1,0) \mapsto (D, L)$
$(\bar{\mathbf{5}}, \mathbf{1}),\ (0,0,0,1,0) \mapsto (D, L)$
$(\mathbf{10}, \mathbf{1}),\ (0,1,0,0,0) \mapsto (E, Q, U)$
$(\mathbf{10}, \mathbf{2}),\ (0,1,0,0,1) \mapsto (E, E, Q, Q, U, U)$
$(\mathbf{1}, \mathbf{3}),\ (0,0,0,0,2) \mapsto (N, N, N)$
Projection matrix for $\alpha$:

$$\begin{pmatrix} 0 & 0 & 1 & 0 & 0 \\ 0 & 0 & 0 & 1 & 0 \\ 1 & 0 & 0 & 0 & 0 \\ 3 & 6 & 4 & 2 & 0 \end{pmatrix}$$

**3 generation subalgebra** 66
Algebra: $\mathfrak{su}(5) \oplus \mathfrak{su}(2)$
$(\bar{\mathbf{5}}, \mathbf{1}),\ (0,0,0,1,0) \mapsto (D, L)$
$(\mathbf{10}, \mathbf{1}),\ (0,1,0,0,0) \mapsto (E, Q, U)$
$(\mathbf{10}, \mathbf{1}),\ (0,1,0,0,0) \mapsto (E, Q, U)$
$(\mathbf{10}, \mathbf{1}),\ (0,1,0,0,0) \mapsto (E, Q, U)$
$(\bar{\mathbf{5}}, \mathbf{2}),\ (0,0,0,1,1) \mapsto (D, D, L, L)$
$(\mathbf{1}, \mathbf{2}),\ (0,0,0,0,1) \mapsto (N, N)$
$(\mathbf{1}, \mathbf{1}),\ (0,0,0,0,0) \mapsto (N)$
Projection matrix for $\alpha$:

$$\begin{pmatrix} 0 & 0 & 1 & 0 & 0 \\ 0 & 0 & 0 & 1 & 0 \\ 1 & 0 & 0 & 0 & 0 \\ 3 & 6 & 4 & 2 & 0 \end{pmatrix}$$

**3 generation subalgebra** 67
Algebra: $\mathfrak{su}(5) \oplus \mathfrak{su}(2)$
$(\bar{\mathbf{5}}, \mathbf{1}),\ (0,0,0,1,0) \mapsto (D, L)$
$(\mathbf{10}, \mathbf{1}),\ (0,1,0,0,0) \mapsto (E, Q, U)$
$(\mathbf{10}, \mathbf{1}),\ (0,1,0,0,0) \mapsto (E, Q, U)$
$(\mathbf{10}, \mathbf{1}),\ (0,1,0,0,0) \mapsto (E, Q, U)$
$(\bar{\mathbf{5}}, \mathbf{2}),\ (0,0,0,1,1) \mapsto (D, D, L, L)$
$(\mathbf{1}, \mathbf{3}),\ (0,0,0,0,2) \mapsto (N, N, N)$
Projection matrix for $\alpha$:

$$\begin{pmatrix} 0 & 0 & 1 & 0 & 0 \\ 0 & 0 & 0 & 1 & 0 \\ 1 & 0 & 0 & 0 & 0 \\ 3 & 6 & 4 & 2 & 0 \end{pmatrix}$$

**3 generation subalgebra** 68
Algebra: $\mathfrak{su}(5) \oplus \mathfrak{su}(2)$
$(\bar{\mathbf{5}}, \mathbf{1}),\ (0,0,0,1,0) \mapsto (D, L)$
$(\bar{\mathbf{5}}, \mathbf{1}),\ (0,0,0,1,0) \mapsto (D, L)$
$(\bar{\mathbf{5}}, \mathbf{1}),\ (0,0,0,1,0) \mapsto (D, L)$
$(\mathbf{10}, \mathbf{1}),\ (0,1,0,0,0) \mapsto (E, Q, U)$
$(\mathbf{10}, \mathbf{1}),\ (0,1,0,0,0) \mapsto (E, Q, U)$
$(\mathbf{10}, \mathbf{1}),\ (0,1,0,0,0) \mapsto (E, Q, U)$
$(\mathbf{1}, \mathbf{2}),\ (0,0,0,0,1) \mapsto (N, N)$
$(\mathbf{1}, \mathbf{1}),\ (0,0,0,0,0) \mapsto (N)$
Projection matrix for $\alpha$:

$$\begin{pmatrix} 0 & 0 & 1 & 0 & 0 \\ 0 & 0 & 0 & 1 & 0 \\ 1 & 0 & 0 & 0 & 0 \\ 3 & 6 & 4 & 2 & 0 \end{pmatrix}$$

**3 generation subalgebra** 69
Algebra: $\mathfrak{su}(5) \oplus \mathfrak{su}(2)$
$(\overline{\mathbf{5}}, \mathbf{1}),\ (0,0,0,1,0) \mapsto (D, L)$
$(\overline{\mathbf{5}}, \mathbf{1}),\ (0,0,0,1,0) \mapsto (D, L)$
$(\overline{\mathbf{5}}, \mathbf{1}),\ (0,0,0,1,0) \mapsto (D, L)$
$(\mathbf{10}, \mathbf{1}),\ (0,1,0,0,0) \mapsto (E, Q, U)$
$(\mathbf{10}, \mathbf{1}),\ (0,1,0,0,0) \mapsto (E, Q, U)$
$(\mathbf{10}, \mathbf{1}),\ (0,1,0,0,0) \mapsto (E, Q, U)$
$(\mathbf{1}, \mathbf{3}),\ (0,0,0,0,2) \mapsto (N, N, N)$
Projection matrix for $\alpha$:

$$\begin{pmatrix} 0 & 0 & 1 & 0 & 0 \\ 0 & 0 & 0 & 1 & 0 \\ 1 & 0 & 0 & 0 & 0 \\ 3 & 6 & 4 & 2 & 0 \end{pmatrix}$$

**3 generation subalgebra** 70
Algebra: $\mathfrak{su}(5) \oplus \mathfrak{su}(5)$
$(\overline{\mathbf{5}}, \mathbf{1}),\ (0,0,0,1,0,0,0,0) \mapsto (D, L)$
$(\overline{\mathbf{5}}, \mathbf{1}),\ (0,0,0,1,0,0,0,0) \mapsto (D, L)$
$(\mathbf{10}, \mathbf{1}),\ (0,1,0,0,0,0,0,0) \mapsto (E, Q, U)$
$(\mathbf{10}, \mathbf{1}),\ (0,1,0,0,0,0,0,0) \mapsto (E, Q, U)$
$(\mathbf{1}, \overline{\mathbf{5}}),\ (0,0,0,0,0,0,0,1) \mapsto (D, L)$
$(\mathbf{1}, \mathbf{10}),\ (0,0,0,0,0,1,0,0) \mapsto (E, Q, U)$
$(\mathbf{1}, \mathbf{1}),\ (0,0,0,0,0,0,0,0) \mapsto (N)$
$(\mathbf{1}, \mathbf{1}),\ (0,0,0,0,0,0,0,0) \mapsto (N)$
$(\mathbf{1}, \mathbf{1}),\ (0,0,0,0,0,0,0,0) \mapsto (N)$
Projection matrix for $\alpha$:

$$\begin{pmatrix} 0 & 0 & 1 & 0 & 0 & 0 & 1 & 0 \\ 0 & 0 & 0 & 1 & 0 & 0 & 0 & 1 \\ 1 & 0 & 0 & 0 & 1 & 0 & 0 & 0 \\ 3 & 6 & 4 & 2 & 3 & 6 & 4 & 2 \end{pmatrix}$$

**3 generation subalgebra** 71
Algebra: $\mathfrak{su}(4) \oplus \mathfrak{sp}(6) \oplus \mathfrak{su}(2)$
$(\overline{\mathbf{4}}, \mathbf{6}, \mathbf{1}),\ (0,0,1,1,0,0,0) \mapsto (L, L, L, Q, Q, Q)$
$(\mathbf{4}, \mathbf{1}, \mathbf{2}),\ (1,0,0,0,0,0,1) \mapsto (D, E, N, U)$
$(\mathbf{4}, \mathbf{1}, \mathbf{2}),\ (1,0,0,0,0,0,1) \mapsto (D, E, N, U)$
$(\mathbf{4}, \mathbf{1}, \mathbf{2}),\ (1,0,0,0,0,0,1) \mapsto (D, E, N, U)$
Projection matrix for $\alpha$:

$$\begin{pmatrix} 0 & 1 & 0 & 0 & 0 & 0 & 0 \\ 1 & 0 & 0 & 0 & 0 & 0 & 0 \\ 0 & 0 & 0 & 1 & 2 & 3 & 0 \\ -1 & -2 & -3 & 0 & 0 & 0 & 3 \end{pmatrix}$$

**3 generation subalgebra** 72
Algebra: $\mathfrak{su}(4) \oplus \mathfrak{sp}(6) \oplus \mathfrak{su}(2)$
$(\overline{\mathbf{4}}, \mathbf{6}, \mathbf{1}),\ (0,0,1,1,0,0,0) \mapsto (D, D, D, E, E, E, N, N, N, U, U, U)$
$(\mathbf{4}, \mathbf{1}, \mathbf{2}),\ (1,0,0,0,0,0,1) \mapsto (L, Q)$
$(\mathbf{4}, \mathbf{1}, \mathbf{2}),\ (1,0,0,0,0,0,1) \mapsto (L, Q)$
$(\mathbf{4}, \mathbf{1}, \mathbf{2}),\ (1,0,0,0,0,0,1) \mapsto (L, Q)$
Projection matrix for $\alpha$:

$$\begin{pmatrix} 1 & 0 & 0 & 0 & 0 & 0 & 0 \\ 0 & 1 & 0 & 0 & 0 & 0 & 0 \\ 0 & 0 & 0 & 0 & 0 & 0 & 1 \\ 1 & 2 & 3 & 3 & 0 & -3 & 0 \end{pmatrix}$$

**3 generation subalgebra** 73
Algebra: $\mathfrak{su}(5) \oplus \mathfrak{so}(10) \oplus \mathfrak{so}(10)$
$(\overline{\mathbf{5}}, \mathbf{1}, \mathbf{1})$, $(0,0,0,1,0,0,0,0,0,0,0,0,0,0) \mapsto (D, L)$
$(\mathbf{10}, \mathbf{1}, \mathbf{1})$, $(0,1,0,0,0,0,0,0,0,0,0,0,0,0) \mapsto (E, Q, U)$
$(\mathbf{1}, \mathbf{16}, \mathbf{1})$, $(0,0,0,0,0,0,0,0,1,0,0,0,0,0) \mapsto (D, E, L, N, Q, U)$
$(\mathbf{1}, \mathbf{1}, \mathbf{16})$, $(0,0,0,0,0,0,0,0,0,0,0,0,0,1) \mapsto (D, E, L, N, Q, U)$
$(\mathbf{1}, \mathbf{1}, \mathbf{1})$, $(0,0,0,0,0,0,0,0,0,0,0,0,0,0) \mapsto (N)$
Projection matrix for $\alpha$:

$$\begin{pmatrix} 0 & 0 & 1 & 0 & 0 & 0 & 1 & 0 & 0 & 0 & 0 & 1 & 0 & 0 \\ 0 & 0 & 0 & 1 & 0 & 0 & 0 & 0 & 1 & 0 & 0 & 0 & 0 & 1 \\ 1 & 0 & 0 & 0 & 1 & 0 & 0 & 0 & 0 & 1 & 0 & 0 & 0 & 0 \\ 3 & 6 & 4 & 2 & 3 & 6 & 4 & 0 & 2 & 3 & 6 & 4 & 0 & 2 \end{pmatrix}$$

**3 generation subalgebra** 74
Algebra: $\mathfrak{su}(5) \oplus \mathfrak{so}(10) \oplus \mathfrak{su}(2)$
$(\mathbf{1}, \mathbf{16}, \mathbf{1})$, $(0,0,0,0,0,0,0,0,1,0) \mapsto (D, E, L, N, Q, U)$
$(\overline{\mathbf{5}}, \mathbf{1}, \mathbf{2})$, $(0,0,0,1,0,0,0,0,0,1) \mapsto (D, D, L, L)$
$(\mathbf{10}, \mathbf{1}, \mathbf{2})$, $(0,1,0,0,0,0,0,0,0,1) \mapsto (E, E, Q, Q, U, U)$
$(\mathbf{1}, \mathbf{1}, \mathbf{1})$, $(0,0,0,0,0,0,0,0,0,0) \mapsto (N)$
$(\mathbf{1}, \mathbf{1}, \mathbf{1})$, $(0,0,0,0,0,0,0,0,0,0) \mapsto (N)$
Projection matrix for $\alpha$:

$$\begin{pmatrix} 0 & 0 & 1 & 0 & 0 & 0 & 1 & 0 & 0 & 0 \\ 0 & 0 & 0 & 1 & 0 & 0 & 0 & 0 & 1 & 0 \\ 1 & 0 & 0 & 0 & 1 & 0 & 0 & 0 & 0 & 0 \\ 3 & 6 & 4 & 2 & 3 & 6 & 4 & 0 & 2 & 0 \end{pmatrix}$$

**3 generation subalgebra** 75
Algebra: $\mathfrak{su}(5) \oplus \mathfrak{so}(10) \oplus \mathfrak{su}(2)$
$(\overline{\mathbf{5}}, \mathbf{1}, \mathbf{1})$, $(0,0,0,1,0,0,0,0,0,0) \mapsto (D, L)$
$(\mathbf{10}, \mathbf{1}, \mathbf{1})$, $(0,1,0,0,0,0,0,0,0,0) \mapsto (E, Q, U)$
$(\mathbf{1}, \mathbf{16}, \mathbf{2})$, $(0,0,0,0,0,0,0,0,1,1) \mapsto (D, D, E, E, L, L, N, N, Q, Q, U, U)$
$(\mathbf{1}, \mathbf{1}, \mathbf{1})$, $(0,0,0,0,0,0,0,0,0,0) \mapsto (N)$
Projection matrix for $\alpha$:

$$\begin{pmatrix} 0 & 0 & 1 & 0 & 0 & 0 & 1 & 0 & 0 & 0 \\ 0 & 0 & 0 & 1 & 0 & 0 & 0 & 0 & 1 & 0 \\ 1 & 0 & 0 & 0 & 1 & 0 & 0 & 0 & 0 & 0 \\ 3 & 6 & 4 & 2 & 3 & 6 & 4 & 0 & 2 & 0 \end{pmatrix}$$

**3 generation subalgebra** 76
Algebra: $\mathfrak{su}(5) \oplus \mathfrak{so}(10) \oplus \mathfrak{su}(2)$
$(\mathbf{1}, \mathbf{16}, \mathbf{1})$, $(0,0,0,0,0,0,0,0,1,0) \mapsto (D, E, L, N, Q, U)$
$(\overline{\mathbf{5}}, \mathbf{1}, \mathbf{2})$, $(0,0,0,1,0,0,0,0,0,1) \mapsto (D, D, L, L)$
$(\mathbf{10}, \mathbf{1}, \mathbf{2})$, $(0,1,0,0,0,0,0,0,0,1) \mapsto (E, E, Q, Q, U, U)$
$(\mathbf{1}, \mathbf{1}, \mathbf{2})$, $(0,0,0,0,0,0,0,0,0,1) \mapsto (N, N)$
Projection matrix for $\alpha$:

$$\begin{pmatrix} 0 & 0 & 1 & 0 & 0 & 0 & 1 & 0 & 0 & 0 \\ 0 & 0 & 0 & 1 & 0 & 0 & 0 & 0 & 1 & 0 \\ 1 & 0 & 0 & 0 & 1 & 0 & 0 & 0 & 0 & 0 \\ 3 & 6 & 4 & 2 & 3 & 6 & 4 & 0 & 2 & 0 \end{pmatrix}$$

**3 generation subalgebra** 77
Algebra: $\mathfrak{su}(5) \oplus \mathfrak{so}(10) \oplus \mathfrak{su}(2)$
$(\overline{\mathbf{5}}, \mathbf{1}, \mathbf{1})$, $(0,0,0,1,0,0,0,0,0,0) \mapsto (D, L)$
$(\overline{\mathbf{5}}, \mathbf{1}, \mathbf{1})$, $(0,0,0,1,0,0,0,0,0,0) \mapsto (D, L)$
$(\mathbf{1}, \mathbf{16}, \mathbf{1})$, $(0,0,0,0,0,0,0,0,1,0) \mapsto (D, E, L, N, Q, U)$
$(\mathbf{10}, \mathbf{1}, \mathbf{2})$, $(0,1,0,0,0,0,0,0,0,1) \mapsto (E, E, Q, Q, U, U)$

$(\mathbf{1},\mathbf{1},\mathbf{1}),\ (0,0,0,0,0,0,0,0,0,0) \mapsto (N)$
$(\mathbf{1},\mathbf{1},\mathbf{1}),\ (0,0,0,0,0,0,0,0,0,0) \mapsto (N)$
Projection matrix for $\alpha$:

$$\begin{pmatrix} 0 & 0 & 1 & 0 & 0 & 0 & 1 & 0 & 0 & 0 \\ 0 & 0 & 0 & 1 & 0 & 0 & 0 & 0 & 1 & 0 \\ 1 & 0 & 0 & 0 & 1 & 0 & 0 & 0 & 0 & 0 \\ 3 & 6 & 4 & 2 & 3 & 6 & 4 & 0 & 2 & 0 \end{pmatrix}$$

**3 generation subalgebra** 78
Algebra: $\mathfrak{su}(5) \oplus \mathfrak{so}(10) \oplus \mathfrak{su}(2)$
$(\mathbf{10},\mathbf{1},\mathbf{1}),\ (0,1,0,0,0,0,0,0,0,0) \mapsto (E,Q,U)$
$(\mathbf{10},\mathbf{1},\mathbf{1}),\ (0,1,0,0,0,0,0,0,0,0) \mapsto (E,Q,U)$
$(\mathbf{1},\mathbf{16},\mathbf{1}),\ (0,0,0,0,0,0,0,0,1,0) \mapsto (D,E,L,N,Q,U)$
$(\overline{\mathbf{5}},\mathbf{1},\mathbf{2}),\ (0,0,0,1,0,0,0,0,0,1) \mapsto (D,D,L,L)$
$(\mathbf{1},\mathbf{1},\mathbf{1}),\ (0,0,0,0,0,0,0,0,0,0) \mapsto (N)$
$(\mathbf{1},\mathbf{1},\mathbf{1}),\ (0,0,0,0,0,0,0,0,0,0) \mapsto (N)$
Projection matrix for $\alpha$:

$$\begin{pmatrix} 0 & 0 & 1 & 0 & 0 & 0 & 1 & 0 & 0 & 0 \\ 0 & 0 & 0 & 1 & 0 & 0 & 0 & 0 & 1 & 0 \\ 1 & 0 & 0 & 0 & 1 & 0 & 0 & 0 & 0 & 0 \\ 3 & 6 & 4 & 2 & 3 & 6 & 4 & 0 & 2 & 0 \end{pmatrix}$$

**3 generation subalgebra** 79
Algebra: $\mathfrak{su}(5) \oplus \mathfrak{so}(10) \oplus \mathfrak{su}(2)$
$(\overline{\mathbf{5}},\mathbf{1},\mathbf{1}),\ (0,0,0,1,0,0,0,0,0,0) \mapsto (D,L)$
$(\overline{\mathbf{5}},\mathbf{1},\mathbf{1}),\ (0,0,0,1,0,0,0,0,0,0) \mapsto (D,L)$
$(\mathbf{1},\mathbf{16},\mathbf{1}),\ (0,0,0,0,0,0,0,0,1,0) \mapsto (D,E,L,N,Q,U)$
$(\mathbf{10},\mathbf{1},\mathbf{2}),\ (0,1,0,0,0,0,0,0,0,1) \mapsto (E,E,Q,Q,U,U)$
$(\mathbf{1},\mathbf{1},\mathbf{2}),\ (0,0,0,0,0,0,0,0,0,1) \mapsto (N,N)$
Projection matrix for $\alpha$:

$$\begin{pmatrix} 0 & 0 & 1 & 0 & 0 & 0 & 1 & 0 & 0 & 0 \\ 0 & 0 & 0 & 1 & 0 & 0 & 0 & 0 & 1 & 0 \\ 1 & 0 & 0 & 0 & 1 & 0 & 0 & 0 & 0 & 0 \\ 3 & 6 & 4 & 2 & 3 & 6 & 4 & 0 & 2 & 0 \end{pmatrix}$$

**3 generation subalgebra** 80
Algebra: $\mathfrak{su}(5) \oplus \mathfrak{so}(10) \oplus \mathfrak{su}(2)$
$(\mathbf{10},\mathbf{1},\mathbf{1}),\ (0,1,0,0,0,0,0,0,0,0) \mapsto (E,Q,U)$
$(\mathbf{10},\mathbf{1},\mathbf{1}),\ (0,1,0,0,0,0,0,0,0,0) \mapsto (E,Q,U)$
$(\mathbf{1},\mathbf{16},\mathbf{1}),\ (0,0,0,0,0,0,0,0,1,0) \mapsto (D,E,L,N,Q,U)$
$(\overline{\mathbf{5}},\mathbf{1},\mathbf{2}),\ (0,0,0,1,0,0,0,0,0,1) \mapsto (D,D,L,L)$
$(\mathbf{1},\mathbf{1},\mathbf{2}),\ (0,0,0,0,0,0,0,0,0,1) \mapsto (N,N)$
Projection matrix for $\alpha$:

$$\begin{pmatrix} 0 & 0 & 1 & 0 & 0 & 0 & 1 & 0 & 0 & 0 \\ 0 & 0 & 0 & 1 & 0 & 0 & 0 & 0 & 1 & 0 \\ 1 & 0 & 0 & 0 & 1 & 0 & 0 & 0 & 0 & 0 \\ 3 & 6 & 4 & 2 & 3 & 6 & 4 & 0 & 2 & 0 \end{pmatrix}$$

**3 generation subalgebra** 81
Algebra: $\mathfrak{su}(5) \oplus \mathfrak{so}(10) \oplus \mathfrak{su}(2)$
$(\overline{\mathbf{5}},\mathbf{1},\mathbf{1}),\ (0,0,0,1,0,0,0,0,0,0) \mapsto (D,L)$
$(\overline{\mathbf{5}},\mathbf{1},\mathbf{1}),\ (0,0,0,1,0,0,0,0,0,0) \mapsto (D,L)$
$(\mathbf{10},\mathbf{1},\mathbf{1}),\ (0,1,0,0,0,0,0,0,0,0) \mapsto (E,Q,U)$
$(\mathbf{10},\mathbf{1},\mathbf{1}),\ (0,1,0,0,0,0,0,0,0,0) \mapsto (E,Q,U)$
$(\mathbf{1},\mathbf{16},\mathbf{1}),\ (0,0,0,0,0,0,0,0,1,0) \mapsto (D,E,L,N,Q,U)$

$(\mathbf{1},\mathbf{1},\mathbf{2})$, $(0,0,0,0,0,0,0,0,0,1) \mapsto (N,N)$
Projection matrix for $\alpha$:

$$\begin{pmatrix} 0&0&1&0&0&0&1&0&0&0\\ 0&0&0&1&0&0&0&0&1&0\\ 1&0&0&0&1&0&0&0&0&0\\ 3&6&4&2&3&6&4&0&2&0 \end{pmatrix}$$

**3 generation subalgebra** 82
Algebra: $\mathfrak{su}(5) \oplus \mathfrak{su}(2) \oplus \mathfrak{su}(2)$
$(\overline{\mathbf{5}},\mathbf{3},\mathbf{1})$, $(0,0,0,1,2,0) \mapsto (D,D,D,L,L,L)$
$(\mathbf{10},\mathbf{1},\mathbf{3})$, $(0,1,0,0,0,2) \mapsto (E,E,E,Q,Q,Q,U,U,U)$
$(\mathbf{1},\mathbf{1},\mathbf{1})$, $(0,0,0,0,0,0) \mapsto (N)$
$(\mathbf{1},\mathbf{1},\mathbf{1})$, $(0,0,0,0,0,0) \mapsto (N)$
$(\mathbf{1},\mathbf{1},\mathbf{1})$, $(0,0,0,0,0,0) \mapsto (N)$
Projection matrix for $\alpha$:

$$\begin{pmatrix} 0&0&1&0&0&0\\ 0&0&0&1&0&0\\ 1&0&0&0&0&0\\ 3&6&4&2&0&0 \end{pmatrix}$$

**3 generation subalgebra** 83
Algebra: $\mathfrak{su}(5) \oplus \mathfrak{su}(2) \oplus \mathfrak{su}(2)$
$(\overline{\mathbf{5}},\mathbf{1},\mathbf{1})$, $(0,0,0,1,0,0) \mapsto (D,L)$
$(\overline{\mathbf{5}},\mathbf{2},\mathbf{1})$, $(0,0,0,1,1,0) \mapsto (D,D,L,L)$
$(\mathbf{10},\mathbf{1},\mathbf{3})$, $(0,1,0,0,0,2) \mapsto (E,E,E,Q,Q,Q,U,U,U)$
$(\mathbf{1},\mathbf{1},\mathbf{1})$, $(0,0,0,0,0,0) \mapsto (N)$
$(\mathbf{1},\mathbf{1},\mathbf{1})$, $(0,0,0,0,0,0) \mapsto (N)$
$(\mathbf{1},\mathbf{1},\mathbf{1})$, $(0,0,0,0,0,0) \mapsto (N)$
Projection matrix for $\alpha$:

$$\begin{pmatrix} 0&0&1&0&0&0\\ 0&0&0&1&0&0\\ 1&0&0&0&0&0\\ 3&6&4&2&0&0 \end{pmatrix}$$

**3 generation subalgebra** 84
Algebra: $\mathfrak{su}(5) \oplus \mathfrak{su}(2) \oplus \mathfrak{su}(2)$
$(\overline{\mathbf{5}},\mathbf{3},\mathbf{1})$, $(0,0,0,1,2,0) \mapsto (D,D,D,L,L,L)$
$(\mathbf{10},\mathbf{1},\mathbf{3})$, $(0,1,0,0,0,2) \mapsto (E,E,E,Q,Q,Q,U,U,U)$
$(\mathbf{1},\mathbf{1},\mathbf{2})$, $(0,0,0,0,0,1) \mapsto (N,N)$
$(\mathbf{1},\mathbf{1},\mathbf{1})$, $(0,0,0,0,0,0) \mapsto (N)$
Projection matrix for $\alpha$:

$$\begin{pmatrix} 0&0&1&0&0&0\\ 0&0&0&1&0&0\\ 1&0&0&0&0&0\\ 3&6&4&2&0&0 \end{pmatrix}$$

**3 generation subalgebra** 85
Algebra: $\mathfrak{su}(5) \oplus \mathfrak{su}(2) \oplus \mathfrak{su}(2)$
$(\overline{\mathbf{5}},\mathbf{3},\mathbf{1})$, $(0,0,0,1,2,0) \mapsto (D,D,D,L,L,L)$
$(\mathbf{10},\mathbf{1},\mathbf{3})$, $(0,1,0,0,0,2) \mapsto (E,E,E,Q,Q,Q,U,U,U)$
$(\mathbf{1},\mathbf{1},\mathbf{3})$, $(0,0,0,0,0,2) \mapsto (N,N,N)$
Projection matrix for $\alpha$:

$$\begin{pmatrix} 0&0&1&0&0&0\\ 0&0&0&1&0&0\\ 1&0&0&0&0&0\\ 3&6&4&2&0&0 \end{pmatrix}$$

**3 generation subalgebra** 86
Algebra: $\mathfrak{su}(5) \oplus \mathfrak{su}(2) \oplus \mathfrak{su}(2)$
$(\overline{\mathbf{5}}, \mathbf{3}, \mathbf{1})$, $(0,0,0,1,2,0) \mapsto (D,D,D,L,L,L)$
$(\mathbf{10}, \mathbf{1}, \mathbf{3})$, $(0,1,0,0,0,2) \mapsto (E,E,E,Q,Q,Q,U,U,U)$
$(\mathbf{1}, \mathbf{2}, \mathbf{1})$, $(0,0,0,0,1,0) \mapsto (N,N)$
$(\mathbf{1}, \mathbf{1}, \mathbf{1})$, $(0,0,0,0,0,0) \mapsto (N)$
Projection matrix for $\alpha$:

$$\begin{pmatrix} 0 & 0 & 1 & 0 & 0 & 0 \\ 0 & 0 & 0 & 1 & 0 & 0 \\ 1 & 0 & 0 & 0 & 0 & 0 \\ 3 & 6 & 4 & 2 & 0 & 0 \end{pmatrix}$$

**3 generation subalgebra** 87
Algebra: $\mathfrak{su}(5) \oplus \mathfrak{su}(2) \oplus \mathfrak{su}(2)$
$(\overline{\mathbf{5}}, \mathbf{3}, \mathbf{1})$, $(0,0,0,1,2,0) \mapsto (D,D,D,L,L,L)$
$(\mathbf{10}, \mathbf{1}, \mathbf{3})$, $(0,1,0,0,0,2) \mapsto (E,E,E,Q,Q,Q,U,U,U)$
$(\mathbf{1}, \mathbf{3}, \mathbf{1})$, $(0,0,0,0,2,0) \mapsto (N,N,N)$
Projection matrix for $\alpha$:

$$\begin{pmatrix} 0 & 0 & 1 & 0 & 0 & 0 \\ 0 & 0 & 0 & 1 & 0 & 0 \\ 1 & 0 & 0 & 0 & 0 & 0 \\ 3 & 6 & 4 & 2 & 0 & 0 \end{pmatrix}$$

**3 generation subalgebra** 88
Algebra: $\mathfrak{su}(5) \oplus \mathfrak{su}(2) \oplus \mathfrak{su}(2)$
$(\overline{\mathbf{5}}, \mathbf{3}, \mathbf{1})$, $(0,0,0,1,2,0) \mapsto (D,D,D,L,L,L)$
$(\mathbf{10}, \mathbf{3}, \mathbf{1})$, $(0,1,0,0,2,0) \mapsto (E,E,E,Q,Q,Q,U,U,U)$
$(\mathbf{1}, \mathbf{1}, \mathbf{2})$, $(0,0,0,0,0,1) \mapsto (N,N)$
$(\mathbf{1}, \mathbf{1}, \mathbf{1})$, $(0,0,0,0,0,0) \mapsto (N)$
Projection matrix for $\alpha$:

$$\begin{pmatrix} 0 & 0 & 1 & 0 & 0 & 0 \\ 0 & 0 & 0 & 1 & 0 & 0 \\ 1 & 0 & 0 & 0 & 0 & 0 \\ 3 & 6 & 4 & 2 & 0 & 0 \end{pmatrix}$$

**3 generation subalgebra** 89
Algebra: $\mathfrak{su}(5) \oplus \mathfrak{su}(2) \oplus \mathfrak{su}(2)$
$(\overline{\mathbf{5}}, \mathbf{3}, \mathbf{1})$, $(0,0,0,1,2,0) \mapsto (D,D,D,L,L,L)$
$(\mathbf{10}, \mathbf{3}, \mathbf{1})$, $(0,1,0,0,2,0) \mapsto (E,E,E,Q,Q,Q,U,U,U)$
$(\mathbf{1}, \mathbf{1}, \mathbf{3})$, $(0,0,0,0,0,2) \mapsto (N,N,N)$
Projection matrix for $\alpha$:

$$\begin{pmatrix} 0 & 0 & 1 & 0 & 0 & 0 \\ 0 & 0 & 0 & 1 & 0 & 0 \\ 1 & 0 & 0 & 0 & 0 & 0 \\ 3 & 6 & 4 & 2 & 0 & 0 \end{pmatrix}$$

**3 generation subalgebra** 90
Algebra: $\mathfrak{su}(5) \oplus \mathfrak{su}(2) \oplus \mathfrak{su}(2)$
$(\mathbf{10}, \mathbf{1}, \mathbf{1})$, $(0,1,0,0,0,0) \mapsto (E,Q,U)$
$(\overline{\mathbf{5}}, \mathbf{3}, \mathbf{1})$, $(0,0,0,1,2,0) \mapsto (D,D,D,L,L,L)$
$(\mathbf{10}, \mathbf{1}, \mathbf{2})$, $(0,1,0,0,0,1) \mapsto (E,E,Q,Q,U,U)$
$(\mathbf{1}, \mathbf{1}, \mathbf{1})$, $(0,0,0,0,0,0) \mapsto (N)$
$(\mathbf{1}, \mathbf{1}, \mathbf{1})$, $(0,0,0,0,0,0) \mapsto (N)$
$(\mathbf{1}, \mathbf{1}, \mathbf{1})$, $(0,0,0,0,0,0) \mapsto (N)$

Projection matrix for $\alpha$:

$$\begin{pmatrix} 0 & 0 & 1 & 0 & 0 & 0 \\ 0 & 0 & 0 & 1 & 0 & 0 \\ 1 & 0 & 0 & 0 & 0 & 0 \\ 3 & 6 & 4 & 2 & 0 & 0 \end{pmatrix}$$

**3 generation subalgebra** 91
Algebra: $\mathfrak{su}(5) \oplus \mathfrak{su}(2) \oplus \mathfrak{su}(2)$
$(\overline{\mathbf{5}}, \mathbf{1}, \mathbf{1})$, $(0, 0, 0, 1, 0, 0) \mapsto (D, L)$
$(\overline{\mathbf{5}}, \mathbf{2}, \mathbf{1})$, $(0, 0, 0, 1, 1, 0) \mapsto (D, D, L, L)$
$(\mathbf{10}, \mathbf{1}, \mathbf{3})$, $(0, 1, 0, 0, 0, 2) \mapsto (E, E, E, Q, Q, Q, U, U, U)$
$(\mathbf{1}, \mathbf{1}, \mathbf{2})$, $(0, 0, 0, 0, 0, 1) \mapsto (N, N)$
$(\mathbf{1}, \mathbf{1}, \mathbf{1})$, $(0, 0, 0, 0, 0, 0) \mapsto (N)$
Projection matrix for $\alpha$:

$$\begin{pmatrix} 0 & 0 & 1 & 0 & 0 & 0 \\ 0 & 0 & 0 & 1 & 0 & 0 \\ 1 & 0 & 0 & 0 & 0 & 0 \\ 3 & 6 & 4 & 2 & 0 & 0 \end{pmatrix}$$

**3 generation subalgebra** 92
Algebra: $\mathfrak{su}(5) \oplus \mathfrak{su}(2) \oplus \mathfrak{su}(2)$
$(\overline{\mathbf{5}}, \mathbf{1}, \mathbf{1})$, $(0, 0, 0, 1, 0, 0) \mapsto (D, L)$
$(\overline{\mathbf{5}}, \mathbf{2}, \mathbf{1})$, $(0, 0, 0, 1, 1, 0) \mapsto (D, D, L, L)$
$(\mathbf{10}, \mathbf{1}, \mathbf{3})$, $(0, 1, 0, 0, 0, 2) \mapsto (E, E, E, Q, Q, Q, U, U, U)$
$(\mathbf{1}, \mathbf{1}, \mathbf{3})$, $(0, 0, 0, 0, 0, 2) \mapsto (N, N, N)$
Projection matrix for $\alpha$:

$$\begin{pmatrix} 0 & 0 & 1 & 0 & 0 & 0 \\ 0 & 0 & 0 & 1 & 0 & 0 \\ 1 & 0 & 0 & 0 & 0 & 0 \\ 3 & 6 & 4 & 2 & 0 & 0 \end{pmatrix}$$

**3 generation subalgebra** 93
Algebra: $\mathfrak{su}(5) \oplus \mathfrak{su}(2) \oplus \mathfrak{su}(2)$
$(\overline{\mathbf{5}}, \mathbf{1}, \mathbf{1})$, $(0, 0, 0, 1, 0, 0) \mapsto (D, L)$
$(\overline{\mathbf{5}}, \mathbf{2}, \mathbf{1})$, $(0, 0, 0, 1, 1, 0) \mapsto (D, D, L, L)$
$(\mathbf{10}, \mathbf{1}, \mathbf{3})$, $(0, 1, 0, 0, 0, 2) \mapsto (E, E, E, Q, Q, Q, U, U, U)$
$(\mathbf{1}, \mathbf{2}, \mathbf{1})$, $(0, 0, 0, 0, 1, 0) \mapsto (N, N)$
$(\mathbf{1}, \mathbf{1}, \mathbf{1})$, $(0, 0, 0, 0, 0, 0) \mapsto (N)$
Projection matrix for $\alpha$:

$$\begin{pmatrix} 0 & 0 & 1 & 0 & 0 & 0 \\ 0 & 0 & 0 & 1 & 0 & 0 \\ 1 & 0 & 0 & 0 & 0 & 0 \\ 3 & 6 & 4 & 2 & 0 & 0 \end{pmatrix}$$

**3 generation subalgebra** 94
Algebra: $\mathfrak{su}(5) \oplus \mathfrak{su}(2) \oplus \mathfrak{su}(2)$
$(\overline{\mathbf{5}}, \mathbf{1}, \mathbf{1})$, $(0, 0, 0, 1, 0, 0) \mapsto (D, L)$
$(\overline{\mathbf{5}}, \mathbf{2}, \mathbf{1})$, $(0, 0, 0, 1, 1, 0) \mapsto (D, D, L, L)$
$(\mathbf{10}, \mathbf{1}, \mathbf{3})$, $(0, 1, 0, 0, 0, 2) \mapsto (E, E, E, Q, Q, Q, U, U, U)$
$(\mathbf{1}, \mathbf{3}, \mathbf{1})$, $(0, 0, 0, 0, 2, 0) \mapsto (N, N, N)$
Projection matrix for $\alpha$:

$$\begin{pmatrix} 0 & 0 & 1 & 0 & 0 & 0 \\ 0 & 0 & 0 & 1 & 0 & 0 \\ 1 & 0 & 0 & 0 & 0 & 0 \\ 3 & 6 & 4 & 2 & 0 & 0 \end{pmatrix}$$

**3 generation subalgebra** 95
Algebra: $\mathfrak{su}(5) \oplus \mathfrak{su}(2) \oplus \mathfrak{su}(2)$
$(\overline{\mathbf{5}}, \mathbf{1}, \mathbf{1})$, $(0,0,0,1,0,0) \mapsto (D, L)$
$(\overline{\mathbf{5}}, \mathbf{2}, \mathbf{1})$, $(0,0,0,1,1,0) \mapsto (D, D, L, L)$
$(\mathbf{10}, \mathbf{3}, \mathbf{1})$, $(0,1,0,0,2,0) \mapsto (E, E, E, Q, Q, Q, U, U, U)$
$(\mathbf{1}, \mathbf{1}, \mathbf{2})$, $(0,0,0,0,0,1) \mapsto (N, N)$
$(\mathbf{1}, \mathbf{1}, \mathbf{1})$, $(0,0,0,0,0,0) \mapsto (N)$
Projection matrix for $\alpha$:

$$\begin{pmatrix} 0 & 0 & 1 & 0 & 0 & 0 \\ 0 & 0 & 0 & 1 & 0 & 0 \\ 1 & 0 & 0 & 0 & 0 & 0 \\ 3 & 6 & 4 & 2 & 0 & 0 \end{pmatrix}$$

**3 generation subalgebra** 96
Algebra: $\mathfrak{su}(5) \oplus \mathfrak{su}(2) \oplus \mathfrak{su}(2)$
$(\overline{\mathbf{5}}, \mathbf{1}, \mathbf{1})$, $(0,0,0,1,0,0) \mapsto (D, L)$
$(\overline{\mathbf{5}}, \mathbf{2}, \mathbf{1})$, $(0,0,0,1,1,0) \mapsto (D, D, L, L)$
$(\mathbf{10}, \mathbf{3}, \mathbf{1})$, $(0,1,0,0,2,0) \mapsto (E, E, E, Q, Q, Q, U, U, U)$
$(\mathbf{1}, \mathbf{1}, \mathbf{3})$, $(0,0,0,0,0,2) \mapsto (N, N, N)$
Projection matrix for $\alpha$:

$$\begin{pmatrix} 0 & 0 & 1 & 0 & 0 & 0 \\ 0 & 0 & 0 & 1 & 0 & 0 \\ 1 & 0 & 0 & 0 & 0 & 0 \\ 3 & 6 & 4 & 2 & 0 & 0 \end{pmatrix}$$

**3 generation subalgebra** 97
Algebra: $\mathfrak{su}(5) \oplus \mathfrak{su}(2) \oplus \mathfrak{su}(2)$
$(\overline{\mathbf{5}}, \mathbf{1}, \mathbf{1})$, $(0,0,0,1,0,0) \mapsto (D, L)$
$(\mathbf{10}, \mathbf{1}, \mathbf{1})$, $(0,1,0,0,0,0) \mapsto (E, Q, U)$
$(\overline{\mathbf{5}}, \mathbf{2}, \mathbf{1})$, $(0,0,0,1,1,0) \mapsto (D, D, L, L)$
$(\mathbf{10}, \mathbf{1}, \mathbf{2})$, $(0,1,0,0,0,1) \mapsto (E, E, Q, Q, U, U)$
$(\mathbf{1}, \mathbf{1}, \mathbf{1})$, $(0,0,0,0,0,0) \mapsto (N)$
$(\mathbf{1}, \mathbf{1}, \mathbf{1})$, $(0,0,0,0,0,0) \mapsto (N)$
$(\mathbf{1}, \mathbf{1}, \mathbf{1})$, $(0,0,0,0,0,0) \mapsto (N)$
Projection matrix for $\alpha$:

$$\begin{pmatrix} 0 & 0 & 1 & 0 & 0 & 0 \\ 0 & 0 & 0 & 1 & 0 & 0 \\ 1 & 0 & 0 & 0 & 0 & 0 \\ 3 & 6 & 4 & 2 & 0 & 0 \end{pmatrix}$$

**3 generation subalgebra** 98
Algebra: $\mathfrak{su}(5) \oplus \mathfrak{su}(2) \oplus \mathfrak{su}(2)$
$(\mathbf{10}, \mathbf{1}, \mathbf{1})$, $(0,1,0,0,0,0) \mapsto (E, Q, U)$
$(\overline{\mathbf{5}}, \mathbf{3}, \mathbf{1})$, $(0,0,0,1,2,0) \mapsto (D, D, D, L, L, L)$
$(\mathbf{10}, \mathbf{1}, \mathbf{2})$, $(0,1,0,0,0,1) \mapsto (E, E, Q, Q, U, U)$
$(\mathbf{1}, \mathbf{1}, \mathbf{2})$, $(0,0,0,0,0,1) \mapsto (N, N)$
$(\mathbf{1}, \mathbf{1}, \mathbf{1})$, $(0,0,0,0,0,0) \mapsto (N)$
Projection matrix for $\alpha$:

$$\begin{pmatrix} 0 & 0 & 1 & 0 & 0 & 0 \\ 0 & 0 & 0 & 1 & 0 & 0 \\ 1 & 0 & 0 & 0 & 0 & 0 \\ 3 & 6 & 4 & 2 & 0 & 0 \end{pmatrix}$$

**3 generation subalgebra** 99
Algebra: $\mathfrak{su}(5) \oplus \mathfrak{su}(2) \oplus \mathfrak{su}(2)$
$(\mathbf{10}, \mathbf{1}, \mathbf{1})$, $(0,1,0,0,0,0) \mapsto (E, Q, U)$

$(\overline{\mathbf{5}},\mathbf{3},\mathbf{1})$, $(0,0,0,1,2,0) \mapsto (D,D,D,L,L,L)$
$(\mathbf{10},\mathbf{1},\mathbf{2})$, $(0,1,0,0,0,1) \mapsto (E,E,Q,Q,U,U)$
$(\mathbf{1},\mathbf{1},\mathbf{3})$, $(0,0,0,0,0,2) \mapsto (N,N,N)$
Projection matrix for $\alpha$:

$$\begin{pmatrix} 0 & 0 & 1 & 0 & 0 & 0 \\ 0 & 0 & 0 & 1 & 0 & 0 \\ 1 & 0 & 0 & 0 & 0 & 0 \\ 3 & 6 & 4 & 2 & 0 & 0 \end{pmatrix}$$

**3 generation subalgebra** 100
Algebra: $\mathfrak{su}(5) \oplus \mathfrak{su}(2) \oplus \mathfrak{su}(2)$
$(\mathbf{10},\mathbf{1},\mathbf{1})$, $(0,1,0,0,0,0) \mapsto (E,Q,U)$
$(\overline{\mathbf{5}},\mathbf{3},\mathbf{1})$, $(0,0,0,1,2,0) \mapsto (D,D,D,L,L,L)$
$(\mathbf{10},\mathbf{1},\mathbf{2})$, $(0,1,0,0,0,1) \mapsto (E,E,Q,Q,U,U)$
$(\mathbf{1},\mathbf{2},\mathbf{1})$, $(0,0,0,0,1,0) \mapsto (N,N)$
$(\mathbf{1},\mathbf{1},\mathbf{1})$, $(0,0,0,0,0,0) \mapsto (N)$
Projection matrix for $\alpha$:

$$\begin{pmatrix} 0 & 0 & 1 & 0 & 0 & 0 \\ 0 & 0 & 0 & 1 & 0 & 0 \\ 1 & 0 & 0 & 0 & 0 & 0 \\ 3 & 6 & 4 & 2 & 0 & 0 \end{pmatrix}$$

**3 generation subalgebra** 101
Algebra: $\mathfrak{su}(5) \oplus \mathfrak{su}(2) \oplus \mathfrak{su}(2)$
$(\mathbf{10},\mathbf{1},\mathbf{1})$, $(0,1,0,0,0,0) \mapsto (E,Q,U)$
$(\overline{\mathbf{5}},\mathbf{3},\mathbf{1})$, $(0,0,0,1,2,0) \mapsto (D,D,D,L,L,L)$
$(\mathbf{10},\mathbf{1},\mathbf{2})$, $(0,1,0,0,0,1) \mapsto (E,E,Q,Q,U,U)$
$(\mathbf{1},\mathbf{3},\mathbf{1})$, $(0,0,0,0,2,0) \mapsto (N,N,N)$
Projection matrix for $\alpha$:

$$\begin{pmatrix} 0 & 0 & 1 & 0 & 0 & 0 \\ 0 & 0 & 0 & 1 & 0 & 0 \\ 1 & 0 & 0 & 0 & 0 & 0 \\ 3 & 6 & 4 & 2 & 0 & 0 \end{pmatrix}$$

**3 generation subalgebra** 102
Algebra: $\mathfrak{su}(5) \oplus \mathfrak{su}(2) \oplus \mathfrak{su}(2)$
$(\mathbf{10},\mathbf{1},\mathbf{1})$, $(0,1,0,0,0,0) \mapsto (E,Q,U)$
$(\overline{\mathbf{5}},\mathbf{3},\mathbf{1})$, $(0,0,0,1,2,0) \mapsto (D,D,D,L,L,L)$
$(\mathbf{10},\mathbf{2},\mathbf{1})$, $(0,1,0,0,1,0) \mapsto (E,E,Q,Q,U,U)$
$(\mathbf{1},\mathbf{1},\mathbf{2})$, $(0,0,0,0,0,1) \mapsto (N,N)$
$(\mathbf{1},\mathbf{1},\mathbf{1})$, $(0,0,0,0,0,0) \mapsto (N)$
Projection matrix for $\alpha$:

$$\begin{pmatrix} 0 & 0 & 1 & 0 & 0 & 0 \\ 0 & 0 & 0 & 1 & 0 & 0 \\ 1 & 0 & 0 & 0 & 0 & 0 \\ 3 & 6 & 4 & 2 & 0 & 0 \end{pmatrix}$$

**3 generation subalgebra** 103
Algebra: $\mathfrak{su}(5) \oplus \mathfrak{su}(2) \oplus \mathfrak{su}(2)$
$(\mathbf{10},\mathbf{1},\mathbf{1})$, $(0,1,0,0,0,0) \mapsto (E,Q,U)$
$(\overline{\mathbf{5}},\mathbf{3},\mathbf{1})$, $(0,0,0,1,2,0) \mapsto (D,D,D,L,L,L)$
$(\mathbf{10},\mathbf{2},\mathbf{1})$, $(0,1,0,0,1,0) \mapsto (E,E,Q,Q,U,U)$
$(\mathbf{1},\mathbf{1},\mathbf{3})$, $(0,0,0,0,0,2) \mapsto (N,N,N)$
Projection matrix for $\alpha$:

$$\begin{pmatrix} 0 & 0 & 1 & 0 & 0 & 0 \\ 0 & 0 & 0 & 1 & 0 & 0 \\ 1 & 0 & 0 & 0 & 0 & 0 \\ 3 & 6 & 4 & 2 & 0 & 0 \end{pmatrix}$$

**3 generation subalgebra** 104
Algebra: $\mathfrak{su}(5) \oplus \mathfrak{su}(2) \oplus \mathfrak{su}(2)$
$(\overline{\mathbf{5}}, \mathbf{1}, \mathbf{1})$, $(0,0,0,1,0,0) \mapsto (D, L)$
$(\overline{\mathbf{5}}, \mathbf{1}, \mathbf{1})$, $(0,0,0,1,0,0) \mapsto (D, L)$
$(\overline{\mathbf{5}}, \mathbf{1}, \mathbf{1})$, $(0,0,0,1,0,0) \mapsto (D, L)$
$(\mathbf{10}, \mathbf{3}, \mathbf{1})$, $(0,1,0,0,2,0) \mapsto (E, E, E, Q, Q, Q, U, U, U)$
$(\mathbf{1}, \mathbf{1}, \mathbf{2})$, $(0,0,0,0,0,1) \mapsto (N, N)$
$(\mathbf{1}, \mathbf{1}, \mathbf{1})$, $(0,0,0,0,0,0) \mapsto (N)$
Projection matrix for $\alpha$:

$$\begin{pmatrix} 0 & 0 & 1 & 0 & 0 & 0 \\ 0 & 0 & 0 & 1 & 0 & 0 \\ 1 & 0 & 0 & 0 & 0 & 0 \\ 3 & 6 & 4 & 2 & 0 & 0 \end{pmatrix}$$

**3 generation subalgebra** 105
Algebra: $\mathfrak{su}(5) \oplus \mathfrak{su}(2) \oplus \mathfrak{su}(2)$
$(\overline{\mathbf{5}}, \mathbf{1}, \mathbf{1})$, $(0,0,0,1,0,0) \mapsto (D, L)$
$(\overline{\mathbf{5}}, \mathbf{1}, \mathbf{1})$, $(0,0,0,1,0,0) \mapsto (D, L)$
$(\overline{\mathbf{5}}, \mathbf{1}, \mathbf{1})$, $(0,0,0,1,0,0) \mapsto (D, L)$
$(\mathbf{10}, \mathbf{3}, \mathbf{1})$, $(0,1,0,0,2,0) \mapsto (E, E, E, Q, Q, Q, U, U, U)$
$(\mathbf{1}, \mathbf{1}, \mathbf{3})$, $(0,0,0,0,0,2) \mapsto (N, N, N)$
Projection matrix for $\alpha$:

$$\begin{pmatrix} 0 & 0 & 1 & 0 & 0 & 0 \\ 0 & 0 & 0 & 1 & 0 & 0 \\ 1 & 0 & 0 & 0 & 0 & 0 \\ 3 & 6 & 4 & 2 & 0 & 0 \end{pmatrix}$$

**3 generation subalgebra** 106
Algebra: $\mathfrak{su}(5) \oplus \mathfrak{su}(2) \oplus \mathfrak{su}(2)$
$(\overline{\mathbf{5}}, \mathbf{1}, \mathbf{1})$, $(0,0,0,1,0,0) \mapsto (D, L)$
$(\mathbf{10}, \mathbf{1}, \mathbf{1})$, $(0,1,0,0,0,0) \mapsto (E, Q, U)$
$(\overline{\mathbf{5}}, \mathbf{2}, \mathbf{1})$, $(0,0,0,1,1,0) \mapsto (D, D, L, L)$
$(\mathbf{10}, \mathbf{1}, \mathbf{2})$, $(0,1,0,0,0,1) \mapsto (E, E, Q, Q, U, U)$
$(\mathbf{1}, \mathbf{1}, \mathbf{2})$, $(0,0,0,0,0,1) \mapsto (N, N)$
$(\mathbf{1}, \mathbf{1}, \mathbf{1})$, $(0,0,0,0,0,0) \mapsto (N)$
Projection matrix for $\alpha$:

$$\begin{pmatrix} 0 & 0 & 1 & 0 & 0 & 0 \\ 0 & 0 & 0 & 1 & 0 & 0 \\ 1 & 0 & 0 & 0 & 0 & 0 \\ 3 & 6 & 4 & 2 & 0 & 0 \end{pmatrix}$$

**3 generation subalgebra** 107
Algebra: $\mathfrak{su}(5) \oplus \mathfrak{su}(2) \oplus \mathfrak{su}(2)$
$(\overline{\mathbf{5}}, \mathbf{1}, \mathbf{1})$, $(0,0,0,1,0,0) \mapsto (D, L)$
$(\mathbf{10}, \mathbf{1}, \mathbf{1})$, $(0,1,0,0,0,0) \mapsto (E, Q, U)$
$(\overline{\mathbf{5}}, \mathbf{2}, \mathbf{1})$, $(0,0,0,1,1,0) \mapsto (D, D, L, L)$
$(\mathbf{10}, \mathbf{1}, \mathbf{2})$, $(0,1,0,0,0,1) \mapsto (E, E, Q, Q, U, U)$
$(\mathbf{1}, \mathbf{1}, \mathbf{3})$, $(0,0,0,0,0,2) \mapsto (N, N, N)$
Projection matrix for $\alpha$:

$$\begin{pmatrix} 0 & 0 & 1 & 0 & 0 & 0 \\ 0 & 0 & 0 & 1 & 0 & 0 \\ 1 & 0 & 0 & 0 & 0 & 0 \\ 3 & 6 & 4 & 2 & 0 & 0 \end{pmatrix}$$

**3 generation subalgebra** 108
Algebra: $\mathfrak{su}(5) \oplus \mathfrak{su}(2) \oplus \mathfrak{su}(2)$

$(\overline{\mathbf{5}}, \mathbf{1}, \mathbf{1})$, $(0,0,0,1,0,0) \mapsto (D, L)$
$(\mathbf{10}, \mathbf{1}, \mathbf{1})$, $(0,1,0,0,0,0) \mapsto (E, Q, U)$
$(\overline{\mathbf{5}}, \mathbf{2}, \mathbf{1})$, $(0,0,0,1,1,0) \mapsto (D, D, L, L)$
$(\mathbf{10}, \mathbf{1}, \mathbf{2})$, $(0,1,0,0,0,1) \mapsto (E, E, Q, Q, U, U)$
$(\mathbf{1}, \mathbf{2}, \mathbf{1})$, $(0,0,0,0,1,0) \mapsto (N, N)$
$(\mathbf{1}, \mathbf{1}, \mathbf{1})$, $(0,0,0,0,0,0) \mapsto (N)$
Projection matrix for $\alpha$:

$$\begin{pmatrix} 0 & 0 & 1 & 0 & 0 & 0 \\ 0 & 0 & 0 & 1 & 0 & 0 \\ 1 & 0 & 0 & 0 & 0 & 0 \\ 3 & 6 & 4 & 2 & 0 & 0 \end{pmatrix}$$

**3 generation subalgebra** 109
Algebra: $\mathfrak{su}(5) \oplus \mathfrak{su}(2) \oplus \mathfrak{su}(2)$
$(\overline{\mathbf{5}}, \mathbf{1}, \mathbf{1})$, $(0,0,0,1,0,0) \mapsto (D, L)$
$(\mathbf{10}, \mathbf{1}, \mathbf{1})$, $(0,1,0,0,0,0) \mapsto (E, Q, U)$
$(\overline{\mathbf{5}}, \mathbf{2}, \mathbf{1})$, $(0,0,0,1,1,0) \mapsto (D, D, L, L)$
$(\mathbf{10}, \mathbf{1}, \mathbf{2})$, $(0,1,0,0,0,1) \mapsto (E, E, Q, Q, U, U)$
$(\mathbf{1}, \mathbf{3}, \mathbf{1})$, $(0,0,0,0,2,0) \mapsto (N, N, N)$
Projection matrix for $\alpha$:

$$\begin{pmatrix} 0 & 0 & 1 & 0 & 0 & 0 \\ 0 & 0 & 0 & 1 & 0 & 0 \\ 1 & 0 & 0 & 0 & 0 & 0 \\ 3 & 6 & 4 & 2 & 0 & 0 \end{pmatrix}$$

**3 generation subalgebra** 110
Algebra: $\mathfrak{su}(5) \oplus \mathfrak{su}(2) \oplus \mathfrak{su}(2)$
$(\overline{\mathbf{5}}, \mathbf{1}, \mathbf{1})$, $(0,0,0,1,0,0) \mapsto (D, L)$
$(\mathbf{10}, \mathbf{1}, \mathbf{1})$, $(0,1,0,0,0,0) \mapsto (E, Q, U)$
$(\overline{\mathbf{5}}, \mathbf{2}, \mathbf{1})$, $(0,0,0,1,1,0) \mapsto (D, D, L, L)$
$(\mathbf{10}, \mathbf{2}, \mathbf{1})$, $(0,1,0,0,1,0) \mapsto (E, E, Q, Q, U, U)$
$(\mathbf{1}, \mathbf{1}, \mathbf{2})$, $(0,0,0,0,0,1) \mapsto (N, N)$
$(\mathbf{1}, \mathbf{1}, \mathbf{1})$, $(0,0,0,0,0,0) \mapsto (N)$
Projection matrix for $\alpha$:

$$\begin{pmatrix} 0 & 0 & 1 & 0 & 0 & 0 \\ 0 & 0 & 0 & 1 & 0 & 0 \\ 1 & 0 & 0 & 0 & 0 & 0 \\ 3 & 6 & 4 & 2 & 0 & 0 \end{pmatrix}$$

**3 generation subalgebra** 111
Algebra: $\mathfrak{su}(5) \oplus \mathfrak{su}(2) \oplus \mathfrak{su}(2)$
$(\overline{\mathbf{5}}, \mathbf{1}, \mathbf{1})$, $(0,0,0,1,0,0) \mapsto (D, L)$
$(\mathbf{10}, \mathbf{1}, \mathbf{1})$, $(0,1,0,0,0,0) \mapsto (E, Q, U)$
$(\overline{\mathbf{5}}, \mathbf{2}, \mathbf{1})$, $(0,0,0,1,1,0) \mapsto (D, D, L, L)$
$(\mathbf{10}, \mathbf{2}, \mathbf{1})$, $(0,1,0,0,1,0) \mapsto (E, E, Q, Q, U, U)$
$(\mathbf{1}, \mathbf{1}, \mathbf{3})$, $(0,0,0,0,0,2) \mapsto (N, N, N)$
Projection matrix for $\alpha$:

$$\begin{pmatrix} 0 & 0 & 1 & 0 & 0 & 0 \\ 0 & 0 & 0 & 1 & 0 & 0 \\ 1 & 0 & 0 & 0 & 0 & 0 \\ 3 & 6 & 4 & 2 & 0 & 0 \end{pmatrix}$$

**3 generation subalgebra** 112
Algebra: $\mathfrak{su}(5) \oplus \mathfrak{su}(2) \oplus \mathfrak{su}(2)$
$(\mathbf{10}, \mathbf{1}, \mathbf{1})$, $(0,1,0,0,0,0) \mapsto (E, Q, U)$
$(\mathbf{10}, \mathbf{1}, \mathbf{1})$, $(0,1,0,0,0,0) \mapsto (E, Q, U)$

$(\mathbf{10}, \mathbf{1}, \mathbf{1}),\ (0,1,0,0,0,0) \mapsto (E, Q, U)$
$(\overline{\mathbf{5}}, \mathbf{3}, \mathbf{1}),\ (0,0,0,1,2,0) \mapsto (D, D, D, L, L, L)$
$(\mathbf{1}, \mathbf{1}, \mathbf{2}),\ (0,0,0,0,0,1) \mapsto (N, N)$
$(\mathbf{1}, \mathbf{1}, \mathbf{1}),\ (0,0,0,0,0,0) \mapsto (N)$
Projection matrix for $\alpha$:

$$\begin{pmatrix} 0 & 0 & 1 & 0 & 0 & 0 \\ 0 & 0 & 0 & 1 & 0 & 0 \\ 1 & 0 & 0 & 0 & 0 & 0 \\ 3 & 6 & 4 & 2 & 0 & 0 \end{pmatrix}$$

**3 generation subalgebra** 113
Algebra: $\mathfrak{su}(5) \oplus \mathfrak{su}(2) \oplus \mathfrak{su}(2)$
$(\mathbf{10}, \mathbf{1}, \mathbf{1}),\ (0,1,0,0,0,0) \mapsto (E, Q, U)$
$(\mathbf{10}, \mathbf{1}, \mathbf{1}),\ (0,1,0,0,0,0) \mapsto (E, Q, U)$
$(\mathbf{10}, \mathbf{1}, \mathbf{1}),\ (0,1,0,0,0,0) \mapsto (E, Q, U)$
$(\overline{\mathbf{5}}, \mathbf{3}, \mathbf{1}),\ (0,0,0,1,2,0) \mapsto (D, D, D, L, L, L)$
$(\mathbf{1}, \mathbf{1}, \mathbf{3}),\ (0,0,0,0,0,2) \mapsto (N, N, N)$
Projection matrix for $\alpha$:

$$\begin{pmatrix} 0 & 0 & 1 & 0 & 0 & 0 \\ 0 & 0 & 0 & 1 & 0 & 0 \\ 1 & 0 & 0 & 0 & 0 & 0 \\ 3 & 6 & 4 & 2 & 0 & 0 \end{pmatrix}$$

**3 generation subalgebra** 114
Algebra: $\mathfrak{su}(5) \oplus \mathfrak{su}(2) \oplus \mathfrak{su}(2)$
$(\overline{\mathbf{5}}, \mathbf{1}, \mathbf{1}),\ (0,0,0,1,0,0) \mapsto (D, L)$
$(\overline{\mathbf{5}}, \mathbf{1}, \mathbf{1}),\ (0,0,0,1,0,0) \mapsto (D, L)$
$(\overline{\mathbf{5}}, \mathbf{1}, \mathbf{1}),\ (0,0,0,1,0,0) \mapsto (D, L)$
$(\mathbf{10}, \mathbf{1}, \mathbf{1}),\ (0,1,0,0,0,0) \mapsto (E, Q, U)$
$(\mathbf{10}, \mathbf{2}, \mathbf{1}),\ (0,1,0,0,1,0) \mapsto (E, E, Q, Q, U, U)$
$(\mathbf{1}, \mathbf{1}, \mathbf{2}),\ (0,0,0,0,0,1) \mapsto (N, N)$
$(\mathbf{1}, \mathbf{1}, \mathbf{1}),\ (0,0,0,0,0,0) \mapsto (N)$
Projection matrix for $\alpha$:

$$\begin{pmatrix} 0 & 0 & 1 & 0 & 0 & 0 \\ 0 & 0 & 0 & 1 & 0 & 0 \\ 1 & 0 & 0 & 0 & 0 & 0 \\ 3 & 6 & 4 & 2 & 0 & 0 \end{pmatrix}$$

**3 generation subalgebra** 115
Algebra: $\mathfrak{su}(5) \oplus \mathfrak{su}(2) \oplus \mathfrak{su}(2)$
$(\overline{\mathbf{5}}, \mathbf{1}, \mathbf{1}),\ (0,0,0,1,0,0) \mapsto (D, L)$
$(\overline{\mathbf{5}}, \mathbf{1}, \mathbf{1}),\ (0,0,0,1,0,0) \mapsto (D, L)$
$(\overline{\mathbf{5}}, \mathbf{1}, \mathbf{1}),\ (0,0,0,1,0,0) \mapsto (D, L)$
$(\mathbf{10}, \mathbf{1}, \mathbf{1}),\ (0,1,0,0,0,0) \mapsto (E, Q, U)$
$(\mathbf{10}, \mathbf{2}, \mathbf{1}),\ (0,1,0,0,1,0) \mapsto (E, E, Q, Q, U, U)$
$(\mathbf{1}, \mathbf{1}, \mathbf{3}),\ (0,0,0,0,0,2) \mapsto (N, N, N)$
Projection matrix for $\alpha$:

$$\begin{pmatrix} 0 & 0 & 1 & 0 & 0 & 0 \\ 0 & 0 & 0 & 1 & 0 & 0 \\ 1 & 0 & 0 & 0 & 0 & 0 \\ 3 & 6 & 4 & 2 & 0 & 0 \end{pmatrix}$$

**3 generation subalgebra** 116
Algebra: $\mathfrak{su}(5) \oplus \mathfrak{su}(2) \oplus \mathfrak{su}(2)$
$(\overline{\mathbf{5}}, \mathbf{1}, \mathbf{1}),\ (0,0,0,1,0,0) \mapsto (D, L)$
$(\mathbf{10}, \mathbf{1}, \mathbf{1}),\ (0,1,0,0,0,0) \mapsto (E, Q, U)$

$(\mathbf{10},\mathbf{1},\mathbf{1})$, $(0,1,0,0,0,0) \mapsto (E,Q,U)$
$(\mathbf{10},\mathbf{1},\mathbf{1})$, $(0,1,0,0,0,0) \mapsto (E,Q,U)$
$(\overline{\mathbf{5}},\mathbf{2},\mathbf{1})$, $(0,0,0,1,1,0) \mapsto (D,D,L,L)$
$(\mathbf{1},\mathbf{1},\mathbf{2})$, $(0,0,0,0,0,1) \mapsto (N,N)$
$(\mathbf{1},\mathbf{1},\mathbf{1})$, $(0,0,0,0,0,0) \mapsto (N)$
Projection matrix for $\alpha$:

$$\begin{pmatrix} 0 & 0 & 1 & 0 & 0 & 0 \\ 0 & 0 & 0 & 1 & 0 & 0 \\ 1 & 0 & 0 & 0 & 0 & 0 \\ 3 & 6 & 4 & 2 & 0 & 0 \end{pmatrix}$$

**3 generation subalgebra** 117
Algebra: $\mathfrak{su}(5) \oplus \mathfrak{su}(2) \oplus \mathfrak{su}(2)$
$(\overline{\mathbf{5}},\mathbf{1},\mathbf{1})$, $(0,0,0,1,0,0) \mapsto (D,L)$
$(\mathbf{10},\mathbf{1},\mathbf{1})$, $(0,1,0,0,0,0) \mapsto (E,Q,U)$
$(\mathbf{10},\mathbf{1},\mathbf{1})$, $(0,1,0,0,0,0) \mapsto (E,Q,U)$
$(\mathbf{10},\mathbf{1},\mathbf{1})$, $(0,1,0,0,0,0) \mapsto (E,Q,U)$
$(\overline{\mathbf{5}},\mathbf{2},\mathbf{1})$, $(0,0,0,1,1,0) \mapsto (D,D,L,L)$
$(\mathbf{1},\mathbf{1},\mathbf{3})$, $(0,0,0,0,0,2) \mapsto (N,N,N)$
Projection matrix for $\alpha$:

$$\begin{pmatrix} 0 & 0 & 1 & 0 & 0 & 0 \\ 0 & 0 & 0 & 1 & 0 & 0 \\ 1 & 0 & 0 & 0 & 0 & 0 \\ 3 & 6 & 4 & 2 & 0 & 0 \end{pmatrix}$$

**3 generation subalgebra** 118
Algebra: $\mathfrak{su}(5) \oplus \mathfrak{su}(5) \oplus \mathfrak{so}(10)$
$(\overline{\mathbf{5}},\mathbf{1},\mathbf{1})$, $(0,0,0,1,0,0,0,0,0,0,0,0,0) \mapsto (D,L)$
$(\mathbf{10},\mathbf{1},\mathbf{1})$, $(0,1,0,0,0,0,0,0,0,0,0,0,0) \mapsto (E,Q,U)$
$(\mathbf{1},\overline{\mathbf{5}},\mathbf{1})$, $(0,0,0,0,0,0,0,1,0,0,0,0,0) \mapsto (D,L)$
$(\mathbf{1},\mathbf{10},\mathbf{1})$, $(0,0,0,0,0,1,0,0,0,0,0,0,0) \mapsto (E,Q,U)$
$(\mathbf{1},\mathbf{1},\mathbf{16})$, $(0,0,0,0,0,0,0,0,0,0,0,0,1) \mapsto (D,E,L,N,Q,U)$
$(\mathbf{1},\mathbf{1},\mathbf{1})$, $(0,0,0,0,0,0,0,0,0,0,0,0,0) \mapsto (N)$
$(\mathbf{1},\mathbf{1},\mathbf{1})$, $(0,0,0,0,0,0,0,0,0,0,0,0,0) \mapsto (N)$
Projection matrix for $\alpha$:

$$\begin{pmatrix} 0 & 0 & 1 & 0 & 0 & 0 & 1 & 0 & 0 & 0 & 1 & 0 & 0 \\ 0 & 0 & 0 & 1 & 0 & 0 & 0 & 1 & 0 & 0 & 0 & 0 & 1 \\ 1 & 0 & 0 & 0 & 1 & 0 & 0 & 0 & 1 & 0 & 0 & 0 & 0 \\ 3 & 6 & 4 & 2 & 3 & 6 & 4 & 2 & 3 & 6 & 4 & 0 & 2 \end{pmatrix}$$

**3 generation subalgebra** 119
Algebra: $\mathfrak{su}(5) \oplus \mathfrak{su}(5) \oplus \mathfrak{su}(2)$
$(\mathbf{1},\overline{\mathbf{5}},\mathbf{1})$, $(0,0,0,0,0,0,0,1,0) \mapsto (D,L)$
$(\mathbf{1},\mathbf{10},\mathbf{1})$, $(0,0,0,0,0,1,0,0,0) \mapsto (E,Q,U)$
$(\overline{\mathbf{5}},\mathbf{1},\mathbf{2})$, $(0,0,0,1,0,0,0,0,1) \mapsto (D,D,L,L)$
$(\mathbf{10},\mathbf{1},\mathbf{2})$, $(0,1,0,0,0,0,0,0,1) \mapsto (E,E,Q,Q,U,U)$
$(\mathbf{1},\mathbf{1},\mathbf{1})$, $(0,0,0,0,0,0,0,0,0) \mapsto (N)$
$(\mathbf{1},\mathbf{1},\mathbf{1})$, $(0,0,0,0,0,0,0,0,0) \mapsto (N)$
$(\mathbf{1},\mathbf{1},\mathbf{1})$, $(0,0,0,0,0,0,0,0,0) \mapsto (N)$
Projection matrix for $\alpha$:

$$\begin{pmatrix} 0 & 0 & 1 & 0 & 0 & 0 & 1 & 0 & 0 \\ 0 & 0 & 0 & 1 & 0 & 0 & 0 & 1 & 0 \\ 1 & 0 & 0 & 0 & 1 & 0 & 0 & 0 & 0 \\ 3 & 6 & 4 & 2 & 3 & 6 & 4 & 2 & 0 \end{pmatrix}$$

**3 generation subalgebra** 120
Algebra: $\mathfrak{su}(5) \oplus \mathfrak{su}(5) \oplus \mathfrak{su}(2)$

$(\mathbf{1},\overline{\mathbf{5}},\mathbf{1}),\ (0,0,0,0,0,0,0,1,0)\mapsto(D,L)$
$(\mathbf{1},\mathbf{10},\mathbf{1}),\ (0,0,0,0,0,1,0,0,0)\mapsto(E,Q,U)$
$(\overline{\mathbf{5}},\mathbf{1},\mathbf{2}),\ (0,0,0,1,0,0,0,0,1)\mapsto(D,D,L,L)$
$(\mathbf{10},\mathbf{1},\mathbf{2}),\ (0,1,0,0,0,0,0,0,1)\mapsto(E,E,Q,Q,U,U)$
$(\mathbf{1},\mathbf{1},\mathbf{2}),\ (0,0,0,0,0,0,0,0,1)\mapsto(N,N)$
$(\mathbf{1},\mathbf{1},\mathbf{1}),\ (0,0,0,0,0,0,0,0,0)\mapsto(N)$
Projection matrix for $\alpha$:

$$\begin{pmatrix}0&0&1&0&0&0&1&0&0\\0&0&0&1&0&0&0&1&0\\1&0&0&0&1&0&0&0&0\\3&6&4&2&3&6&4&2&0\end{pmatrix}$$

**3 generation subalgebra** 121
Algebra: $\mathfrak{su}(5)\oplus\mathfrak{su}(5)\oplus\mathfrak{su}(2)$
$(\mathbf{1},\overline{\mathbf{5}},\mathbf{1}),\ (0,0,0,0,0,0,0,1,0)\mapsto(D,L)$
$(\mathbf{1},\mathbf{10},\mathbf{1}),\ (0,0,0,0,0,1,0,0,0)\mapsto(E,Q,U)$
$(\overline{\mathbf{5}},\mathbf{1},\mathbf{2}),\ (0,0,0,1,0,0,0,0,1)\mapsto(D,D,L,L)$
$(\mathbf{10},\mathbf{1},\mathbf{2}),\ (0,1,0,0,0,0,0,0,1)\mapsto(E,E,Q,Q,U,U)$
$(\mathbf{1},\mathbf{1},\mathbf{3}),\ (0,0,0,0,0,0,0,0,2)\mapsto(N,N,N)$
Projection matrix for $\alpha$:

$$\begin{pmatrix}0&0&1&0&0&0&1&0&0\\0&0&0&1&0&0&0&1&0\\1&0&0&0&1&0&0&0&0\\3&6&4&2&3&6&4&2&0\end{pmatrix}$$

**3 generation subalgebra** 122
Algebra: $\mathfrak{su}(5)\oplus\mathfrak{su}(5)\oplus\mathfrak{su}(2)$
$(\overline{\mathbf{5}},\mathbf{1},\mathbf{1}),\ (0,0,0,1,0,0,0,0,0)\mapsto(D,L)$
$(\overline{\mathbf{5}},\mathbf{1},\mathbf{1}),\ (0,0,0,1,0,0,0,0,0)\mapsto(D,L)$
$(\mathbf{1},\overline{\mathbf{5}},\mathbf{1}),\ (0,0,0,0,0,0,0,1,0)\mapsto(D,L)$
$(\mathbf{1},\mathbf{10},\mathbf{1}),\ (0,0,0,0,0,1,0,0,0)\mapsto(E,Q,U)$
$(\mathbf{10},\mathbf{1},\mathbf{2}),\ (0,1,0,0,0,0,0,0,1)\mapsto(E,E,Q,Q,U,U)$
$(\mathbf{1},\mathbf{1},\mathbf{1}),\ (0,0,0,0,0,0,0,0,0)\mapsto(N)$
$(\mathbf{1},\mathbf{1},\mathbf{1}),\ (0,0,0,0,0,0,0,0,0)\mapsto(N)$
$(\mathbf{1},\mathbf{1},\mathbf{1}),\ (0,0,0,0,0,0,0,0,0)\mapsto(N)$
Projection matrix for $\alpha$:

$$\begin{pmatrix}0&0&1&0&0&0&1&0&0\\0&0&0&1&0&0&0&1&0\\1&0&0&0&1&0&0&0&0\\3&6&4&2&3&6&4&2&0\end{pmatrix}$$

**3 generation subalgebra** 123
Algebra: $\mathfrak{su}(5)\oplus\mathfrak{su}(5)\oplus\mathfrak{su}(2)$
$(\mathbf{10},\mathbf{1},\mathbf{1}),\ (0,1,0,0,0,0,0,0,0)\mapsto(E,Q,U)$
$(\mathbf{10},\mathbf{1},\mathbf{1}),\ (0,1,0,0,0,0,0,0,0)\mapsto(E,Q,U)$
$(\mathbf{1},\overline{\mathbf{5}},\mathbf{1}),\ (0,0,0,0,0,0,0,1,0)\mapsto(D,L)$
$(\mathbf{1},\mathbf{10},\mathbf{1}),\ (0,0,0,0,0,1,0,0,0)\mapsto(E,Q,U)$
$(\overline{\mathbf{5}},\mathbf{1},\mathbf{2}),\ (0,0,0,1,0,0,0,0,1)\mapsto(D,D,L,L)$
$(\mathbf{1},\mathbf{1},\mathbf{1}),\ (0,0,0,0,0,0,0,0,0)\mapsto(N)$
$(\mathbf{1},\mathbf{1},\mathbf{1}),\ (0,0,0,0,0,0,0,0,0)\mapsto(N)$
$(\mathbf{1},\mathbf{1},\mathbf{1}),\ (0,0,0,0,0,0,0,0,0)\mapsto(N)$
Projection matrix for $\alpha$:

$$\begin{pmatrix}0&0&1&0&0&0&1&0&0\\0&0&0&1&0&0&0&1&0\\1&0&0&0&1&0&0&0&0\\3&6&4&2&3&6&4&2&0\end{pmatrix}$$

**3 generation subalgebra** 124
Algebra: $\mathfrak{su}(5) \oplus \mathfrak{su}(5) \oplus \mathfrak{su}(2)$
$(\overline{\mathbf{5}}, \mathbf{1}, \mathbf{1})$, $(0,0,0,1,0,0,0,0,0) \mapsto (D, L)$
$(\overline{\mathbf{5}}, \mathbf{1}, \mathbf{1})$, $(0,0,0,1,0,0,0,0,0) \mapsto (D, L)$
$(\mathbf{1}, \overline{\mathbf{5}}, \mathbf{1})$, $(0,0,0,0,0,0,0,1,0) \mapsto (D, L)$
$(\mathbf{1}, \mathbf{10}, \mathbf{1})$, $(0,0,0,0,0,1,0,0,0) \mapsto (E, Q, U)$
$(\mathbf{10}, \mathbf{1}, \mathbf{2})$, $(0,1,0,0,0,0,0,0,1) \mapsto (E, E, Q, Q, U, U)$
$(\mathbf{1}, \mathbf{1}, \mathbf{2})$, $(0,0,0,0,0,0,0,0,1) \mapsto (N, N)$
$(\mathbf{1}, \mathbf{1}, \mathbf{1})$, $(0,0,0,0,0,0,0,0,0) \mapsto (N)$
Projection matrix for $\alpha$:

$$\begin{pmatrix} 0 & 0 & 1 & 0 & 0 & 0 & 1 & 0 & 0 \\ 0 & 0 & 0 & 1 & 0 & 0 & 0 & 1 & 0 \\ 1 & 0 & 0 & 0 & 1 & 0 & 0 & 0 & 0 \\ 3 & 6 & 4 & 2 & 3 & 6 & 4 & 2 & 0 \end{pmatrix}$$

**3 generation subalgebra** 125
Algebra: $\mathfrak{su}(5) \oplus \mathfrak{su}(5) \oplus \mathfrak{su}(2)$
$(\overline{\mathbf{5}}, \mathbf{1}, \mathbf{1})$, $(0,0,0,1,0,0,0,0,0) \mapsto (D, L)$
$(\overline{\mathbf{5}}, \mathbf{1}, \mathbf{1})$, $(0,0,0,1,0,0,0,0,0) \mapsto (D, L)$
$(\mathbf{1}, \overline{\mathbf{5}}, \mathbf{1})$, $(0,0,0,0,0,0,0,1,0) \mapsto (D, L)$
$(\mathbf{1}, \mathbf{10}, \mathbf{1})$, $(0,0,0,0,0,1,0,0,0) \mapsto (E, Q, U)$
$(\mathbf{10}, \mathbf{1}, \mathbf{2})$, $(0,1,0,0,0,0,0,0,1) \mapsto (E, E, Q, Q, U, U)$
$(\mathbf{1}, \mathbf{1}, \mathbf{3})$, $(0,0,0,0,0,0,0,0,2) \mapsto (N, N, N)$
Projection matrix for $\alpha$:

$$\begin{pmatrix} 0 & 0 & 1 & 0 & 0 & 0 & 1 & 0 & 0 \\ 0 & 0 & 0 & 1 & 0 & 0 & 0 & 1 & 0 \\ 1 & 0 & 0 & 0 & 1 & 0 & 0 & 0 & 0 \\ 3 & 6 & 4 & 2 & 3 & 6 & 4 & 2 & 0 \end{pmatrix}$$

**3 generation subalgebra** 126
Algebra: $\mathfrak{su}(5) \oplus \mathfrak{su}(5) \oplus \mathfrak{su}(2)$
$(\mathbf{10}, \mathbf{1}, \mathbf{1})$, $(0,1,0,0,0,0,0,0,0) \mapsto (E, Q, U)$
$(\mathbf{10}, \mathbf{1}, \mathbf{1})$, $(0,1,0,0,0,0,0,0,0) \mapsto (E, Q, U)$
$(\mathbf{1}, \overline{\mathbf{5}}, \mathbf{1})$, $(0,0,0,0,0,0,0,1,0) \mapsto (D, L)$
$(\mathbf{1}, \mathbf{10}, \mathbf{1})$, $(0,0,0,0,0,1,0,0,0) \mapsto (E, Q, U)$
$(\overline{\mathbf{5}}, \mathbf{1}, \mathbf{2})$, $(0,0,0,1,0,0,0,0,1) \mapsto (D, D, L, L)$
$(\mathbf{1}, \mathbf{1}, \mathbf{2})$, $(0,0,0,0,0,0,0,0,1) \mapsto (N, N)$
$(\mathbf{1}, \mathbf{1}, \mathbf{1})$, $(0,0,0,0,0,0,0,0,0) \mapsto (N)$
Projection matrix for $\alpha$:

$$\begin{pmatrix} 0 & 0 & 1 & 0 & 0 & 0 & 1 & 0 & 0 \\ 0 & 0 & 0 & 1 & 0 & 0 & 0 & 1 & 0 \\ 1 & 0 & 0 & 0 & 1 & 0 & 0 & 0 & 0 \\ 3 & 6 & 4 & 2 & 3 & 6 & 4 & 2 & 0 \end{pmatrix}$$

**3 generation subalgebra** 127
Algebra: $\mathfrak{su}(5) \oplus \mathfrak{su}(5) \oplus \mathfrak{su}(2)$
$(\mathbf{10}, \mathbf{1}, \mathbf{1})$, $(0,1,0,0,0,0,0,0,0) \mapsto (E, Q, U)$
$(\mathbf{10}, \mathbf{1}, \mathbf{1})$, $(0,1,0,0,0,0,0,0,0) \mapsto (E, Q, U)$
$(\mathbf{1}, \overline{\mathbf{5}}, \mathbf{1})$, $(0,0,0,0,0,0,0,1,0) \mapsto (D, L)$
$(\mathbf{1}, \mathbf{10}, \mathbf{1})$, $(0,0,0,0,0,1,0,0,0) \mapsto (E, Q, U)$
$(\overline{\mathbf{5}}, \mathbf{1}, \mathbf{2})$, $(0,0,0,1,0,0,0,0,1) \mapsto (D, D, L, L)$
$(\mathbf{1}, \mathbf{1}, \mathbf{3})$, $(0,0,0,0,0,0,0,0,2) \mapsto (N, N, N)$
Projection matrix for $\alpha$:

$$\begin{pmatrix} 0 & 0 & 1 & 0 & 0 & 0 & 1 & 0 & 0 \\ 0 & 0 & 0 & 1 & 0 & 0 & 0 & 1 & 0 \\ 1 & 0 & 0 & 0 & 1 & 0 & 0 & 0 & 0 \\ 3 & 6 & 4 & 2 & 3 & 6 & 4 & 2 & 0 \end{pmatrix}$$

**3 generation subalgebra** 128
Algebra: $\mathfrak{su}(5) \oplus \mathfrak{su}(5) \oplus \mathfrak{su}(2)$
$(\bar{\mathbf{5}}, \mathbf{1}, \mathbf{1})$, $(0,0,0,1,0,0,0,0,0) \mapsto (D, L)$
$(\bar{\mathbf{5}}, \mathbf{1}, \mathbf{1})$, $(0,0,0,1,0,0,0,0,0) \mapsto (D, L)$
$(\mathbf{10}, \mathbf{1}, \mathbf{1})$, $(0,1,0,0,0,0,0,0,0) \mapsto (E, Q, U)$
$(\mathbf{10}, \mathbf{1}, \mathbf{1})$, $(0,1,0,0,0,0,0,0,0) \mapsto (E, Q, U)$
$(\mathbf{1}, \bar{\mathbf{5}}, \mathbf{1})$, $(0,0,0,0,0,0,0,1,0) \mapsto (D, L)$
$(\mathbf{1}, \mathbf{10}, \mathbf{1})$, $(0,0,0,0,0,1,0,0,0) \mapsto (E, Q, U)$
$(\mathbf{1}, \mathbf{1}, \mathbf{2})$, $(0,0,0,0,0,0,0,0,1) \mapsto (N, N)$
$(\mathbf{1}, \mathbf{1}, \mathbf{1})$, $(0,0,0,0,0,0,0,0,0) \mapsto (N)$
Projection matrix for $\alpha$:

$$\begin{pmatrix} 0 & 0 & 1 & 0 & 0 & 0 & 1 & 0 & 0 \\ 0 & 0 & 0 & 1 & 0 & 0 & 0 & 1 & 0 \\ 1 & 0 & 0 & 0 & 1 & 0 & 0 & 0 & 0 \\ 3 & 6 & 4 & 2 & 3 & 6 & 4 & 2 & 0 \end{pmatrix}$$

**3 generation subalgebra** 129
Algebra: $\mathfrak{su}(5) \oplus \mathfrak{su}(5) \oplus \mathfrak{su}(2)$
$(\bar{\mathbf{5}}, \mathbf{1}, \mathbf{1})$, $(0,0,0,1,0,0,0,0,0) \mapsto (D, L)$
$(\bar{\mathbf{5}}, \mathbf{1}, \mathbf{1})$, $(0,0,0,1,0,0,0,0,0) \mapsto (D, L)$
$(\mathbf{10}, \mathbf{1}, \mathbf{1})$, $(0,1,0,0,0,0,0,0,0) \mapsto (E, Q, U)$
$(\mathbf{10}, \mathbf{1}, \mathbf{1})$, $(0,1,0,0,0,0,0,0,0) \mapsto (E, Q, U)$
$(\mathbf{1}, \bar{\mathbf{5}}, \mathbf{1})$, $(0,0,0,0,0,0,0,1,0) \mapsto (D, L)$
$(\mathbf{1}, \mathbf{10}, \mathbf{1})$, $(0,0,0,0,0,1,0,0,0) \mapsto (E, Q, U)$
$(\mathbf{1}, \mathbf{1}, \mathbf{3})$, $(0,0,0,0,0,0,0,0,2) \mapsto (N, N, N)$
Projection matrix for $\alpha$:

$$\begin{pmatrix} 0 & 0 & 1 & 0 & 0 & 0 & 1 & 0 & 0 \\ 0 & 0 & 0 & 1 & 0 & 0 & 0 & 1 & 0 \\ 1 & 0 & 0 & 0 & 1 & 0 & 0 & 0 & 0 \\ 3 & 6 & 4 & 2 & 3 & 6 & 4 & 2 & 0 \end{pmatrix}$$

**3 generation subalgebra** 130
Algebra: $\mathfrak{su}(5) \oplus \mathfrak{su}(5) \oplus \mathfrak{su}(5)$
$(\bar{\mathbf{5}}, \mathbf{1}, \mathbf{1})$, $(0,0,0,1,0,0,0,0,0,0,0,0) \mapsto (D, L)$
$(\mathbf{10}, \mathbf{1}, \mathbf{1})$, $(0,1,0,0,0,0,0,0,0,0,0,0) \mapsto (E, Q, U)$
$(\mathbf{1}, \bar{\mathbf{5}}, \mathbf{1})$, $(0,0,0,0,0,0,0,1,0,0,0,0) \mapsto (D, L)$
$(\mathbf{1}, \mathbf{10}, \mathbf{1})$, $(0,0,0,0,0,1,0,0,0,0,0,0) \mapsto (E, Q, U)$
$(\mathbf{1}, \mathbf{1}, \bar{\mathbf{5}})$, $(0,0,0,0,0,0,0,0,0,0,0,1) \mapsto (D, L)$
$(\mathbf{1}, \mathbf{1}, \mathbf{10})$, $(0,0,0,0,0,0,0,0,0,1,0,0) \mapsto (E, Q, U)$
$(\mathbf{1}, \mathbf{1}, \mathbf{1})$, $(0,0,0,0,0,0,0,0,0,0,0,0) \mapsto (N)$
$(\mathbf{1}, \mathbf{1}, \mathbf{1})$, $(0,0,0,0,0,0,0,0,0,0,0,0) \mapsto (N)$
$(\mathbf{1}, \mathbf{1}, \mathbf{1})$, $(0,0,0,0,0,0,0,0,0,0,0,0) \mapsto (N)$
Projection matrix for $\alpha$:

$$\begin{pmatrix} 0 & 0 & 1 & 0 & 0 & 0 & 1 & 0 & 0 & 0 & 1 & 0 \\ 0 & 0 & 0 & 1 & 0 & 0 & 0 & 1 & 0 & 0 & 0 & 1 \\ 1 & 0 & 0 & 0 & 1 & 0 & 0 & 0 & 1 & 0 & 0 & 0 \\ 3 & 6 & 4 & 2 & 3 & 6 & 4 & 2 & 3 & 6 & 4 & 2 \end{pmatrix}$$

**3 generation subalgebra** 131
Algebra: $\mathfrak{su}(3) \oplus \mathfrak{su}(4) \oplus \mathfrak{su}(2) \oplus \mathfrak{su}(2)$
$(\bar{\mathbf{3}}, \bar{\mathbf{4}}, \mathbf{2}, \mathbf{1})$, $(0,1,0,0,1,1,0) \mapsto (L, L, L, Q, Q, Q)$
$(\mathbf{3}, \mathbf{4}, \mathbf{1}, \mathbf{2})$, $(1,0,1,0,0,0,1) \mapsto (D, D, D, E, E, E, N, N, N, U, U, U)$
Projection matrix for $\alpha$:

$$\begin{pmatrix} 0 & 0 & 0 & 1 & 0 & 0 & 0 \\ 0 & 0 & 1 & 0 & 0 & 0 & 0 \\ 0 & 0 & 0 & 0 & 0 & 1 & 0 \\ 0 & 0 & -1 & -2 & -3 & 0 & 3 \end{pmatrix}$$

**3 generation subalgebra** 132
Algebra: $\mathfrak{su}(4) \oplus \mathfrak{so}(10) \oplus \mathfrak{su}(2) \oplus \mathfrak{su}(2)$
$(\mathbf{1}, \mathbf{16}, \mathbf{1}, \mathbf{1})$, $(0,0,0,0,0,0,0,1,0,0) \mapsto (D,E,L,N,Q,U)$
$(\mathbf{1}, \mathbf{16}, \mathbf{1}, \mathbf{1})$, $(0,0,0,0,0,0,0,1,0,0) \mapsto (D,E,L,N,Q,U)$
$(\overline{\mathbf{4}}, \mathbf{1}, \mathbf{2}, \mathbf{1})$, $(0,0,1,0,0,0,0,0,1,0) \mapsto (L,Q)$
$(\mathbf{4}, \mathbf{1}, \mathbf{1}, \mathbf{2})$, $(1,0,0,0,0,0,0,0,0,1) \mapsto (D,E,N,U)$
Projection matrix for $\alpha$:

$$\begin{pmatrix} 0 & 1 & 0 & 0 & 0 & 1 & 0 & 0 & 0 & 0 \\ 1 & 0 & 0 & 0 & 0 & 0 & 0 & 1 & 0 & 0 \\ 0 & 0 & 0 & 1 & 0 & 0 & 0 & 0 & 1 & 0 \\ -1 & -2 & -3 & 3 & 6 & 4 & 0 & 2 & 0 & 3 \end{pmatrix}$$

**3 generation subalgebra** 133
Algebra: $\mathfrak{su}(4) \oplus \mathfrak{so}(10) \oplus \mathfrak{su}(2) \oplus \mathfrak{su}(2)$
$(\mathbf{1}, \mathbf{16}, \mathbf{1}, \mathbf{1})$, $(0,0,0,0,0,0,0,1,0,0) \mapsto (D,E,L,N,Q,U)$
$(\overline{\mathbf{4}}, \mathbf{1}, \mathbf{2}, \mathbf{1})$, $(0,0,1,0,0,0,0,0,1,0) \mapsto (L,Q)$
$(\overline{\mathbf{4}}, \mathbf{1}, \mathbf{2}, \mathbf{1})$, $(0,0,1,0,0,0,0,0,1,0) \mapsto (L,Q)$
$(\mathbf{4}, \mathbf{1}, \mathbf{1}, \mathbf{2})$, $(1,0,0,0,0,0,0,0,0,1) \mapsto (D,E,N,U)$
$(\mathbf{4}, \mathbf{1}, \mathbf{1}, \mathbf{2})$, $(1,0,0,0,0,0,0,0,0,1) \mapsto (D,E,N,U)$
Projection matrix for $\alpha$:

$$\begin{pmatrix} 0 & 1 & 0 & 0 & 0 & 1 & 0 & 0 & 0 & 0 \\ 1 & 0 & 0 & 0 & 0 & 0 & 0 & 1 & 0 & 0 \\ 0 & 0 & 0 & 1 & 0 & 0 & 0 & 0 & 1 & 0 \\ -1 & -2 & -3 & 3 & 6 & 4 & 0 & 2 & 0 & 3 \end{pmatrix}$$

**3 generation subalgebra** 134
Algebra: $\mathfrak{su}(4) \oplus \mathfrak{sp}(4) \oplus \mathfrak{so}(10) \oplus \mathfrak{su}(2)$
$(\overline{\mathbf{4}}, \mathbf{4}, \mathbf{1}, \mathbf{1})$, $(0,0,1,1,0,0,0,0,0,0,0,0) \mapsto (L,L,Q,Q)$
$(\mathbf{1}, \mathbf{1}, \mathbf{16}, \mathbf{1})$, $(0,0,0,0,0,0,0,0,0,0,1,0) \mapsto (D,E,L,N,Q,U)$
$(\mathbf{4}, \mathbf{1}, \mathbf{1}, \mathbf{2})$, $(1,0,0,0,0,0,0,0,0,0,0,1) \mapsto (D,E,N,U)$
$(\mathbf{4}, \mathbf{1}, \mathbf{1}, \mathbf{2})$, $(1,0,0,0,0,0,0,0,0,0,0,1) \mapsto (D,E,N,U)$
Projection matrix for $\alpha$:

$$\begin{pmatrix} 0 & 1 & 0 & 0 & 0 & 0 & 0 & 1 & 0 & 0 & 0 \\ 1 & 0 & 0 & 0 & 0 & 0 & 0 & 0 & 0 & 1 & 0 \\ 0 & 0 & 0 & 1 & 2 & 1 & 0 & 0 & 0 & 0 & 0 \\ -1 & -2 & -3 & 0 & 0 & 3 & 6 & 4 & 0 & 2 & 3 \end{pmatrix}$$

**3 generation subalgebra** 135
Algebra: $\mathfrak{su}(4) \oplus \mathfrak{sp}(4) \oplus \mathfrak{so}(10) \oplus \mathfrak{su}(2)$
$(\overline{\mathbf{4}}, \mathbf{4}, \mathbf{1}, \mathbf{1})$, $(0,0,1,1,0,0,0,0,0,0,0,0) \mapsto (D,D,E,E,N,N,U,U)$
$(\mathbf{1}, \mathbf{1}, \mathbf{16}, \mathbf{1})$, $(0,0,0,0,0,0,0,0,0,0,1,0) \mapsto (D,E,L,N,Q,U)$
$(\mathbf{4}, \mathbf{1}, \mathbf{1}, \mathbf{2})$, $(1,0,0,0,0,0,0,0,0,0,0,1) \mapsto (L,Q)$
$(\mathbf{4}, \mathbf{1}, \mathbf{1}, \mathbf{2})$, $(1,0,0,0,0,0,0,0,0,0,0,1) \mapsto (L,Q)$
Projection matrix for $\alpha$:

$$\begin{pmatrix} 1 & 0 & 0 & 0 & 0 & 0 & 0 & 1 & 0 & 0 & 0 \\ 0 & 1 & 0 & 0 & 0 & 0 & 0 & 0 & 0 & 1 & 0 \\ 0 & 0 & 0 & 0 & 0 & 1 & 0 & 0 & 0 & 0 & 1 \\ 1 & 2 & 3 & 3 & 0 & 3 & 6 & 4 & 0 & 2 & 0 \end{pmatrix}$$

**3 generation subalgebra** 136
Algebra: $\mathfrak{su}(4) \oplus \mathfrak{sp}(4) \oplus \mathfrak{sp}(6) \oplus \mathfrak{su}(2)$
$(\overline{\mathbf{4}}, \mathbf{4}, \mathbf{1}, \mathbf{1})$, $(0,0,1,1,0,0,0,0,0,0) \mapsto (L,L,Q,Q)$
$(\mathbf{4}, \mathbf{1}, \mathbf{6}, \mathbf{1})$, $(1,0,0,0,0,1,0,0,0,0) \mapsto (D,D,D,E,E,E,N,N,N,U,U,U)$
$(\overline{\mathbf{4}}, \mathbf{1}, \mathbf{1}, \mathbf{2})$, $(0,0,1,0,0,0,0,0,0,1) \mapsto (L,Q)$

Projection matrix for $\alpha$:

$$\begin{pmatrix} 0 & 1 & 0 & 0 & 0 & 0 & 0 & 0 & 0 \\ 1 & 0 & 0 & 0 & 0 & 0 & 0 & 0 & 0 \\ 0 & 0 & 0 & 1 & 2 & 0 & 0 & 0 & 1 \\ -1 & -2 & -3 & 0 & 0 & 3 & 0 & -3 & 0 \end{pmatrix}$$

**3 generation subalgebra** 137
Algebra: $\mathfrak{su}(4) \oplus \mathfrak{sp}(4) \oplus \mathfrak{sp}(6) \oplus \mathfrak{su}(2)$
$(\overline{\mathbf{4}}, \mathbf{4}, \mathbf{1}, \mathbf{1}),\ (0,0,1,1,0,0,0,0,0) \mapsto (D,D,E,E,N,N,U,U)$
$(\mathbf{4}, \mathbf{1}, \mathbf{6}, \mathbf{1}),\ (1,0,0,0,0,1,0,0,0) \mapsto (L,L,L,Q,Q,Q)$
$(\overline{\mathbf{4}}, \mathbf{1}, \mathbf{1}, \mathbf{2}),\ (0,0,1,0,0,0,0,0,1) \mapsto (D,E,N,U)$
Projection matrix for $\alpha$:

$$\begin{pmatrix} 1 & 0 & 0 & 0 & 0 & 0 & 0 & 0 & 0 \\ 0 & 1 & 0 & 0 & 0 & 0 & 0 & 0 & 0 \\ 0 & 0 & 0 & 0 & 0 & 1 & 2 & 3 & 0 \\ 1 & 2 & 3 & 3 & 0 & 0 & 0 & 0 & 3 \end{pmatrix}$$

**3 generation subalgebra** 138
Algebra: $\mathfrak{su}(4) \oplus \mathfrak{sp}(4) \oplus \mathfrak{su}(2) \oplus \mathfrak{su}(2)$
$(\overline{\mathbf{4}}, \mathbf{4}, \mathbf{1}, \mathbf{1}),\ (0,0,1,1,0,0,0) \mapsto (L,L,Q,Q)$
$(\overline{\mathbf{4}}, \mathbf{1}, \mathbf{2}, \mathbf{1}),\ (0,0,1,0,0,1,0) \mapsto (L,Q)$
$(\mathbf{4}, \mathbf{1}, \mathbf{1}, \mathbf{2}),\ (1,0,0,0,0,0,1) \mapsto (D,E,N,U)$
$(\mathbf{4}, \mathbf{1}, \mathbf{1}, \mathbf{2}),\ (1,0,0,0,0,0,1) \mapsto (D,E,N,U)$
$(\mathbf{4}, \mathbf{1}, \mathbf{1}, \mathbf{2}),\ (1,0,0,0,0,0,1) \mapsto (D,E,N,U)$
Projection matrix for $\alpha$:

$$\begin{pmatrix} 0 & 1 & 0 & 0 & 0 & 0 & 0 \\ 1 & 0 & 0 & 0 & 0 & 0 & 0 \\ 0 & 0 & 0 & 1 & 2 & 1 & 0 \\ -1 & -2 & -3 & 0 & 0 & 0 & 3 \end{pmatrix}$$

**3 generation subalgebra** 139
Algebra: $\mathfrak{su}(4) \oplus \mathfrak{sp}(4) \oplus \mathfrak{su}(2) \oplus \mathfrak{su}(2)$
$(\overline{\mathbf{4}}, \mathbf{4}, \mathbf{1}, \mathbf{1}),\ (0,0,1,1,0,0,0) \mapsto (D,D,E,E,N,N,U,U)$
$(\overline{\mathbf{4}}, \mathbf{1}, \mathbf{2}, \mathbf{1}),\ (0,0,1,0,0,1,0) \mapsto (D,E,N,U)$
$(\mathbf{4}, \mathbf{1}, \mathbf{1}, \mathbf{2}),\ (1,0,0,0,0,0,1) \mapsto (L,Q)$
$(\mathbf{4}, \mathbf{1}, \mathbf{1}, \mathbf{2}),\ (1,0,0,0,0,0,1) \mapsto (L,Q)$
$(\mathbf{4}, \mathbf{1}, \mathbf{1}, \mathbf{2}),\ (1,0,0,0,0,0,1) \mapsto (L,Q)$
Projection matrix for $\alpha$:

$$\begin{pmatrix} 1 & 0 & 0 & 0 & 0 & 0 & 0 \\ 0 & 1 & 0 & 0 & 0 & 0 & 0 \\ 0 & 0 & 0 & 0 & 0 & 0 & 1 \\ 1 & 2 & 3 & 3 & 0 & 3 & 0 \end{pmatrix}$$

**3 generation subalgebra** 140
Algebra: $\mathfrak{su}(4) \oplus \mathfrak{sp}(6) \oplus \mathfrak{su}(2) \oplus \mathfrak{su}(2)$
$(\overline{\mathbf{4}}, \mathbf{6}, \mathbf{1}, \mathbf{1}),\ (0,0,1,1,0,0,0,0) \mapsto (L,L,L,Q,Q,Q)$
$(\mathbf{4}, \mathbf{1}, \mathbf{3}, \mathbf{2}),\ (1,0,0,0,0,0,2,1) \mapsto (D,D,D,E,E,E,N,N,N,U,U,U)$
Projection matrix for $\alpha$:

$$\begin{pmatrix} 0 & 1 & 0 & 0 & 0 & 0 & 0 & 0 \\ 1 & 0 & 0 & 0 & 0 & 0 & 0 & 0 \\ 0 & 0 & 0 & 1 & 2 & 3 & 0 & 0 \\ -1 & -2 & -3 & 0 & 0 & 0 & 0 & 3 \end{pmatrix}$$

**3 generation subalgebra** 141
Algebra: $\mathfrak{su}(4) \oplus \mathfrak{sp}(6) \oplus \mathfrak{su}(2) \oplus \mathfrak{su}(2)$

$(\bar{\mathbf{4}},\mathbf{6},\mathbf{1},\mathbf{1})$, $(0,0,1,1,0,0,0,0) \mapsto (D,D,D,E,E,E,N,N,N,U,U,U)$
$(\mathbf{4},\mathbf{1},\mathbf{3},\mathbf{2})$, $(1,0,0,0,0,0,2,1) \mapsto (L,L,L,Q,Q,Q)$
Projection matrix for $\alpha$:

$$\begin{pmatrix} 1 & 0 & 0 & 0 & 0 & 0 & 0 & 0 \\ 0 & 1 & 0 & 0 & 0 & 0 & 0 & 0 \\ 0 & 0 & 0 & 0 & 0 & 0 & 0 & 1 \\ 1 & 2 & 3 & 3 & 0 & -3 & 0 & 0 \end{pmatrix}$$

**3 generation subalgebra** 142
Algebra: $\mathfrak{su}(4) \oplus \mathfrak{sp}(6) \oplus \mathfrak{su}(2) \oplus \mathfrak{su}(2)$
$(\bar{\mathbf{4}},\mathbf{6},\mathbf{1},\mathbf{1})$, $(0,0,1,1,0,0,0,0) \mapsto (L,L,L,Q,Q,Q)$
$(\mathbf{4},\mathbf{1},\mathbf{2},\mathbf{2})$, $(1,0,0,0,0,0,1,1) \mapsto (D,D,E,E,N,N,U,U)$
$(\mathbf{4},\mathbf{1},\mathbf{2},\mathbf{1})$, $(1,0,0,0,0,0,1,0) \mapsto (D,E,N,U)$
Projection matrix for $\alpha$:

$$\begin{pmatrix} 0 & 1 & 0 & 0 & 0 & 0 & 0 & 0 \\ 1 & 0 & 0 & 0 & 0 & 0 & 0 & 0 \\ 0 & 0 & 0 & 1 & 2 & 3 & 0 & 0 \\ -1 & -2 & -3 & 0 & 0 & 0 & 3 & 0 \end{pmatrix}$$

**3 generation subalgebra** 143
Algebra: $\mathfrak{su}(4) \oplus \mathfrak{sp}(6) \oplus \mathfrak{su}(2) \oplus \mathfrak{su}(2)$
$(\bar{\mathbf{4}},\mathbf{6},\mathbf{1},\mathbf{1})$, $(0,0,1,1,0,0,0,0) \mapsto (D,D,D,E,E,E,N,N,N,U,U,U)$
$(\mathbf{4},\mathbf{1},\mathbf{2},\mathbf{2})$, $(1,0,0,0,0,0,1,1) \mapsto (L,L,Q,Q)$
$(\mathbf{4},\mathbf{1},\mathbf{2},\mathbf{1})$, $(1,0,0,0,0,0,1,0) \mapsto (L,Q)$
Projection matrix for $\alpha$:

$$\begin{pmatrix} 1 & 0 & 0 & 0 & 0 & 0 & 0 & 0 \\ 0 & 1 & 0 & 0 & 0 & 0 & 0 & 0 \\ 0 & 0 & 0 & 0 & 0 & 0 & 1 & 0 \\ 1 & 2 & 3 & 3 & 0 & -3 & 0 & 0 \end{pmatrix}$$

**3 generation subalgebra** 144
Algebra: $\mathfrak{su}(4) \oplus \mathfrak{sp}(6) \oplus \mathfrak{su}(2) \oplus \mathfrak{su}(2)$
$(\bar{\mathbf{4}},\mathbf{6},\mathbf{1},\mathbf{1})$, $(0,0,1,1,0,0,0,0) \mapsto (L,L,L,Q,Q,Q)$
$(\mathbf{4},\mathbf{1},\mathbf{2},\mathbf{1})$, $(1,0,0,0,0,0,1,0) \mapsto (D,E,N,U)$
$(\mathbf{4},\mathbf{1},\mathbf{2},\mathbf{1})$, $(1,0,0,0,0,0,1,0) \mapsto (D,E,N,U)$
$(\mathbf{4},\mathbf{1},\mathbf{1},\mathbf{2})$, $(1,0,0,0,0,0,0,1) \mapsto (D,E,N,U)$
Projection matrix for $\alpha$:

$$\begin{pmatrix} 0 & 1 & 0 & 0 & 0 & 0 & 0 & 0 \\ 1 & 0 & 0 & 0 & 0 & 0 & 0 & 0 \\ 0 & 0 & 0 & 1 & 2 & 3 & 0 & 0 \\ -1 & -2 & -3 & 0 & 0 & 0 & 3 & 3 \end{pmatrix}$$

**3 generation subalgebra** 145
Algebra: $\mathfrak{su}(4) \oplus \mathfrak{sp}(6) \oplus \mathfrak{su}(2) \oplus \mathfrak{su}(2)$
$(\bar{\mathbf{4}},\mathbf{6},\mathbf{1},\mathbf{1})$, $(0,0,1,1,0,0,0,0) \mapsto (D,D,D,E,E,E,N,N,N,U,U,U)$
$(\mathbf{4},\mathbf{1},\mathbf{2},\mathbf{1})$, $(1,0,0,0,0,0,1,0) \mapsto (L,Q)$
$(\mathbf{4},\mathbf{1},\mathbf{2},\mathbf{1})$, $(1,0,0,0,0,0,1,0) \mapsto (L,Q)$
$(\mathbf{4},\mathbf{1},\mathbf{1},\mathbf{2})$, $(1,0,0,0,0,0,0,1) \mapsto (L,Q)$
Projection matrix for $\alpha$:

$$\begin{pmatrix} 1 & 0 & 0 & 0 & 0 & 0 & 0 & 0 \\ 0 & 1 & 0 & 0 & 0 & 0 & 0 & 0 \\ 0 & 0 & 0 & 0 & 0 & 0 & 1 & 1 \\ 1 & 2 & 3 & 3 & 0 & -3 & 0 & 0 \end{pmatrix}$$

**3 generation subalgebra** 146
Algebra: $\mathfrak{su}(4) \oplus \mathfrak{su}(2) \oplus \mathfrak{su}(2) \oplus \mathfrak{su}(2)$

$(\mathbf{4},\mathbf{3},\mathbf{2},\mathbf{1})$, $(1,0,0,2,1,0)\mapsto(L,L,L,Q,Q,Q)$
$(\overline{\mathbf{4}},\mathbf{3},\mathbf{1},\mathbf{2})$, $(0,0,1,2,0,1)\mapsto(D,D,D,E,E,E,N,N,N,U,U,U)$
Projection matrix for $\alpha$:

$$\begin{pmatrix}1&0&0&0&0&0\\0&1&0&0&0&0\\0&0&0&0&1&0\\1&2&3&0&0&3\end{pmatrix}$$

**3 generation subalgebra** 147
Algebra: $\mathfrak{su}(4)\oplus\mathfrak{su}(2)\oplus\mathfrak{su}(2)\oplus\mathfrak{su}(2)$
$(\mathbf{4},\mathbf{2},\mathbf{2},\mathbf{1})$, $(1,0,0,1,1,0)\mapsto(D,D,E,E,N,N,U,U)$
$(\overline{\mathbf{4}},\mathbf{3},\mathbf{1},\mathbf{2})$, $(0,0,1,2,0,1)\mapsto(L,L,L,Q,Q,Q)$
$(\mathbf{4},\mathbf{1},\mathbf{2},\mathbf{1})$, $(1,0,0,0,1,0)\mapsto(D,E,N,U)$
Projection matrix for $\alpha$:

$$\begin{pmatrix}0&1&0&0&0&0\\1&0&0&0&0&0\\0&0&0&0&0&1\\-1&-2&-3&0&3&0\end{pmatrix}$$

**3 generation subalgebra** 148
Algebra: $\mathfrak{su}(4)\oplus\mathfrak{su}(2)\oplus\mathfrak{su}(2)\oplus\mathfrak{su}(2)$
$(\mathbf{4},\mathbf{2},\mathbf{2},\mathbf{1})$, $(1,0,0,1,1,0)\mapsto(L,L,Q,Q)$
$(\overline{\mathbf{4}},\mathbf{3},\mathbf{1},\mathbf{2})$, $(0,0,1,2,0,1)\mapsto(D,D,D,E,E,E,N,N,N,U,U,U)$
$(\mathbf{4},\mathbf{1},\mathbf{2},\mathbf{1})$, $(1,0,0,0,1,0)\mapsto(L,Q)$
Projection matrix for $\alpha$:

$$\begin{pmatrix}1&0&0&0&0&0\\0&1&0&0&0&0\\0&0&0&0&1&0\\1&2&3&0&0&3\end{pmatrix}$$

**3 generation subalgebra** 149
Algebra: $\mathfrak{su}(4)\oplus\mathfrak{su}(2)\oplus\mathfrak{su}(2)\oplus\mathfrak{su}(2)$
$(\mathbf{4},\mathbf{2},\mathbf{2},\mathbf{1})$, $(1,0,0,1,1,0)\mapsto(L,L,Q,Q)$
$(\overline{\mathbf{4}},\mathbf{2},\mathbf{1},\mathbf{2})$, $(0,0,1,1,0,1)\mapsto(D,D,E,E,N,N,U,U)$
$(\mathbf{4},\mathbf{1},\mathbf{2},\mathbf{1})$, $(1,0,0,0,1,0)\mapsto(L,Q)$
$(\overline{\mathbf{4}},\mathbf{1},\mathbf{1},\mathbf{2})$, $(0,0,1,0,0,1)\mapsto(D,E,N,U)$
Projection matrix for $\alpha$:

$$\begin{pmatrix}1&0&0&0&0&0\\0&1&0&0&0&0\\0&0&0&0&1&0\\1&2&3&0&0&3\end{pmatrix}$$

**3 generation subalgebra** 150
Algebra: $\mathfrak{su}(4)\oplus\mathfrak{su}(2)\oplus\mathfrak{su}(2)\oplus\mathfrak{su}(2)$
$(\mathbf{4},\mathbf{3},\mathbf{2},\mathbf{1})$, $(1,0,0,2,1,0)\mapsto(D,D,D,E,E,E,N,N,N,U,U,U)$
$(\overline{\mathbf{4}},\mathbf{1},\mathbf{1},\mathbf{2})$, $(0,0,1,0,0,1)\mapsto(L,Q)$
$(\overline{\mathbf{4}},\mathbf{1},\mathbf{1},\mathbf{2})$, $(0,0,1,0,0,1)\mapsto(L,Q)$
$(\overline{\mathbf{4}},\mathbf{1},\mathbf{1},\mathbf{2})$, $(0,0,1,0,0,1)\mapsto(L,Q)$
Projection matrix for $\alpha$:

$$\begin{pmatrix}0&1&0&0&0&0\\1&0&0&0&0&0\\0&0&0&0&0&1\\-1&-2&-3&0&3&0\end{pmatrix}$$

**3 generation subalgebra** 151
Algebra: $\mathfrak{su}(4)\oplus\mathfrak{su}(2)\oplus\mathfrak{su}(2)\oplus\mathfrak{su}(2)$

$(\mathbf{4}, \mathbf{3}, \mathbf{2}, \mathbf{1})$, $(1,0,0,2,1,0) \mapsto (L,L,L,Q,Q,Q)$
$(\overline{\mathbf{4}}, \mathbf{1}, \mathbf{1}, \mathbf{2})$, $(0,0,1,0,0,1) \mapsto (D,E,N,U)$
$(\overline{\mathbf{4}}, \mathbf{1}, \mathbf{1}, \mathbf{2})$, $(0,0,1,0,0,1) \mapsto (D,E,N,U)$
$(\overline{\mathbf{4}}, \mathbf{1}, \mathbf{1}, \mathbf{2})$, $(0,0,1,0,0,1) \mapsto (D,E,N,U)$
Projection matrix for $\alpha$:

$$\begin{pmatrix} 1 & 0 & 0 & 0 & 0 & 0 \\ 0 & 1 & 0 & 0 & 0 & 0 \\ 0 & 0 & 0 & 0 & 1 & 0 \\ 1 & 2 & 3 & 0 & 0 & 3 \end{pmatrix}$$

**3 generation subalgebra** 152
Algebra: $\mathfrak{su}(4) \oplus \mathfrak{su}(2) \oplus \mathfrak{su}(2) \oplus \mathfrak{su}(2)$
$(\mathbf{4}, \mathbf{2}, \mathbf{2}, \mathbf{1})$, $(1,0,0,1,1,0) \mapsto (D,D,E,E,N,N,U,U)$
$(\mathbf{4}, \mathbf{2}, \mathbf{1}, \mathbf{1})$, $(1,0,0,1,0,0) \mapsto (D,E,N,U)$
$(\overline{\mathbf{4}}, \mathbf{1}, \mathbf{1}, \mathbf{2})$, $(0,0,1,0,0,1) \mapsto (L,Q)$
$(\overline{\mathbf{4}}, \mathbf{1}, \mathbf{1}, \mathbf{2})$, $(0,0,1,0,0,1) \mapsto (L,Q)$
$(\overline{\mathbf{4}}, \mathbf{1}, \mathbf{1}, \mathbf{2})$, $(0,0,1,0,0,1) \mapsto (L,Q)$
Projection matrix for $\alpha$:

$$\begin{pmatrix} 0 & 1 & 0 & 0 & 0 & 0 \\ 1 & 0 & 0 & 0 & 0 & 0 \\ 0 & 0 & 0 & 0 & 0 & 1 \\ -1 & -2 & -3 & 3 & 0 & 0 \end{pmatrix}$$

**3 generation subalgebra** 153
Algebra: $\mathfrak{su}(4) \oplus \mathfrak{su}(2) \oplus \mathfrak{su}(2) \oplus \mathfrak{su}(2)$
$(\mathbf{4}, \mathbf{2}, \mathbf{2}, \mathbf{1})$, $(1,0,0,1,1,0) \mapsto (L,L,Q,Q)$
$(\mathbf{4}, \mathbf{2}, \mathbf{1}, \mathbf{1})$, $(1,0,0,1,0,0) \mapsto (L,Q)$
$(\overline{\mathbf{4}}, \mathbf{1}, \mathbf{1}, \mathbf{2})$, $(0,0,1,0,0,1) \mapsto (D,E,N,U)$
$(\overline{\mathbf{4}}, \mathbf{1}, \mathbf{1}, \mathbf{2})$, $(0,0,1,0,0,1) \mapsto (D,E,N,U)$
$(\overline{\mathbf{4}}, \mathbf{1}, \mathbf{1}, \mathbf{2})$, $(0,0,1,0,0,1) \mapsto (D,E,N,U)$
Projection matrix for $\alpha$:

$$\begin{pmatrix} 1 & 0 & 0 & 0 & 0 & 0 \\ 0 & 1 & 0 & 0 & 0 & 0 \\ 0 & 0 & 0 & 1 & 0 & 0 \\ 1 & 2 & 3 & 0 & 0 & 3 \end{pmatrix}$$

**3 generation subalgebra** 154
Algebra: $\mathfrak{su}(4) \oplus \mathfrak{su}(2) \oplus \mathfrak{su}(2) \oplus \mathfrak{su}(2)$
$(\overline{\mathbf{4}}, \mathbf{2}, \mathbf{1}, \mathbf{1})$, $(0,0,1,1,0,0) \mapsto (L,Q)$
$(\overline{\mathbf{4}}, \mathbf{2}, \mathbf{1}, \mathbf{1})$, $(0,0,1,1,0,0) \mapsto (L,Q)$
$(\overline{\mathbf{4}}, \mathbf{2}, \mathbf{1}, \mathbf{1})$, $(0,0,1,1,0,0) \mapsto (L,Q)$
$(\mathbf{4}, \mathbf{1}, \mathbf{2}, \mathbf{1})$, $(1,0,0,0,1,0) \mapsto (D,E,N,U)$
$(\mathbf{4}, \mathbf{1}, \mathbf{2}, \mathbf{1})$, $(1,0,0,0,1,0) \mapsto (D,E,N,U)$
$(\mathbf{4}, \mathbf{1}, \mathbf{1}, \mathbf{2})$, $(1,0,0,0,0,1) \mapsto (D,E,N,U)$
Projection matrix for $\alpha$:

$$\begin{pmatrix} 0 & 1 & 0 & 0 & 0 & 0 \\ 1 & 0 & 0 & 0 & 0 & 0 \\ 0 & 0 & 0 & 1 & 0 & 0 \\ -1 & -2 & -3 & 0 & 3 & 3 \end{pmatrix}$$

**3 generation subalgebra** 155
Algebra: $\mathfrak{su}(4) \oplus \mathfrak{su}(2) \oplus \mathfrak{su}(2) \oplus \mathfrak{su}(2)$
$(\overline{\mathbf{4}}, \mathbf{2}, \mathbf{1}, \mathbf{1})$, $(0,0,1,1,0,0) \mapsto (D,E,N,U)$
$(\overline{\mathbf{4}}, \mathbf{2}, \mathbf{1}, \mathbf{1})$, $(0,0,1,1,0,0) \mapsto (D,E,N,U)$
$(\overline{\mathbf{4}}, \mathbf{2}, \mathbf{1}, \mathbf{1})$, $(0,0,1,1,0,0) \mapsto (D,E,N,U)$
$(\mathbf{4}, \mathbf{1}, \mathbf{2}, \mathbf{1})$, $(1,0,0,0,1,0) \mapsto (L,Q)$

$(\mathbf{4},\mathbf{1},\mathbf{2},\mathbf{1}),\ (1,0,0,0,1,0)\mapsto(L,Q)$
$(\mathbf{4},\mathbf{1},\mathbf{1},\mathbf{2}),\ (1,0,0,0,0,1)\mapsto(L,Q)$
Projection matrix for $\alpha$:

$$\begin{pmatrix}1&0&0&0&0&0\\0&1&0&0&0&0\\0&0&0&0&1&1\\1&2&3&3&0&0\end{pmatrix}$$

**3 generation subalgebra** 156
Algebra: $\mathfrak{su}(4)\oplus\mathfrak{su}(4)\oplus\mathfrak{sp}(4)\oplus\mathfrak{su}(2)$
$(\overline{\mathbf{4}},\mathbf{6},\mathbf{1},\mathbf{1}),\ (0,0,1,0,1,0,0,0,0)\mapsto(D,D,D,E,E,E,N,N,N,U,U,U)$
$(\mathbf{4},\mathbf{1},\mathbf{4},\mathbf{1}),\ (1,0,0,0,0,0,1,0,0)\mapsto(L,L,Q,Q)$
$(\mathbf{4},\mathbf{1},\mathbf{1},\mathbf{2}),\ (1,0,0,0,0,0,0,0,1)\mapsto(L,Q)$
Projection matrix for $\alpha$:

$$\begin{pmatrix}1&0&0&0&0&0&0&0&0\\0&1&0&0&0&0&0&0&0\\0&0&0&0&0&0&1&2&1\\1&2&3&\frac{9}{2}&3&\frac{3}{2}&0&0&0\end{pmatrix}$$

**3 generation subalgebra** 157
Algebra: $\mathfrak{su}(4)\oplus\mathfrak{su}(4)\oplus\mathfrak{su}(2)\oplus\mathfrak{su}(2)$
$(\overline{\mathbf{4}},\mathbf{6},\mathbf{1},\mathbf{1}),\ (0,0,1,0,1,0,0,0)\mapsto(D,D,D,E,E,E,N,N,N,U,U,U)$
$(\mathbf{4},\mathbf{1},\mathbf{3},\mathbf{2}),\ (1,0,0,0,0,0,2,1)\mapsto(L,L,L,Q,Q,Q)$
Projection matrix for $\alpha$:

$$\begin{pmatrix}1&0&0&0&0&0&0&0\\0&1&0&0&0&0&0&0\\0&0&0&0&0&0&0&1\\1&2&3&\frac{9}{2}&3&\frac{3}{2}&0&0\end{pmatrix}$$

**3 generation subalgebra** 158
Algebra: $\mathfrak{su}(4)\oplus\mathfrak{su}(4)\oplus\mathfrak{su}(2)\oplus\mathfrak{su}(2)$
$(\overline{\mathbf{4}},\mathbf{6},\mathbf{1},\mathbf{1}),\ (0,0,1,0,1,0,0,0)\mapsto(D,D,D,E,E,E,N,N,N,U,U,U)$
$(\mathbf{4},\mathbf{1},\mathbf{2},\mathbf{2}),\ (1,0,0,0,0,0,1,1)\mapsto(L,L,Q,Q)$
$(\mathbf{4},\mathbf{1},\mathbf{2},\mathbf{1}),\ (1,0,0,0,0,0,1,0)\mapsto(L,Q)$
Projection matrix for $\alpha$:

$$\begin{pmatrix}1&0&0&0&0&0&0&0\\0&1&0&0&0&0&0&0\\0&0&0&0&0&0&1&0\\1&2&3&\frac{9}{2}&3&\frac{3}{2}&0&0\end{pmatrix}$$

**3 generation subalgebra** 159
Algebra: $\mathfrak{su}(4)\oplus\mathfrak{su}(4)\oplus\mathfrak{su}(2)\oplus\mathfrak{su}(2)$
$(\overline{\mathbf{4}},\mathbf{6},\mathbf{1},\mathbf{1}),\ (0,0,1,0,1,0,0,0)\mapsto(D,D,D,E,E,E,N,N,N,U,U,U)$
$(\mathbf{4},\mathbf{1},\mathbf{2},\mathbf{1}),\ (1,0,0,0,0,0,1,0)\mapsto(L,Q)$
$(\mathbf{4},\mathbf{1},\mathbf{2},\mathbf{1}),\ (1,0,0,0,0,0,1,0)\mapsto(L,Q)$
$(\mathbf{4},\mathbf{1},\mathbf{1},\mathbf{2}),\ (1,0,0,0,0,0,0,1)\mapsto(L,Q)$
Projection matrix for $\alpha$:

$$\begin{pmatrix}1&0&0&0&0&0&0&0\\0&1&0&0&0&0&0&0\\0&0&0&0&0&0&1&1\\1&2&3&\frac{9}{2}&3&\frac{3}{2}&0&0\end{pmatrix}$$

**3 generation subalgebra** 160
Algebra: $\mathfrak{su}(4)\oplus\mathfrak{su}(4)\oplus\mathfrak{su}(2)\oplus\mathfrak{su}(2)$
$(\overline{\mathbf{4}},\mathbf{1},\mathbf{2},\mathbf{1}),\ (0,0,1,0,0,0,1,0)\mapsto(L,Q)$

$(\overline{\mathbf{4}}, \mathbf{1}, \mathbf{2}, \mathbf{1})$, $(0,0,1,0,0,0,1,0) \mapsto (L, Q)$
$(\mathbf{1}, \overline{\mathbf{4}}, \mathbf{2}, \mathbf{1})$, $(0,0,0,0,0,1,1,0) \mapsto (L, Q)$
$(\mathbf{4}, \mathbf{1}, \mathbf{1}, \mathbf{2})$, $(1,0,0,0,0,0,0,1) \mapsto (D, E, N, U)$
$(\mathbf{4}, \mathbf{1}, \mathbf{1}, \mathbf{2})$, $(1,0,0,0,0,0,0,1) \mapsto (D, E, N, U)$
$(\mathbf{1}, \mathbf{4}, \mathbf{1}, \mathbf{2})$, $(0,0,0,1,0,0,0,1) \mapsto (D, E, N, U)$
Projection matrix for $\alpha$:

$$\begin{pmatrix} 0 & 1 & 0 & 0 & 1 & 0 & 0 & 0 \\ 1 & 0 & 0 & 1 & 0 & 0 & 0 & 0 \\ 0 & 0 & 0 & 0 & 0 & 0 & 1 & 0 \\ -1 & -2 & -3 & -1 & -2 & -3 & 0 & 3 \end{pmatrix}$$

**3 generation subalgebra** 161
Algebra: $\mathfrak{su}(4) \oplus \mathfrak{su}(5) \oplus \mathfrak{sp}(4) \oplus \mathfrak{sp}(4)$
$(\overline{\mathbf{4}}, \mathbf{1}, \mathbf{4}, \mathbf{1})$, $(0,0,1,0,0,0,0,1,0,0,0) \mapsto (L, L, Q, Q)$
$(\mathbf{4}, \mathbf{1}, \mathbf{1}, \mathbf{4})$, $(1,0,0,0,0,0,0,0,0,1,0) \mapsto (D, D, E, E, N, N, U, U)$
$(\mathbf{1}, \overline{\mathbf{5}}, \mathbf{1}, \mathbf{1})$, $(0,0,0,0,0,0,1,0,0,0,0) \mapsto (D, L)$
$(\mathbf{1}, \mathbf{10}, \mathbf{1}, \mathbf{1})$, $(0,0,0,0,1,0,0,0,0,0,0) \mapsto (E, Q, U)$
$(\mathbf{1}, \mathbf{1}, \mathbf{1}, \mathbf{1})$, $(0,0,0,0,0,0,0,0,0,0,0) \mapsto (N)$
Projection matrix for $\alpha$:

$$\begin{pmatrix} 0 & 1 & 0 & 0 & 0 & 1 & 0 & 0 & 0 & 0 & 0 \\ 1 & 0 & 0 & 0 & 0 & 0 & 1 & 0 & 0 & 0 & 0 \\ 0 & 0 & 0 & 1 & 0 & 0 & 0 & 1 & 2 & 0 & 0 \\ -1 & -2 & -3 & 3 & 6 & 4 & 2 & 0 & 0 & 3 & 0 \end{pmatrix}$$

**3 generation subalgebra** 162
Algebra: $\mathfrak{su}(4) \oplus \mathfrak{su}(5) \oplus \mathfrak{sp}(4) \oplus \mathfrak{su}(2)$
$(\overline{\mathbf{4}}, \mathbf{1}, \mathbf{4}, \mathbf{1})$, $(0,0,1,0,0,0,0,1,0,0) \mapsto (L, L, Q, Q)$
$(\mathbf{1}, \overline{\mathbf{5}}, \mathbf{1}, \mathbf{1})$, $(0,0,0,0,0,0,1,0,0,0) \mapsto (D, L)$
$(\mathbf{1}, \mathbf{10}, \mathbf{1}, \mathbf{1})$, $(0,0,0,0,1,0,0,0,0,0) \mapsto (E, Q, U)$
$(\mathbf{4}, \mathbf{1}, \mathbf{1}, \mathbf{2})$, $(1,0,0,0,0,0,0,0,0,1) \mapsto (D, E, N, U)$
$(\mathbf{4}, \mathbf{1}, \mathbf{1}, \mathbf{2})$, $(1,0,0,0,0,0,0,0,0,1) \mapsto (D, E, N, U)$
$(\mathbf{1}, \mathbf{1}, \mathbf{1}, \mathbf{1})$, $(0,0,0,0,0,0,0,0,0,0) \mapsto (N)$
Projection matrix for $\alpha$:

$$\begin{pmatrix} 0 & 1 & 0 & 0 & 0 & 1 & 0 & 0 & 0 & 0 \\ 1 & 0 & 0 & 0 & 0 & 0 & 1 & 0 & 0 & 0 \\ 0 & 0 & 0 & 1 & 0 & 0 & 0 & 1 & 2 & 0 \\ -1 & -2 & -3 & 3 & 6 & 4 & 2 & 0 & 0 & 3 \end{pmatrix}$$

**3 generation subalgebra** 163
Algebra: $\mathfrak{su}(4) \oplus \mathfrak{su}(5) \oplus \mathfrak{sp}(4) \oplus \mathfrak{su}(2)$
$(\overline{\mathbf{4}}, \mathbf{1}, \mathbf{4}, \mathbf{1})$, $(0,0,1,0,0,0,0,1,0,0) \mapsto (D, D, E, E, N, N, U, U)$
$(\mathbf{1}, \overline{\mathbf{5}}, \mathbf{1}, \mathbf{1})$, $(0,0,0,0,0,0,1,0,0,0) \mapsto (D, L)$
$(\mathbf{1}, \mathbf{10}, \mathbf{1}, \mathbf{1})$, $(0,0,0,0,1,0,0,0,0,0) \mapsto (E, Q, U)$
$(\mathbf{4}, \mathbf{1}, \mathbf{1}, \mathbf{2})$, $(1,0,0,0,0,0,0,0,0,1) \mapsto (L, Q)$
$(\mathbf{4}, \mathbf{1}, \mathbf{1}, \mathbf{2})$, $(1,0,0,0,0,0,0,0,0,1) \mapsto (L, Q)$
$(\mathbf{1}, \mathbf{1}, \mathbf{1}, \mathbf{1})$, $(0,0,0,0,0,0,0,0,0,0) \mapsto (N)$
Projection matrix for $\alpha$:

$$\begin{pmatrix} 1 & 0 & 0 & 0 & 0 & 1 & 0 & 0 & 0 & 0 \\ 0 & 1 & 0 & 0 & 0 & 0 & 1 & 0 & 0 & 0 \\ 0 & 0 & 0 & 1 & 0 & 0 & 0 & 0 & 0 & 1 \\ 1 & 2 & 3 & 3 & 6 & 4 & 2 & 3 & 0 & 0 \end{pmatrix}$$

**3 generation subalgebra** 164
Algebra: $\mathfrak{su}(4) \oplus \mathfrak{su}(8) \oplus \mathfrak{su}(2) \oplus \mathfrak{su}(2)$
$(\overline{\mathbf{4}}, \mathbf{1}, \mathbf{2}, \mathbf{1})$, $(0,0,1,0,0,0,0,0,0,0,0,1,0) \mapsto (L, Q)$
$(\mathbf{1}, \overline{\mathbf{8}}, \mathbf{2}, \mathbf{1})$, $(0,0,0,0,0,0,0,0,0,0,1,1,0) \mapsto (L, L, Q, Q)$

$(\mathbf{4},\mathbf{1},\mathbf{1},\mathbf{2})$, $(1,0,0,0,0,0,0,0,0,0,0,1) \mapsto (D,E,N,U)$
$(\mathbf{1},\mathbf{8},\mathbf{1},\mathbf{2})$, $(0,0,0,1,0,0,0,0,0,0,0,1) \mapsto (D,D,E,E,N,N,U,U)$
Projection matrix for $\alpha$:

$$\begin{pmatrix} 0 & 1 & 0 & 0 & 1 & 0 & 0 & 1 & 0 & 0 & 0 & 0 \\ 1 & 0 & 0 & 1 & 0 & 0 & 1 & 0 & 0 & 0 & 0 & 0 \\ 0 & 0 & 0 & 0 & 0 & 0 & 0 & 0 & 0 & 0 & 1 & 0 \\ -1 & -2 & -3 & -1 & -2 & -3 & -4 & -5 & -6 & -3 & 0 & 3 \end{pmatrix}$$

**3 generation subalgebra** 165
Algebra: $\mathfrak{su}(5) \oplus \mathfrak{so}(10) \oplus \mathfrak{su}(2) \oplus \mathfrak{su}(2)$
$(\mathbf{1},\mathbf{16},\mathbf{1},\mathbf{1})$, $(0,0,0,0,0,0,0,0,1,0,0) \mapsto (D,E,L,N,Q,U)$
$(\overline{\mathbf{5}},\mathbf{1},\mathbf{2},\mathbf{1})$, $(0,0,0,1,0,0,0,0,0,1,0) \mapsto (D,D,L,L)$
$(\mathbf{10},\mathbf{1},\mathbf{1},\mathbf{2})$, $(0,1,0,0,0,0,0,0,0,0,1) \mapsto (E,E,Q,Q,U,U)$
$(\mathbf{1},\mathbf{1},\mathbf{1},\mathbf{1})$, $(0,0,0,0,0,0,0,0,0,0,0) \mapsto (N)$
$(\mathbf{1},\mathbf{1},\mathbf{1},\mathbf{1})$, $(0,0,0,0,0,0,0,0,0,0,0) \mapsto (N)$
Projection matrix for $\alpha$:

$$\begin{pmatrix} 0 & 0 & 1 & 0 & 0 & 0 & 1 & 0 & 0 & 0 & 0 \\ 0 & 0 & 0 & 1 & 0 & 0 & 0 & 0 & 1 & 0 & 0 \\ 1 & 0 & 0 & 0 & 1 & 0 & 0 & 0 & 0 & 0 & 0 \\ 3 & 6 & 4 & 2 & 3 & 6 & 4 & 0 & 2 & 0 & 0 \end{pmatrix}$$

**3 generation subalgebra** 166
Algebra: $\mathfrak{su}(5) \oplus \mathfrak{so}(10) \oplus \mathfrak{su}(2) \oplus \mathfrak{su}(2)$
$(\mathbf{1},\mathbf{16},\mathbf{1},\mathbf{1})$, $(0,0,0,0,0,0,0,0,1,0,0) \mapsto (D,E,L,N,Q,U)$
$(\overline{\mathbf{5}},\mathbf{1},\mathbf{2},\mathbf{1})$, $(0,0,0,1,0,0,0,0,0,1,0) \mapsto (D,D,L,L)$
$(\mathbf{10},\mathbf{1},\mathbf{1},\mathbf{2})$, $(0,1,0,0,0,0,0,0,0,0,1) \mapsto (E,E,Q,Q,U,U)$
$(\mathbf{1},\mathbf{1},\mathbf{1},\mathbf{2})$, $(0,0,0,0,0,0,0,0,0,0,1) \mapsto (N,N)$
Projection matrix for $\alpha$:

$$\begin{pmatrix} 0 & 0 & 1 & 0 & 0 & 0 & 1 & 0 & 0 & 0 & 0 \\ 0 & 0 & 0 & 1 & 0 & 0 & 0 & 0 & 1 & 0 & 0 \\ 1 & 0 & 0 & 0 & 1 & 0 & 0 & 0 & 0 & 0 & 0 \\ 3 & 6 & 4 & 2 & 3 & 6 & 4 & 0 & 2 & 0 & 0 \end{pmatrix}$$

**3 generation subalgebra** 167
Algebra: $\mathfrak{su}(5) \oplus \mathfrak{so}(10) \oplus \mathfrak{su}(2) \oplus \mathfrak{su}(2)$
$(\mathbf{1},\mathbf{16},\mathbf{1},\mathbf{1})$, $(0,0,0,0,0,0,0,0,1,0,0) \mapsto (D,E,L,N,Q,U)$
$(\overline{\mathbf{5}},\mathbf{1},\mathbf{2},\mathbf{1})$, $(0,0,0,1,0,0,0,0,0,1,0) \mapsto (D,D,L,L)$
$(\mathbf{10},\mathbf{1},\mathbf{1},\mathbf{2})$, $(0,1,0,0,0,0,0,0,0,0,1) \mapsto (E,E,Q,Q,U,U)$
$(\mathbf{1},\mathbf{1},\mathbf{2},\mathbf{1})$, $(0,0,0,0,0,0,0,0,0,1,0) \mapsto (N,N)$
Projection matrix for $\alpha$:

$$\begin{pmatrix} 0 & 0 & 1 & 0 & 0 & 0 & 1 & 0 & 0 & 0 & 0 \\ 0 & 0 & 0 & 1 & 0 & 0 & 0 & 0 & 1 & 0 & 0 \\ 1 & 0 & 0 & 0 & 1 & 0 & 0 & 0 & 0 & 0 & 0 \\ 3 & 6 & 4 & 2 & 3 & 6 & 4 & 0 & 2 & 0 & 0 \end{pmatrix}$$

**3 generation subalgebra** 168
Algebra: $\mathfrak{su}(5) \oplus \mathfrak{so}(10) \oplus \mathfrak{su}(2) \oplus \mathfrak{su}(2)$
$(\mathbf{1},\mathbf{16},\mathbf{1},\mathbf{1})$, $(0,0,0,0,0,0,0,0,1,0,0) \mapsto (D,E,L,N,Q,U)$
$(\overline{\mathbf{5}},\mathbf{1},\mathbf{2},\mathbf{1})$, $(0,0,0,1,0,0,0,0,0,1,0) \mapsto (D,D,L,L)$
$(\mathbf{10},\mathbf{1},\mathbf{2},\mathbf{1})$, $(0,1,0,0,0,0,0,0,0,1,0) \mapsto (E,E,Q,Q,U,U)$
$(\mathbf{1},\mathbf{1},\mathbf{1},\mathbf{2})$, $(0,0,0,0,0,0,0,0,0,0,1) \mapsto (N,N)$
Projection matrix for $\alpha$:

$$\begin{pmatrix} 0 & 0 & 1 & 0 & 0 & 0 & 1 & 0 & 0 & 0 & 0 \\ 0 & 0 & 0 & 1 & 0 & 0 & 0 & 0 & 1 & 0 & 0 \\ 1 & 0 & 0 & 0 & 1 & 0 & 0 & 0 & 0 & 0 & 0 \\ 3 & 6 & 4 & 2 & 3 & 6 & 4 & 0 & 2 & 0 & 0 \end{pmatrix}$$

**3 generation subalgebra** 169
Algebra: $\mathfrak{su}(5) \oplus \mathfrak{so}(10) \oplus \mathfrak{su}(2) \oplus \mathfrak{su}(2)$
$(\overline{\mathbf{5}}, \mathbf{1}, \mathbf{1}, \mathbf{1}),\ (0,0,0,1,0,0,0,0,0,0,0) \mapsto (D, L)$
$(\overline{\mathbf{5}}, \mathbf{1}, \mathbf{1}, \mathbf{1}),\ (0,0,0,1,0,0,0,0,0,0,0) \mapsto (D, L)$
$(\mathbf{1}, \mathbf{16}, \mathbf{1}, \mathbf{1}),\ (0,0,0,0,0,0,0,0,1,0,0) \mapsto (D, E, L, N, Q, U)$
$(\mathbf{10}, \mathbf{1}, \mathbf{2}, \mathbf{1}),\ (0,1,0,0,0,0,0,0,0,1,0) \mapsto (E, E, Q, Q, U, U)$
$(\mathbf{1}, \mathbf{1}, \mathbf{1}, \mathbf{2}),\ (0,0,0,0,0,0,0,0,0,0,1) \mapsto (N, N)$
Projection matrix for $\alpha$:

$$\begin{pmatrix} 0 & 0 & 1 & 0 & 0 & 0 & 1 & 0 & 0 & 0 & 0 \\ 0 & 0 & 0 & 1 & 0 & 0 & 0 & 0 & 1 & 0 & 0 \\ 1 & 0 & 0 & 0 & 1 & 0 & 0 & 0 & 0 & 0 & 0 \\ 3 & 6 & 4 & 2 & 3 & 6 & 4 & 0 & 2 & 0 & 0 \end{pmatrix}$$

**3 generation subalgebra** 170
Algebra: $\mathfrak{su}(5) \oplus \mathfrak{so}(10) \oplus \mathfrak{su}(2) \oplus \mathfrak{su}(2)$
$(\mathbf{10}, \mathbf{1}, \mathbf{1}, \mathbf{1}),\ (0,1,0,0,0,0,0,0,0,0,0) \mapsto (E, Q, U)$
$(\mathbf{10}, \mathbf{1}, \mathbf{1}, \mathbf{1}),\ (0,1,0,0,0,0,0,0,0,0,0) \mapsto (E, Q, U)$
$(\mathbf{1}, \mathbf{16}, \mathbf{1}, \mathbf{1}),\ (0,0,0,0,0,0,0,0,1,0,0) \mapsto (D, E, L, N, Q, U)$
$(\overline{\mathbf{5}}, \mathbf{1}, \mathbf{2}, \mathbf{1}),\ (0,0,0,1,0,0,0,0,0,1,0) \mapsto (D, D, L, L)$
$(\mathbf{1}, \mathbf{1}, \mathbf{1}, \mathbf{2}),\ (0,0,0,0,0,0,0,0,0,0,1) \mapsto (N, N)$
Projection matrix for $\alpha$:

$$\begin{pmatrix} 0 & 0 & 1 & 0 & 0 & 0 & 1 & 0 & 0 & 0 & 0 \\ 0 & 0 & 0 & 1 & 0 & 0 & 0 & 0 & 1 & 0 & 0 \\ 1 & 0 & 0 & 0 & 1 & 0 & 0 & 0 & 0 & 0 & 0 \\ 3 & 6 & 4 & 2 & 3 & 6 & 4 & 0 & 2 & 0 & 0 \end{pmatrix}$$

**3 generation subalgebra** 171
Algebra: $\mathfrak{su}(5) \oplus \mathfrak{su}(2) \oplus \mathfrak{su}(2) \oplus \mathfrak{su}(2)$
$(\overline{\mathbf{5}}, \mathbf{1}, \mathbf{1}, \mathbf{1}),\ (0,0,0,1,0,0,0) \mapsto (D, L)$
$(\mathbf{10}, \mathbf{1}, \mathbf{1}, \mathbf{1}),\ (0,1,0,0,0,0,0) \mapsto (E, Q, U)$
$(\overline{\mathbf{5}}, \mathbf{2}, \mathbf{1}, \mathbf{1}),\ (0,0,0,1,1,0,0) \mapsto (D, D, L, L)$
$(\mathbf{10}, \mathbf{1}, \mathbf{2}, \mathbf{1}),\ (0,1,0,0,0,1,0) \mapsto (E, E, Q, Q, U, U)$
$(\mathbf{1}, \mathbf{1}, \mathbf{1}, \mathbf{2}),\ (0,0,0,0,0,0,1) \mapsto (N, N)$
$(\mathbf{1}, \mathbf{1}, \mathbf{1}, \mathbf{1}),\ (0,0,0,0,0,0,0) \mapsto (N)$
Projection matrix for $\alpha$:

$$\begin{pmatrix} 0 & 0 & 1 & 0 & 0 & 0 & 0 \\ 0 & 0 & 0 & 1 & 0 & 0 & 0 \\ 1 & 0 & 0 & 0 & 0 & 0 & 0 \\ 3 & 6 & 4 & 2 & 0 & 0 & 0 \end{pmatrix}$$

**3 generation subalgebra** 172
Algebra: $\mathfrak{su}(5) \oplus \mathfrak{su}(2) \oplus \mathfrak{su}(2) \oplus \mathfrak{su}(2)$
$(\overline{\mathbf{5}}, \mathbf{1}, \mathbf{1}, \mathbf{1}),\ (0,0,0,1,0,0,0) \mapsto (D, L)$
$(\mathbf{10}, \mathbf{1}, \mathbf{1}, \mathbf{1}),\ (0,1,0,0,0,0,0) \mapsto (E, Q, U)$
$(\overline{\mathbf{5}}, \mathbf{2}, \mathbf{1}, \mathbf{1}),\ (0,0,0,1,1,0,0) \mapsto (D, D, L, L)$
$(\mathbf{10}, \mathbf{1}, \mathbf{2}, \mathbf{1}),\ (0,1,0,0,0,1,0) \mapsto (E, E, Q, Q, U, U)$
$(\mathbf{1}, \mathbf{1}, \mathbf{1}, \mathbf{3}),\ (0,0,0,0,0,0,2) \mapsto (N, N, N)$
Projection matrix for $\alpha$:

$$\begin{pmatrix} 0 & 0 & 1 & 0 & 0 & 0 & 0 \\ 0 & 0 & 0 & 1 & 0 & 0 & 0 \\ 1 & 0 & 0 & 0 & 0 & 0 & 0 \\ 3 & 6 & 4 & 2 & 0 & 0 & 0 \end{pmatrix}$$

**3 generation subalgebra** 173
Algebra: $\mathfrak{su}(5) \oplus \mathfrak{su}(5) \oplus \mathfrak{su}(2) \oplus \mathfrak{su}(2)$
$(\mathbf{1}, \overline{\mathbf{5}}, \mathbf{1}, \mathbf{1}),\ (0,0,0,0,0,0,0,1,0,0) \mapsto (D, L)$

$(\mathbf{1}, \mathbf{10}, \mathbf{1}, \mathbf{1})$, $(0,0,0,0,0,1,0,0,0,0) \mapsto (E, Q, U)$
$(\overline{\mathbf{5}}, \mathbf{1}, \mathbf{2}, \mathbf{1})$, $(0,0,0,1,0,0,0,0,1,0) \mapsto (D, D, L, L)$
$(\mathbf{10}, \mathbf{1}, \mathbf{1}, \mathbf{2})$, $(0,1,0,0,0,0,0,0,0,1) \mapsto (E, E, Q, Q, U, U)$
$(\mathbf{1}, \mathbf{1}, \mathbf{1}, \mathbf{1})$, $(0,0,0,0,0,0,0,0,0,0) \mapsto (N)$
$(\mathbf{1}, \mathbf{1}, \mathbf{1}, \mathbf{1})$, $(0,0,0,0,0,0,0,0,0,0) \mapsto (N)$
$(\mathbf{1}, \mathbf{1}, \mathbf{1}, \mathbf{1})$, $(0,0,0,0,0,0,0,0,0,0) \mapsto (N)$
Projection matrix for $\alpha$:

$$\begin{pmatrix} 0&0&1&0&0&0&1&0&0&0\\ 0&0&0&1&0&0&0&1&0&0\\ 1&0&0&0&1&0&0&0&0&0\\ 3&6&4&2&3&6&4&2&0&0 \end{pmatrix}$$

**3 generation subalgebra** 174
Algebra: $\mathfrak{su}(5) \oplus \mathfrak{su}(5) \oplus \mathfrak{su}(2) \oplus \mathfrak{su}(2)$
$(\mathbf{1}, \overline{\mathbf{5}}, \mathbf{1}, \mathbf{1})$, $(0,0,0,0,0,0,0,1,0,0) \mapsto (D, L)$
$(\mathbf{1}, \mathbf{10}, \mathbf{1}, \mathbf{1})$, $(0,0,0,0,0,1,0,0,0,0) \mapsto (E, Q, U)$
$(\overline{\mathbf{5}}, \mathbf{1}, \mathbf{2}, \mathbf{1})$, $(0,0,0,1,0,0,0,0,1,0) \mapsto (D, D, L, L)$
$(\mathbf{10}, \mathbf{1}, \mathbf{1}, \mathbf{2})$, $(0,1,0,0,0,0,0,0,0,1) \mapsto (E, E, Q, Q, U, U)$
$(\mathbf{1}, \mathbf{1}, \mathbf{1}, \mathbf{2})$, $(0,0,0,0,0,0,0,0,0,1) \mapsto (N, N)$
$(\mathbf{1}, \mathbf{1}, \mathbf{1}, \mathbf{1})$, $(0,0,0,0,0,0,0,0,0,0) \mapsto (N)$
Projection matrix for $\alpha$:

$$\begin{pmatrix} 0&0&1&0&0&0&1&0&0&0\\ 0&0&0&1&0&0&0&1&0&0\\ 1&0&0&0&1&0&0&0&0&0\\ 3&6&4&2&3&6&4&2&0&0 \end{pmatrix}$$

**3 generation subalgebra** 175
Algebra: $\mathfrak{su}(5) \oplus \mathfrak{su}(5) \oplus \mathfrak{su}(2) \oplus \mathfrak{su}(2)$
$(\mathbf{1}, \overline{\mathbf{5}}, \mathbf{1}, \mathbf{1})$, $(0,0,0,0,0,0,0,1,0,0) \mapsto (D, L)$
$(\mathbf{1}, \mathbf{10}, \mathbf{1}, \mathbf{1})$, $(0,0,0,0,0,1,0,0,0,0) \mapsto (E, Q, U)$
$(\overline{\mathbf{5}}, \mathbf{1}, \mathbf{2}, \mathbf{1})$, $(0,0,0,1,0,0,0,0,1,0) \mapsto (D, D, L, L)$
$(\mathbf{10}, \mathbf{1}, \mathbf{1}, \mathbf{2})$, $(0,1,0,0,0,0,0,0,0,1) \mapsto (E, E, Q, Q, U, U)$
$(\mathbf{1}, \mathbf{1}, \mathbf{1}, \mathbf{3})$, $(0,0,0,0,0,0,0,0,0,2) \mapsto (N, N, N)$
Projection matrix for $\alpha$:

$$\begin{pmatrix} 0&0&1&0&0&0&1&0&0&0\\ 0&0&0&1&0&0&0&1&0&0\\ 1&0&0&0&1&0&0&0&0&0\\ 3&6&4&2&3&6&4&2&0&0 \end{pmatrix}$$

**3 generation subalgebra** 176
Algebra: $\mathfrak{su}(5) \oplus \mathfrak{su}(5) \oplus \mathfrak{su}(2) \oplus \mathfrak{su}(2)$
$(\mathbf{1}, \overline{\mathbf{5}}, \mathbf{1}, \mathbf{1})$, $(0,0,0,0,0,0,0,1,0,0) \mapsto (D, L)$
$(\mathbf{1}, \mathbf{10}, \mathbf{1}, \mathbf{1})$, $(0,0,0,0,0,1,0,0,0,0) \mapsto (E, Q, U)$
$(\overline{\mathbf{5}}, \mathbf{1}, \mathbf{2}, \mathbf{1})$, $(0,0,0,1,0,0,0,0,1,0) \mapsto (D, D, L, L)$
$(\mathbf{10}, \mathbf{1}, \mathbf{1}, \mathbf{2})$, $(0,1,0,0,0,0,0,0,0,1) \mapsto (E, E, Q, Q, U, U)$
$(\mathbf{1}, \mathbf{1}, \mathbf{2}, \mathbf{1})$, $(0,0,0,0,0,0,0,0,1,0) \mapsto (N, N)$
$(\mathbf{1}, \mathbf{1}, \mathbf{1}, \mathbf{1})$, $(0,0,0,0,0,0,0,0,0,0) \mapsto (N)$
Projection matrix for $\alpha$:

$$\begin{pmatrix} 0&0&1&0&0&0&1&0&0&0\\ 0&0&0&1&0&0&0&1&0&0\\ 1&0&0&0&1&0&0&0&0&0\\ 3&6&4&2&3&6&4&2&0&0 \end{pmatrix}$$

**3 generation subalgebra** 177
Algebra: $\mathfrak{su}(5) \oplus \mathfrak{su}(5) \oplus \mathfrak{su}(2) \oplus \mathfrak{su}(2)$
$(\mathbf{1}, \overline{\mathbf{5}}, \mathbf{1}, \mathbf{1})$, $(0,0,0,0,0,0,0,1,0,0) \mapsto (D, L)$

$(\mathbf{1},\mathbf{10},\mathbf{1},\mathbf{1}),\ (0,0,0,0,0,1,0,0,0,0) \mapsto (E,Q,U)$
$(\overline{\mathbf{5}},\mathbf{1},\mathbf{2},\mathbf{1}),\ (0,0,0,1,0,0,0,0,1,0) \mapsto (D,D,L,L)$
$(\mathbf{10},\mathbf{1},\mathbf{1},\mathbf{2}),\ (0,1,0,0,0,0,0,0,0,1) \mapsto (E,E,Q,Q,U,U)$
$(\mathbf{1},\mathbf{1},\mathbf{3},\mathbf{1}),\ (0,0,0,0,0,0,0,0,2,0) \mapsto (N,N,N)$
Projection matrix for $\alpha$:

$$\begin{pmatrix} 0 & 0 & 1 & 0 & 0 & 0 & 1 & 0 & 0 & 0 \\ 0 & 0 & 0 & 1 & 0 & 0 & 0 & 1 & 0 & 0 \\ 1 & 0 & 0 & 0 & 1 & 0 & 0 & 0 & 0 & 0 \\ 3 & 6 & 4 & 2 & 3 & 6 & 4 & 2 & 0 & 0 \end{pmatrix}$$

**3 generation subalgebra** 178
Algebra: $\mathfrak{su}(5) \oplus \mathfrak{su}(5) \oplus \mathfrak{su}(2) \oplus \mathfrak{su}(2)$
$(\mathbf{1},\overline{\mathbf{5}},\mathbf{1},\mathbf{1}),\ (0,0,0,0,0,0,0,1,0,0) \mapsto (D,L)$
$(\mathbf{1},\mathbf{10},\mathbf{1},\mathbf{1}),\ (0,0,0,0,0,1,0,0,0,0) \mapsto (E,Q,U)$
$(\overline{\mathbf{5}},\mathbf{1},\mathbf{2},\mathbf{1}),\ (0,0,0,1,0,0,0,0,1,0) \mapsto (D,D,L,L)$
$(\mathbf{10},\mathbf{1},\mathbf{2},\mathbf{1}),\ (0,1,0,0,0,0,0,0,1,0) \mapsto (E,E,Q,Q,U,U)$
$(\mathbf{1},\mathbf{1},\mathbf{1},\mathbf{2}),\ (0,0,0,0,0,0,0,0,0,1) \mapsto (N,N)$
$(\mathbf{1},\mathbf{1},\mathbf{1},\mathbf{1}),\ (0,0,0,0,0,0,0,0,0,0) \mapsto (N)$
Projection matrix for $\alpha$:

$$\begin{pmatrix} 0 & 0 & 1 & 0 & 0 & 0 & 1 & 0 & 0 & 0 \\ 0 & 0 & 0 & 1 & 0 & 0 & 0 & 1 & 0 & 0 \\ 1 & 0 & 0 & 0 & 1 & 0 & 0 & 0 & 0 & 0 \\ 3 & 6 & 4 & 2 & 3 & 6 & 4 & 2 & 0 & 0 \end{pmatrix}$$

**3 generation subalgebra** 179
Algebra: $\mathfrak{su}(5) \oplus \mathfrak{su}(5) \oplus \mathfrak{su}(2) \oplus \mathfrak{su}(2)$
$(\mathbf{1},\overline{\mathbf{5}},\mathbf{1},\mathbf{1}),\ (0,0,0,0,0,0,0,1,0,0) \mapsto (D,L)$
$(\mathbf{1},\mathbf{10},\mathbf{1},\mathbf{1}),\ (0,0,0,0,0,1,0,0,0,0) \mapsto (E,Q,U)$
$(\overline{\mathbf{5}},\mathbf{1},\mathbf{2},\mathbf{1}),\ (0,0,0,1,0,0,0,0,1,0) \mapsto (D,D,L,L)$
$(\mathbf{10},\mathbf{1},\mathbf{2},\mathbf{1}),\ (0,1,0,0,0,0,0,0,1,0) \mapsto (E,E,Q,Q,U,U)$
$(\mathbf{1},\mathbf{1},\mathbf{1},\mathbf{3}),\ (0,0,0,0,0,0,0,0,0,2) \mapsto (N,N,N)$
Projection matrix for $\alpha$:

$$\begin{pmatrix} 0 & 0 & 1 & 0 & 0 & 0 & 1 & 0 & 0 & 0 \\ 0 & 0 & 0 & 1 & 0 & 0 & 0 & 1 & 0 & 0 \\ 1 & 0 & 0 & 0 & 1 & 0 & 0 & 0 & 0 & 0 \\ 3 & 6 & 4 & 2 & 3 & 6 & 4 & 2 & 0 & 0 \end{pmatrix}$$

**3 generation subalgebra** 180
Algebra: $\mathfrak{su}(5) \oplus \mathfrak{su}(5) \oplus \mathfrak{su}(2) \oplus \mathfrak{su}(2)$
$(\overline{\mathbf{5}},\mathbf{1},\mathbf{1},\mathbf{1}),\ (0,0,0,1,0,0,0,0,0,0) \mapsto (D,L)$
$(\overline{\mathbf{5}},\mathbf{1},\mathbf{1},\mathbf{1}),\ (0,0,0,1,0,0,0,0,0,0) \mapsto (D,L)$
$(\mathbf{1},\overline{\mathbf{5}},\mathbf{1},\mathbf{1}),\ (0,0,0,0,0,0,0,1,0,0) \mapsto (D,L)$
$(\mathbf{1},\mathbf{10},\mathbf{1},\mathbf{1}),\ (0,0,0,0,0,1,0,0,0,0) \mapsto (E,Q,U)$
$(\mathbf{10},\mathbf{1},\mathbf{2},\mathbf{1}),\ (0,1,0,0,0,0,0,0,1,0) \mapsto (E,E,Q,Q,U,U)$
$(\mathbf{1},\mathbf{1},\mathbf{1},\mathbf{2}),\ (0,0,0,0,0,0,0,0,0,1) \mapsto (N,N)$
$(\mathbf{1},\mathbf{1},\mathbf{1},\mathbf{1}),\ (0,0,0,0,0,0,0,0,0,0) \mapsto (N)$
Projection matrix for $\alpha$:

$$\begin{pmatrix} 0 & 0 & 1 & 0 & 0 & 0 & 1 & 0 & 0 & 0 \\ 0 & 0 & 0 & 1 & 0 & 0 & 0 & 1 & 0 & 0 \\ 1 & 0 & 0 & 0 & 1 & 0 & 0 & 0 & 0 & 0 \\ 3 & 6 & 4 & 2 & 3 & 6 & 4 & 2 & 0 & 0 \end{pmatrix}$$

**3 generation subalgebra** 181
Algebra: $\mathfrak{su}(5) \oplus \mathfrak{su}(5) \oplus \mathfrak{su}(2) \oplus \mathfrak{su}(2)$
$(\overline{\mathbf{5}},\mathbf{1},\mathbf{1},\mathbf{1}),\ (0,0,0,1,0,0,0,0,0,0) \mapsto (D,L)$
$(\overline{\mathbf{5}},\mathbf{1},\mathbf{1},\mathbf{1}),\ (0,0,0,1,0,0,0,0,0,0) \mapsto (D,L)$

$(\mathbf{1},\overline{\mathbf{5}},\mathbf{1},\mathbf{1})$, $(0,0,0,0,0,0,0,1,0,0) \mapsto (D,L)$
$(\mathbf{1},\mathbf{10},\mathbf{1},\mathbf{1})$, $(0,0,0,0,0,1,0,0,0,0) \mapsto (E,Q,U)$
$(\mathbf{10},\mathbf{1},\mathbf{2},\mathbf{1})$, $(0,1,0,0,0,0,0,0,1,0) \mapsto (E,E,Q,Q,U,U)$
$(\mathbf{1},\mathbf{1},\mathbf{1},\mathbf{3})$, $(0,0,0,0,0,0,0,0,0,2) \mapsto (N,N,N)$
Projection matrix for $\alpha$:

$$\begin{pmatrix} 0&0&1&0&0&0&1&0&0&0\\ 0&0&0&1&0&0&0&1&0&0\\ 1&0&0&0&1&0&0&0&0&0\\ 3&6&4&2&3&6&4&2&0&0 \end{pmatrix}$$

**3 generation subalgebra** 182
Algebra: $\mathfrak{su}(5)\oplus\mathfrak{su}(5)\oplus\mathfrak{su}(2)\oplus\mathfrak{su}(2)$
$(\mathbf{10},\mathbf{1},\mathbf{1},\mathbf{1})$, $(0,1,0,0,0,0,0,0,0,0) \mapsto (E,Q,U)$
$(\mathbf{10},\mathbf{1},\mathbf{1},\mathbf{1})$, $(0,1,0,0,0,0,0,0,0,0) \mapsto (E,Q,U)$
$(\mathbf{1},\overline{\mathbf{5}},\mathbf{1},\mathbf{1})$, $(0,0,0,0,0,0,0,1,0,0) \mapsto (D,L)$
$(\mathbf{1},\mathbf{10},\mathbf{1},\mathbf{1})$, $(0,0,0,0,0,1,0,0,0,0) \mapsto (E,Q,U)$
$(\overline{\mathbf{5}},\mathbf{1},\mathbf{2},\mathbf{1})$, $(0,0,0,1,0,0,0,0,1,0) \mapsto (D,D,L,L)$
$(\mathbf{1},\mathbf{1},\mathbf{1},\mathbf{2})$, $(0,0,0,0,0,0,0,0,0,1) \mapsto (N,N)$
$(\mathbf{1},\mathbf{1},\mathbf{1},\mathbf{1})$, $(0,0,0,0,0,0,0,0,0,0) \mapsto (N)$
Projection matrix for $\alpha$:

$$\begin{pmatrix} 0&0&1&0&0&0&1&0&0&0\\ 0&0&0&1&0&0&0&1&0&0\\ 1&0&0&0&1&0&0&0&0&0\\ 3&6&4&2&3&6&4&2&0&0 \end{pmatrix}$$

**3 generation subalgebra** 183
Algebra: $\mathfrak{su}(5)\oplus\mathfrak{su}(5)\oplus\mathfrak{su}(2)\oplus\mathfrak{su}(2)$
$(\mathbf{10},\mathbf{1},\mathbf{1},\mathbf{1})$, $(0,1,0,0,0,0,0,0,0,0) \mapsto (E,Q,U)$
$(\mathbf{10},\mathbf{1},\mathbf{1},\mathbf{1})$, $(0,1,0,0,0,0,0,0,0,0) \mapsto (E,Q,U)$
$(\mathbf{1},\overline{\mathbf{5}},\mathbf{1},\mathbf{1})$, $(0,0,0,0,0,0,0,1,0,0) \mapsto (D,L)$
$(\mathbf{1},\mathbf{10},\mathbf{1},\mathbf{1})$, $(0,0,0,0,0,1,0,0,0,0) \mapsto (E,Q,U)$
$(\overline{\mathbf{5}},\mathbf{1},\mathbf{2},\mathbf{1})$, $(0,0,0,1,0,0,0,0,1,0) \mapsto (D,D,L,L)$
$(\mathbf{1},\mathbf{1},\mathbf{1},\mathbf{3})$, $(0,0,0,0,0,0,0,0,0,2) \mapsto (N,N,N)$
Projection matrix for $\alpha$:

$$\begin{pmatrix} 0&0&1&0&0&0&1&0&0&0\\ 0&0&0&1&0&0&0&1&0&0\\ 1&0&0&0&1&0&0&0&0&0\\ 3&6&4&2&3&6&4&2&0&0 \end{pmatrix}$$

**3 generation subalgebra** 184
Algebra: $\mathfrak{su}(5)\oplus\mathfrak{su}(5)\oplus\mathfrak{su}(5)\oplus\mathfrak{su}(2)$
$(\overline{\mathbf{5}},\mathbf{1},\mathbf{1},\mathbf{1})$, $(0,0,0,1,0,0,0,0,0,0,0,0,0) \mapsto (D,L)$
$(\mathbf{10},\mathbf{1},\mathbf{1},\mathbf{1})$, $(0,1,0,0,0,0,0,0,0,0,0,0,0) \mapsto (E,Q,U)$
$(\mathbf{1},\overline{\mathbf{5}},\mathbf{1},\mathbf{1})$, $(0,0,0,0,0,0,0,1,0,0,0,0,0) \mapsto (D,L)$
$(\mathbf{1},\mathbf{10},\mathbf{1},\mathbf{1})$, $(0,0,0,0,0,1,0,0,0,0,0,0,0) \mapsto (E,Q,U)$
$(\mathbf{1},\mathbf{1},\overline{\mathbf{5}},\mathbf{1})$, $(0,0,0,0,0,0,0,0,0,0,0,1,0) \mapsto (D,L)$
$(\mathbf{1},\mathbf{1},\mathbf{10},\mathbf{1})$, $(0,0,0,0,0,0,0,0,0,1,0,0,0) \mapsto (E,Q,U)$
$(\mathbf{1},\mathbf{1},\mathbf{1},\mathbf{2})$, $(0,0,0,0,0,0,0,0,0,0,0,0,1) \mapsto (N,N)$
$(\mathbf{1},\mathbf{1},\mathbf{1},\mathbf{1})$, $(0,0,0,0,0,0,0,0,0,0,0,0,0) \mapsto (N)$
Projection matrix for $\alpha$:

$$\begin{pmatrix} 0&0&1&0&0&0&1&0&0&0&1&0&0\\ 0&0&0&1&0&0&0&1&0&0&0&1&0\\ 1&0&0&0&1&0&0&0&1&0&0&0&0\\ 3&6&4&2&3&6&4&2&3&6&4&2&0 \end{pmatrix}$$

**3 generation subalgebra** 185
Algebra: $\mathfrak{su}(5)\oplus\mathfrak{su}(8)\oplus\mathfrak{su}(2)\oplus\mathfrak{su}(2)$

$(\overline{\mathbf{5}}, \mathbf{1}, \mathbf{1}, \mathbf{1})$, $(0, 0, 0, 1, 0, 0, 0, 0, 0, 0, 0, 0, 0) \mapsto (D, L)$
$(\mathbf{10}, \mathbf{1}, \mathbf{1}, \mathbf{1})$, $(0, 1, 0, 0, 0, 0, 0, 0, 0, 0, 0, 0, 0) \mapsto (E, Q, U)$
$(\mathbf{1}, \overline{\mathbf{8}}, \mathbf{2}, \mathbf{1})$, $(0, 0, 0, 0, 0, 0, 0, 0, 0, 0, 1, 1, 0) \mapsto (L, L, Q, Q)$
$(\mathbf{1}, \mathbf{8}, \mathbf{1}, \mathbf{2})$, $(0, 0, 0, 0, 1, 0, 0, 0, 0, 0, 0, 0, 1) \mapsto (D, D, E, E, N, N, U, U)$
$(\mathbf{1}, \mathbf{1}, \mathbf{1}, \mathbf{1})$, $(0, 0, 0, 0, 0, 0, 0, 0, 0, 0, 0, 0, 0) \mapsto (N)$
Projection matrix for $\alpha$:

$$\begin{pmatrix} 0 & 0 & 1 & 0 & 0 & 1 & 0 & 0 & 1 & 0 & 0 & 0 & 0 \\ 0 & 0 & 0 & 1 & 1 & 0 & 0 & 1 & 0 & 0 & 0 & 0 & 0 \\ 1 & 0 & 0 & 0 & 0 & 0 & 0 & 0 & 0 & 0 & 0 & 1 & 0 \\ 3 & 6 & 4 & 2 & -1 & -2 & -3 & -4 & -5 & -6 & -3 & 0 & 3 \end{pmatrix}$$

**3 generation subalgebra** 186
Algebra: $\mathfrak{su}(4) \oplus \mathfrak{so}(10) \oplus \mathfrak{so}(10) \oplus \mathfrak{su}(2) \oplus \mathfrak{su}(2)$
$(\mathbf{1}, \mathbf{16}, \mathbf{1}, \mathbf{1}, \mathbf{1})$, $(0, 0, 0, 0, 0, 0, 0, 1, 0, 0, 0, 0, 0, 0, 0, 0) \mapsto (D, E, L, N, Q, U)$
$(\mathbf{1}, \mathbf{1}, \mathbf{16}, \mathbf{1}, \mathbf{1})$, $(0, 0, 0, 0, 0, 0, 0, 0, 0, 0, 0, 0, 1, 0, 0, 0) \mapsto (D, E, L, N, Q, U)$
$(\overline{\mathbf{4}}, \mathbf{1}, \mathbf{1}, \mathbf{2}, \mathbf{1})$, $(0, 0, 1, 0, 0, 0, 0, 0, 0, 0, 0, 0, 0, 0, 1, 0) \mapsto (L, Q)$
$(\mathbf{4}, \mathbf{1}, \mathbf{1}, \mathbf{1}, \mathbf{2})$, $(1, 0, 0, 0, 0, 0, 0, 0, 0, 0, 0, 0, 0, 0, 0, 1) \mapsto (D, E, N, U)$
Projection matrix for $\alpha$:

$$\begin{pmatrix} 0 & 1 & 0 & 0 & 0 & 1 & 0 & 0 & 0 & 0 & 1 & 0 & 0 & 0 & 0 \\ 1 & 0 & 0 & 0 & 0 & 0 & 0 & 1 & 0 & 0 & 0 & 0 & 1 & 0 & 0 \\ 0 & 0 & 0 & 1 & 0 & 0 & 0 & 0 & 1 & 0 & 0 & 0 & 0 & 1 & 0 \\ -1 & -2 & -3 & 3 & 6 & 4 & 0 & 2 & 3 & 6 & 4 & 0 & 2 & 0 & 3 \end{pmatrix}$$

**3 generation subalgebra** 187
Algebra: $\mathfrak{su}(4) \oplus \mathfrak{so}(10) \oplus \mathfrak{su}(2) \oplus \mathfrak{su}(2) \oplus \mathfrak{su}(2)$
$(\mathbf{1}, \mathbf{16}, \mathbf{1}, \mathbf{1}, \mathbf{1})$, $(0, 0, 0, 0, 0, 0, 0, 1, 0, 0, 0) \mapsto (D, E, L, N, Q, U)$
$(\mathbf{4}, \mathbf{1}, \mathbf{2}, \mathbf{2}, \mathbf{1})$, $(1, 0, 0, 0, 0, 0, 0, 0, 1, 1, 0) \mapsto (L, L, Q, Q)$
$(\overline{\mathbf{4}}, \mathbf{1}, \mathbf{2}, \mathbf{1}, \mathbf{2})$, $(0, 0, 1, 0, 0, 0, 0, 0, 1, 0, 1) \mapsto (D, D, E, E, N, N, U, U)$
Projection matrix for $\alpha$:

$$\begin{pmatrix} 1 & 0 & 0 & 0 & 0 & 1 & 0 & 0 & 0 & 0 & 0 \\ 0 & 1 & 0 & 0 & 0 & 0 & 0 & 1 & 0 & 0 & 0 \\ 0 & 0 & 0 & 1 & 0 & 0 & 0 & 0 & 0 & 1 & 0 \\ 1 & 2 & 3 & 3 & 6 & 4 & 0 & 2 & 0 & 0 & 3 \end{pmatrix}$$

**3 generation subalgebra** 188
Algebra: $\mathfrak{su}(4) \oplus \mathfrak{so}(10) \oplus \mathfrak{su}(2) \oplus \mathfrak{su}(2) \oplus \mathfrak{su}(2)$
$(\overline{\mathbf{4}}, \mathbf{1}, \mathbf{2}, \mathbf{1}, \mathbf{1})$, $(0, 0, 1, 0, 0, 0, 0, 0, 1, 0, 0) \mapsto (L, Q)$
$(\mathbf{4}, \mathbf{1}, \mathbf{1}, \mathbf{2}, \mathbf{1})$, $(1, 0, 0, 0, 0, 0, 0, 0, 0, 1, 0) \mapsto (D, E, N, U)$
$(\mathbf{1}, \mathbf{16}, \mathbf{1}, \mathbf{1}, \mathbf{2})$, $(0, 0, 0, 0, 0, 0, 0, 1, 0, 0, 1) \mapsto (D, D, E, E, L, L, N, N, Q, Q, U, U)$
Projection matrix for $\alpha$:

$$\begin{pmatrix} 0 & 1 & 0 & 0 & 0 & 1 & 0 & 0 & 0 & 0 & 0 \\ 1 & 0 & 0 & 0 & 0 & 0 & 0 & 1 & 0 & 0 & 0 \\ 0 & 0 & 0 & 1 & 0 & 0 & 0 & 0 & 1 & 0 & 0 \\ -1 & -2 & -3 & 3 & 6 & 4 & 0 & 2 & 0 & 3 & 0 \end{pmatrix}$$

**3 generation subalgebra** 189
Algebra: $\mathfrak{su}(4) \oplus \mathfrak{so}(10) \oplus \mathfrak{su}(2) \oplus \mathfrak{su}(2) \oplus \mathfrak{su}(2)$
$(\mathbf{1}, \mathbf{16}, \mathbf{1}, \mathbf{1}, \mathbf{1})$, $(0, 0, 0, 0, 0, 0, 0, 1, 0, 0, 0) \mapsto (D, E, L, N, Q, U)$
$(\mathbf{4}, \mathbf{1}, \mathbf{2}, \mathbf{2}, \mathbf{1})$, $(1, 0, 0, 0, 0, 0, 0, 0, 1, 1, 0) \mapsto (D, D, E, E, N, N, U, U)$
$(\overline{\mathbf{4}}, \mathbf{1}, \mathbf{1}, \mathbf{1}, \mathbf{2})$, $(0, 0, 1, 0, 0, 0, 0, 0, 0, 0, 1) \mapsto (L, Q)$
$(\overline{\mathbf{4}}, \mathbf{1}, \mathbf{1}, \mathbf{1}, \mathbf{2})$, $(0, 0, 1, 0, 0, 0, 0, 0, 0, 0, 1) \mapsto (L, Q)$
Projection matrix for $\alpha$:

$$\begin{pmatrix} 0 & 1 & 0 & 0 & 0 & 1 & 0 & 0 & 0 & 0 & 0 \\ 1 & 0 & 0 & 0 & 0 & 0 & 0 & 1 & 0 & 0 & 0 \\ 0 & 0 & 0 & 1 & 0 & 0 & 0 & 0 & 0 & 0 & 1 \\ -1 & -2 & -3 & 3 & 6 & 4 & 0 & 2 & 3 & 0 & 0 \end{pmatrix}$$

**3 generation subalgebra** 190
Algebra: $\mathfrak{su}(4) \oplus \mathfrak{so}(10) \oplus \mathfrak{su}(2) \oplus \mathfrak{su}(2) \oplus \mathfrak{su}(2)$
$(\mathbf{1}, \mathbf{16}, \mathbf{1}, \mathbf{1}, \mathbf{1})$, $(0,0,0,0,0,0,0,1,0,0,0) \mapsto (D,E,L,N,Q,U)$
$(\mathbf{4}, \mathbf{1}, \mathbf{2}, \mathbf{2}, \mathbf{1})$, $(1,0,0,0,0,0,0,0,1,1,0) \mapsto (L,L,Q,Q)$
$(\overline{\mathbf{4}}, \mathbf{1}, \mathbf{1}, \mathbf{1}, \mathbf{2})$, $(0,0,1,0,0,0,0,0,0,0,1) \mapsto (D,E,N,U)$
$(\overline{\mathbf{4}}, \mathbf{1}, \mathbf{1}, \mathbf{1}, \mathbf{2})$, $(0,0,1,0,0,0,0,0,0,0,1) \mapsto (D,E,N,U)$
Projection matrix for $\alpha$:

$$\begin{pmatrix} 1 & 0 & 0 & 0 & 0 & 1 & 0 & 0 & 0 & 0 & 0 \\ 0 & 1 & 0 & 0 & 0 & 0 & 0 & 1 & 0 & 0 & 0 \\ 0 & 0 & 0 & 1 & 0 & 0 & 0 & 0 & 1 & 0 & 0 \\ 1 & 2 & 3 & 3 & 6 & 4 & 0 & 2 & 0 & 0 & 3 \end{pmatrix}$$

**3 generation subalgebra** 191
Algebra: $\mathfrak{su}(4) \oplus \mathfrak{so}(10) \oplus \mathfrak{su}(2) \oplus \mathfrak{su}(2) \oplus \mathfrak{su}(2)$
$(\mathbf{1}, \mathbf{16}, \mathbf{1}, \mathbf{1}, \mathbf{1})$, $(0,0,0,0,0,0,0,1,0,0,0) \mapsto (D,E,L,N,Q,U)$
$(\overline{\mathbf{4}}, \mathbf{1}, \mathbf{2}, \mathbf{1}, \mathbf{1})$, $(0,0,1,0,0,0,0,0,1,0,0) \mapsto (L,Q)$
$(\overline{\mathbf{4}}, \mathbf{1}, \mathbf{2}, \mathbf{1}, \mathbf{1})$, $(0,0,1,0,0,0,0,0,1,0,0) \mapsto (L,Q)$
$(\mathbf{4}, \mathbf{1}, \mathbf{1}, \mathbf{2}, \mathbf{1})$, $(1,0,0,0,0,0,0,0,0,1,0) \mapsto (D,E,N,U)$
$(\mathbf{4}, \mathbf{1}, \mathbf{1}, \mathbf{1}, \mathbf{2})$, $(1,0,0,0,0,0,0,0,0,0,1) \mapsto (D,E,N,U)$
Projection matrix for $\alpha$:

$$\begin{pmatrix} 0 & 1 & 0 & 0 & 0 & 1 & 0 & 0 & 0 & 0 & 0 \\ 1 & 0 & 0 & 0 & 0 & 0 & 0 & 1 & 0 & 0 & 0 \\ 0 & 0 & 0 & 1 & 0 & 0 & 0 & 0 & 1 & 0 & 0 \\ -1 & -2 & -3 & 3 & 6 & 4 & 0 & 2 & 0 & 3 & 3 \end{pmatrix}$$

**3 generation subalgebra** 192
Algebra: $\mathfrak{su}(4) \oplus \mathfrak{so}(10) \oplus \mathfrak{su}(2) \oplus \mathfrak{su}(2) \oplus \mathfrak{su}(2)$
$(\mathbf{1}, \mathbf{16}, \mathbf{1}, \mathbf{1}, \mathbf{1})$, $(0,0,0,0,0,0,0,1,0,0,0) \mapsto (D,E,L,N,Q,U)$
$(\overline{\mathbf{4}}, \mathbf{1}, \mathbf{2}, \mathbf{1}, \mathbf{1})$, $(0,0,1,0,0,0,0,0,1,0,0) \mapsto (D,E,N,U)$
$(\overline{\mathbf{4}}, \mathbf{1}, \mathbf{2}, \mathbf{1}, \mathbf{1})$, $(0,0,1,0,0,0,0,0,1,0,0) \mapsto (D,E,N,U)$
$(\mathbf{4}, \mathbf{1}, \mathbf{1}, \mathbf{2}, \mathbf{1})$, $(1,0,0,0,0,0,0,0,0,1,0) \mapsto (L,Q)$
$(\mathbf{4}, \mathbf{1}, \mathbf{1}, \mathbf{1}, \mathbf{2})$, $(1,0,0,0,0,0,0,0,0,0,1) \mapsto (L,Q)$
Projection matrix for $\alpha$:

$$\begin{pmatrix} 1 & 0 & 0 & 0 & 0 & 1 & 0 & 0 & 0 & 0 & 0 \\ 0 & 1 & 0 & 0 & 0 & 0 & 0 & 1 & 0 & 0 & 0 \\ 0 & 0 & 0 & 1 & 0 & 0 & 0 & 0 & 0 & 1 & 1 \\ 1 & 2 & 3 & 3 & 6 & 4 & 0 & 2 & 3 & 0 & 0 \end{pmatrix}$$

**3 generation subalgebra** 193
Algebra: $\mathfrak{su}(4) \oplus \mathfrak{sp}(4) \oplus \mathfrak{so}(10) \oplus \mathfrak{su}(2) \oplus \mathfrak{su}(2)$
$(\overline{\mathbf{4}}, \mathbf{4}, \mathbf{1}, \mathbf{1}, \mathbf{1})$, $(0,0,1,1,0,0,0,0,0,0,0,0,0) \mapsto (L,L,Q,Q)$
$(\mathbf{1}, \mathbf{1}, \mathbf{16}, \mathbf{1}, \mathbf{1})$, $(0,0,0,0,0,0,0,0,0,1,0,0) \mapsto (D,E,L,N,Q,U)$
$(\mathbf{4}, \mathbf{1}, \mathbf{1}, \mathbf{2}, \mathbf{1})$, $(1,0,0,0,0,0,0,0,0,0,0,1,0) \mapsto (D,E,N,U)$
$(\mathbf{4}, \mathbf{1}, \mathbf{1}, \mathbf{1}, \mathbf{2})$, $(1,0,0,0,0,0,0,0,0,0,0,0,1) \mapsto (D,E,N,U)$
Projection matrix for $\alpha$:

$$\begin{pmatrix} 0 & 1 & 0 & 0 & 0 & 0 & 0 & 1 & 0 & 0 & 0 & 0 \\ 1 & 0 & 0 & 0 & 0 & 0 & 0 & 0 & 0 & 1 & 0 & 0 \\ 0 & 0 & 0 & 1 & 2 & 1 & 0 & 0 & 0 & 0 & 0 & 0 \\ -1 & -2 & -3 & 0 & 0 & 3 & 6 & 4 & 0 & 2 & 3 & 3 \end{pmatrix}$$

**3 generation subalgebra** 194
Algebra: $\mathfrak{su}(4) \oplus \mathfrak{sp}(4) \oplus \mathfrak{so}(10) \oplus \mathfrak{su}(2) \oplus \mathfrak{su}(2)$
$(\overline{\mathbf{4}}, \mathbf{4}, \mathbf{1}, \mathbf{1}, \mathbf{1})$, $(0,0,1,1,0,0,0,0,0,0,0,0,0) \mapsto (D,D,E,E,N,N,U,U)$
$(\mathbf{1}, \mathbf{1}, \mathbf{16}, \mathbf{1}, \mathbf{1})$, $(0,0,0,0,0,0,0,0,0,1,0,0) \mapsto (D,E,L,N,Q,U)$
$(\mathbf{4}, \mathbf{1}, \mathbf{1}, \mathbf{2}, \mathbf{1})$, $(1,0,0,0,0,0,0,0,0,0,0,1,0) \mapsto (L,Q)$

$(\mathbf{4}, \mathbf{1}, \mathbf{1}, \mathbf{1}, \mathbf{2})$, $(1,0,0,0,0,0,0,0,0,0,0,1) \mapsto (L, Q)$
Projection matrix for $\alpha$:

$$\begin{pmatrix} 1&0&0&0&0&0&0&1&0&0&0&0\\ 0&1&0&0&0&0&0&0&0&1&0&0\\ 0&0&0&0&0&1&0&0&0&0&1&1\\ 1&2&3&3&0&3&6&4&0&2&0&0 \end{pmatrix}$$

**3 generation subalgebra** 195
Algebra: $\mathfrak{su}(4) \oplus \mathfrak{sp}(4) \oplus \mathfrak{sp}(4) \oplus \mathfrak{su}(2) \oplus \mathfrak{su}(2)$
$(\overline{\mathbf{4}}, \mathbf{4}, \mathbf{1}, \mathbf{1}, \mathbf{1})$, $(0,0,1,1,0,0,0,0,0) \mapsto (L, L, Q, Q)$
$(\mathbf{4}, \mathbf{1}, \mathbf{4}, \mathbf{1}, \mathbf{1})$, $(1,0,0,0,0,1,0,0,0) \mapsto (D, D, E, E, N, N, U, U)$
$(\overline{\mathbf{4}}, \mathbf{1}, \mathbf{1}, \mathbf{2}, \mathbf{1})$, $(0,0,1,0,0,0,0,1,0) \mapsto (L, Q)$
$(\mathbf{4}, \mathbf{1}, \mathbf{1}, \mathbf{1}, \mathbf{2})$, $(1,0,0,0,0,0,0,0,1) \mapsto (D, E, N, U)$
Projection matrix for $\alpha$:

$$\begin{pmatrix} 0&1&0&0&0&0&0&0&0\\ 1&0&0&0&0&0&0&0&0\\ 0&0&0&1&2&0&0&1&0\\ -1&-2&-3&0&0&3&0&0&3 \end{pmatrix}$$

**3 generation subalgebra** 196
Algebra: $\mathfrak{su}(4) \oplus \mathfrak{sp}(4) \oplus \mathfrak{su}(2) \oplus \mathfrak{su}(2) \oplus \mathfrak{su}(2)$
$(\overline{\mathbf{4}}, \mathbf{4}, \mathbf{1}, \mathbf{1}, \mathbf{1})$, $(0,0,1,1,0,0,0,0) \mapsto (L, L, Q, Q)$
$(\mathbf{4}, \mathbf{1}, \mathbf{3}, \mathbf{2}, \mathbf{1})$, $(1,0,0,0,0,2,1,0) \mapsto (D, D, D, E, E, E, N, N, N, U, U, U)$
$(\overline{\mathbf{4}}, \mathbf{1}, \mathbf{1}, \mathbf{1}, \mathbf{2})$, $(0,0,1,0,0,0,0,1) \mapsto (L, Q)$
Projection matrix for $\alpha$:

$$\begin{pmatrix} 0&1&0&0&0&0&0&0\\ 1&0&0&0&0&0&0&0\\ 0&0&0&1&2&0&0&1\\ -1&-2&-3&0&0&0&3&0 \end{pmatrix}$$

**3 generation subalgebra** 197
Algebra: $\mathfrak{su}(4) \oplus \mathfrak{sp}(4) \oplus \mathfrak{su}(2) \oplus \mathfrak{su}(2) \oplus \mathfrak{su}(2)$
$(\overline{\mathbf{4}}, \mathbf{4}, \mathbf{1}, \mathbf{1}, \mathbf{1})$, $(0,0,1,1,0,0,0,0) \mapsto (D, D, E, E, N, N, U, U)$
$(\mathbf{4}, \mathbf{1}, \mathbf{3}, \mathbf{2}, \mathbf{1})$, $(1,0,0,0,0,2,1,0) \mapsto (L, L, L, Q, Q, Q)$
$(\overline{\mathbf{4}}, \mathbf{1}, \mathbf{1}, \mathbf{1}, \mathbf{2})$, $(0,0,1,0,0,0,0,1) \mapsto (D, E, N, U)$
Projection matrix for $\alpha$:

$$\begin{pmatrix} 1&0&0&0&0&0&0&0\\ 0&1&0&0&0&0&0&0\\ 0&0&0&0&0&0&1&0\\ 1&2&3&3&0&0&0&3 \end{pmatrix}$$

**3 generation subalgebra** 198
Algebra: $\mathfrak{su}(4) \oplus \mathfrak{sp}(4) \oplus \mathfrak{su}(2) \oplus \mathfrak{su}(2) \oplus \mathfrak{su}(2)$
$(\overline{\mathbf{4}}, \mathbf{4}, \mathbf{1}, \mathbf{1}, \mathbf{1})$, $(0,0,1,1,0,0,0,0) \mapsto (L, L, Q, Q)$
$(\mathbf{4}, \mathbf{1}, \mathbf{2}, \mathbf{2}, \mathbf{1})$, $(1,0,0,0,0,1,1,0) \mapsto (D, D, E, E, N, N, U, U)$
$(\mathbf{4}, \mathbf{1}, \mathbf{2}, \mathbf{1}, \mathbf{1})$, $(1,0,0,0,0,1,0,0) \mapsto (D, E, N, U)$
$(\overline{\mathbf{4}}, \mathbf{1}, \mathbf{1}, \mathbf{1}, \mathbf{2})$, $(0,0,1,0,0,0,0,1) \mapsto (L, Q)$
Projection matrix for $\alpha$:

$$\begin{pmatrix} 0&1&0&0&0&0&0&0\\ 1&0&0&0&0&0&0&0\\ 0&0&0&1&2&0&0&1\\ -1&-2&-3&0&0&3&0&0 \end{pmatrix}$$

**3 generation subalgebra** 199
Algebra: $\mathfrak{su}(4) \oplus \mathfrak{sp}(4) \oplus \mathfrak{su}(2) \oplus \mathfrak{su}(2) \oplus \mathfrak{su}(2)$

$(\overline{\mathbf{4}}, \mathbf{4}, \mathbf{1}, \mathbf{1}, \mathbf{1})$, $(0,0,1,1,0,0,0,0) \mapsto (D,D,E,E,N,N,U,U)$
$(\mathbf{4}, \mathbf{1}, \mathbf{2}, \mathbf{2}, \mathbf{1})$, $(1,0,0,0,0,1,1,0) \mapsto (L,L,Q,Q)$
$(\mathbf{4}, \mathbf{1}, \mathbf{2}, \mathbf{1}, \mathbf{1})$, $(1,0,0,0,0,1,0,0) \mapsto (L,Q)$
$(\overline{\mathbf{4}}, \mathbf{1}, \mathbf{1}, \mathbf{1}, \mathbf{2})$, $(0,0,1,0,0,0,0,1) \mapsto (D,E,N,U)$
Projection matrix for $\alpha$:

$$\begin{pmatrix} 1 & 0 & 0 & 0 & 0 & 0 & 0 & 0 \\ 0 & 1 & 0 & 0 & 0 & 0 & 0 & 0 \\ 0 & 0 & 0 & 0 & 0 & 1 & 0 & 0 \\ 1 & 2 & 3 & 3 & 0 & 0 & 0 & 3 \end{pmatrix}$$

**3 generation subalgebra** 200
Algebra: $\mathfrak{su}(4) \oplus \mathfrak{sp}(4) \oplus \mathfrak{su}(2) \oplus \mathfrak{su}(2) \oplus \mathfrak{su}(2)$
$(\overline{\mathbf{4}}, \mathbf{4}, \mathbf{1}, \mathbf{1}, \mathbf{1})$, $(0,0,1,1,0,0,0,0) \mapsto (L,L,Q,Q)$
$(\overline{\mathbf{4}}, \mathbf{1}, \mathbf{2}, \mathbf{1}, \mathbf{1})$, $(0,0,1,0,0,1,0,0) \mapsto (L,Q)$
$(\mathbf{4}, \mathbf{1}, \mathbf{1}, \mathbf{2}, \mathbf{1})$, $(1,0,0,0,0,0,1,0) \mapsto (D,E,N,U)$
$(\mathbf{4}, \mathbf{1}, \mathbf{1}, \mathbf{2}, \mathbf{1})$, $(1,0,0,0,0,0,1,0) \mapsto (D,E,N,U)$
$(\mathbf{4}, \mathbf{1}, \mathbf{1}, \mathbf{1}, \mathbf{2})$, $(1,0,0,0,0,0,0,1) \mapsto (D,E,N,U)$
Projection matrix for $\alpha$:

$$\begin{pmatrix} 0 & 1 & 0 & 0 & 0 & 0 & 0 & 0 \\ 1 & 0 & 0 & 0 & 0 & 0 & 0 & 0 \\ 0 & 0 & 0 & 1 & 2 & 1 & 0 & 0 \\ -1 & -2 & -3 & 0 & 0 & 0 & 3 & 3 \end{pmatrix}$$

**3 generation subalgebra** 201
Algebra: $\mathfrak{su}(4) \oplus \mathfrak{sp}(4) \oplus \mathfrak{su}(2) \oplus \mathfrak{su}(2) \oplus \mathfrak{su}(2)$
$(\overline{\mathbf{4}}, \mathbf{4}, \mathbf{1}, \mathbf{1}, \mathbf{1})$, $(0,0,1,1,0,0,0,0) \mapsto (D,D,E,E,N,N,U,U)$
$(\overline{\mathbf{4}}, \mathbf{1}, \mathbf{2}, \mathbf{1}, \mathbf{1})$, $(0,0,1,0,0,1,0,0) \mapsto (D,E,N,U)$
$(\mathbf{4}, \mathbf{1}, \mathbf{1}, \mathbf{2}, \mathbf{1})$, $(1,0,0,0,0,0,1,0) \mapsto (L,Q)$
$(\mathbf{4}, \mathbf{1}, \mathbf{1}, \mathbf{2}, \mathbf{1})$, $(1,0,0,0,0,0,1,0) \mapsto (L,Q)$
$(\mathbf{4}, \mathbf{1}, \mathbf{1}, \mathbf{1}, \mathbf{2})$, $(1,0,0,0,0,0,0,1) \mapsto (L,Q)$
Projection matrix for $\alpha$:

$$\begin{pmatrix} 1 & 0 & 0 & 0 & 0 & 0 & 0 & 0 \\ 0 & 1 & 0 & 0 & 0 & 0 & 0 & 0 \\ 0 & 0 & 0 & 0 & 0 & 0 & 1 & 1 \\ 1 & 2 & 3 & 3 & 0 & 3 & 0 & 0 \end{pmatrix}$$

**3 generation subalgebra** 202
Algebra: $\mathfrak{su}(4) \oplus \mathfrak{sp}(6) \oplus \mathfrak{su}(2) \oplus \mathfrak{su}(2) \oplus \mathfrak{su}(2)$
$(\overline{\mathbf{4}}, \mathbf{6}, \mathbf{1}, \mathbf{1}, \mathbf{1})$, $(0,0,1,1,0,0,0,0,0) \mapsto (L,L,L,Q,Q,Q)$
$(\mathbf{4}, \mathbf{1}, \mathbf{2}, \mathbf{1}, \mathbf{1})$, $(1,0,0,0,0,0,1,0,0) \mapsto (D,E,N,U)$
$(\mathbf{4}, \mathbf{1}, \mathbf{1}, \mathbf{2}, \mathbf{1})$, $(1,0,0,0,0,0,0,1,0) \mapsto (D,E,N,U)$
$(\mathbf{4}, \mathbf{1}, \mathbf{1}, \mathbf{1}, \mathbf{2})$, $(1,0,0,0,0,0,0,0,1) \mapsto (D,E,N,U)$
Projection matrix for $\alpha$:

$$\begin{pmatrix} 0 & 1 & 0 & 0 & 0 & 0 & 0 & 0 & 0 \\ 1 & 0 & 0 & 0 & 0 & 0 & 0 & 0 & 0 \\ 0 & 0 & 0 & 1 & 2 & 3 & 0 & 0 & 0 \\ -1 & -2 & -3 & 0 & 0 & 0 & 3 & 3 & 3 \end{pmatrix}$$

**3 generation subalgebra** 203
Algebra: $\mathfrak{su}(4) \oplus \mathfrak{sp}(6) \oplus \mathfrak{su}(2) \oplus \mathfrak{su}(2) \oplus \mathfrak{su}(2)$
$(\overline{\mathbf{4}}, \mathbf{6}, \mathbf{1}, \mathbf{1}, \mathbf{1})$, $(0,0,1,1,0,0,0,0,0) \mapsto (D,D,D,E,E,E,N,N,N,U,U,U)$
$(\mathbf{4}, \mathbf{1}, \mathbf{2}, \mathbf{1}, \mathbf{1})$, $(1,0,0,0,0,0,1,0,0) \mapsto (L,Q)$
$(\mathbf{4}, \mathbf{1}, \mathbf{1}, \mathbf{2}, \mathbf{1})$, $(1,0,0,0,0,0,0,1,0) \mapsto (L,Q)$
$(\mathbf{4}, \mathbf{1}, \mathbf{1}, \mathbf{1}, \mathbf{2})$, $(1,0,0,0,0,0,0,0,1) \mapsto (L,Q)$

Projection matrix for $\alpha$:

$$\begin{pmatrix} 1 & 0 & 0 & 0 & 0 & 0 & 0 & 0 & 0 \\ 0 & 1 & 0 & 0 & 0 & 0 & 0 & 0 & 0 \\ 0 & 0 & 0 & 0 & 0 & 0 & 1 & 1 & 1 \\ 1 & 2 & 3 & 3 & 0 & -3 & 0 & 0 & 0 \end{pmatrix}$$

**3 generation subalgebra** 204
Algebra: $\mathfrak{su}(4) \oplus \mathfrak{su}(2) \oplus \mathfrak{su}(2) \oplus \mathfrak{su}(2) \oplus \mathfrak{su}(2)$
$(\mathbf{4}, \mathbf{3}, \mathbf{2}, \mathbf{1}, \mathbf{1})$, $(1, 0, 0, 2, 1, 0, 0) \mapsto (L, L, L, Q, Q, Q)$
$(\overline{\mathbf{4}}, \mathbf{1}, \mathbf{1}, \mathbf{3}, \mathbf{2})$, $(0, 0, 1, 0, 0, 2, 1) \mapsto (D, D, D, E, E, E, N, N, N, U, U, U)$
Projection matrix for $\alpha$:

$$\begin{pmatrix} 1 & 0 & 0 & 0 & 0 & 0 & 0 \\ 0 & 1 & 0 & 0 & 0 & 0 & 0 \\ 0 & 0 & 0 & 0 & 1 & 0 & 0 \\ 1 & 2 & 3 & 0 & 0 & 0 & 3 \end{pmatrix}$$

**3 generation subalgebra** 205
Algebra: $\mathfrak{su}(4) \oplus \mathfrak{su}(2) \oplus \mathfrak{su}(2) \oplus \mathfrak{su}(2) \oplus \mathfrak{su}(2)$
$(\mathbf{4}, \mathbf{2}, \mathbf{2}, \mathbf{1}, \mathbf{1})$, $(1, 0, 0, 1, 1, 0, 0) \mapsto (D, D, E, E, N, N, U, U)$
$(\overline{\mathbf{4}}, \mathbf{3}, \mathbf{1}, \mathbf{2}, \mathbf{1})$, $(0, 0, 1, 2, 0, 1, 0) \mapsto (L, L, L, Q, Q, Q)$
$(\mathbf{4}, \mathbf{1}, \mathbf{1}, \mathbf{1}, \mathbf{2})$, $(1, 0, 0, 0, 0, 0, 1) \mapsto (D, E, N, U)$
Projection matrix for $\alpha$:

$$\begin{pmatrix} 0 & 1 & 0 & 0 & 0 & 0 & 0 \\ 1 & 0 & 0 & 0 & 0 & 0 & 0 \\ 0 & 0 & 0 & 0 & 0 & 1 & 0 \\ -1 & -2 & -3 & 0 & 3 & 0 & 3 \end{pmatrix}$$

**3 generation subalgebra** 206
Algebra: $\mathfrak{su}(4) \oplus \mathfrak{su}(2) \oplus \mathfrak{su}(2) \oplus \mathfrak{su}(2) \oplus \mathfrak{su}(2)$
$(\mathbf{4}, \mathbf{2}, \mathbf{2}, \mathbf{1}, \mathbf{1})$, $(1, 0, 0, 1, 1, 0, 0) \mapsto (L, L, Q, Q)$
$(\overline{\mathbf{4}}, \mathbf{3}, \mathbf{1}, \mathbf{2}, \mathbf{1})$, $(0, 0, 1, 2, 0, 1, 0) \mapsto (D, D, D, E, E, E, N, N, N, U, U, U)$
$(\mathbf{4}, \mathbf{1}, \mathbf{1}, \mathbf{1}, \mathbf{2})$, $(1, 0, 0, 0, 0, 0, 1) \mapsto (L, Q)$
Projection matrix for $\alpha$:

$$\begin{pmatrix} 1 & 0 & 0 & 0 & 0 & 0 & 0 \\ 0 & 1 & 0 & 0 & 0 & 0 & 0 \\ 0 & 0 & 0 & 0 & 1 & 0 & 1 \\ 1 & 2 & 3 & 0 & 0 & 3 & 0 \end{pmatrix}$$

**3 generation subalgebra** 207
Algebra: $\mathfrak{su}(4) \oplus \mathfrak{su}(2) \oplus \mathfrak{su}(2) \oplus \mathfrak{su}(2) \oplus \mathfrak{su}(2)$
$(\mathbf{4}, \mathbf{2}, \mathbf{2}, \mathbf{1}, \mathbf{1})$, $(1, 0, 0, 1, 1, 0, 0) \mapsto (D, D, E, E, N, N, U, U)$
$(\mathbf{4}, \mathbf{2}, \mathbf{1}, \mathbf{1}, \mathbf{1})$, $(1, 0, 0, 1, 0, 0, 0) \mapsto (D, E, N, U)$
$(\overline{\mathbf{4}}, \mathbf{1}, \mathbf{1}, \mathbf{3}, \mathbf{2})$, $(0, 0, 1, 0, 0, 2, 1) \mapsto (L, L, L, Q, Q, Q)$
Projection matrix for $\alpha$:

$$\begin{pmatrix} 0 & 1 & 0 & 0 & 0 & 0 & 0 \\ 1 & 0 & 0 & 0 & 0 & 0 & 0 \\ 0 & 0 & 0 & 0 & 0 & 0 & 1 \\ -1 & -2 & -3 & 3 & 0 & 0 & 0 \end{pmatrix}$$

**3 generation subalgebra** 208
Algebra: $\mathfrak{su}(4) \oplus \mathfrak{su}(2) \oplus \mathfrak{su}(2) \oplus \mathfrak{su}(2) \oplus \mathfrak{su}(2)$
$(\mathbf{4}, \mathbf{2}, \mathbf{2}, \mathbf{1}, \mathbf{1})$, $(1, 0, 0, 1, 1, 0, 0) \mapsto (L, L, Q, Q)$
$(\mathbf{4}, \mathbf{2}, \mathbf{1}, \mathbf{1}, \mathbf{1})$, $(1, 0, 0, 1, 0, 0, 0) \mapsto (L, Q)$
$(\overline{\mathbf{4}}, \mathbf{1}, \mathbf{1}, \mathbf{3}, \mathbf{2})$, $(0, 0, 1, 0, 0, 2, 1) \mapsto (D, D, D, E, E, E, N, N, N, U, U, U)$

Projection matrix for $\alpha$:

$$\begin{pmatrix} 1 & 0 & 0 & 0 & 0 & 0 & 0 \\ 0 & 1 & 0 & 0 & 0 & 0 & 0 \\ 0 & 0 & 0 & 1 & 0 & 0 & 0 \\ 1 & 2 & 3 & 0 & 0 & 0 & 3 \end{pmatrix}$$

**3 generation subalgebra** 209
Algebra: $\mathfrak{su}(4) \oplus \mathfrak{su}(2) \oplus \mathfrak{su}(2) \oplus \mathfrak{su}(2) \oplus \mathfrak{su}(2)$
$(\mathbf{4}, \mathbf{2}, \mathbf{2}, \mathbf{1}, \mathbf{1})$, $(1, 0, 0, 1, 1, 0, 0) \mapsto (D, D, E, E, N, N, U, U)$
$(\overline{\mathbf{4}}, \mathbf{2}, \mathbf{1}, \mathbf{2}, \mathbf{1})$, $(0, 0, 1, 1, 0, 1, 0) \mapsto (L, L, Q, Q)$
$(\mathbf{4}, \mathbf{1}, \mathbf{2}, \mathbf{1}, \mathbf{1})$, $(1, 0, 0, 0, 1, 0, 0) \mapsto (D, E, N, U)$
$(\overline{\mathbf{4}}, \mathbf{1}, \mathbf{1}, \mathbf{1}, \mathbf{2})$, $(0, 0, 1, 0, 0, 0, 1) \mapsto (L, Q)$
Projection matrix for $\alpha$:

$$\begin{pmatrix} 0 & 1 & 0 & 0 & 0 & 0 & 0 \\ 1 & 0 & 0 & 0 & 0 & 0 & 0 \\ 0 & 0 & 0 & 0 & 0 & 1 & 1 \\ -1 & -2 & -3 & 0 & 3 & 0 & 0 \end{pmatrix}$$

**3 generation subalgebra** 210
Algebra: $\mathfrak{su}(4) \oplus \mathfrak{su}(2) \oplus \mathfrak{su}(2) \oplus \mathfrak{su}(2) \oplus \mathfrak{su}(2)$
$(\mathbf{4}, \mathbf{2}, \mathbf{2}, \mathbf{1}, \mathbf{1})$, $(1, 0, 0, 1, 1, 0, 0) \mapsto (L, L, Q, Q)$
$(\overline{\mathbf{4}}, \mathbf{2}, \mathbf{1}, \mathbf{2}, \mathbf{1})$, $(0, 0, 1, 1, 0, 1, 0) \mapsto (D, D, E, E, N, N, U, U)$
$(\mathbf{4}, \mathbf{1}, \mathbf{2}, \mathbf{1}, \mathbf{1})$, $(1, 0, 0, 0, 1, 0, 0) \mapsto (L, Q)$
$(\overline{\mathbf{4}}, \mathbf{1}, \mathbf{1}, \mathbf{1}, \mathbf{2})$, $(0, 0, 1, 0, 0, 0, 1) \mapsto (D, E, N, U)$
Projection matrix for $\alpha$:

$$\begin{pmatrix} 1 & 0 & 0 & 0 & 0 & 0 & 0 \\ 0 & 1 & 0 & 0 & 0 & 0 & 0 \\ 0 & 0 & 0 & 0 & 1 & 0 & 0 \\ 1 & 2 & 3 & 0 & 0 & 3 & 3 \end{pmatrix}$$

**3 generation subalgebra** 211
Algebra: $\mathfrak{su}(4) \oplus \mathfrak{su}(2) \oplus \mathfrak{su}(2) \oplus \mathfrak{su}(2) \oplus \mathfrak{su}(2)$
$(\mathbf{4}, \mathbf{2}, \mathbf{2}, \mathbf{1}, \mathbf{1})$, $(1, 0, 0, 1, 1, 0, 0) \mapsto (L, L, Q, Q)$
$(\mathbf{4}, \mathbf{2}, \mathbf{1}, \mathbf{1}, \mathbf{1})$, $(1, 0, 0, 1, 0, 0, 0) \mapsto (L, Q)$
$(\overline{\mathbf{4}}, \mathbf{1}, \mathbf{1}, \mathbf{2}, \mathbf{2})$, $(0, 0, 1, 0, 0, 1, 1) \mapsto (D, D, E, E, N, N, U, U)$
$(\overline{\mathbf{4}}, \mathbf{1}, \mathbf{1}, \mathbf{2}, \mathbf{1})$, $(0, 0, 1, 0, 0, 1, 0) \mapsto (D, E, N, U)$
Projection matrix for $\alpha$:

$$\begin{pmatrix} 1 & 0 & 0 & 0 & 0 & 0 & 0 \\ 0 & 1 & 0 & 0 & 0 & 0 & 0 \\ 0 & 0 & 0 & 1 & 0 & 0 & 0 \\ 1 & 2 & 3 & 0 & 0 & 3 & 0 \end{pmatrix}$$

**3 generation subalgebra** 212
Algebra: $\mathfrak{su}(4) \oplus \mathfrak{su}(2) \oplus \mathfrak{su}(2) \oplus \mathfrak{su}(2) \oplus \mathfrak{su}(2)$
$(\mathbf{4}, \mathbf{3}, \mathbf{2}, \mathbf{1}, \mathbf{1})$, $(1, 0, 0, 2, 1, 0, 0) \mapsto (D, D, D, E, E, E, N, N, N, U, U, U)$
$(\overline{\mathbf{4}}, \mathbf{1}, \mathbf{1}, \mathbf{2}, \mathbf{1})$, $(0, 0, 1, 0, 0, 1, 0) \mapsto (L, Q)$
$(\overline{\mathbf{4}}, \mathbf{1}, \mathbf{1}, \mathbf{2}, \mathbf{1})$, $(0, 0, 1, 0, 0, 1, 0) \mapsto (L, Q)$
$(\overline{\mathbf{4}}, \mathbf{1}, \mathbf{1}, \mathbf{1}, \mathbf{2})$, $(0, 0, 1, 0, 0, 0, 1) \mapsto (L, Q)$
Projection matrix for $\alpha$:

$$\begin{pmatrix} 0 & 1 & 0 & 0 & 0 & 0 & 0 \\ 1 & 0 & 0 & 0 & 0 & 0 & 0 \\ 0 & 0 & 0 & 0 & 0 & 1 & 1 \\ -1 & -2 & -3 & 0 & 3 & 0 & 0 \end{pmatrix}$$

**3 generation subalgebra** 213
Algebra: $\mathfrak{su}(4) \oplus \mathfrak{su}(2) \oplus \mathfrak{su}(2) \oplus \mathfrak{su}(2) \oplus \mathfrak{su}(2)$

$(\mathbf{4},\mathbf{3},\mathbf{2},\mathbf{1},\mathbf{1})$, $(1,0,0,2,1,0,0) \mapsto (L,L,L,Q,Q,Q)$
$(\overline{\mathbf{4}},\mathbf{1},\mathbf{1},\mathbf{2},\mathbf{1})$, $(0,0,1,0,0,1,0) \mapsto (D,E,N,U)$
$(\overline{\mathbf{4}},\mathbf{1},\mathbf{1},\mathbf{2},\mathbf{1})$, $(0,0,1,0,0,1,0) \mapsto (D,E,N,U)$
$(\overline{\mathbf{4}},\mathbf{1},\mathbf{1},\mathbf{1},\mathbf{2})$, $(0,0,1,0,0,0,1) \mapsto (D,E,N,U)$
Projection matrix for $\alpha$:

$$\begin{pmatrix} 1 & 0 & 0 & 0 & 0 & 0 & 0 \\ 0 & 1 & 0 & 0 & 0 & 0 & 0 \\ 0 & 0 & 0 & 0 & 1 & 0 & 0 \\ 1 & 2 & 3 & 0 & 0 & 3 & 3 \end{pmatrix}$$

**3 generation subalgebra** 214
Algebra: $\mathfrak{su}(4) \oplus \mathfrak{su}(2) \oplus \mathfrak{su}(2) \oplus \mathfrak{su}(2) \oplus \mathfrak{su}(2)$
$(\mathbf{4},\mathbf{2},\mathbf{2},\mathbf{1},\mathbf{1})$, $(1,0,0,1,1,0,0) \mapsto (D,D,E,E,N,N,U,U)$
$(\overline{\mathbf{4}},\mathbf{1},\mathbf{1},\mathbf{2},\mathbf{1})$, $(0,0,1,0,0,1,0) \mapsto (L,Q)$
$(\overline{\mathbf{4}},\mathbf{1},\mathbf{1},\mathbf{2},\mathbf{1})$, $(0,0,1,0,0,1,0) \mapsto (L,Q)$
$(\overline{\mathbf{4}},\mathbf{1},\mathbf{1},\mathbf{2},\mathbf{1})$, $(0,0,1,0,0,1,0) \mapsto (L,Q)$
$(\mathbf{4},\mathbf{1},\mathbf{1},\mathbf{1},\mathbf{2})$, $(1,0,0,0,0,0,1) \mapsto (D,E,N,U)$
Projection matrix for $\alpha$:

$$\begin{pmatrix} 0 & 1 & 0 & 0 & 0 & 0 & 0 \\ 1 & 0 & 0 & 0 & 0 & 0 & 0 \\ 0 & 0 & 0 & 0 & 0 & 1 & 0 \\ -1 & -2 & -3 & 3 & 0 & 0 & 3 \end{pmatrix}$$

**3 generation subalgebra** 215
Algebra: $\mathfrak{su}(4) \oplus \mathfrak{su}(2) \oplus \mathfrak{su}(2) \oplus \mathfrak{su}(2) \oplus \mathfrak{su}(2)$
$(\mathbf{4},\mathbf{2},\mathbf{2},\mathbf{1},\mathbf{1})$, $(1,0,0,1,1,0,0) \mapsto (L,L,Q,Q)$
$(\overline{\mathbf{4}},\mathbf{1},\mathbf{1},\mathbf{2},\mathbf{1})$, $(0,0,1,0,0,1,0) \mapsto (D,E,N,U)$
$(\overline{\mathbf{4}},\mathbf{1},\mathbf{1},\mathbf{2},\mathbf{1})$, $(0,0,1,0,0,1,0) \mapsto (D,E,N,U)$
$(\overline{\mathbf{4}},\mathbf{1},\mathbf{1},\mathbf{2},\mathbf{1})$, $(0,0,1,0,0,1,0) \mapsto (D,E,N,U)$
$(\mathbf{4},\mathbf{1},\mathbf{1},\mathbf{1},\mathbf{2})$, $(1,0,0,0,0,0,1) \mapsto (L,Q)$
Projection matrix for $\alpha$:

$$\begin{pmatrix} 1 & 0 & 0 & 0 & 0 & 0 & 0 \\ 0 & 1 & 0 & 0 & 0 & 0 & 0 \\ 0 & 0 & 0 & 1 & 0 & 0 & 1 \\ 1 & 2 & 3 & 0 & 0 & 3 & 0 \end{pmatrix}$$

**3 generation subalgebra** 216
Algebra: $\mathfrak{su}(4) \oplus \mathfrak{su}(2) \oplus \mathfrak{su}(2) \oplus \mathfrak{su}(2) \oplus \mathfrak{su}(2)$
$(\mathbf{4},\mathbf{2},\mathbf{2},\mathbf{1},\mathbf{1})$, $(1,0,0,1,1,0,0) \mapsto (D,D,E,E,N,N,U,U)$
$(\mathbf{4},\mathbf{2},\mathbf{1},\mathbf{1},\mathbf{1})$, $(1,0,0,1,0,0,0) \mapsto (D,E,N,U)$
$(\overline{\mathbf{4}},\mathbf{1},\mathbf{1},\mathbf{2},\mathbf{1})$, $(0,0,1,0,0,1,0) \mapsto (L,Q)$
$(\overline{\mathbf{4}},\mathbf{1},\mathbf{1},\mathbf{2},\mathbf{1})$, $(0,0,1,0,0,1,0) \mapsto (L,Q)$
$(\overline{\mathbf{4}},\mathbf{1},\mathbf{1},\mathbf{1},\mathbf{2})$, $(0,0,1,0,0,0,1) \mapsto (L,Q)$
Projection matrix for $\alpha$:

$$\begin{pmatrix} 0 & 1 & 0 & 0 & 0 & 0 & 0 \\ 1 & 0 & 0 & 0 & 0 & 0 & 0 \\ 0 & 0 & 0 & 0 & 0 & 1 & 1 \\ -1 & -2 & -3 & 3 & 0 & 0 & 0 \end{pmatrix}$$

**3 generation subalgebra** 217
Algebra: $\mathfrak{su}(4) \oplus \mathfrak{su}(2) \oplus \mathfrak{su}(2) \oplus \mathfrak{su}(2) \oplus \mathfrak{su}(2)$
$(\mathbf{4},\mathbf{2},\mathbf{2},\mathbf{1},\mathbf{1})$, $(1,0,0,1,1,0,0) \mapsto (L,L,Q,Q)$
$(\mathbf{4},\mathbf{2},\mathbf{1},\mathbf{1},\mathbf{1})$, $(1,0,0,1,0,0,0) \mapsto (L,Q)$
$(\overline{\mathbf{4}},\mathbf{1},\mathbf{1},\mathbf{2},\mathbf{1})$, $(0,0,1,0,0,1,0) \mapsto (D,E,N,U)$
$(\overline{\mathbf{4}},\mathbf{1},\mathbf{1},\mathbf{2},\mathbf{1})$, $(0,0,1,0,0,1,0) \mapsto (D,E,N,U)$

$(\overline{\mathbf{4}},\mathbf{1},\mathbf{1},\mathbf{1},\mathbf{2})$, $(0,0,1,0,0,0,1) \mapsto (D,E,N,U)$
Projection matrix for $\alpha$:

$$\begin{pmatrix} 1&0&0&0&0&0&0\\ 0&1&0&0&0&0&0\\ 0&0&0&1&0&0&0\\ 1&2&3&0&0&3&3 \end{pmatrix}$$

**3 generation subalgebra** 218
Algebra: $\mathfrak{su}(4)\oplus\mathfrak{su}(2)\oplus\mathfrak{su}(2)\oplus\mathfrak{su}(2)\oplus\mathfrak{su}(2)$
$(\overline{\mathbf{4}},\mathbf{2},\mathbf{1},\mathbf{1},\mathbf{1})$, $(0,0,1,1,0,0,0) \mapsto (L,Q)$
$(\overline{\mathbf{4}},\mathbf{2},\mathbf{1},\mathbf{1},\mathbf{1})$, $(0,0,1,1,0,0,0) \mapsto (L,Q)$
$(\overline{\mathbf{4}},\mathbf{1},\mathbf{2},\mathbf{1},\mathbf{1})$, $(0,0,1,0,1,0,0) \mapsto (L,Q)$
$(\mathbf{4},\mathbf{1},\mathbf{1},\mathbf{2},\mathbf{1})$, $(1,0,0,0,0,1,0) \mapsto (D,E,N,U)$
$(\mathbf{4},\mathbf{1},\mathbf{1},\mathbf{2},\mathbf{1})$, $(1,0,0,0,0,1,0) \mapsto (D,E,N,U)$
$(\mathbf{4},\mathbf{1},\mathbf{1},\mathbf{1},\mathbf{2})$, $(1,0,0,0,0,0,1) \mapsto (D,E,N,U)$
Projection matrix for $\alpha$:

$$\begin{pmatrix} 0&1&0&0&0&0&0\\ 1&0&0&0&0&0&0\\ 0&0&0&1&1&0&0\\ -1&-2&-3&0&0&3&3 \end{pmatrix}$$

**3 generation subalgebra** 219
Algebra: $\mathfrak{su}(4)\oplus\mathfrak{su}(2)\oplus\mathfrak{su}(2)\oplus\mathfrak{su}(2)\oplus\mathfrak{su}(2)$
$(\overline{\mathbf{4}},\mathbf{2},\mathbf{1},\mathbf{1},\mathbf{1})$, $(0,0,1,1,0,0,0) \mapsto (L,Q)$
$(\overline{\mathbf{4}},\mathbf{2},\mathbf{1},\mathbf{1},\mathbf{1})$, $(0,0,1,1,0,0,0) \mapsto (L,Q)$
$(\overline{\mathbf{4}},\mathbf{2},\mathbf{1},\mathbf{1},\mathbf{1})$, $(0,0,1,1,0,0,0) \mapsto (L,Q)$
$(\mathbf{4},\mathbf{1},\mathbf{2},\mathbf{1},\mathbf{1})$, $(1,0,0,0,1,0,0) \mapsto (D,E,N,U)$
$(\mathbf{4},\mathbf{1},\mathbf{1},\mathbf{2},\mathbf{1})$, $(1,0,0,0,0,1,0) \mapsto (D,E,N,U)$
$(\mathbf{4},\mathbf{1},\mathbf{1},\mathbf{1},\mathbf{2})$, $(1,0,0,0,0,0,1) \mapsto (D,E,N,U)$
Projection matrix for $\alpha$:

$$\begin{pmatrix} 0&1&0&0&0&0&0\\ 1&0&0&0&0&0&0\\ 0&0&0&1&0&0&0\\ -1&-2&-3&0&3&3&3 \end{pmatrix}$$

**3 generation subalgebra** 220
Algebra: $\mathfrak{su}(4)\oplus\mathfrak{su}(2)\oplus\mathfrak{su}(2)\oplus\mathfrak{su}(2)\oplus\mathfrak{su}(2)$
$(\overline{\mathbf{4}},\mathbf{2},\mathbf{1},\mathbf{1},\mathbf{1})$, $(0,0,1,1,0,0,0) \mapsto (D,E,N,U)$
$(\overline{\mathbf{4}},\mathbf{2},\mathbf{1},\mathbf{1},\mathbf{1})$, $(0,0,1,1,0,0,0) \mapsto (D,E,N,U)$
$(\overline{\mathbf{4}},\mathbf{2},\mathbf{1},\mathbf{1},\mathbf{1})$, $(0,0,1,1,0,0,0) \mapsto (D,E,N,U)$
$(\mathbf{4},\mathbf{1},\mathbf{2},\mathbf{1},\mathbf{1})$, $(1,0,0,0,1,0,0) \mapsto (L,Q)$
$(\mathbf{4},\mathbf{1},\mathbf{1},\mathbf{2},\mathbf{1})$, $(1,0,0,0,0,1,0) \mapsto (L,Q)$
$(\mathbf{4},\mathbf{1},\mathbf{1},\mathbf{1},\mathbf{2})$, $(1,0,0,0,0,0,1) \mapsto (L,Q)$
Projection matrix for $\alpha$:

$$\begin{pmatrix} 1&0&0&0&0&0&0\\ 0&1&0&0&0&0&0\\ 0&0&0&0&1&1&1\\ 1&2&3&3&0&0&0 \end{pmatrix}$$

**3 generation subalgebra** 221
Algebra: $\mathfrak{su}(4)\oplus\mathfrak{su}(4)\oplus\mathfrak{so}(10)\oplus\mathfrak{su}(2)\oplus\mathfrak{su}(2)$
$(\mathbf{1},\mathbf{1},\mathbf{16},\mathbf{1},\mathbf{1})$, $(0,0,0,0,0,0,0,0,0,0,1,0,0) \mapsto (D,E,L,N,Q,U)$
$(\overline{\mathbf{4}},\mathbf{1},\mathbf{1},\mathbf{2},\mathbf{1})$, $(0,0,1,0,0,0,0,0,0,0,0,1,0) \mapsto (L,Q)$
$(\mathbf{1},\overline{\mathbf{4}},\mathbf{1},\mathbf{2},\mathbf{1})$, $(0,0,0,0,0,1,0,0,0,0,0,1,0) \mapsto (L,Q)$
$(\mathbf{4},\mathbf{1},\mathbf{1},\mathbf{1},\mathbf{2})$, $(1,0,0,0,0,0,0,0,0,0,0,0,1) \mapsto (D,E,N,U)$

$(\mathbf{1},\mathbf{4},\mathbf{1},\mathbf{1},\mathbf{2})$, $(0,0,0,1,0,0,0,0,0,0,0,0,1) \mapsto (D,E,N,U)$
Projection matrix for $\alpha$:

$$\begin{pmatrix} 0 & 1 & 0 & 0 & 1 & 0 & 0 & 0 & 1 & 0 & 0 & 0 & 0 \\ 1 & 0 & 0 & 1 & 0 & 0 & 0 & 0 & 0 & 0 & 1 & 0 & 0 \\ 0 & 0 & 0 & 0 & 0 & 0 & 1 & 0 & 0 & 0 & 0 & 1 & 0 \\ -1 & -2 & -3 & -1 & -2 & -3 & 3 & 6 & 4 & 0 & 2 & 0 & 3 \end{pmatrix}$$

**3 generation subalgebra** 222
Algebra: $\mathfrak{su}(4) \oplus \mathfrak{su}(4) \oplus \mathfrak{sp}(4) \oplus \mathfrak{su}(2) \oplus \mathfrak{su}(2)$
$(\overline{\mathbf{4}},\mathbf{1},\mathbf{4},\mathbf{1},\mathbf{1})$, $(0,0,1,0,0,0,1,0,0,0) \mapsto (L,L,Q,Q)$
$(\mathbf{4},\mathbf{1},\mathbf{1},\mathbf{2},\mathbf{1})$, $(1,0,0,0,0,0,0,0,1,0) \mapsto (D,E,N,U)$
$(\mathbf{4},\mathbf{1},\mathbf{1},\mathbf{2},\mathbf{1})$, $(1,0,0,0,0,0,0,0,1,0) \mapsto (D,E,N,U)$
$(\mathbf{1},\overline{\mathbf{4}},\mathbf{1},\mathbf{2},\mathbf{1})$, $(0,0,0,0,0,1,0,0,1,0) \mapsto (D,E,N,U)$
$(\mathbf{1},\mathbf{4},\mathbf{1},\mathbf{1},\mathbf{2})$, $(0,0,0,1,0,0,0,0,0,1) \mapsto (L,Q)$
Projection matrix for $\alpha$:

$$\begin{pmatrix} 0 & 1 & 0 & 1 & 0 & 0 & 0 & 0 & 0 & 0 \\ 1 & 0 & 0 & 0 & 1 & 0 & 0 & 0 & 0 & 0 \\ 0 & 0 & 0 & 0 & 0 & 0 & 1 & 2 & 0 & 1 \\ -1 & -2 & -3 & 1 & 2 & 3 & 0 & 0 & 3 & 0 \end{pmatrix}$$

**3 generation subalgebra** 223
Algebra: $\mathfrak{su}(4) \oplus \mathfrak{su}(4) \oplus \mathfrak{sp}(4) \oplus \mathfrak{su}(2) \oplus \mathfrak{su}(2)$
$(\overline{\mathbf{4}},\mathbf{1},\mathbf{4},\mathbf{1},\mathbf{1})$, $(0,0,1,0,0,0,1,0,0,0) \mapsto (D,D,E,E,N,N,U,U)$
$(\mathbf{4},\mathbf{1},\mathbf{1},\mathbf{2},\mathbf{1})$, $(1,0,0,0,0,0,0,0,1,0) \mapsto (L,Q)$
$(\mathbf{4},\mathbf{1},\mathbf{1},\mathbf{2},\mathbf{1})$, $(1,0,0,0,0,0,0,0,1,0) \mapsto (L,Q)$
$(\mathbf{1},\overline{\mathbf{4}},\mathbf{1},\mathbf{2},\mathbf{1})$, $(0,0,0,0,0,1,0,0,1,0) \mapsto (L,Q)$
$(\mathbf{1},\mathbf{4},\mathbf{1},\mathbf{1},\mathbf{2})$, $(0,0,0,1,0,0,0,0,0,1) \mapsto (D,E,N,U)$
Projection matrix for $\alpha$:

$$\begin{pmatrix} 1 & 0 & 0 & 0 & 1 & 0 & 0 & 0 & 0 & 0 \\ 0 & 1 & 0 & 1 & 0 & 0 & 0 & 0 & 0 & 0 \\ 0 & 0 & 0 & 0 & 0 & 0 & 0 & 0 & 1 & 0 \\ 1 & 2 & 3 & -1 & -2 & -3 & 3 & 0 & 0 & 3 \end{pmatrix}$$

**3 generation subalgebra** 224
Algebra: $\mathfrak{su}(4) \oplus \mathfrak{su}(4) \oplus \mathfrak{su}(2) \oplus \mathfrak{su}(2) \oplus \mathfrak{su}(2)$
$(\overline{\mathbf{4}},\mathbf{6},\mathbf{1},\mathbf{1},\mathbf{1})$, $(0,0,1,0,1,0,0,0,0) \mapsto (D,D,D,E,E,E,N,N,N,U,U,U)$
$(\mathbf{4},\mathbf{1},\mathbf{2},\mathbf{1},\mathbf{1})$, $(1,0,0,0,0,0,1,0,0) \mapsto (L,Q)$
$(\mathbf{4},\mathbf{1},\mathbf{1},\mathbf{2},\mathbf{1})$, $(1,0,0,0,0,0,0,1,0) \mapsto (L,Q)$
$(\mathbf{4},\mathbf{1},\mathbf{1},\mathbf{1},\mathbf{2})$, $(1,0,0,0,0,0,0,0,1) \mapsto (L,Q)$
Projection matrix for $\alpha$:

$$\begin{pmatrix} 1 & 0 & 0 & 0 & 0 & 0 & 0 & 0 & 0 \\ 0 & 1 & 0 & 0 & 0 & 0 & 0 & 0 & 0 \\ 0 & 0 & 0 & 0 & 0 & 0 & 1 & 1 & 1 \\ 1 & 2 & 3 & \frac{9}{2} & 3 & \frac{3}{2} & 0 & 0 & 0 \end{pmatrix}$$

**3 generation subalgebra** 225
Algebra: $\mathfrak{su}(4) \oplus \mathfrak{su}(4) \oplus \mathfrak{su}(2) \oplus \mathfrak{su}(2) \oplus \mathfrak{su}(2)$
$(\mathbf{4},\mathbf{1},\mathbf{2},\mathbf{2},\mathbf{1})$, $(1,0,0,0,0,0,1,1,0) \mapsto (L,L,Q,Q)$
$(\overline{\mathbf{4}},\mathbf{1},\mathbf{2},\mathbf{1},\mathbf{2})$, $(0,0,1,0,0,0,1,0,1) \mapsto (D,D,E,E,N,N,U,U)$
$(\mathbf{1},\overline{\mathbf{4}},\mathbf{1},\mathbf{2},\mathbf{1})$, $(0,0,0,0,0,1,0,1,0) \mapsto (L,Q)$
$(\mathbf{1},\mathbf{4},\mathbf{1},\mathbf{1},\mathbf{2})$, $(0,0,0,1,0,0,0,0,1) \mapsto (D,E,N,U)$
Projection matrix for $\alpha$:

$$\begin{pmatrix} 1 & 0 & 0 & 0 & 1 & 0 & 0 & 0 & 0 \\ 0 & 1 & 0 & 1 & 0 & 0 & 0 & 0 & 0 \\ 0 & 0 & 0 & 0 & 0 & 0 & 0 & 1 & 0 \\ 1 & 2 & 3 & -1 & -2 & -3 & 0 & 0 & 3 \end{pmatrix}$$

**3 generation subalgebra** 226
Algebra: $\mathfrak{su}(4) \oplus \mathfrak{su}(4) \oplus \mathfrak{su}(2) \oplus \mathfrak{su}(2) \oplus \mathfrak{su}(2)$
$(\mathbf{4}, \mathbf{1}, \mathbf{2}, \mathbf{2}, \mathbf{1})$, $(1,0,0,0,0,0,1,1,0) \mapsto (D, D, E, E, N, N, U, U)$
$(\mathbf{1}, \overline{\mathbf{4}}, \mathbf{2}, \mathbf{1}, \mathbf{1})$, $(0,0,0,0,0,1,1,0,0) \mapsto (D, E, N, U)$
$(\overline{\mathbf{4}}, \mathbf{1}, \mathbf{1}, \mathbf{1}, \mathbf{2})$, $(0,0,1,0,0,0,0,0,1) \mapsto (L, Q)$
$(\overline{\mathbf{4}}, \mathbf{1}, \mathbf{1}, \mathbf{1}, \mathbf{2})$, $(0,0,1,0,0,0,0,0,1) \mapsto (L, Q)$
$(\mathbf{1}, \mathbf{4}, \mathbf{1}, \mathbf{1}, \mathbf{2})$, $(0,0,0,1,0,0,0,0,1) \mapsto (L, Q)$
Projection matrix for $\alpha$:

$$\begin{pmatrix} 0 & 1 & 0 & 1 & 0 & 0 & 0 & 0 & 0 \\ 1 & 0 & 0 & 0 & 1 & 0 & 0 & 0 & 0 \\ 0 & 0 & 0 & 0 & 0 & 0 & 0 & 0 & 1 \\ -1 & -2 & -3 & 1 & 2 & 3 & 3 & 0 & 0 \end{pmatrix}$$

**3 generation subalgebra** 227
Algebra: $\mathfrak{su}(4) \oplus \mathfrak{su}(4) \oplus \mathfrak{su}(2) \oplus \mathfrak{su}(2) \oplus \mathfrak{su}(2)$
$(\mathbf{4}, \mathbf{1}, \mathbf{2}, \mathbf{2}, \mathbf{1})$, $(1,0,0,0,0,0,1,1,0) \mapsto (L, L, Q, Q)$
$(\mathbf{1}, \overline{\mathbf{4}}, \mathbf{2}, \mathbf{1}, \mathbf{1})$, $(0,0,0,0,0,1,1,0,0) \mapsto (L, Q)$
$(\overline{\mathbf{4}}, \mathbf{1}, \mathbf{1}, \mathbf{1}, \mathbf{2})$, $(0,0,1,0,0,0,0,0,1) \mapsto (D, E, N, U)$
$(\overline{\mathbf{4}}, \mathbf{1}, \mathbf{1}, \mathbf{1}, \mathbf{2})$, $(0,0,1,0,0,0,0,0,1) \mapsto (D, E, N, U)$
$(\mathbf{1}, \mathbf{4}, \mathbf{1}, \mathbf{1}, \mathbf{2})$, $(0,0,0,1,0,0,0,0,1) \mapsto (D, E, N, U)$
Projection matrix for $\alpha$:

$$\begin{pmatrix} 1 & 0 & 0 & 0 & 1 & 0 & 0 & 0 & 0 \\ 0 & 1 & 0 & 1 & 0 & 0 & 0 & 0 & 0 \\ 0 & 0 & 0 & 0 & 0 & 0 & 1 & 0 & 0 \\ 1 & 2 & 3 & -1 & -2 & -3 & 0 & 0 & 3 \end{pmatrix}$$

**3 generation subalgebra** 228
Algebra: $\mathfrak{su}(4) \oplus \mathfrak{su}(4) \oplus \mathfrak{su}(2) \oplus \mathfrak{su}(2) \oplus \mathfrak{su}(2)$
$(\overline{\mathbf{4}}, \mathbf{1}, \mathbf{2}, \mathbf{1}, \mathbf{1})$, $(0,0,1,0,0,0,1,0,0) \mapsto (L, Q)$
$(\overline{\mathbf{4}}, \mathbf{1}, \mathbf{2}, \mathbf{1}, \mathbf{1})$, $(0,0,1,0,0,0,1,0,0) \mapsto (L, Q)$
$(\mathbf{1}, \overline{\mathbf{4}}, \mathbf{2}, \mathbf{1}, \mathbf{1})$, $(0,0,0,0,0,1,1,0,0) \mapsto (L, Q)$
$(\mathbf{4}, \mathbf{1}, \mathbf{1}, \mathbf{2}, \mathbf{1})$, $(1,0,0,0,0,0,0,1,0) \mapsto (D, E, N, U)$
$(\mathbf{1}, \mathbf{4}, \mathbf{1}, \mathbf{2}, \mathbf{1})$, $(0,0,0,1,0,0,0,1,0) \mapsto (D, E, N, U)$
$(\mathbf{4}, \mathbf{1}, \mathbf{1}, \mathbf{1}, \mathbf{2})$, $(1,0,0,0,0,0,0,0,1) \mapsto (D, E, N, U)$
Projection matrix for $\alpha$:

$$\begin{pmatrix} 0 & 1 & 0 & 0 & 1 & 0 & 0 & 0 & 0 \\ 1 & 0 & 0 & 1 & 0 & 0 & 0 & 0 & 0 \\ 0 & 0 & 0 & 0 & 0 & 0 & 1 & 0 & 0 \\ -1 & -2 & -3 & -1 & -2 & -3 & 0 & 3 & 3 \end{pmatrix}$$

**3 generation subalgebra** 229
Algebra: $\mathfrak{su}(4) \oplus \mathfrak{su}(4) \oplus \mathfrak{su}(2) \oplus \mathfrak{su}(2) \oplus \mathfrak{su}(2)$
$(\overline{\mathbf{4}}, \mathbf{1}, \mathbf{2}, \mathbf{1}, \mathbf{1})$, $(0,0,1,0,0,0,1,0,0) \mapsto (D, E, N, U)$
$(\overline{\mathbf{4}}, \mathbf{1}, \mathbf{2}, \mathbf{1}, \mathbf{1})$, $(0,0,1,0,0,0,1,0,0) \mapsto (D, E, N, U)$
$(\mathbf{1}, \overline{\mathbf{4}}, \mathbf{2}, \mathbf{1}, \mathbf{1})$, $(0,0,0,0,0,1,1,0,0) \mapsto (D, E, N, U)$
$(\mathbf{4}, \mathbf{1}, \mathbf{1}, \mathbf{2}, \mathbf{1})$, $(1,0,0,0,0,0,0,1,0) \mapsto (L, Q)$
$(\mathbf{1}, \mathbf{4}, \mathbf{1}, \mathbf{2}, \mathbf{1})$, $(0,0,0,1,0,0,0,1,0) \mapsto (L, Q)$
$(\mathbf{4}, \mathbf{1}, \mathbf{1}, \mathbf{1}, \mathbf{2})$, $(1,0,0,0,0,0,0,0,1) \mapsto (L, Q)$
Projection matrix for $\alpha$:

$$\begin{pmatrix} 1 & 0 & 0 & 1 & 0 & 0 & 0 & 0 & 0 \\ 0 & 1 & 0 & 0 & 1 & 0 & 0 & 0 & 0 \\ 0 & 0 & 0 & 0 & 0 & 0 & 0 & 1 & 1 \\ 1 & 2 & 3 & 1 & 2 & 3 & 3 & 0 & 0 \end{pmatrix}$$

**3 generation subalgebra** 230
Algebra: $\mathfrak{su}(4) \oplus \mathfrak{su}(4) \oplus \mathfrak{su}(2) \oplus \mathfrak{su}(2) \oplus \mathfrak{su}(2)$

$(\bar{\mathbf{4}},\mathbf{1},\mathbf{2},\mathbf{1},\mathbf{1})$, $(0,0,1,0,0,0,1,0,0) \mapsto (L,Q)$
$(\bar{\mathbf{4}},\mathbf{1},\mathbf{2},\mathbf{1},\mathbf{1})$, $(0,0,1,0,0,0,1,0,0) \mapsto (L,Q)$
$(\mathbf{1},\bar{\mathbf{4}},\mathbf{2},\mathbf{1},\mathbf{1})$, $(0,0,0,0,0,1,1,0,0) \mapsto (L,Q)$
$(\mathbf{4},\mathbf{1},\mathbf{1},\mathbf{2},\mathbf{1})$, $(1,0,0,0,0,0,0,1,0) \mapsto (D,E,N,U)$
$(\mathbf{4},\mathbf{1},\mathbf{1},\mathbf{2},\mathbf{1})$, $(1,0,0,0,0,0,0,1,0) \mapsto (D,E,N,U)$
$(\mathbf{1},\mathbf{4},\mathbf{1},\mathbf{1},\mathbf{2})$, $(0,0,0,1,0,0,0,0,1) \mapsto (D,E,N,U)$
Projection matrix for $\alpha$:

$$\begin{pmatrix} 0 & 1 & 0 & 0 & 1 & 0 & 0 & 0 & 0 \\ 1 & 0 & 0 & 1 & 0 & 0 & 0 & 0 & 0 \\ 0 & 0 & 0 & 0 & 0 & 0 & 1 & 0 & 0 \\ -1 & -2 & -3 & -1 & -2 & -3 & 0 & 3 & 3 \end{pmatrix}$$

**3 generation subalgebra** 231
Algebra: $\mathfrak{su}(4) \oplus \mathfrak{su}(4) \oplus \mathfrak{su}(2) \oplus \mathfrak{su}(2) \oplus \mathfrak{su}(2)$
$(\bar{\mathbf{4}},\mathbf{1},\mathbf{2},\mathbf{1},\mathbf{1})$, $(0,0,1,0,0,0,1,0,0) \mapsto (D,E,N,U)$
$(\bar{\mathbf{4}},\mathbf{1},\mathbf{2},\mathbf{1},\mathbf{1})$, $(0,0,1,0,0,0,1,0,0) \mapsto (D,E,N,U)$
$(\mathbf{1},\bar{\mathbf{4}},\mathbf{2},\mathbf{1},\mathbf{1})$, $(0,0,0,0,0,1,1,0,0) \mapsto (D,E,N,U)$
$(\mathbf{4},\mathbf{1},\mathbf{1},\mathbf{2},\mathbf{1})$, $(1,0,0,0,0,0,0,1,0) \mapsto (L,Q)$
$(\mathbf{4},\mathbf{1},\mathbf{1},\mathbf{2},\mathbf{1})$, $(1,0,0,0,0,0,0,1,0) \mapsto (L,Q)$
$(\mathbf{1},\mathbf{4},\mathbf{1},\mathbf{1},\mathbf{2})$, $(0,0,0,1,0,0,0,0,1) \mapsto (L,Q)$
Projection matrix for $\alpha$:

$$\begin{pmatrix} 1 & 0 & 0 & 1 & 0 & 0 & 0 & 0 & 0 \\ 0 & 1 & 0 & 0 & 1 & 0 & 0 & 0 & 0 \\ 0 & 0 & 0 & 0 & 0 & 0 & 0 & 1 & 1 \\ 1 & 2 & 3 & 1 & 2 & 3 & 3 & 0 & 0 \end{pmatrix}$$

**3 generation subalgebra** 232
Algebra: $\mathfrak{su}(4) \oplus \mathfrak{su}(4) \oplus \mathfrak{su}(5) \oplus \mathfrak{su}(2) \oplus \mathfrak{su}(2)$
$(\mathbf{1},\mathbf{1},\bar{\mathbf{5}},\mathbf{1},\mathbf{1})$, $(0,0,0,0,0,0,0,0,0,1,0,0) \mapsto (D,L)$
$(\mathbf{1},\mathbf{1},\mathbf{10},\mathbf{1},\mathbf{1})$, $(0,0,0,0,0,0,0,1,0,0,0,0) \mapsto (E,Q,U)$
$(\bar{\mathbf{4}},\mathbf{1},\mathbf{1},\mathbf{2},\mathbf{1})$, $(0,0,1,0,0,0,0,0,0,0,1,0) \mapsto (L,Q)$
$(\mathbf{1},\bar{\mathbf{4}},\mathbf{1},\mathbf{2},\mathbf{1})$, $(0,0,0,0,0,1,0,0,0,0,1,0) \mapsto (L,Q)$
$(\mathbf{4},\mathbf{1},\mathbf{1},\mathbf{1},\mathbf{2})$, $(1,0,0,0,0,0,0,0,0,0,0,1) \mapsto (D,E,N,U)$
$(\mathbf{1},\mathbf{4},\mathbf{1},\mathbf{1},\mathbf{2})$, $(0,0,0,1,0,0,0,0,0,0,0,1) \mapsto (D,E,N,U)$
$(\mathbf{1},\mathbf{1},\mathbf{1},\mathbf{1},\mathbf{1})$, $(0,0,0,0,0,0,0,0,0,0,0,0) \mapsto (N)$
Projection matrix for $\alpha$:

$$\begin{pmatrix} 0 & 1 & 0 & 0 & 1 & 0 & 0 & 0 & 1 & 0 & 0 & 0 \\ 1 & 0 & 0 & 1 & 0 & 0 & 0 & 0 & 0 & 1 & 0 & 0 \\ 0 & 0 & 0 & 0 & 0 & 0 & 1 & 0 & 0 & 0 & 1 & 0 \\ -1 & -2 & -3 & -1 & -2 & -3 & 3 & 6 & 4 & 2 & 0 & 3 \end{pmatrix}$$

**3 generation subalgebra** 233
Algebra: $\mathfrak{su}(4) \oplus \mathfrak{su}(5) \oplus \mathfrak{so}(10) \oplus \mathfrak{su}(2) \oplus \mathfrak{su}(2)$
$(\mathbf{1},\bar{\mathbf{5}},\mathbf{1},\mathbf{1},\mathbf{1})$, $(0,0,0,0,0,0,1,0,0,0,0,0,0,0) \mapsto (D,L)$
$(\mathbf{1},\mathbf{10},\mathbf{1},\mathbf{1},\mathbf{1})$, $(0,0,0,0,1,0,0,0,0,0,0,0,0,0) \mapsto (E,Q,U)$
$(\mathbf{1},\mathbf{1},\mathbf{16},\mathbf{1},\mathbf{1})$, $(0,0,0,0,0,0,0,0,0,0,0,1,0,0) \mapsto (D,E,L,N,Q,U)$
$(\bar{\mathbf{4}},\mathbf{1},\mathbf{1},\mathbf{2},\mathbf{1})$, $(0,0,1,0,0,0,0,0,0,0,0,0,1,0) \mapsto (L,Q)$
$(\mathbf{4},\mathbf{1},\mathbf{1},\mathbf{1},\mathbf{2})$, $(1,0,0,0,0,0,0,0,0,0,0,0,0,1) \mapsto (D,E,N,U)$
$(\mathbf{1},\mathbf{1},\mathbf{1},\mathbf{1},\mathbf{1})$, $(0,0,0,0,0,0,0,0,0,0,0,0,0,0) \mapsto (N)$
Projection matrix for $\alpha$:

$$\begin{pmatrix} 0 & 1 & 0 & 0 & 0 & 1 & 0 & 0 & 0 & 1 & 0 & 0 & 0 & 0 \\ 1 & 0 & 0 & 0 & 0 & 0 & 1 & 0 & 0 & 0 & 0 & 1 & 0 & 0 \\ 0 & 0 & 0 & 1 & 0 & 0 & 0 & 1 & 0 & 0 & 0 & 0 & 1 & 0 \\ -1 & -2 & -3 & 3 & 6 & 4 & 2 & 3 & 6 & 4 & 0 & 2 & 0 & 3 \end{pmatrix}$$

**3 generation subalgebra** 234
Algebra: $\mathfrak{su}(4) \oplus \mathfrak{su}(5) \oplus \mathfrak{sp}(4) \oplus \mathfrak{su}(2) \oplus \mathfrak{su}(2)$

$(\overline{\mathbf{4}}, \mathbf{1}, \mathbf{4}, \mathbf{1}, \mathbf{1})$, $(0,0,1,0,0,0,0,1,0,0,0) \mapsto (L, L, Q, Q)$
$(\mathbf{1}, \overline{\mathbf{5}}, \mathbf{1}, \mathbf{1}, \mathbf{1})$, $(0,0,0,0,0,0,1,0,0,0,0) \mapsto (D, L)$
$(\mathbf{1}, \mathbf{10}, \mathbf{1}, \mathbf{1}, \mathbf{1})$, $(0,0,0,0,1,0,0,0,0,0,0) \mapsto (E, Q, U)$
$(\mathbf{4}, \mathbf{1}, \mathbf{1}, \mathbf{2}, \mathbf{2})$, $(1,0,0,0,0,0,0,0,0,1,1) \mapsto (D, D, E, E, N, N, U, U)$
$(\mathbf{1}, \mathbf{1}, \mathbf{1}, \mathbf{1}, \mathbf{1})$, $(0,0,0,0,0,0,0,0,0,0,0) \mapsto (N)$
Projection matrix for $\alpha$:

$$\begin{pmatrix} 0 & 1 & 0 & 0 & 0 & 1 & 0 & 0 & 0 & 0 & 0 \\ 1 & 0 & 0 & 0 & 0 & 0 & 1 & 0 & 0 & 0 & 0 \\ 0 & 0 & 0 & 1 & 0 & 0 & 0 & 1 & 2 & 0 & 0 \\ -1 & -2 & -3 & 3 & 6 & 4 & 2 & 0 & 0 & 3 & 0 \end{pmatrix}$$

**3 generation subalgebra** 235
Algebra: $\mathfrak{su}(4) \oplus \mathfrak{su}(5) \oplus \mathfrak{sp}(4) \oplus \mathfrak{su}(2) \oplus \mathfrak{su}(2)$
$(\overline{\mathbf{4}}, \mathbf{1}, \mathbf{4}, \mathbf{1}, \mathbf{1})$, $(0,0,1,0,0,0,0,1,0,0,0) \mapsto (D, D, E, E, N, N, U, U)$
$(\mathbf{1}, \overline{\mathbf{5}}, \mathbf{1}, \mathbf{1}, \mathbf{1})$, $(0,0,0,0,0,0,1,0,0,0,0) \mapsto (D, L)$
$(\mathbf{1}, \mathbf{10}, \mathbf{1}, \mathbf{1}, \mathbf{1})$, $(0,0,0,0,1,0,0,0,0,0,0) \mapsto (E, Q, U)$
$(\mathbf{4}, \mathbf{1}, \mathbf{1}, \mathbf{2}, \mathbf{2})$, $(1,0,0,0,0,0,0,0,0,1,1) \mapsto (L, L, Q, Q)$
$(\mathbf{1}, \mathbf{1}, \mathbf{1}, \mathbf{1}, \mathbf{1})$, $(0,0,0,0,0,0,0,0,0,0,0) \mapsto (N)$
Projection matrix for $\alpha$:

$$\begin{pmatrix} 1 & 0 & 0 & 0 & 0 & 1 & 0 & 0 & 0 & 0 & 0 \\ 0 & 1 & 0 & 0 & 0 & 0 & 1 & 0 & 0 & 0 & 0 \\ 0 & 0 & 0 & 1 & 0 & 0 & 0 & 0 & 0 & 1 & 0 \\ 1 & 2 & 3 & 3 & 6 & 4 & 2 & 3 & 0 & 0 & 0 \end{pmatrix}$$

**3 generation subalgebra** 236
Algebra: $\mathfrak{su}(4) \oplus \mathfrak{su}(5) \oplus \mathfrak{sp}(4) \oplus \mathfrak{su}(2) \oplus \mathfrak{su}(2)$
$(\overline{\mathbf{4}}, \mathbf{1}, \mathbf{4}, \mathbf{1}, \mathbf{1})$, $(0,0,1,0,0,0,0,1,0,0,0) \mapsto (L, L, Q, Q)$
$(\mathbf{1}, \overline{\mathbf{5}}, \mathbf{1}, \mathbf{1}, \mathbf{1})$, $(0,0,0,0,0,0,1,0,0,0,0) \mapsto (D, L)$
$(\mathbf{1}, \mathbf{10}, \mathbf{1}, \mathbf{1}, \mathbf{1})$, $(0,0,0,0,1,0,0,0,0,0,0) \mapsto (E, Q, U)$
$(\mathbf{4}, \mathbf{1}, \mathbf{1}, \mathbf{2}, \mathbf{1})$, $(1,0,0,0,0,0,0,0,0,1,0) \mapsto (D, E, N, U)$
$(\mathbf{4}, \mathbf{1}, \mathbf{1}, \mathbf{1}, \mathbf{2})$, $(1,0,0,0,0,0,0,0,0,0,1) \mapsto (D, E, N, U)$
$(\mathbf{1}, \mathbf{1}, \mathbf{1}, \mathbf{1}, \mathbf{1})$, $(0,0,0,0,0,0,0,0,0,0,0) \mapsto (N)$
Projection matrix for $\alpha$:

$$\begin{pmatrix} 0 & 1 & 0 & 0 & 0 & 1 & 0 & 0 & 0 & 0 & 0 \\ 1 & 0 & 0 & 0 & 0 & 0 & 1 & 0 & 0 & 0 & 0 \\ 0 & 0 & 0 & 1 & 0 & 0 & 0 & 1 & 2 & 0 & 0 \\ -1 & -2 & -3 & 3 & 6 & 4 & 2 & 0 & 0 & 3 & 3 \end{pmatrix}$$

**3 generation subalgebra** 237
Algebra: $\mathfrak{su}(4) \oplus \mathfrak{su}(5) \oplus \mathfrak{sp}(4) \oplus \mathfrak{su}(2) \oplus \mathfrak{su}(2)$
$(\overline{\mathbf{4}}, \mathbf{1}, \mathbf{4}, \mathbf{1}, \mathbf{1})$, $(0,0,1,0,0,0,0,1,0,0,0) \mapsto (D, D, E, E, N, N, U, U)$
$(\mathbf{1}, \overline{\mathbf{5}}, \mathbf{1}, \mathbf{1}, \mathbf{1})$, $(0,0,0,0,0,0,1,0,0,0,0) \mapsto (D, L)$
$(\mathbf{1}, \mathbf{10}, \mathbf{1}, \mathbf{1}, \mathbf{1})$, $(0,0,0,0,1,0,0,0,0,0,0) \mapsto (E, Q, U)$
$(\mathbf{4}, \mathbf{1}, \mathbf{1}, \mathbf{2}, \mathbf{1})$, $(1,0,0,0,0,0,0,0,0,1,0) \mapsto (L, Q)$
$(\mathbf{4}, \mathbf{1}, \mathbf{1}, \mathbf{1}, \mathbf{2})$, $(1,0,0,0,0,0,0,0,0,0,1) \mapsto (L, Q)$
$(\mathbf{1}, \mathbf{1}, \mathbf{1}, \mathbf{1}, \mathbf{1})$, $(0,0,0,0,0,0,0,0,0,0,0) \mapsto (N)$
Projection matrix for $\alpha$:

$$\begin{pmatrix} 1 & 0 & 0 & 0 & 0 & 1 & 0 & 0 & 0 & 0 & 0 \\ 0 & 1 & 0 & 0 & 0 & 0 & 1 & 0 & 0 & 0 & 0 \\ 0 & 0 & 0 & 1 & 0 & 0 & 0 & 0 & 0 & 1 & 1 \\ 1 & 2 & 3 & 3 & 6 & 4 & 2 & 3 & 0 & 0 & 0 \end{pmatrix}$$

**3 generation subalgebra** 238
Algebra: $\mathfrak{su}(4) \oplus \mathfrak{su}(5) \oplus \mathfrak{su}(2) \oplus \mathfrak{su}(2) \oplus \mathfrak{su}(2)$
$(\mathbf{1}, \overline{\mathbf{5}}, \mathbf{1}, \mathbf{1}, \mathbf{1})$, $(0,0,0,0,0,0,1,0,0,0,0) \mapsto (D, L)$
$(\mathbf{1}, \mathbf{10}, \mathbf{1}, \mathbf{1}, \mathbf{1})$, $(0,0,0,0,1,0,0,0,0,0,0) \mapsto (E, Q, U)$

$(\mathbf{4},\mathbf{1},\mathbf{2},\mathbf{2},\mathbf{1}),\ (1,0,0,0,0,0,0,1,1,0)\mapsto(L,L,Q,Q)$
$(\overline{\mathbf{4}},\mathbf{1},\mathbf{2},\mathbf{1},\mathbf{2}),\ (0,0,1,0,0,0,0,1,0,1)\mapsto(D,D,E,E,N,N,U,U)$
$(\mathbf{1},\mathbf{1},\mathbf{1},\mathbf{1},\mathbf{1}),\ (0,0,0,0,0,0,0,0,0,0)\mapsto(N)$
Projection matrix for $\alpha$:

$$\begin{pmatrix}1&0&0&0&0&1&0&0&0&0\\0&1&0&0&0&0&1&0&0&0\\0&0&0&1&0&0&0&0&1&0\\1&2&3&3&6&4&2&0&0&3\end{pmatrix}$$

**3 generation subalgebra** 239
Algebra: $\mathfrak{su}(4)\oplus\mathfrak{su}(5)\oplus\mathfrak{su}(2)\oplus\mathfrak{su}(2)\oplus\mathfrak{su}(2)$
$(\overline{\mathbf{4}},\mathbf{1},\mathbf{2},\mathbf{1},\mathbf{1}),\ (0,0,1,0,0,0,0,1,0,0)\mapsto(L,Q)$
$(\mathbf{4},\mathbf{1},\mathbf{1},\mathbf{2},\mathbf{1}),\ (1,0,0,0,0,0,0,0,1,0)\mapsto(D,E,N,U)$
$(\mathbf{1},\overline{\mathbf{5}},\mathbf{1},\mathbf{1},\mathbf{2}),\ (0,0,0,0,0,0,1,0,0,1)\mapsto(D,D,L,L)$
$(\mathbf{1},\mathbf{10},\mathbf{1},\mathbf{1},\mathbf{2}),\ (0,0,0,0,1,0,0,0,0,1)\mapsto(E,E,Q,Q,U,U)$
$(\mathbf{1},\mathbf{1},\mathbf{1},\mathbf{1},\mathbf{1}),\ (0,0,0,0,0,0,0,0,0,0)\mapsto(N)$
$(\mathbf{1},\mathbf{1},\mathbf{1},\mathbf{1},\mathbf{1}),\ (0,0,0,0,0,0,0,0,0,0)\mapsto(N)$
Projection matrix for $\alpha$:

$$\begin{pmatrix}0&1&0&0&0&1&0&0&0&0\\1&0&0&0&0&0&1&0&0&0\\0&0&0&1&0&0&0&1&0&0\\-1&-2&-3&3&6&4&2&0&3&0\end{pmatrix}$$

**3 generation subalgebra** 240
Algebra: $\mathfrak{su}(4)\oplus\mathfrak{su}(5)\oplus\mathfrak{su}(2)\oplus\mathfrak{su}(2)\oplus\mathfrak{su}(2)$
$(\mathbf{1},\overline{\mathbf{5}},\mathbf{1},\mathbf{1},\mathbf{1}),\ (0,0,0,0,0,0,1,0,0,0)\mapsto(D,L)$
$(\mathbf{1},\overline{\mathbf{5}},\mathbf{1},\mathbf{1},\mathbf{1}),\ (0,0,0,0,0,0,1,0,0,0)\mapsto(D,L)$
$(\overline{\mathbf{4}},\mathbf{1},\mathbf{2},\mathbf{1},\mathbf{1}),\ (0,0,1,0,0,0,0,1,0,0)\mapsto(L,Q)$
$(\mathbf{4},\mathbf{1},\mathbf{1},\mathbf{2},\mathbf{1}),\ (1,0,0,0,0,0,0,0,1,0)\mapsto(D,E,N,U)$
$(\mathbf{1},\mathbf{10},\mathbf{1},\mathbf{1},\mathbf{2}),\ (0,0,0,0,1,0,0,0,0,1)\mapsto(E,E,Q,Q,U,U)$
$(\mathbf{1},\mathbf{1},\mathbf{1},\mathbf{1},\mathbf{1}),\ (0,0,0,0,0,0,0,0,0,0)\mapsto(N)$
$(\mathbf{1},\mathbf{1},\mathbf{1},\mathbf{1},\mathbf{1}),\ (0,0,0,0,0,0,0,0,0,0)\mapsto(N)$
Projection matrix for $\alpha$:

$$\begin{pmatrix}0&1&0&0&0&1&0&0&0&0\\1&0&0&0&0&0&1&0&0&0\\0&0&0&1&0&0&0&1&0&0\\-1&-2&-3&3&6&4&2&0&3&0\end{pmatrix}$$

**3 generation subalgebra** 241
Algebra: $\mathfrak{su}(4)\oplus\mathfrak{su}(5)\oplus\mathfrak{su}(2)\oplus\mathfrak{su}(2)\oplus\mathfrak{su}(2)$
$(\mathbf{1},\overline{\mathbf{5}},\mathbf{1},\mathbf{1},\mathbf{1}),\ (0,0,0,0,0,0,1,0,0,0)\mapsto(D,L)$
$(\mathbf{1},\mathbf{10},\mathbf{1},\mathbf{1},\mathbf{1}),\ (0,0,0,0,1,0,0,0,0,0)\mapsto(E,Q,U)$
$(\mathbf{4},\mathbf{1},\mathbf{2},\mathbf{2},\mathbf{1}),\ (1,0,0,0,0,0,0,1,1,0)\mapsto(D,D,E,E,N,N,U,U)$
$(\overline{\mathbf{4}},\mathbf{1},\mathbf{1},\mathbf{1},\mathbf{2}),\ (0,0,1,0,0,0,0,0,0,1)\mapsto(L,Q)$
$(\overline{\mathbf{4}},\mathbf{1},\mathbf{1},\mathbf{1},\mathbf{2}),\ (0,0,1,0,0,0,0,0,0,1)\mapsto(L,Q)$
$(\mathbf{1},\mathbf{1},\mathbf{1},\mathbf{1},\mathbf{1}),\ (0,0,0,0,0,0,0,0,0,0)\mapsto(N)$
Projection matrix for $\alpha$:

$$\begin{pmatrix}0&1&0&0&0&1&0&0&0&0\\1&0&0&0&0&0&1&0&0&0\\0&0&0&1&0&0&0&0&0&1\\-1&-2&-3&3&6&4&2&3&0&0\end{pmatrix}$$

**3 generation subalgebra** 242
Algebra: $\mathfrak{su}(4)\oplus\mathfrak{su}(5)\oplus\mathfrak{su}(2)\oplus\mathfrak{su}(2)\oplus\mathfrak{su}(2)$
$(\mathbf{1},\overline{\mathbf{5}},\mathbf{1},\mathbf{1},\mathbf{1}),\ (0,0,0,0,0,0,1,0,0,0)\mapsto(D,L)$
$(\mathbf{1},\mathbf{10},\mathbf{1},\mathbf{1},\mathbf{1}),\ (0,0,0,0,1,0,0,0,0,0)\mapsto(E,Q,U)$

$(\mathbf{4}, \mathbf{1}, \mathbf{2}, \mathbf{2}, \mathbf{1}),\ (1, 0, 0, 0, 0, 0, 0, 1, 1, 0) \mapsto (L, L, Q, Q)$
$(\overline{\mathbf{4}}, \mathbf{1}, \mathbf{1}, \mathbf{1}, \mathbf{2}),\ (0, 0, 1, 0, 0, 0, 0, 0, 0, 1) \mapsto (D, E, N, U)$
$(\overline{\mathbf{4}}, \mathbf{1}, \mathbf{1}, \mathbf{1}, \mathbf{2}),\ (0, 0, 1, 0, 0, 0, 0, 0, 0, 1) \mapsto (D, E, N, U)$
$(\mathbf{1}, \mathbf{1}, \mathbf{1}, \mathbf{1}, \mathbf{1}),\ (0, 0, 0, 0, 0, 0, 0, 0, 0, 0) \mapsto (N)$
Projection matrix for $\alpha$:

$$\begin{pmatrix} 1 & 0 & 0 & 0 & 0 & 1 & 0 & 0 & 0 & 0 \\ 0 & 1 & 0 & 0 & 0 & 0 & 1 & 0 & 0 & 0 \\ 0 & 0 & 0 & 1 & 0 & 0 & 0 & 1 & 0 & 0 \\ 1 & 2 & 3 & 3 & 6 & 4 & 2 & 0 & 0 & 3 \end{pmatrix}$$

**3 generation subalgebra** 243
Algebra: $\mathfrak{su}(4) \oplus \mathfrak{su}(5) \oplus \mathfrak{su}(2) \oplus \mathfrak{su}(2) \oplus \mathfrak{su}(2)$
$(\mathbf{1}, \mathbf{10}, \mathbf{1}, \mathbf{1}, \mathbf{1}),\ (0, 0, 0, 0, 1, 0, 0, 0, 0, 0) \mapsto (E, Q, U)$
$(\mathbf{1}, \mathbf{10}, \mathbf{1}, \mathbf{1}, \mathbf{1}),\ (0, 0, 0, 0, 1, 0, 0, 0, 0, 0) \mapsto (E, Q, U)$
$(\overline{\mathbf{4}}, \mathbf{1}, \mathbf{2}, \mathbf{1}, \mathbf{1}),\ (0, 0, 1, 0, 0, 0, 0, 1, 0, 0) \mapsto (L, Q)$
$(\mathbf{4}, \mathbf{1}, \mathbf{1}, \mathbf{2}, \mathbf{1}),\ (1, 0, 0, 0, 0, 0, 0, 0, 1, 0) \mapsto (D, E, N, U)$
$(\mathbf{1}, \overline{\mathbf{5}}, \mathbf{1}, \mathbf{1}, \mathbf{2}),\ (0, 0, 0, 0, 0, 0, 1, 0, 0, 1) \mapsto (D, D, L, L)$
$(\mathbf{1}, \mathbf{1}, \mathbf{1}, \mathbf{1}, \mathbf{1}),\ (0, 0, 0, 0, 0, 0, 0, 0, 0, 0) \mapsto (N)$
$(\mathbf{1}, \mathbf{1}, \mathbf{1}, \mathbf{1}, \mathbf{1}),\ (0, 0, 0, 0, 0, 0, 0, 0, 0, 0) \mapsto (N)$
Projection matrix for $\alpha$:

$$\begin{pmatrix} 0 & 1 & 0 & 0 & 0 & 1 & 0 & 0 & 0 & 0 \\ 1 & 0 & 0 & 0 & 0 & 0 & 1 & 0 & 0 & 0 \\ 0 & 0 & 0 & 1 & 0 & 0 & 0 & 1 & 0 & 0 \\ -1 & -2 & -3 & 3 & 6 & 4 & 2 & 0 & 3 & 0 \end{pmatrix}$$

**3 generation subalgebra** 244
Algebra: $\mathfrak{su}(4) \oplus \mathfrak{su}(5) \oplus \mathfrak{su}(2) \oplus \mathfrak{su}(2) \oplus \mathfrak{su}(2)$
$(\overline{\mathbf{4}}, \mathbf{1}, \mathbf{2}, \mathbf{1}, \mathbf{1}),\ (0, 0, 1, 0, 0, 0, 0, 1, 0, 0) \mapsto (L, Q)$
$(\mathbf{4}, \mathbf{1}, \mathbf{1}, \mathbf{2}, \mathbf{1}),\ (1, 0, 0, 0, 0, 0, 0, 0, 1, 0) \mapsto (D, E, N, U)$
$(\mathbf{1}, \overline{\mathbf{5}}, \mathbf{1}, \mathbf{1}, \mathbf{2}),\ (0, 0, 0, 0, 0, 0, 1, 0, 0, 1) \mapsto (D, D, L, L)$
$(\mathbf{1}, \mathbf{10}, \mathbf{1}, \mathbf{1}, \mathbf{2}),\ (0, 0, 0, 0, 1, 0, 0, 0, 0, 1) \mapsto (E, E, Q, Q, U, U)$
$(\mathbf{1}, \mathbf{1}, \mathbf{1}, \mathbf{1}, \mathbf{2}),\ (0, 0, 0, 0, 0, 0, 0, 0, 0, 1) \mapsto (N, N)$
Projection matrix for $\alpha$:

$$\begin{pmatrix} 0 & 1 & 0 & 0 & 0 & 1 & 0 & 0 & 0 & 0 \\ 1 & 0 & 0 & 0 & 0 & 0 & 1 & 0 & 0 & 0 \\ 0 & 0 & 0 & 1 & 0 & 0 & 0 & 1 & 0 & 0 \\ -1 & -2 & -3 & 3 & 6 & 4 & 2 & 0 & 3 & 0 \end{pmatrix}$$

**3 generation subalgebra** 245
Algebra: $\mathfrak{su}(4) \oplus \mathfrak{su}(5) \oplus \mathfrak{su}(2) \oplus \mathfrak{su}(2) \oplus \mathfrak{su}(2)$
$(\overline{\mathbf{4}}, \mathbf{1}, \mathbf{2}, \mathbf{1}, \mathbf{1}),\ (0, 0, 1, 0, 0, 0, 0, 1, 0, 0) \mapsto (L, Q)$
$(\mathbf{4}, \mathbf{1}, \mathbf{1}, \mathbf{2}, \mathbf{1}),\ (1, 0, 0, 0, 0, 0, 0, 0, 1, 0) \mapsto (D, E, N, U)$
$(\mathbf{1}, \overline{\mathbf{5}}, \mathbf{1}, \mathbf{1}, \mathbf{2}),\ (0, 0, 0, 0, 0, 0, 1, 0, 0, 1) \mapsto (D, D, L, L)$
$(\mathbf{1}, \mathbf{10}, \mathbf{1}, \mathbf{1}, \mathbf{2}),\ (0, 0, 0, 0, 1, 0, 0, 0, 0, 1) \mapsto (E, E, Q, Q, U, U)$
$(\mathbf{1}, \mathbf{1}, \mathbf{1}, \mathbf{2}, \mathbf{1}),\ (0, 0, 0, 0, 0, 0, 0, 0, 1, 0) \mapsto (N, N)$
Projection matrix for $\alpha$:

$$\begin{pmatrix} 0 & 1 & 0 & 0 & 0 & 1 & 0 & 0 & 0 & 0 \\ 1 & 0 & 0 & 0 & 0 & 0 & 1 & 0 & 0 & 0 \\ 0 & 0 & 0 & 1 & 0 & 0 & 0 & 1 & 0 & 0 \\ -1 & -2 & -3 & 3 & 6 & 4 & 2 & 0 & 3 & 0 \end{pmatrix}$$

**3 generation subalgebra** 246
Algebra: $\mathfrak{su}(4) \oplus \mathfrak{su}(5) \oplus \mathfrak{su}(2) \oplus \mathfrak{su}(2) \oplus \mathfrak{su}(2)$
$(\overline{\mathbf{4}}, \mathbf{1}, \mathbf{2}, \mathbf{1}, \mathbf{1}),\ (0, 0, 1, 0, 0, 0, 0, 1, 0, 0) \mapsto (L, Q)$
$(\mathbf{4}, \mathbf{1}, \mathbf{1}, \mathbf{2}, \mathbf{1}),\ (1, 0, 0, 0, 0, 0, 0, 0, 1, 0) \mapsto (D, E, N, U)$
$(\mathbf{1}, \overline{\mathbf{5}}, \mathbf{1}, \mathbf{1}, \mathbf{2}),\ (0, 0, 0, 0, 0, 0, 1, 0, 0, 1) \mapsto (D, D, L, L)$

$(\mathbf{1}, \mathbf{10}, \mathbf{1}, \mathbf{1}, \mathbf{2})$, $(0,0,0,0,1,0,0,0,0,1) \mapsto (E,E,Q,Q,U,U)$
$(\mathbf{1}, \mathbf{1}, \mathbf{2}, \mathbf{1}, \mathbf{1})$, $(0,0,0,0,0,0,0,1,0,0) \mapsto (N,N)$
Projection matrix for $\alpha$:

$$\begin{pmatrix} 0 & 1 & 0 & 0 & 0 & 1 & 0 & 0 & 0 & 0 \\ 1 & 0 & 0 & 0 & 0 & 0 & 1 & 0 & 0 & 0 \\ 0 & 0 & 0 & 1 & 0 & 0 & 0 & 1 & 0 & 0 \\ -1 & -2 & -3 & 3 & 6 & 4 & 2 & 0 & 3 & 0 \end{pmatrix}$$

**3 generation subalgebra** 247
Algebra: $\mathfrak{su}(4) \oplus \mathfrak{su}(5) \oplus \mathfrak{su}(2) \oplus \mathfrak{su}(2) \oplus \mathfrak{su}(2)$
$(\mathbf{1}, \overline{\mathbf{5}}, \mathbf{1}, \mathbf{1}, \mathbf{1})$, $(0,0,0,0,0,0,1,0,0,0) \mapsto (D,L)$
$(\mathbf{1}, \overline{\mathbf{5}}, \mathbf{1}, \mathbf{1}, \mathbf{1})$, $(0,0,0,0,0,0,1,0,0,0) \mapsto (D,L)$
$(\overline{\mathbf{4}}, \mathbf{1}, \mathbf{2}, \mathbf{1}, \mathbf{1})$, $(0,0,1,0,0,0,0,1,0,0) \mapsto (L,Q)$
$(\mathbf{4}, \mathbf{1}, \mathbf{1}, \mathbf{2}, \mathbf{1})$, $(1,0,0,0,0,0,0,0,1,0) \mapsto (D,E,N,U)$
$(\mathbf{1}, \mathbf{10}, \mathbf{1}, \mathbf{1}, \mathbf{2})$, $(0,0,0,0,1,0,0,0,0,1) \mapsto (E,E,Q,Q,U,U)$
$(\mathbf{1}, \mathbf{1}, \mathbf{1}, \mathbf{1}, \mathbf{2})$, $(0,0,0,0,0,0,0,0,0,1) \mapsto (N,N)$
Projection matrix for $\alpha$:

$$\begin{pmatrix} 0 & 1 & 0 & 0 & 0 & 1 & 0 & 0 & 0 & 0 \\ 1 & 0 & 0 & 0 & 0 & 0 & 1 & 0 & 0 & 0 \\ 0 & 0 & 0 & 1 & 0 & 0 & 0 & 1 & 0 & 0 \\ -1 & -2 & -3 & 3 & 6 & 4 & 2 & 0 & 3 & 0 \end{pmatrix}$$

**3 generation subalgebra** 248
Algebra: $\mathfrak{su}(4) \oplus \mathfrak{su}(5) \oplus \mathfrak{su}(2) \oplus \mathfrak{su}(2) \oplus \mathfrak{su}(2)$
$(\mathbf{1}, \overline{\mathbf{5}}, \mathbf{1}, \mathbf{1}, \mathbf{1})$, $(0,0,0,0,0,0,1,0,0,0) \mapsto (D,L)$
$(\mathbf{1}, \overline{\mathbf{5}}, \mathbf{1}, \mathbf{1}, \mathbf{1})$, $(0,0,0,0,0,0,1,0,0,0) \mapsto (D,L)$
$(\overline{\mathbf{4}}, \mathbf{1}, \mathbf{2}, \mathbf{1}, \mathbf{1})$, $(0,0,1,0,0,0,0,1,0,0) \mapsto (L,Q)$
$(\mathbf{4}, \mathbf{1}, \mathbf{1}, \mathbf{2}, \mathbf{1})$, $(1,0,0,0,0,0,0,0,1,0) \mapsto (D,E,N,U)$
$(\mathbf{1}, \mathbf{10}, \mathbf{1}, \mathbf{1}, \mathbf{2})$, $(0,0,0,0,1,0,0,0,0,1) \mapsto (E,E,Q,Q,U,U)$
$(\mathbf{1}, \mathbf{1}, \mathbf{1}, \mathbf{2}, \mathbf{1})$, $(0,0,0,0,0,0,0,0,1,0) \mapsto (N,N)$
Projection matrix for $\alpha$:

$$\begin{pmatrix} 0 & 1 & 0 & 0 & 0 & 1 & 0 & 0 & 0 & 0 \\ 1 & 0 & 0 & 0 & 0 & 0 & 1 & 0 & 0 & 0 \\ 0 & 0 & 0 & 1 & 0 & 0 & 0 & 1 & 0 & 0 \\ -1 & -2 & -3 & 3 & 6 & 4 & 2 & 0 & 3 & 0 \end{pmatrix}$$

**3 generation subalgebra** 249
Algebra: $\mathfrak{su}(4) \oplus \mathfrak{su}(5) \oplus \mathfrak{su}(2) \oplus \mathfrak{su}(2) \oplus \mathfrak{su}(2)$
$(\mathbf{1}, \overline{\mathbf{5}}, \mathbf{1}, \mathbf{1}, \mathbf{1})$, $(0,0,0,0,0,0,1,0,0,0) \mapsto (D,L)$
$(\mathbf{1}, \overline{\mathbf{5}}, \mathbf{1}, \mathbf{1}, \mathbf{1})$, $(0,0,0,0,0,0,1,0,0,0) \mapsto (D,L)$
$(\overline{\mathbf{4}}, \mathbf{1}, \mathbf{2}, \mathbf{1}, \mathbf{1})$, $(0,0,1,0,0,0,0,1,0,0) \mapsto (L,Q)$
$(\mathbf{4}, \mathbf{1}, \mathbf{1}, \mathbf{2}, \mathbf{1})$, $(1,0,0,0,0,0,0,0,1,0) \mapsto (D,E,N,U)$
$(\mathbf{1}, \mathbf{10}, \mathbf{1}, \mathbf{1}, \mathbf{2})$, $(0,0,0,0,1,0,0,0,0,1) \mapsto (E,E,Q,Q,U,U)$
$(\mathbf{1}, \mathbf{1}, \mathbf{2}, \mathbf{1}, \mathbf{1})$, $(0,0,0,0,0,0,0,1,0,0) \mapsto (N,N)$
Projection matrix for $\alpha$:

$$\begin{pmatrix} 0 & 1 & 0 & 0 & 0 & 1 & 0 & 0 & 0 & 0 \\ 1 & 0 & 0 & 0 & 0 & 0 & 1 & 0 & 0 & 0 \\ 0 & 0 & 0 & 1 & 0 & 0 & 0 & 1 & 0 & 0 \\ -1 & -2 & -3 & 3 & 6 & 4 & 2 & 0 & 3 & 0 \end{pmatrix}$$

**3 generation subalgebra** 250
Algebra: $\mathfrak{su}(4) \oplus \mathfrak{su}(5) \oplus \mathfrak{su}(2) \oplus \mathfrak{su}(2) \oplus \mathfrak{su}(2)$
$(\mathbf{1}, \overline{\mathbf{5}}, \mathbf{1}, \mathbf{1}, \mathbf{1})$, $(0,0,0,0,0,0,1,0,0,0) \mapsto (D,L)$
$(\mathbf{1}, \mathbf{10}, \mathbf{1}, \mathbf{1}, \mathbf{1})$, $(0,0,0,0,1,0,0,0,0,0) \mapsto (E,Q,U)$
$(\overline{\mathbf{4}}, \mathbf{1}, \mathbf{2}, \mathbf{1}, \mathbf{1})$, $(0,0,1,0,0,0,0,1,0,0) \mapsto (L,Q)$
$(\overline{\mathbf{4}}, \mathbf{1}, \mathbf{2}, \mathbf{1}, \mathbf{1})$, $(0,0,1,0,0,0,0,1,0,0) \mapsto (L,Q)$

$(\mathbf{4},\mathbf{1},\mathbf{1},\mathbf{2},\mathbf{1}),\ (1,0,0,0,0,0,0,0,1,0)\mapsto(D,E,N,U)$
$(\mathbf{4},\mathbf{1},\mathbf{1},\mathbf{1},\mathbf{2}),\ (1,0,0,0,0,0,0,0,0,1)\mapsto(D,E,N,U)$
$(\mathbf{1},\mathbf{1},\mathbf{1},\mathbf{1},\mathbf{1}),\ (0,0,0,0,0,0,0,0,0,0)\mapsto(N)$
Projection matrix for $\alpha$:

$$\begin{pmatrix} 0 & 1 & 0 & 0 & 0 & 1 & 0 & 0 & 0 & 0 \\ 1 & 0 & 0 & 0 & 0 & 0 & 1 & 0 & 0 & 0 \\ 0 & 0 & 0 & 1 & 0 & 0 & 0 & 1 & 0 & 0 \\ -1 & -2 & -3 & 3 & 6 & 4 & 2 & 0 & 3 & 3 \end{pmatrix}$$

**3 generation subalgebra** 251
Algebra: $\mathfrak{su}(4)\oplus\mathfrak{su}(5)\oplus\mathfrak{su}(2)\oplus\mathfrak{su}(2)\oplus\mathfrak{su}(2)$
$(\mathbf{1},\overline{\mathbf{5}},\mathbf{1},\mathbf{1},\mathbf{1}),\ (0,0,0,0,0,0,1,0,0,0)\mapsto(D,L)$
$(\mathbf{1},\mathbf{10},\mathbf{1},\mathbf{1},\mathbf{1}),\ (0,0,0,0,1,0,0,0,0,0)\mapsto(E,Q,U)$
$(\overline{\mathbf{4}},\mathbf{1},\mathbf{2},\mathbf{1},\mathbf{1}),\ (0,0,1,0,0,0,0,1,0,0)\mapsto(D,E,N,U)$
$(\overline{\mathbf{4}},\mathbf{1},\mathbf{2},\mathbf{1},\mathbf{1}),\ (0,0,1,0,0,0,0,1,0,0)\mapsto(D,E,N,U)$
$(\mathbf{4},\mathbf{1},\mathbf{1},\mathbf{2},\mathbf{1}),\ (1,0,0,0,0,0,0,0,1,0)\mapsto(L,Q)$
$(\mathbf{4},\mathbf{1},\mathbf{1},\mathbf{1},\mathbf{2}),\ (1,0,0,0,0,0,0,0,0,1)\mapsto(L,Q)$
$(\mathbf{1},\mathbf{1},\mathbf{1},\mathbf{1},\mathbf{1}),\ (0,0,0,0,0,0,0,0,0,0)\mapsto(N)$
Projection matrix for $\alpha$:

$$\begin{pmatrix} 1 & 0 & 0 & 0 & 0 & 1 & 0 & 0 & 0 & 0 \\ 0 & 1 & 0 & 0 & 0 & 0 & 1 & 0 & 0 & 0 \\ 0 & 0 & 0 & 1 & 0 & 0 & 0 & 0 & 1 & 1 \\ 1 & 2 & 3 & 3 & 6 & 4 & 2 & 3 & 0 & 0 \end{pmatrix}$$

**3 generation subalgebra** 252
Algebra: $\mathfrak{su}(4)\oplus\mathfrak{su}(5)\oplus\mathfrak{su}(2)\oplus\mathfrak{su}(2)\oplus\mathfrak{su}(2)$
$(\mathbf{1},\mathbf{10},\mathbf{1},\mathbf{1},\mathbf{1}),\ (0,0,0,0,1,0,0,0,0,0)\mapsto(E,Q,U)$
$(\mathbf{1},\mathbf{10},\mathbf{1},\mathbf{1},\mathbf{1}),\ (0,0,0,0,1,0,0,0,0,0)\mapsto(E,Q,U)$
$(\overline{\mathbf{4}},\mathbf{1},\mathbf{2},\mathbf{1},\mathbf{1}),\ (0,0,1,0,0,0,0,1,0,0)\mapsto(L,Q)$
$(\mathbf{4},\mathbf{1},\mathbf{1},\mathbf{2},\mathbf{1}),\ (1,0,0,0,0,0,0,0,1,0)\mapsto(D,E,N,U)$
$(\mathbf{1},\overline{\mathbf{5}},\mathbf{1},\mathbf{1},\mathbf{2}),\ (0,0,0,0,0,0,1,0,0,1)\mapsto(D,D,L,L)$
$(\mathbf{1},\mathbf{1},\mathbf{1},\mathbf{1},\mathbf{2}),\ (0,0,0,0,0,0,0,0,0,1)\mapsto(N,N)$
Projection matrix for $\alpha$:

$$\begin{pmatrix} 0 & 1 & 0 & 0 & 0 & 1 & 0 & 0 & 0 & 0 \\ 1 & 0 & 0 & 0 & 0 & 0 & 1 & 0 & 0 & 0 \\ 0 & 0 & 0 & 1 & 0 & 0 & 0 & 1 & 0 & 0 \\ -1 & -2 & -3 & 3 & 6 & 4 & 2 & 0 & 3 & 0 \end{pmatrix}$$

**3 generation subalgebra** 253
Algebra: $\mathfrak{su}(4)\oplus\mathfrak{su}(5)\oplus\mathfrak{su}(2)\oplus\mathfrak{su}(2)\oplus\mathfrak{su}(2)$
$(\mathbf{1},\mathbf{10},\mathbf{1},\mathbf{1},\mathbf{1}),\ (0,0,0,0,1,0,0,0,0,0)\mapsto(E,Q,U)$
$(\mathbf{1},\mathbf{10},\mathbf{1},\mathbf{1},\mathbf{1}),\ (0,0,0,0,1,0,0,0,0,0)\mapsto(E,Q,U)$
$(\overline{\mathbf{4}},\mathbf{1},\mathbf{2},\mathbf{1},\mathbf{1}),\ (0,0,1,0,0,0,0,1,0,0)\mapsto(L,Q)$
$(\mathbf{4},\mathbf{1},\mathbf{1},\mathbf{2},\mathbf{1}),\ (1,0,0,0,0,0,0,0,1,0)\mapsto(D,E,N,U)$
$(\mathbf{1},\overline{\mathbf{5}},\mathbf{1},\mathbf{1},\mathbf{2}),\ (0,0,0,0,0,0,1,0,0,1)\mapsto(D,D,L,L)$
$(\mathbf{1},\mathbf{1},\mathbf{1},\mathbf{2},\mathbf{1}),\ (0,0,0,0,0,0,0,0,1,0)\mapsto(N,N)$
Projection matrix for $\alpha$:

$$\begin{pmatrix} 0 & 1 & 0 & 0 & 0 & 1 & 0 & 0 & 0 & 0 \\ 1 & 0 & 0 & 0 & 0 & 0 & 1 & 0 & 0 & 0 \\ 0 & 0 & 0 & 1 & 0 & 0 & 0 & 1 & 0 & 0 \\ -1 & -2 & -3 & 3 & 6 & 4 & 2 & 0 & 3 & 0 \end{pmatrix}$$

**3 generation subalgebra** 254
Algebra: $\mathfrak{su}(4)\oplus\mathfrak{su}(5)\oplus\mathfrak{su}(2)\oplus\mathfrak{su}(2)\oplus\mathfrak{su}(2)$
$(\mathbf{1},\mathbf{10},\mathbf{1},\mathbf{1},\mathbf{1}),\ (0,0,0,0,1,0,0,0,0,0)\mapsto(E,Q,U)$
$(\mathbf{1},\mathbf{10},\mathbf{1},\mathbf{1},\mathbf{1}),\ (0,0,0,0,1,0,0,0,0,0)\mapsto(E,Q,U)$

$(\overline{\mathbf{4}}, \mathbf{1}, \mathbf{2}, \mathbf{1}, \mathbf{1})$, $(0,0,1,0,0,0,0,1,0,0) \mapsto (L, Q)$
$(\mathbf{4}, \mathbf{1}, \mathbf{1}, \mathbf{2}, \mathbf{1})$, $(1,0,0,0,0,0,0,0,1,0) \mapsto (D, E, N, U)$
$(\mathbf{1}, \overline{\mathbf{5}}, \mathbf{1}, \mathbf{1}, \mathbf{2})$, $(0,0,0,0,0,0,1,0,0,1) \mapsto (D, D, L, L)$
$(\mathbf{1}, \mathbf{1}, \mathbf{2}, \mathbf{1}, \mathbf{1})$, $(0,0,0,0,0,0,0,1,0,0) \mapsto (N, N)$
Projection matrix for $\alpha$:

$$\begin{pmatrix} 0 & 1 & 0 & 0 & 0 & 1 & 0 & 0 & 0 & 0 \\ 1 & 0 & 0 & 0 & 0 & 0 & 1 & 0 & 0 & 0 \\ 0 & 0 & 0 & 1 & 0 & 0 & 0 & 1 & 0 & 0 \\ -1 & -2 & -3 & 3 & 6 & 4 & 2 & 0 & 3 & 0 \end{pmatrix}$$

**3 generation subalgebra** 255
Algebra: $\mathfrak{su}(4) \oplus \mathfrak{su}(5) \oplus \mathfrak{su}(2) \oplus \mathfrak{su}(2) \oplus \mathfrak{su}(2)$
$(\mathbf{1}, \overline{\mathbf{5}}, \mathbf{1}, \mathbf{1}, \mathbf{1})$, $(0,0,0,0,0,0,1,0,0,0) \mapsto (D, L)$
$(\mathbf{1}, \overline{\mathbf{5}}, \mathbf{1}, \mathbf{1}, \mathbf{1})$, $(0,0,0,0,0,0,1,0,0,0) \mapsto (D, L)$
$(\mathbf{1}, \mathbf{10}, \mathbf{1}, \mathbf{1}, \mathbf{1})$, $(0,0,0,0,1,0,0,0,0,0) \mapsto (E, Q, U)$
$(\mathbf{1}, \mathbf{10}, \mathbf{1}, \mathbf{1}, \mathbf{1})$, $(0,0,0,0,1,0,0,0,0,0) \mapsto (E, Q, U)$
$(\overline{\mathbf{4}}, \mathbf{1}, \mathbf{2}, \mathbf{1}, \mathbf{1})$, $(0,0,1,0,0,0,0,1,0,0) \mapsto (L, Q)$
$(\mathbf{4}, \mathbf{1}, \mathbf{1}, \mathbf{2}, \mathbf{1})$, $(1,0,0,0,0,0,0,0,1,0) \mapsto (D, E, N, U)$
$(\mathbf{1}, \mathbf{1}, \mathbf{1}, \mathbf{1}, \mathbf{2})$, $(0,0,0,0,0,0,0,0,0,1) \mapsto (N, N)$
Projection matrix for $\alpha$:

$$\begin{pmatrix} 0 & 1 & 0 & 0 & 0 & 1 & 0 & 0 & 0 & 0 \\ 1 & 0 & 0 & 0 & 0 & 0 & 1 & 0 & 0 & 0 \\ 0 & 0 & 0 & 1 & 0 & 0 & 0 & 1 & 0 & 0 \\ -1 & -2 & -3 & 3 & 6 & 4 & 2 & 0 & 3 & 0 \end{pmatrix}$$

**3 generation subalgebra** 256
Algebra: $\mathfrak{su}(4) \oplus \mathfrak{su}(5) \oplus \mathfrak{su}(5) \oplus \mathfrak{su}(2) \oplus \mathfrak{su}(2)$
$(\mathbf{1}, \overline{\mathbf{5}}, \mathbf{1}, \mathbf{1}, \mathbf{1})$, $(0,0,0,0,0,0,1,0,0,0,0,0,0) \mapsto (D, L)$
$(\mathbf{1}, \mathbf{10}, \mathbf{1}, \mathbf{1}, \mathbf{1})$, $(0,0,0,0,1,0,0,0,0,0,0,0,0) \mapsto (E, Q, U)$
$(\mathbf{1}, \mathbf{1}, \overline{\mathbf{5}}, \mathbf{1}, \mathbf{1})$, $(0,0,0,0,0,0,0,0,0,0,1,0,0) \mapsto (D, L)$
$(\mathbf{1}, \mathbf{1}, \mathbf{10}, \mathbf{1}, \mathbf{1})$, $(0,0,0,0,0,0,0,0,1,0,0,0,0) \mapsto (E, Q, U)$
$(\overline{\mathbf{4}}, \mathbf{1}, \mathbf{1}, \mathbf{2}, \mathbf{1})$, $(0,0,1,0,0,0,0,0,0,0,0,1,0) \mapsto (L, Q)$
$(\mathbf{4}, \mathbf{1}, \mathbf{1}, \mathbf{1}, \mathbf{2})$, $(1,0,0,0,0,0,0,0,0,0,0,0,1) \mapsto (D, E, N, U)$
$(\mathbf{1}, \mathbf{1}, \mathbf{1}, \mathbf{1}, \mathbf{1})$, $(0,0,0,0,0,0,0,0,0,0,0,0,0) \mapsto (N)$
$(\mathbf{1}, \mathbf{1}, \mathbf{1}, \mathbf{1}, \mathbf{1})$, $(0,0,0,0,0,0,0,0,0,0,0,0,0) \mapsto (N)$
Projection matrix for $\alpha$:

$$\begin{pmatrix} 0 & 1 & 0 & 0 & 0 & 1 & 0 & 0 & 0 & 1 & 0 & 0 & 0 \\ 1 & 0 & 0 & 0 & 0 & 0 & 1 & 0 & 0 & 0 & 1 & 0 & 0 \\ 0 & 0 & 0 & 1 & 0 & 0 & 0 & 1 & 0 & 0 & 0 & 1 & 0 \\ -1 & -2 & -3 & 3 & 6 & 4 & 2 & 3 & 6 & 4 & 2 & 0 & 3 \end{pmatrix}$$

**3 generation subalgebra** 257
Algebra: $\mathfrak{su}(4) \oplus \mathfrak{su}(8) \oplus \mathfrak{su}(2) \oplus \mathfrak{su}(2) \oplus \mathfrak{su}(2)$
$(\overline{\mathbf{4}}, \mathbf{1}, \mathbf{2}, \mathbf{1}, \mathbf{1})$, $(0,0,1,0,0,0,0,0,0,0,1,0,0) \mapsto (L, Q)$
$(\mathbf{1}, \overline{\mathbf{8}}, \mathbf{2}, \mathbf{1}, \mathbf{1})$, $(0,0,0,0,0,0,0,0,0,1,1,0,0) \mapsto (L, L, Q, Q)$
$(\mathbf{4}, \mathbf{1}, \mathbf{1}, \mathbf{2}, \mathbf{1})$, $(1,0,0,0,0,0,0,0,0,0,0,1,0) \mapsto (D, E, N, U)$
$(\mathbf{1}, \mathbf{8}, \mathbf{1}, \mathbf{1}, \mathbf{2})$, $(0,0,0,1,0,0,0,0,0,0,0,0,1) \mapsto (D, D, E, E, N, N, U, U)$
Projection matrix for $\alpha$:

$$\begin{pmatrix} 0 & 1 & 0 & 0 & 1 & 0 & 0 & 1 & 0 & 0 & 0 & 0 & 0 \\ 1 & 0 & 0 & 1 & 0 & 0 & 1 & 0 & 0 & 0 & 0 & 0 & 0 \\ 0 & 0 & 0 & 0 & 0 & 0 & 0 & 0 & 0 & 0 & 1 & 0 & 0 \\ -1 & -2 & -3 & -1 & -2 & -3 & -4 & -5 & -6 & -3 & 0 & 3 & 3 \end{pmatrix}$$

**3 generation subalgebra** 258
Algebra: $\mathfrak{su}(4) \oplus \mathfrak{su}(8) \oplus \mathfrak{su}(2) \oplus \mathfrak{su}(2) \oplus \mathfrak{su}(2)$
$(\overline{\mathbf{4}}, \mathbf{1}, \mathbf{2}, \mathbf{1}, \mathbf{1})$, $(0,0,1,0,0,0,0,0,0,0,1,0,0) \mapsto (D, E, N, U)$

$(\mathbf{1},\overline{\mathbf{8}},\mathbf{2},\mathbf{1},\mathbf{1})$, $(0,0,0,0,0,0,0,0,0,1,1,0,0) \mapsto (D,D,E,E,N,N,U,U)$
$(\mathbf{4},\mathbf{1},\mathbf{1},\mathbf{2},\mathbf{1})$, $(1,0,0,0,0,0,0,0,0,0,0,1,0) \mapsto (L,Q)$
$(\mathbf{1},\mathbf{8},\mathbf{1},\mathbf{1},\mathbf{2})$, $(0,0,0,1,0,0,0,0,0,0,0,0,1) \mapsto (L,L,Q,Q)$
Projection matrix for $\alpha$:

$$\begin{pmatrix} 1&0&0&1&0&0&1&0&0&0&0&0&0 \\ 0&1&0&0&1&0&0&1&0&0&0&0&0 \\ 0&0&0&0&0&0&0&0&0&0&0&1&1 \\ 1&2&3&1&2&3&4&5&6&3&3&0&0 \end{pmatrix}$$

**3 generation subalgebra** 259
Algebra: $\mathfrak{su}(4) \oplus \mathfrak{so}(10) \oplus \mathfrak{su}(2) \oplus \mathfrak{su}(2) \oplus \mathfrak{su}(2) \oplus \mathfrak{su}(2)$
$(\mathbf{1},\mathbf{16},\mathbf{1},\mathbf{1},\mathbf{1},\mathbf{1})$, $(0,0,0,0,0,0,0,1,0,0,0,0) \mapsto (D,E,L,N,Q,U)$
$(\mathbf{4},\mathbf{1},\mathbf{2},\mathbf{2},\mathbf{1},\mathbf{1})$, $(1,0,0,0,0,0,0,0,1,1,0,0) \mapsto (D,D,E,E,N,N,U,U)$
$(\overline{\mathbf{4}},\mathbf{1},\mathbf{1},\mathbf{1},\mathbf{2},\mathbf{1})$, $(0,0,1,0,0,0,0,0,0,0,1,0) \mapsto (L,Q)$
$(\overline{\mathbf{4}},\mathbf{1},\mathbf{1},\mathbf{1},\mathbf{1},\mathbf{2})$, $(0,0,1,0,0,0,0,0,0,0,0,1) \mapsto (L,Q)$
Projection matrix for $\alpha$:

$$\begin{pmatrix} 0&1&0&0&0&1&0&0&0&0&0&0 \\ 1&0&0&0&0&0&0&1&0&0&0&0 \\ 0&0&0&1&0&0&0&0&0&0&1&1 \\ -1&-2&-3&3&6&4&0&2&3&0&0&0 \end{pmatrix}$$

**3 generation subalgebra** 260
Algebra: $\mathfrak{su}(4) \oplus \mathfrak{so}(10) \oplus \mathfrak{su}(2) \oplus \mathfrak{su}(2) \oplus \mathfrak{su}(2) \oplus \mathfrak{su}(2)$
$(\mathbf{1},\mathbf{16},\mathbf{1},\mathbf{1},\mathbf{1},\mathbf{1})$, $(0,0,0,0,0,0,0,1,0,0,0,0) \mapsto (D,E,L,N,Q,U)$
$(\mathbf{4},\mathbf{1},\mathbf{2},\mathbf{2},\mathbf{1},\mathbf{1})$, $(1,0,0,0,0,0,0,0,1,1,0,0) \mapsto (L,L,Q,Q)$
$(\overline{\mathbf{4}},\mathbf{1},\mathbf{1},\mathbf{1},\mathbf{2},\mathbf{1})$, $(0,0,1,0,0,0,0,0,0,0,1,0) \mapsto (D,E,N,U)$
$(\overline{\mathbf{4}},\mathbf{1},\mathbf{1},\mathbf{1},\mathbf{1},\mathbf{2})$, $(0,0,1,0,0,0,0,0,0,0,0,1) \mapsto (D,E,N,U)$
Projection matrix for $\alpha$:

$$\begin{pmatrix} 1&0&0&0&0&1&0&0&0&0&0&0 \\ 0&1&0&0&0&0&0&1&0&0&0&0 \\ 0&0&0&1&0&0&0&0&1&0&0&0 \\ 1&2&3&3&6&4&0&2&0&0&3&3 \end{pmatrix}$$

**3 generation subalgebra** 261
Algebra: $\mathfrak{su}(4) \oplus \mathfrak{so}(10) \oplus \mathfrak{su}(2) \oplus \mathfrak{su}(2) \oplus \mathfrak{su}(2) \oplus \mathfrak{su}(2)$
$(\mathbf{1},\mathbf{16},\mathbf{1},\mathbf{1},\mathbf{1},\mathbf{1})$, $(0,0,0,0,0,0,0,1,0,0,0,0) \mapsto (D,E,L,N,Q,U)$
$(\overline{\mathbf{4}},\mathbf{1},\mathbf{2},\mathbf{1},\mathbf{1},\mathbf{1})$, $(0,0,1,0,0,0,0,0,1,0,0,0) \mapsto (L,Q)$
$(\overline{\mathbf{4}},\mathbf{1},\mathbf{1},\mathbf{2},\mathbf{1},\mathbf{1})$, $(0,0,1,0,0,0,0,0,0,1,0,0) \mapsto (L,Q)$
$(\mathbf{4},\mathbf{1},\mathbf{1},\mathbf{1},\mathbf{2},\mathbf{1})$, $(1,0,0,0,0,0,0,0,0,0,1,0) \mapsto (D,E,N,U)$
$(\mathbf{4},\mathbf{1},\mathbf{1},\mathbf{1},\mathbf{1},\mathbf{2})$, $(1,0,0,0,0,0,0,0,0,0,0,1) \mapsto (D,E,N,U)$
Projection matrix for $\alpha$:

$$\begin{pmatrix} 0&1&0&0&0&1&0&0&0&0&0&0 \\ 1&0&0&0&0&0&0&1&0&0&0&0 \\ 0&0&0&1&0&0&0&0&1&1&0&0 \\ -1&-2&-3&3&6&4&0&2&0&0&3&3 \end{pmatrix}$$

**3 generation subalgebra** 262
Algebra: $\mathfrak{su}(4) \oplus \mathfrak{sp}(4) \oplus \mathfrak{su}(2) \oplus \mathfrak{su}(2) \oplus \mathfrak{su}(2) \oplus \mathfrak{su}(2)$
$(\overline{\mathbf{4}},\mathbf{4},\mathbf{1},\mathbf{1},\mathbf{1},\mathbf{1})$, $(0,0,1,1,0,0,0,0,0) \mapsto (L,L,Q,Q)$
$(\mathbf{4},\mathbf{1},\mathbf{2},\mathbf{2},\mathbf{1},\mathbf{1})$, $(1,0,0,0,0,1,1,0,0) \mapsto (D,D,E,E,N,N,U,U)$
$(\overline{\mathbf{4}},\mathbf{1},\mathbf{1},\mathbf{1},\mathbf{2},\mathbf{1})$, $(0,0,1,0,0,0,0,1,0) \mapsto (L,Q)$
$(\mathbf{4},\mathbf{1},\mathbf{1},\mathbf{1},\mathbf{1},\mathbf{2})$, $(1,0,0,0,0,0,0,0,1) \mapsto (D,E,N,U)$
Projection matrix for $\alpha$:

$$\begin{pmatrix} 0&1&0&0&0&0&0&0&0 \\ 1&0&0&0&0&0&0&0&0 \\ 0&0&0&1&2&0&0&1&0 \\ -1&-2&-3&0&0&3&0&0&3 \end{pmatrix}$$

**3 generation subalgebra** 263
Algebra: $\mathfrak{su}(4) \oplus \mathfrak{sp}(4) \oplus \mathfrak{su}(2) \oplus \mathfrak{su}(2) \oplus \mathfrak{su}(2) \oplus \mathfrak{su}(2)$
$(\overline{\mathbf{4}}, \mathbf{4}, \mathbf{1}, \mathbf{1}, \mathbf{1}, \mathbf{1})$, $(0, 0, 1, 1, 0, 0, 0, 0, 0) \mapsto (D, D, E, E, N, N, U, U)$
$(\mathbf{4}, \mathbf{1}, \mathbf{2}, \mathbf{2}, \mathbf{1}, \mathbf{1})$, $(1, 0, 0, 0, 0, 1, 1, 0, 0) \mapsto (L, L, Q, Q)$
$(\overline{\mathbf{4}}, \mathbf{1}, \mathbf{1}, \mathbf{1}, \mathbf{2}, \mathbf{1})$, $(0, 0, 1, 0, 0, 0, 0, 1, 0) \mapsto (D, E, N, U)$
$(\mathbf{4}, \mathbf{1}, \mathbf{1}, \mathbf{1}, \mathbf{1}, \mathbf{2})$, $(1, 0, 0, 0, 0, 0, 0, 0, 1) \mapsto (L, Q)$
Projection matrix for $\alpha$:

$$\begin{pmatrix} 1 & 0 & 0 & 0 & 0 & 0 & 0 & 0 & 0 \\ 0 & 1 & 0 & 0 & 0 & 0 & 0 & 0 & 0 \\ 0 & 0 & 0 & 0 & 0 & 1 & 0 & 0 & 1 \\ 1 & 2 & 3 & 3 & 0 & 0 & 0 & 3 & 0 \end{pmatrix}$$

**3 generation subalgebra** 264
Algebra: $\mathfrak{su}(4) \oplus \mathfrak{sp}(4) \oplus \mathfrak{su}(2) \oplus \mathfrak{su}(2) \oplus \mathfrak{su}(2) \oplus \mathfrak{su}(2)$
$(\overline{\mathbf{4}}, \mathbf{4}, \mathbf{1}, \mathbf{1}, \mathbf{1}, \mathbf{1})$, $(0, 0, 1, 1, 0, 0, 0, 0, 0) \mapsto (L, L, Q, Q)$
$(\overline{\mathbf{4}}, \mathbf{1}, \mathbf{2}, \mathbf{1}, \mathbf{1}, \mathbf{1})$, $(0, 0, 1, 0, 0, 1, 0, 0, 0) \mapsto (L, Q)$
$(\mathbf{4}, \mathbf{1}, \mathbf{1}, \mathbf{2}, \mathbf{1}, \mathbf{1})$, $(1, 0, 0, 0, 0, 0, 1, 0, 0) \mapsto (D, E, N, U)$
$(\mathbf{4}, \mathbf{1}, \mathbf{1}, \mathbf{1}, \mathbf{2}, \mathbf{1})$, $(1, 0, 0, 0, 0, 0, 0, 1, 0) \mapsto (D, E, N, U)$
$(\mathbf{4}, \mathbf{1}, \mathbf{1}, \mathbf{1}, \mathbf{1}, \mathbf{2})$, $(1, 0, 0, 0, 0, 0, 0, 0, 1) \mapsto (D, E, N, U)$
Projection matrix for $\alpha$:

$$\begin{pmatrix} 0 & 1 & 0 & 0 & 0 & 0 & 0 & 0 & 0 \\ 1 & 0 & 0 & 0 & 0 & 0 & 0 & 0 & 0 \\ 0 & 0 & 0 & 1 & 2 & 1 & 0 & 0 & 0 \\ -1 & -2 & -3 & 0 & 0 & 0 & 3 & 3 & 3 \end{pmatrix}$$

**3 generation subalgebra** 265
Algebra: $\mathfrak{su}(4) \oplus \mathfrak{sp}(4) \oplus \mathfrak{su}(2) \oplus \mathfrak{su}(2) \oplus \mathfrak{su}(2) \oplus \mathfrak{su}(2)$
$(\overline{\mathbf{4}}, \mathbf{4}, \mathbf{1}, \mathbf{1}, \mathbf{1}, \mathbf{1})$, $(0, 0, 1, 1, 0, 0, 0, 0, 0) \mapsto (D, D, E, E, N, N, U, U)$
$(\overline{\mathbf{4}}, \mathbf{1}, \mathbf{2}, \mathbf{1}, \mathbf{1}, \mathbf{1})$, $(0, 0, 1, 0, 0, 1, 0, 0, 0) \mapsto (D, E, N, U)$
$(\mathbf{4}, \mathbf{1}, \mathbf{1}, \mathbf{2}, \mathbf{1}, \mathbf{1})$, $(1, 0, 0, 0, 0, 0, 1, 0, 0) \mapsto (L, Q)$
$(\mathbf{4}, \mathbf{1}, \mathbf{1}, \mathbf{1}, \mathbf{2}, \mathbf{1})$, $(1, 0, 0, 0, 0, 0, 0, 1, 0) \mapsto (L, Q)$
$(\mathbf{4}, \mathbf{1}, \mathbf{1}, \mathbf{1}, \mathbf{1}, \mathbf{2})$, $(1, 0, 0, 0, 0, 0, 0, 0, 1) \mapsto (L, Q)$
Projection matrix for $\alpha$:

$$\begin{pmatrix} 1 & 0 & 0 & 0 & 0 & 0 & 0 & 0 & 0 \\ 0 & 1 & 0 & 0 & 0 & 0 & 0 & 0 & 0 \\ 0 & 0 & 0 & 0 & 0 & 0 & 1 & 1 & 1 \\ 1 & 2 & 3 & 3 & 0 & 3 & 0 & 0 & 0 \end{pmatrix}$$

**3 generation subalgebra** 266
Algebra: $\mathfrak{su}(4) \oplus \mathfrak{su}(2) \oplus \mathfrak{su}(2) \oplus \mathfrak{su}(2) \oplus \mathfrak{su}(2) \oplus \mathfrak{su}(2)$
$(\mathbf{4}, \mathbf{2}, \mathbf{2}, \mathbf{1}, \mathbf{1}, \mathbf{1})$, $(1, 0, 0, 1, 1, 0, 0, 0) \mapsto (D, D, E, E, N, N, U, U)$
$(\overline{\mathbf{4}}, \mathbf{1}, \mathbf{1}, \mathbf{3}, \mathbf{2}, \mathbf{1})$, $(0, 0, 1, 0, 0, 2, 1, 0) \mapsto (L, L, L, Q, Q, Q)$
$(\mathbf{4}, \mathbf{1}, \mathbf{1}, \mathbf{1}, \mathbf{1}, \mathbf{2})$, $(1, 0, 0, 0, 0, 0, 0, 1) \mapsto (D, E, N, U)$
Projection matrix for $\alpha$:

$$\begin{pmatrix} 0 & 1 & 0 & 0 & 0 & 0 & 0 & 0 \\ 1 & 0 & 0 & 0 & 0 & 0 & 0 & 0 \\ 0 & 0 & 0 & 0 & 0 & 0 & 1 & 0 \\ -1 & -2 & -3 & 3 & 0 & 0 & 0 & 3 \end{pmatrix}$$

**3 generation subalgebra** 267
Algebra: $\mathfrak{su}(4) \oplus \mathfrak{su}(2) \oplus \mathfrak{su}(2) \oplus \mathfrak{su}(2) \oplus \mathfrak{su}(2) \oplus \mathfrak{su}(2)$
$(\mathbf{4}, \mathbf{2}, \mathbf{2}, \mathbf{1}, \mathbf{1}, \mathbf{1})$, $(1, 0, 0, 1, 1, 0, 0, 0) \mapsto (L, L, Q, Q)$
$(\overline{\mathbf{4}}, \mathbf{1}, \mathbf{1}, \mathbf{3}, \mathbf{2}, \mathbf{1})$, $(0, 0, 1, 0, 0, 2, 1, 0) \mapsto (D, D, D, E, E, E, N, N, N, U, U, U)$
$(\mathbf{4}, \mathbf{1}, \mathbf{1}, \mathbf{1}, \mathbf{1}, \mathbf{2})$, $(1, 0, 0, 0, 0, 0, 0, 1) \mapsto (L, Q)$

Projection matrix for $\alpha$:

$$\begin{pmatrix} 1 & 0 & 0 & 0 & 0 & 0 & 0 & 0 \\ 0 & 1 & 0 & 0 & 0 & 0 & 0 & 0 \\ 0 & 0 & 0 & 1 & 0 & 0 & 0 & 1 \\ 1 & 2 & 3 & 0 & 0 & 0 & 3 & 0 \end{pmatrix}$$

**3 generation subalgebra** 268
Algebra: $\mathfrak{su}(4) \oplus \mathfrak{su}(2) \oplus \mathfrak{su}(2) \oplus \mathfrak{su}(2) \oplus \mathfrak{su}(2) \oplus \mathfrak{su}(2)$
$(\mathbf{4}, \mathbf{2}, \mathbf{2}, \mathbf{1}, \mathbf{1}, \mathbf{1})$, $(1, 0, 0, 1, 1, 0, 0, 0) \mapsto (D, D, E, E, N, N, U, U)$
$(\overline{\mathbf{4}}, \mathbf{2}, \mathbf{1}, \mathbf{2}, \mathbf{1}, \mathbf{1})$, $(0, 0, 1, 1, 0, 1, 0, 0) \mapsto (L, L, Q, Q)$
$(\overline{\mathbf{4}}, \mathbf{1}, \mathbf{1}, \mathbf{1}, \mathbf{2}, \mathbf{1})$, $(0, 0, 1, 0, 0, 0, 1, 0) \mapsto (L, Q)$
$(\mathbf{4}, \mathbf{1}, \mathbf{1}, \mathbf{1}, \mathbf{1}, \mathbf{2})$, $(1, 0, 0, 0, 0, 0, 0, 1) \mapsto (D, E, N, U)$
Projection matrix for $\alpha$:

$$\begin{pmatrix} 0 & 1 & 0 & 0 & 0 & 0 & 0 & 0 \\ 1 & 0 & 0 & 0 & 0 & 0 & 0 & 0 \\ 0 & 0 & 0 & 0 & 0 & 1 & 1 & 0 \\ -1 & -2 & -3 & 0 & 3 & 0 & 0 & 3 \end{pmatrix}$$

**3 generation subalgebra** 269
Algebra: $\mathfrak{su}(4) \oplus \mathfrak{su}(2) \oplus \mathfrak{su}(2) \oplus \mathfrak{su}(2) \oplus \mathfrak{su}(2) \oplus \mathfrak{su}(2)$
$(\mathbf{4}, \mathbf{2}, \mathbf{2}, \mathbf{1}, \mathbf{1}, \mathbf{1})$, $(1, 0, 0, 1, 1, 0, 0, 0) \mapsto (D, D, E, E, N, N, U, U)$
$(\mathbf{4}, \mathbf{2}, \mathbf{1}, \mathbf{1}, \mathbf{1}, \mathbf{1})$, $(1, 0, 0, 1, 0, 0, 0, 0) \mapsto (D, E, N, U)$
$(\overline{\mathbf{4}}, \mathbf{1}, \mathbf{1}, \mathbf{2}, \mathbf{2}, \mathbf{1})$, $(0, 0, 1, 0, 0, 1, 1, 0) \mapsto (L, L, Q, Q)$
$(\overline{\mathbf{4}}, \mathbf{1}, \mathbf{1}, \mathbf{1}, \mathbf{1}, \mathbf{2})$, $(0, 0, 1, 0, 0, 0, 0, 1) \mapsto (L, Q)$
Projection matrix for $\alpha$:

$$\begin{pmatrix} 0 & 1 & 0 & 0 & 0 & 0 & 0 & 0 \\ 1 & 0 & 0 & 0 & 0 & 0 & 0 & 0 \\ 0 & 0 & 0 & 0 & 0 & 1 & 0 & 1 \\ -1 & -2 & -3 & 3 & 0 & 0 & 0 & 0 \end{pmatrix}$$

**3 generation subalgebra** 270
Algebra: $\mathfrak{su}(4) \oplus \mathfrak{su}(2) \oplus \mathfrak{su}(2) \oplus \mathfrak{su}(2) \oplus \mathfrak{su}(2) \oplus \mathfrak{su}(2)$
$(\mathbf{4}, \mathbf{2}, \mathbf{2}, \mathbf{1}, \mathbf{1}, \mathbf{1})$, $(1, 0, 0, 1, 1, 0, 0, 0) \mapsto (L, L, Q, Q)$
$(\mathbf{4}, \mathbf{2}, \mathbf{1}, \mathbf{1}, \mathbf{1}, \mathbf{1})$, $(1, 0, 0, 1, 0, 0, 0, 0) \mapsto (L, Q)$
$(\overline{\mathbf{4}}, \mathbf{1}, \mathbf{1}, \mathbf{2}, \mathbf{2}, \mathbf{1})$, $(0, 0, 1, 0, 0, 1, 1, 0) \mapsto (D, D, E, E, N, N, U, U)$
$(\overline{\mathbf{4}}, \mathbf{1}, \mathbf{1}, \mathbf{1}, \mathbf{1}, \mathbf{2})$, $(0, 0, 1, 0, 0, 0, 0, 1) \mapsto (D, E, N, U)$
Projection matrix for $\alpha$:

$$\begin{pmatrix} 1 & 0 & 0 & 0 & 0 & 0 & 0 & 0 \\ 0 & 1 & 0 & 0 & 0 & 0 & 0 & 0 \\ 0 & 0 & 0 & 1 & 0 & 0 & 0 & 0 \\ 1 & 2 & 3 & 0 & 0 & 3 & 0 & 3 \end{pmatrix}$$

**3 generation subalgebra** 271
Algebra: $\mathfrak{su}(4) \oplus \mathfrak{su}(2) \oplus \mathfrak{su}(2) \oplus \mathfrak{su}(2) \oplus \mathfrak{su}(2) \oplus \mathfrak{su}(2)$
$(\mathbf{4}, \mathbf{3}, \mathbf{2}, \mathbf{1}, \mathbf{1}, \mathbf{1})$, $(1, 0, 0, 2, 1, 0, 0, 0) \mapsto (D, D, D, E, E, E, N, N, N, U, U, U)$
$(\overline{\mathbf{4}}, \mathbf{1}, \mathbf{1}, \mathbf{2}, \mathbf{1}, \mathbf{1})$, $(0, 0, 1, 0, 0, 1, 0, 0) \mapsto (L, Q)$
$(\overline{\mathbf{4}}, \mathbf{1}, \mathbf{1}, \mathbf{1}, \mathbf{2}, \mathbf{1})$, $(0, 0, 1, 0, 0, 0, 1, 0) \mapsto (L, Q)$
$(\overline{\mathbf{4}}, \mathbf{1}, \mathbf{1}, \mathbf{1}, \mathbf{1}, \mathbf{2})$, $(0, 0, 1, 0, 0, 0, 0, 1) \mapsto (L, Q)$
Projection matrix for $\alpha$:

$$\begin{pmatrix} 0 & 1 & 0 & 0 & 0 & 0 & 0 & 0 \\ 1 & 0 & 0 & 0 & 0 & 0 & 0 & 0 \\ 0 & 0 & 0 & 0 & 0 & 1 & 1 & 1 \\ -1 & -2 & -3 & 0 & 3 & 0 & 0 & 0 \end{pmatrix}$$

**3 generation subalgebra** 272
Algebra: $\mathfrak{su}(4) \oplus \mathfrak{su}(2) \oplus \mathfrak{su}(2) \oplus \mathfrak{su}(2) \oplus \mathfrak{su}(2) \oplus \mathfrak{su}(2)$

$(\mathbf{4},\mathbf{3},\mathbf{2},\mathbf{1},\mathbf{1},\mathbf{1}),\ (1,0,0,2,1,0,0,0)\mapsto(L,L,L,Q,Q,Q)$
$(\overline{\mathbf{4}},\mathbf{1},\mathbf{1},\mathbf{2},\mathbf{1},\mathbf{1}),\ (0,0,1,0,0,1,0,0)\mapsto(D,E,N,U)$
$(\overline{\mathbf{4}},\mathbf{1},\mathbf{1},\mathbf{1},\mathbf{2},\mathbf{1}),\ (0,0,1,0,0,0,1,0)\mapsto(D,E,N,U)$
$(\overline{\mathbf{4}},\mathbf{1},\mathbf{1},\mathbf{1},\mathbf{1},\mathbf{2}),\ (0,0,1,0,0,0,0,1)\mapsto(D,E,N,U)$
Projection matrix for $\alpha$:

$$\begin{pmatrix}1&0&0&0&0&0&0&0\\0&1&0&0&0&0&0&0\\0&0&0&0&1&0&0&0\\1&2&3&0&0&3&3&3\end{pmatrix}$$

**3 generation subalgebra** 273
Algebra: $\mathfrak{su}(4)\oplus\mathfrak{su}(2)\oplus\mathfrak{su}(2)\oplus\mathfrak{su}(2)\oplus\mathfrak{su}(2)\oplus\mathfrak{su}(2)$
$(\mathbf{4},\mathbf{2},\mathbf{2},\mathbf{1},\mathbf{1},\mathbf{1}),\ (1,0,0,1,1,0,0,0)\mapsto(D,D,E,E,N,N,U,U)$
$(\overline{\mathbf{4}},\mathbf{1},\mathbf{1},\mathbf{2},\mathbf{1},\mathbf{1}),\ (0,0,1,0,0,1,0,0)\mapsto(L,Q)$
$(\overline{\mathbf{4}},\mathbf{1},\mathbf{1},\mathbf{2},\mathbf{1},\mathbf{1}),\ (0,0,1,0,0,1,0,0)\mapsto(L,Q)$
$(\overline{\mathbf{4}},\mathbf{1},\mathbf{1},\mathbf{1},\mathbf{2},\mathbf{1}),\ (0,0,1,0,0,0,1,0)\mapsto(L,Q)$
$(\mathbf{4},\mathbf{1},\mathbf{1},\mathbf{1},\mathbf{1},\mathbf{2}),\ (1,0,0,0,0,0,0,1)\mapsto(D,E,N,U)$
Projection matrix for $\alpha$:

$$\begin{pmatrix}0&1&0&0&0&0&0&0\\1&0&0&0&0&0&0&0\\0&0&0&0&0&1&1&0\\-1&-2&-3&3&0&0&0&3\end{pmatrix}$$

**3 generation subalgebra** 274
Algebra: $\mathfrak{su}(4)\oplus\mathfrak{su}(2)\oplus\mathfrak{su}(2)\oplus\mathfrak{su}(2)\oplus\mathfrak{su}(2)\oplus\mathfrak{su}(2)$
$(\mathbf{4},\mathbf{2},\mathbf{2},\mathbf{1},\mathbf{1},\mathbf{1}),\ (1,0,0,1,1,0,0,0)\mapsto(L,L,Q,Q)$
$(\overline{\mathbf{4}},\mathbf{1},\mathbf{1},\mathbf{2},\mathbf{1},\mathbf{1}),\ (0,0,1,0,0,1,0,0)\mapsto(D,E,N,U)$
$(\overline{\mathbf{4}},\mathbf{1},\mathbf{1},\mathbf{2},\mathbf{1},\mathbf{1}),\ (0,0,1,0,0,1,0,0)\mapsto(D,E,N,U)$
$(\overline{\mathbf{4}},\mathbf{1},\mathbf{1},\mathbf{1},\mathbf{2},\mathbf{1}),\ (0,0,1,0,0,0,1,0)\mapsto(D,E,N,U)$
$(\mathbf{4},\mathbf{1},\mathbf{1},\mathbf{1},\mathbf{1},\mathbf{2}),\ (1,0,0,0,0,0,0,1)\mapsto(L,Q)$
Projection matrix for $\alpha$:

$$\begin{pmatrix}1&0&0&0&0&0&0&0\\0&1&0&0&0&0&0&0\\0&0&0&1&0&0&0&1\\1&2&3&0&0&3&3&0\end{pmatrix}$$

**3 generation subalgebra** 275
Algebra: $\mathfrak{su}(4)\oplus\mathfrak{su}(2)\oplus\mathfrak{su}(2)\oplus\mathfrak{su}(2)\oplus\mathfrak{su}(2)\oplus\mathfrak{su}(2)$
$(\mathbf{4},\mathbf{2},\mathbf{2},\mathbf{1},\mathbf{1},\mathbf{1}),\ (1,0,0,1,1,0,0,0)\mapsto(D,D,E,E,N,N,U,U)$
$(\mathbf{4},\mathbf{2},\mathbf{1},\mathbf{1},\mathbf{1},\mathbf{1}),\ (1,0,0,1,0,0,0,0)\mapsto(D,E,N,U)$
$(\overline{\mathbf{4}},\mathbf{1},\mathbf{1},\mathbf{2},\mathbf{1},\mathbf{1}),\ (0,0,1,0,0,1,0,0)\mapsto(L,Q)$
$(\overline{\mathbf{4}},\mathbf{1},\mathbf{1},\mathbf{1},\mathbf{2},\mathbf{1}),\ (0,0,1,0,0,0,1,0)\mapsto(L,Q)$
$(\overline{\mathbf{4}},\mathbf{1},\mathbf{1},\mathbf{1},\mathbf{1},\mathbf{2}),\ (0,0,1,0,0,0,0,1)\mapsto(L,Q)$
Projection matrix for $\alpha$:

$$\begin{pmatrix}0&1&0&0&0&0&0&0\\1&0&0&0&0&0&0&0\\0&0&0&0&0&1&1&1\\-1&-2&-3&3&0&0&0&0\end{pmatrix}$$

**3 generation subalgebra** 276
Algebra: $\mathfrak{su}(4)\oplus\mathfrak{su}(2)\oplus\mathfrak{su}(2)\oplus\mathfrak{su}(2)\oplus\mathfrak{su}(2)\oplus\mathfrak{su}(2)$
$(\mathbf{4},\mathbf{2},\mathbf{2},\mathbf{1},\mathbf{1},\mathbf{1}),\ (1,0,0,1,1,0,0,0)\mapsto(L,L,Q,Q)$
$(\mathbf{4},\mathbf{2},\mathbf{1},\mathbf{1},\mathbf{1},\mathbf{1}),\ (1,0,0,1,0,0,0,0)\mapsto(L,Q)$
$(\overline{\mathbf{4}},\mathbf{1},\mathbf{1},\mathbf{2},\mathbf{1},\mathbf{1}),\ (0,0,1,0,0,1,0,0)\mapsto(D,E,N,U)$
$(\overline{\mathbf{4}},\mathbf{1},\mathbf{1},\mathbf{1},\mathbf{2},\mathbf{1}),\ (0,0,1,0,0,0,1,0)\mapsto(D,E,N,U)$

$(\overline{\mathbf{4}}, \mathbf{1}, \mathbf{1}, \mathbf{1}, \mathbf{1}, \mathbf{2})$, $(0,0,1,0,0,0,0,1) \mapsto (D,E,N,U)$
Projection matrix for $\alpha$:

$$\begin{pmatrix} 1 & 0 & 0 & 0 & 0 & 0 & 0 & 0 \\ 0 & 1 & 0 & 0 & 0 & 0 & 0 & 0 \\ 0 & 0 & 0 & 1 & 0 & 0 & 0 & 0 \\ 1 & 2 & 3 & 0 & 0 & 3 & 3 & 3 \end{pmatrix}$$

**3 generation subalgebra** 277
Algebra: $\mathfrak{su}(4) \oplus \mathfrak{su}(2) \oplus \mathfrak{su}(2) \oplus \mathfrak{su}(2) \oplus \mathfrak{su}(2) \oplus \mathfrak{su}(2)$
$(\overline{\mathbf{4}}, \mathbf{2}, \mathbf{1}, \mathbf{1}, \mathbf{1}, \mathbf{1})$, $(0,0,1,1,0,0,0,0) \mapsto (L,Q)$
$(\overline{\mathbf{4}}, \mathbf{2}, \mathbf{1}, \mathbf{1}, \mathbf{1}, \mathbf{1})$, $(0,0,1,1,0,0,0,0) \mapsto (L,Q)$
$(\overline{\mathbf{4}}, \mathbf{1}, \mathbf{2}, \mathbf{1}, \mathbf{1}, \mathbf{1})$, $(0,0,1,0,1,0,0,0) \mapsto (L,Q)$
$(\mathbf{4}, \mathbf{1}, \mathbf{1}, \mathbf{2}, \mathbf{1}, \mathbf{1})$, $(1,0,0,0,0,1,0,0) \mapsto (D,E,N,U)$
$(\mathbf{4}, \mathbf{1}, \mathbf{1}, \mathbf{1}, \mathbf{2}, \mathbf{1})$, $(1,0,0,0,0,0,1,0) \mapsto (D,E,N,U)$
$(\mathbf{4}, \mathbf{1}, \mathbf{1}, \mathbf{1}, \mathbf{1}, \mathbf{2})$, $(1,0,0,0,0,0,0,1) \mapsto (D,E,N,U)$
Projection matrix for $\alpha$:

$$\begin{pmatrix} 0 & 1 & 0 & 0 & 0 & 0 & 0 & 0 \\ 1 & 0 & 0 & 0 & 0 & 0 & 0 & 0 \\ 0 & 0 & 0 & 1 & 1 & 0 & 0 & 0 \\ -1 & -2 & -3 & 0 & 0 & 3 & 3 & 3 \end{pmatrix}$$

**3 generation subalgebra** 278
Algebra: $\mathfrak{su}(4) \oplus \mathfrak{su}(2) \oplus \mathfrak{su}(2) \oplus \mathfrak{su}(2) \oplus \mathfrak{su}(2) \oplus \mathfrak{su}(2)$
$(\overline{\mathbf{4}}, \mathbf{2}, \mathbf{1}, \mathbf{1}, \mathbf{1}, \mathbf{1})$, $(0,0,1,1,0,0,0,0) \mapsto (D,E,N,U)$
$(\overline{\mathbf{4}}, \mathbf{2}, \mathbf{1}, \mathbf{1}, \mathbf{1}, \mathbf{1})$, $(0,0,1,1,0,0,0,0) \mapsto (D,E,N,U)$
$(\overline{\mathbf{4}}, \mathbf{1}, \mathbf{2}, \mathbf{1}, \mathbf{1}, \mathbf{1})$, $(0,0,1,0,1,0,0,0) \mapsto (D,E,N,U)$
$(\mathbf{4}, \mathbf{1}, \mathbf{1}, \mathbf{2}, \mathbf{1}, \mathbf{1})$, $(1,0,0,0,0,1,0,0) \mapsto (L,Q)$
$(\mathbf{4}, \mathbf{1}, \mathbf{1}, \mathbf{1}, \mathbf{2}, \mathbf{1})$, $(1,0,0,0,0,0,1,0) \mapsto (L,Q)$
$(\mathbf{4}, \mathbf{1}, \mathbf{1}, \mathbf{1}, \mathbf{1}, \mathbf{2})$, $(1,0,0,0,0,0,0,1) \mapsto (L,Q)$
Projection matrix for $\alpha$:

$$\begin{pmatrix} 1 & 0 & 0 & 0 & 0 & 0 & 0 & 0 \\ 0 & 1 & 0 & 0 & 0 & 0 & 0 & 0 \\ 0 & 0 & 0 & 0 & 0 & 1 & 1 & 1 \\ 1 & 2 & 3 & 3 & 3 & 0 & 0 & 0 \end{pmatrix}$$

**3 generation subalgebra** 279
Algebra: $\mathfrak{su}(4) \oplus \mathfrak{su}(4) \oplus \mathfrak{so}(10) \oplus \mathfrak{su}(2) \oplus \mathfrak{su}(2) \oplus \mathfrak{su}(2)$
$(\mathbf{1}, \mathbf{1}, \mathbf{16}, \mathbf{1}, \mathbf{1}, \mathbf{1})$, $(0,0,0,0,0,0,0,0,0,0,1,0,0,0) \mapsto (D,E,L,N,Q,U)$
$(\overline{\mathbf{4}}, \mathbf{1}, \mathbf{1}, \mathbf{2}, \mathbf{1}, \mathbf{1})$, $(0,0,1,0,0,0,0,0,0,0,0,1,0,0) \mapsto (L,Q)$
$(\mathbf{1}, \overline{\mathbf{4}}, \mathbf{1}, \mathbf{2}, \mathbf{1}, \mathbf{1})$, $(0,0,0,0,0,1,0,0,0,0,0,1,0,0) \mapsto (L,Q)$
$(\mathbf{4}, \mathbf{1}, \mathbf{1}, \mathbf{1}, \mathbf{2}, \mathbf{1})$, $(1,0,0,0,0,0,0,0,0,0,0,0,1,0) \mapsto (D,E,N,U)$
$(\mathbf{1}, \mathbf{4}, \mathbf{1}, \mathbf{1}, \mathbf{1}, \mathbf{2})$, $(0,0,0,1,0,0,0,0,0,0,0,0,0,1) \mapsto (D,E,N,U)$
Projection matrix for $\alpha$:

$$\begin{pmatrix} 0 & 1 & 0 & 0 & 1 & 0 & 0 & 0 & 1 & 0 & 0 & 0 & 0 & 0 \\ 1 & 0 & 0 & 1 & 0 & 0 & 0 & 0 & 0 & 0 & 1 & 0 & 0 & 0 \\ 0 & 0 & 0 & 0 & 0 & 0 & 1 & 0 & 0 & 0 & 0 & 1 & 0 & 0 \\ -1 & -2 & -3 & -1 & -2 & -3 & 3 & 6 & 4 & 0 & 2 & 0 & 3 & 3 \end{pmatrix}$$

**3 generation subalgebra** 280
Algebra: $\mathfrak{su}(4) \oplus \mathfrak{su}(4) \oplus \mathfrak{so}(10) \oplus \mathfrak{su}(2) \oplus \mathfrak{su}(2) \oplus \mathfrak{su}(2)$
$(\mathbf{1}, \mathbf{1}, \mathbf{16}, \mathbf{1}, \mathbf{1}, \mathbf{1})$, $(0,0,0,0,0,0,0,0,0,0,1,0,0,0) \mapsto (D,E,L,N,Q,U)$
$(\overline{\mathbf{4}}, \mathbf{1}, \mathbf{1}, \mathbf{2}, \mathbf{1}, \mathbf{1})$, $(0,0,1,0,0,0,0,0,0,0,0,1,0,0) \mapsto (D,E,N,U)$
$(\mathbf{1}, \overline{\mathbf{4}}, \mathbf{1}, \mathbf{2}, \mathbf{1}, \mathbf{1})$, $(0,0,0,0,0,1,0,0,0,0,0,1,0,0) \mapsto (D,E,N,U)$
$(\mathbf{4}, \mathbf{1}, \mathbf{1}, \mathbf{1}, \mathbf{2}, \mathbf{1})$, $(1,0,0,0,0,0,0,0,0,0,0,0,1,0) \mapsto (L,Q)$
$(\mathbf{1}, \mathbf{4}, \mathbf{1}, \mathbf{1}, \mathbf{1}, \mathbf{2})$, $(0,0,0,1,0,0,0,0,0,0,0,0,0,1) \mapsto (L,Q)$

Projection matrix for $\alpha$:

$$\begin{pmatrix} 1 & 0 & 0 & 1 & 0 & 0 & 0 & 0 & 1 & 0 & 0 & 0 & 0 & 0 \\ 0 & 1 & 0 & 0 & 1 & 0 & 0 & 0 & 0 & 0 & 1 & 0 & 0 & 0 \\ 0 & 0 & 0 & 0 & 0 & 0 & 1 & 0 & 0 & 0 & 0 & 0 & 1 & 1 \\ 1 & 2 & 3 & 1 & 2 & 3 & 3 & 6 & 4 & 0 & 2 & 3 & 0 & 0 \end{pmatrix}$$

**3 generation subalgebra** 281
Algebra: $\mathfrak{su}(4) \oplus \mathfrak{su}(4) \oplus \mathfrak{sp}(4) \oplus \mathfrak{su}(2) \oplus \mathfrak{su}(2) \oplus \mathfrak{su}(2)$
$(\bar{\mathbf{4}}, \mathbf{1}, \mathbf{4}, \mathbf{1}, \mathbf{1}, \mathbf{1})$, $(0, 0, 1, 0, 0, 0, 1, 0, 0, 0, 0) \mapsto (L, L, Q, Q)$
$(\mathbf{4}, \mathbf{1}, \mathbf{1}, \mathbf{2}, \mathbf{2}, \mathbf{1})$, $(1, 0, 0, 0, 0, 0, 0, 0, 1, 1, 0) \mapsto (D, D, E, E, N, N, U, U)$
$(\mathbf{1}, \bar{\mathbf{4}}, \mathbf{1}, \mathbf{2}, \mathbf{1}, \mathbf{1})$, $(0, 0, 0, 0, 0, 1, 0, 0, 1, 0, 0) \mapsto (D, E, N, U)$
$(\mathbf{1}, \mathbf{4}, \mathbf{1}, \mathbf{1}, \mathbf{1}, \mathbf{2})$, $(0, 0, 0, 1, 0, 0, 0, 0, 0, 0, 1) \mapsto (L, Q)$
Projection matrix for $\alpha$:

$$\begin{pmatrix} 0 & 1 & 0 & 1 & 0 & 0 & 0 & 0 & 0 & 0 & 0 \\ 1 & 0 & 0 & 0 & 1 & 0 & 0 & 0 & 0 & 0 & 0 \\ 0 & 0 & 0 & 0 & 0 & 0 & 1 & 2 & 0 & 0 & 1 \\ -1 & -2 & -3 & 1 & 2 & 3 & 0 & 0 & 3 & 0 & 0 \end{pmatrix}$$

**3 generation subalgebra** 282
Algebra: $\mathfrak{su}(4) \oplus \mathfrak{su}(4) \oplus \mathfrak{sp}(4) \oplus \mathfrak{su}(2) \oplus \mathfrak{su}(2) \oplus \mathfrak{su}(2)$
$(\bar{\mathbf{4}}, \mathbf{1}, \mathbf{4}, \mathbf{1}, \mathbf{1}, \mathbf{1})$, $(0, 0, 1, 0, 0, 0, 1, 0, 0, 0, 0) \mapsto (D, D, E, E, N, N, U, U)$
$(\mathbf{4}, \mathbf{1}, \mathbf{1}, \mathbf{2}, \mathbf{2}, \mathbf{1})$, $(1, 0, 0, 0, 0, 0, 0, 0, 1, 1, 0) \mapsto (L, L, Q, Q)$
$(\mathbf{1}, \bar{\mathbf{4}}, \mathbf{1}, \mathbf{2}, \mathbf{1}, \mathbf{1})$, $(0, 0, 0, 0, 0, 1, 0, 0, 1, 0, 0) \mapsto (L, Q)$
$(\mathbf{1}, \mathbf{4}, \mathbf{1}, \mathbf{1}, \mathbf{1}, \mathbf{2})$, $(0, 0, 0, 1, 0, 0, 0, 0, 0, 0, 1) \mapsto (D, E, N, U)$
Projection matrix for $\alpha$:

$$\begin{pmatrix} 1 & 0 & 0 & 0 & 1 & 0 & 0 & 0 & 0 & 0 & 0 \\ 0 & 1 & 0 & 1 & 0 & 0 & 0 & 0 & 0 & 0 & 0 \\ 0 & 0 & 0 & 0 & 0 & 0 & 0 & 0 & 1 & 0 & 0 \\ 1 & 2 & 3 & -1 & -2 & -3 & 3 & 0 & 0 & 0 & 3 \end{pmatrix}$$

**3 generation subalgebra** 283
Algebra: $\mathfrak{su}(4) \oplus \mathfrak{su}(4) \oplus \mathfrak{sp}(4) \oplus \mathfrak{su}(2) \oplus \mathfrak{su}(2) \oplus \mathfrak{su}(2)$
$(\bar{\mathbf{4}}, \mathbf{1}, \mathbf{4}, \mathbf{1}, \mathbf{1}, \mathbf{1})$, $(0, 0, 1, 0, 0, 0, 1, 0, 0, 0, 0) \mapsto (L, L, Q, Q)$
$(\mathbf{4}, \mathbf{1}, \mathbf{1}, \mathbf{2}, \mathbf{1}, \mathbf{1})$, $(1, 0, 0, 0, 0, 0, 0, 0, 1, 0, 0) \mapsto (D, E, N, U)$
$(\mathbf{1}, \bar{\mathbf{4}}, \mathbf{1}, \mathbf{2}, \mathbf{1}, \mathbf{1})$, $(0, 0, 0, 0, 0, 1, 0, 0, 1, 0, 0) \mapsto (D, E, N, U)$
$(\mathbf{4}, \mathbf{1}, \mathbf{1}, \mathbf{1}, \mathbf{2}, \mathbf{1})$, $(1, 0, 0, 0, 0, 0, 0, 0, 0, 1, 0) \mapsto (D, E, N, U)$
$(\mathbf{1}, \mathbf{4}, \mathbf{1}, \mathbf{1}, \mathbf{1}, \mathbf{2})$, $(0, 0, 0, 1, 0, 0, 0, 0, 0, 0, 1) \mapsto (L, Q)$
Projection matrix for $\alpha$:

$$\begin{pmatrix} 0 & 1 & 0 & 1 & 0 & 0 & 0 & 0 & 0 & 0 & 0 \\ 1 & 0 & 0 & 0 & 1 & 0 & 0 & 0 & 0 & 0 & 0 \\ 0 & 0 & 0 & 0 & 0 & 0 & 1 & 2 & 0 & 0 & 1 \\ -1 & -2 & -3 & 1 & 2 & 3 & 0 & 0 & 3 & 3 & 0 \end{pmatrix}$$

**3 generation subalgebra** 284
Algebra: $\mathfrak{su}(4) \oplus \mathfrak{su}(4) \oplus \mathfrak{sp}(4) \oplus \mathfrak{su}(2) \oplus \mathfrak{su}(2) \oplus \mathfrak{su}(2)$
$(\bar{\mathbf{4}}, \mathbf{1}, \mathbf{4}, \mathbf{1}, \mathbf{1}, \mathbf{1})$, $(0, 0, 1, 0, 0, 0, 1, 0, 0, 0, 0) \mapsto (D, D, E, E, N, N, U, U)$
$(\mathbf{4}, \mathbf{1}, \mathbf{1}, \mathbf{2}, \mathbf{1}, \mathbf{1})$, $(1, 0, 0, 0, 0, 0, 0, 0, 1, 0, 0) \mapsto (L, Q)$
$(\mathbf{1}, \bar{\mathbf{4}}, \mathbf{1}, \mathbf{2}, \mathbf{1}, \mathbf{1})$, $(0, 0, 0, 0, 0, 1, 0, 0, 1, 0, 0) \mapsto (L, Q)$
$(\mathbf{4}, \mathbf{1}, \mathbf{1}, \mathbf{1}, \mathbf{2}, \mathbf{1})$, $(1, 0, 0, 0, 0, 0, 0, 0, 0, 1, 0) \mapsto (L, Q)$
$(\mathbf{1}, \mathbf{4}, \mathbf{1}, \mathbf{1}, \mathbf{1}, \mathbf{2})$, $(0, 0, 0, 1, 0, 0, 0, 0, 0, 0, 1) \mapsto (D, E, N, U)$
Projection matrix for $\alpha$:

$$\begin{pmatrix} 1 & 0 & 0 & 0 & 1 & 0 & 0 & 0 & 0 & 0 & 0 \\ 0 & 1 & 0 & 1 & 0 & 0 & 0 & 0 & 0 & 0 & 0 \\ 0 & 0 & 0 & 0 & 0 & 0 & 0 & 0 & 1 & 1 & 0 \\ 1 & 2 & 3 & -1 & -2 & -3 & 3 & 0 & 0 & 0 & 3 \end{pmatrix}$$

**3 generation subalgebra** 285
Algebra: $\mathfrak{su}(4) \oplus \mathfrak{su}(4) \oplus \mathfrak{sp}(4) \oplus \mathfrak{su}(2) \oplus \mathfrak{su}(2) \oplus \mathfrak{su}(2)$
$(\overline{\mathbf{4}}, \mathbf{1}, \mathbf{4}, \mathbf{1}, \mathbf{1}, \mathbf{1})$, $(0,0,1,0,0,0,1,0,0,0,0) \mapsto (L, L, Q, Q)$
$(\mathbf{4}, \mathbf{1}, \mathbf{1}, \mathbf{2}, \mathbf{1}, \mathbf{1})$, $(1,0,0,0,0,0,0,0,1,0,0) \mapsto (D, E, N, U)$
$(\mathbf{4}, \underline{\mathbf{1}}, \mathbf{1}, \mathbf{2}, \mathbf{1}, \mathbf{1})$, $(1,0,0,0,0,0,0,0,1,0,0) \mapsto (D, E, N, U)$
$(\mathbf{1}, \overline{\mathbf{4}}, \mathbf{1}, \mathbf{1}, \mathbf{2}, \mathbf{1})$, $(0,0,0,0,0,1,0,0,0,1,0) \mapsto (L, Q)$
$(\mathbf{1}, \mathbf{4}, \mathbf{1}, \mathbf{1}, \mathbf{1}, \mathbf{2})$, $(0,0,0,1,0,0,0,0,0,0,1) \mapsto (D, E, N, U)$
Projection matrix for $\alpha$:

$$\begin{pmatrix} 0 & 1 & 0 & 0 & 1 & 0 & 0 & 0 & 0 & 0 & 0 \\ 1 & 0 & 0 & 1 & 0 & 0 & 0 & 0 & 0 & 0 & 0 \\ 0 & 0 & 0 & 0 & 0 & 0 & 1 & 2 & 0 & 1 & 0 \\ -1 & -2 & -3 & -1 & -2 & -3 & 0 & 0 & 3 & 0 & 3 \end{pmatrix}$$

**3 generation subalgebra** 286
Algebra: $\mathfrak{su}(4) \oplus \mathfrak{su}(4) \oplus \mathfrak{sp}(4) \oplus \mathfrak{su}(2) \oplus \mathfrak{su}(2) \oplus \mathfrak{su}(2)$
$(\overline{\mathbf{4}}, \mathbf{1}, \mathbf{4}, \mathbf{1}, \mathbf{1}, \mathbf{1})$, $(0,0,1,0,0,0,1,0,0,0,0) \mapsto (D, D, E, E, N, N, U, U)$
$(\mathbf{4}, \mathbf{1}, \mathbf{1}, \mathbf{2}, \mathbf{1}, \mathbf{1})$, $(1,0,0,0,0,0,0,0,1,0,0) \mapsto (L, Q)$
$(\mathbf{4}, \underline{\mathbf{1}}, \mathbf{1}, \mathbf{2}, \mathbf{1}, \mathbf{1})$, $(1,0,0,0,0,0,0,0,1,0,0) \mapsto (L, Q)$
$(\mathbf{1}, \overline{\mathbf{4}}, \mathbf{1}, \mathbf{1}, \mathbf{2}, \mathbf{1})$, $(0,0,0,0,0,1,0,0,0,1,0) \mapsto (L, Q)$
$(\mathbf{1}, \mathbf{4}, \mathbf{1}, \mathbf{1}, \mathbf{1}, \mathbf{2})$, $(0,0,0,1,0,0,0,0,0,0,1) \mapsto (D, E, N, U)$
Projection matrix for $\alpha$:

$$\begin{pmatrix} 1 & 0 & 0 & 0 & 1 & 0 & 0 & 0 & 0 & 0 & 0 \\ 0 & 1 & 0 & 1 & 0 & 0 & 0 & 0 & 0 & 0 & 0 \\ 0 & 0 & 0 & 0 & 0 & 0 & 0 & 0 & 1 & 1 & 0 \\ 1 & 2 & 3 & -1 & -2 & -3 & 3 & 0 & 0 & 0 & 3 \end{pmatrix}$$

**3 generation subalgebra** 287
Algebra: $\mathfrak{su}(4) \oplus \mathfrak{su}(4) \oplus \mathfrak{su}(2) \oplus \mathfrak{su}(2) \oplus \mathfrak{su}(2) \oplus \mathfrak{su}(2)$
$(\mathbf{4}, \underline{\mathbf{1}}, \mathbf{2}, \mathbf{2}, \mathbf{1}, \mathbf{1})$, $(1,0,0,0,0,0,1,1,0,0) \mapsto (L, L, Q, Q)$
$(\underline{\mathbf{1}}, \overline{\mathbf{4}}, \mathbf{2}, \mathbf{1}, \mathbf{1}, \mathbf{1})$, $(0,0,0,0,0,1,1,0,0,0) \mapsto (L, Q)$
$(\overline{\mathbf{4}}, \mathbf{1}, \mathbf{1}, \mathbf{1}, \mathbf{2}, \mathbf{2})$, $(0,0,1,0,0,0,0,0,1,1) \mapsto (D, D, E, E, N, N, U, U)$
$(\mathbf{1}, \mathbf{4}, \mathbf{1}, \mathbf{1}, \mathbf{2}, \mathbf{1})$, $(0,0,0,1,0,0,0,0,1,0) \mapsto (D, E, N, U)$
Projection matrix for $\alpha$:

$$\begin{pmatrix} 1 & 0 & 0 & 0 & 1 & 0 & 0 & 0 & 0 & 0 \\ 0 & 1 & 0 & 1 & 0 & 0 & 0 & 0 & 0 & 0 \\ 0 & 0 & 0 & 0 & 0 & 0 & 1 & 0 & 0 & 0 \\ 1 & 2 & 3 & -1 & -2 & -3 & 0 & 0 & 3 & 0 \end{pmatrix}$$

**3 generation subalgebra** 288
Algebra: $\mathfrak{su}(4) \oplus \mathfrak{su}(4) \oplus \mathfrak{su}(2) \oplus \mathfrak{su}(2) \oplus \mathfrak{su}(2) \oplus \mathfrak{su}(2)$
$(\underline{\mathbf{4}}, \mathbf{1}, \mathbf{2}, \mathbf{2}, \mathbf{1}, \mathbf{1})$, $(1,0,0,0,0,0,1,1,0,0) \mapsto (D, D, E, E, N, N, U, U)$
$(\overline{\mathbf{4}}, \underline{\mathbf{1}}, \mathbf{2}, \mathbf{1}, \mathbf{2}, \mathbf{1})$, $(0,0,1,0,0,0,1,0,1,0) \mapsto (L, L, Q, Q)$
$(\mathbf{1}, \overline{\mathbf{4}}, \mathbf{1}, \mathbf{2}, \mathbf{1}, \mathbf{1})$, $(0,0,0,0,0,1,0,1,0,0) \mapsto (D, E, N, U)$
$(\mathbf{1}, \mathbf{4}, \mathbf{1}, \mathbf{1}, \mathbf{1}, \mathbf{2})$, $(0,0,0,1,0,0,0,0,0,1) \mapsto (L, Q)$
Projection matrix for $\alpha$:

$$\begin{pmatrix} 0 & 1 & 0 & 1 & 0 & 0 & 0 & 0 & 0 & 0 \\ 1 & 0 & 0 & 0 & 1 & 0 & 0 & 0 & 0 & 0 \\ 0 & 0 & 0 & 0 & 0 & 0 & 0 & 0 & 1 & 1 \\ -1 & -2 & -3 & 1 & 2 & 3 & 0 & 3 & 0 & 0 \end{pmatrix}$$

**3 generation subalgebra** 289
Algebra: $\mathfrak{su}(4) \oplus \mathfrak{su}(4) \oplus \mathfrak{su}(2) \oplus \mathfrak{su}(2) \oplus \mathfrak{su}(2) \oplus \mathfrak{su}(2)$
$(\underline{\mathbf{4}}, \mathbf{1}, \mathbf{2}, \mathbf{2}, \mathbf{1}, \mathbf{1})$, $(1,0,0,0,0,0,1,1,0,0) \mapsto (L, L, Q, Q)$
$(\overline{\mathbf{4}}, \underline{\mathbf{1}}, \mathbf{2}, \mathbf{1}, \mathbf{2}, \mathbf{1})$, $(0,0,1,0,0,0,1,0,1,0) \mapsto (D, D, E, E, N, N, U, U)$
$(\mathbf{1}, \overline{\mathbf{4}}, \mathbf{1}, \mathbf{2}, \mathbf{1}, \mathbf{1})$, $(0,0,0,0,0,1,0,1,0,0) \mapsto (L, Q)$

$(\mathbf{1},\mathbf{4},\mathbf{1},\mathbf{1},\mathbf{1},\mathbf{2})$, $(0,0,0,1,0,0,0,0,0,1) \mapsto (D,E,N,U)$
Projection matrix for $\alpha$:

$$\begin{pmatrix} 1 & 0 & 0 & 0 & 1 & 0 & 0 & 0 & 0 & 0 \\ 0 & 1 & 0 & 1 & 0 & 0 & 0 & 0 & 0 & 0 \\ 0 & 0 & 0 & 0 & 0 & 0 & 0 & 1 & 0 & 0 \\ 1 & 2 & 3 & -1 & -2 & -3 & 0 & 0 & 3 & 3 \end{pmatrix}$$

**3 generation subalgebra** 290
Algebra: $\mathfrak{su}(4) \oplus \mathfrak{su}(4) \oplus \mathfrak{su}(2) \oplus \mathfrak{su}(2) \oplus \mathfrak{su}(2) \oplus \mathfrak{su}(2)$
$(\mathbf{4},\mathbf{1},\mathbf{2},\mathbf{2},\mathbf{1},\mathbf{1})$, $(1,0,0,0,0,0,1,1,0,0) \mapsto (D,D,E,E,N,N,U,U)$
$(\mathbf{1},\bar{\mathbf{4}},\mathbf{2},\mathbf{1},\mathbf{1},\mathbf{1})$, $(0,0,0,0,0,1,1,0,0,0) \mapsto (D,E,N,U)$
$(\bar{\mathbf{4}},\mathbf{1},\mathbf{1},\mathbf{1},\mathbf{2},\mathbf{1})$, $(0,0,1,0,0,0,0,0,1,0) \mapsto (L,Q)$
$(\mathbf{1},\mathbf{4},\mathbf{1},\mathbf{1},\mathbf{2},\mathbf{1})$, $(0,0,0,1,0,0,0,0,1,0) \mapsto (L,Q)$
$(\bar{\mathbf{4}},\mathbf{1},\mathbf{1},\mathbf{1},\mathbf{1},\mathbf{2})$, $(0,0,1,0,0,0,0,0,0,1) \mapsto (L,Q)$
Projection matrix for $\alpha$:

$$\begin{pmatrix} 0 & 1 & 0 & 1 & 0 & 0 & 0 & 0 & 0 & 0 \\ 1 & 0 & 0 & 0 & 1 & 0 & 0 & 0 & 0 & 0 \\ 0 & 0 & 0 & 0 & 0 & 0 & 0 & 0 & 1 & 1 \\ -1 & -2 & -3 & 1 & 2 & 3 & 3 & 0 & 0 & 0 \end{pmatrix}$$

**3 generation subalgebra** 291
Algebra: $\mathfrak{su}(4) \oplus \mathfrak{su}(4) \oplus \mathfrak{su}(2) \oplus \mathfrak{su}(2) \oplus \mathfrak{su}(2) \oplus \mathfrak{su}(2)$
$(\mathbf{4},\mathbf{1},\mathbf{2},\mathbf{2},\mathbf{1},\mathbf{1})$, $(1,0,0,0,0,0,1,1,0,0) \mapsto (L,L,Q,Q)$
$(\mathbf{1},\bar{\mathbf{4}},\mathbf{2},\mathbf{1},\mathbf{1},\mathbf{1})$, $(0,0,0,0,0,1,1,0,0,0) \mapsto (L,Q)$
$(\bar{\mathbf{4}},\mathbf{1},\mathbf{1},\mathbf{1},\mathbf{2},\mathbf{1})$, $(0,0,1,0,0,0,0,0,1,0) \mapsto (D,E,N,U)$
$(\mathbf{1},\mathbf{4},\mathbf{1},\mathbf{1},\mathbf{2},\mathbf{1})$, $(0,0,0,1,0,0,0,0,1,0) \mapsto (D,E,N,U)$
$(\bar{\mathbf{4}},\mathbf{1},\mathbf{1},\mathbf{1},\mathbf{1},\mathbf{2})$, $(0,0,1,0,0,0,0,0,0,1) \mapsto (D,E,N,U)$
Projection matrix for $\alpha$:

$$\begin{pmatrix} 1 & 0 & 0 & 0 & 1 & 0 & 0 & 0 & 0 & 0 \\ 0 & 1 & 0 & 1 & 0 & 0 & 0 & 0 & 0 & 0 \\ 0 & 0 & 0 & 0 & 0 & 0 & 1 & 0 & 0 & 0 \\ 1 & 2 & 3 & -1 & -2 & -3 & 0 & 0 & 3 & 3 \end{pmatrix}$$

**3 generation subalgebra** 292
Algebra: $\mathfrak{su}(4) \oplus \mathfrak{su}(4) \oplus \mathfrak{su}(2) \oplus \mathfrak{su}(2) \oplus \mathfrak{su}(2) \oplus \mathfrak{su}(2)$
$(\mathbf{4},\mathbf{1},\mathbf{2},\mathbf{2},\mathbf{1},\mathbf{1})$, $(1,0,0,0,0,0,1,1,0,0) \mapsto (D,D,E,E,N,N,U,U)$
$(\mathbf{1},\bar{\mathbf{4}},\mathbf{2},\mathbf{1},\mathbf{1},\mathbf{1})$, $(0,0,0,0,0,1,1,0,0,0) \mapsto (D,E,N,U)$
$(\bar{\mathbf{4}},\mathbf{1},\mathbf{1},\mathbf{1},\mathbf{2},\mathbf{1})$, $(0,0,1,0,0,0,0,0,1,0) \mapsto (L,Q)$
$(\bar{\mathbf{4}},\mathbf{1},\mathbf{1},\mathbf{1},\mathbf{2},\mathbf{1})$, $(0,0,1,0,0,0,0,0,1,0) \mapsto (L,Q)$
$(\mathbf{1},\mathbf{4},\mathbf{1},\mathbf{1},\mathbf{1},\mathbf{2})$, $(0,0,0,1,0,0,0,0,0,1) \mapsto (L,Q)$
Projection matrix for $\alpha$:

$$\begin{pmatrix} 0 & 1 & 0 & 1 & 0 & 0 & 0 & 0 & 0 & 0 \\ 1 & 0 & 0 & 0 & 1 & 0 & 0 & 0 & 0 & 0 \\ 0 & 0 & 0 & 0 & 0 & 0 & 0 & 0 & 1 & 1 \\ -1 & -2 & -3 & 1 & 2 & 3 & 3 & 0 & 0 & 0 \end{pmatrix}$$

**3 generation subalgebra** 293
Algebra: $\mathfrak{su}(4) \oplus \mathfrak{su}(4) \oplus \mathfrak{su}(2) \oplus \mathfrak{su}(2) \oplus \mathfrak{su}(2) \oplus \mathfrak{su}(2)$
$(\mathbf{4},\mathbf{1},\mathbf{2},\mathbf{2},\mathbf{1},\mathbf{1})$, $(1,0,0,0,0,0,1,1,0,0) \mapsto (L,L,Q,Q)$
$(\mathbf{1},\bar{\mathbf{4}},\mathbf{2},\mathbf{1},\mathbf{1},\mathbf{1})$, $(0,0,0,0,0,1,1,0,0,0) \mapsto (L,Q)$
$(\bar{\mathbf{4}},\mathbf{1},\mathbf{1},\mathbf{1},\mathbf{2},\mathbf{1})$, $(0,0,1,0,0,0,0,0,1,0) \mapsto (D,E,N,U)$
$(\bar{\mathbf{4}},\mathbf{1},\mathbf{1},\mathbf{1},\mathbf{2},\mathbf{1})$, $(0,0,1,0,0,0,0,0,1,0) \mapsto (D,E,N,U)$
$(\mathbf{1},\mathbf{4},\mathbf{1},\mathbf{1},\mathbf{1},\mathbf{2})$, $(0,0,0,1,0,0,0,0,0,1) \mapsto (D,E,N,U)$
Projection matrix for $\alpha$:

$$\begin{pmatrix} 1 & 0 & 0 & 0 & 1 & 0 & 0 & 0 & 0 & 0 \\ 0 & 1 & 0 & 1 & 0 & 0 & 0 & 0 & 0 & 0 \\ 0 & 0 & 0 & 0 & 0 & 0 & 1 & 0 & 0 & 0 \\ 1 & 2 & 3 & -1 & -2 & -3 & 0 & 0 & 3 & 3 \end{pmatrix}$$

**3 generation subalgebra** 294
Algebra: $\mathfrak{su}(4) \oplus \mathfrak{su}(4) \oplus \mathfrak{su}(2) \oplus \mathfrak{su}(2) \oplus \mathfrak{su}(2) \oplus \mathfrak{su}(2)$
$(\mathbf{4}, \mathbf{1}, \mathbf{2}, \mathbf{2}, \mathbf{1}, \mathbf{1})$, $(1, 0, 0, 0, 0, 0, 1, 1, 0, 0) \mapsto (D, D, E, E, N, N, U, U)$
$(\overline{\mathbf{4}}, \mathbf{1}, \mathbf{1}, \mathbf{1}, \mathbf{2}, \mathbf{1})$, $(0, 0, 1, 0, 0, 0, 0, 0, 1, 0) \mapsto (L, Q)$
$(\overline{\mathbf{4}}, \mathbf{1}, \mathbf{1}, \mathbf{1}, \mathbf{2}, \mathbf{1})$, $(0, 0, 1, 0, 0, 0, 0, 0, 1, 0) \mapsto (L, Q)$
$(\mathbf{1}, \overline{\mathbf{4}}, \mathbf{1}, \mathbf{1}, \mathbf{2}, \mathbf{1})$, $(0, 0, 0, 0, 0, 1, 0, 0, 1, 0) \mapsto (L, Q)$
$(\mathbf{1}, \mathbf{4}, \mathbf{1}, \mathbf{1}, \mathbf{1}, \mathbf{2})$, $(0, 0, 0, 1, 0, 0, 0, 0, 0, 1) \mapsto (D, E, N, U)$
Projection matrix for $\alpha$:

$$\begin{pmatrix} 0 & 1 & 0 & 0 & 1 & 0 & 0 & 0 & 0 & 0 \\ 1 & 0 & 0 & 1 & 0 & 0 & 0 & 0 & 0 & 0 \\ 0 & 0 & 0 & 0 & 0 & 0 & 0 & 0 & 1 & 0 \\ -1 & -2 & -3 & -1 & -2 & -3 & 3 & 0 & 0 & 3 \end{pmatrix}$$

**3 generation subalgebra** 295
Algebra: $\mathfrak{su}(4) \oplus \mathfrak{su}(4) \oplus \mathfrak{su}(2) \oplus \mathfrak{su}(2) \oplus \mathfrak{su}(2) \oplus \mathfrak{su}(2)$
$(\mathbf{4}, \mathbf{1}, \mathbf{2}, \mathbf{2}, \mathbf{1}, \mathbf{1})$, $(1, 0, 0, 0, 0, 0, 1, 1, 0, 0) \mapsto (L, L, Q, Q)$
$(\overline{\mathbf{4}}, \mathbf{1}, \mathbf{1}, \mathbf{1}, \mathbf{2}, \mathbf{1})$, $(0, 0, 1, 0, 0, 0, 0, 0, 1, 0) \mapsto (D, E, N, U)$
$(\overline{\mathbf{4}}, \mathbf{1}, \mathbf{1}, \mathbf{1}, \mathbf{2}, \mathbf{1})$, $(0, 0, 1, 0, 0, 0, 0, 0, 1, 0) \mapsto (D, E, N, U)$
$(\mathbf{1}, \overline{\mathbf{4}}, \mathbf{1}, \mathbf{1}, \mathbf{2}, \mathbf{1})$, $(0, 0, 0, 0, 0, 1, 0, 0, 1, 0) \mapsto (D, E, N, U)$
$(\mathbf{1}, \mathbf{4}, \mathbf{1}, \mathbf{1}, \mathbf{1}, \mathbf{2})$, $(0, 0, 0, 1, 0, 0, 0, 0, 0, 1) \mapsto (L, Q)$
Projection matrix for $\alpha$:

$$\begin{pmatrix} 1 & 0 & 0 & 1 & 0 & 0 & 0 & 0 & 0 & 0 \\ 0 & 1 & 0 & 0 & 1 & 0 & 0 & 0 & 0 & 0 \\ 0 & 0 & 0 & 0 & 0 & 0 & 1 & 0 & 0 & 1 \\ 1 & 2 & 3 & 1 & 2 & 3 & 0 & 0 & 3 & 0 \end{pmatrix}$$

**3 generation subalgebra** 296
Algebra: $\mathfrak{su}(4) \oplus \mathfrak{su}(4) \oplus \mathfrak{su}(2) \oplus \mathfrak{su}(2) \oplus \mathfrak{su}(2) \oplus \mathfrak{su}(2)$
$(\overline{\mathbf{4}}, \mathbf{1}, \mathbf{2}, \mathbf{1}, \mathbf{1}, \mathbf{1})$, $(0, 0, 1, 0, 0, 0, 1, 0, 0, 0) \mapsto (L, Q)$
$(\mathbf{1}, \overline{\mathbf{4}}, \mathbf{2}, \mathbf{1}, \mathbf{1}, \mathbf{1})$, $(0, 0, 0, 0, 0, 1, 1, 0, 0, 0) \mapsto (L, Q)$
$(\overline{\mathbf{4}}, \mathbf{1}, \mathbf{1}, \mathbf{2}, \mathbf{1}, \mathbf{1})$, $(0, 0, 1, 0, 0, 0, 0, 1, 0, 0) \mapsto (L, Q)$
$(\mathbf{4}, \mathbf{1}, \mathbf{1}, \mathbf{1}, \mathbf{2}, \mathbf{1})$, $(1, 0, 0, 0, 0, 0, 0, 0, 1, 0) \mapsto (D, E, N, U)$
$(\mathbf{1}, \mathbf{4}, \mathbf{1}, \mathbf{1}, \mathbf{2}, \mathbf{1})$, $(0, 0, 0, 1, 0, 0, 0, 0, 1, 0) \mapsto (D, E, N, U)$
$(\mathbf{4}, \mathbf{1}, \mathbf{1}, \mathbf{1}, \mathbf{1}, \mathbf{2})$, $(1, 0, 0, 0, 0, 0, 0, 0, 0, 1) \mapsto (D, E, N, U)$
Projection matrix for $\alpha$:

$$\begin{pmatrix} 0 & 1 & 0 & 0 & 1 & 0 & 0 & 0 & 0 & 0 \\ 1 & 0 & 0 & 1 & 0 & 0 & 0 & 0 & 0 & 0 \\ 0 & 0 & 0 & 0 & 0 & 0 & 1 & 1 & 0 & 0 \\ -1 & -2 & -3 & -1 & -2 & -3 & 0 & 0 & 3 & 3 \end{pmatrix}$$

**3 generation subalgebra** 297
Algebra: $\mathfrak{su}(4) \oplus \mathfrak{su}(4) \oplus \mathfrak{su}(2) \oplus \mathfrak{su}(2) \oplus \mathfrak{su}(2) \oplus \mathfrak{su}(2)$
$(\overline{\mathbf{4}}, \mathbf{1}, \mathbf{2}, \mathbf{1}, \mathbf{1}, \mathbf{1})$, $(0, 0, 1, 0, 0, 0, 1, 0, 0, 0) \mapsto (L, Q)$
$(\overline{\mathbf{4}}, \mathbf{1}, \mathbf{2}, \mathbf{1}, \mathbf{1}, \mathbf{1})$, $(0, 0, 1, 0, 0, 0, 1, 0, 0, 0) \mapsto (L, Q)$
$(\mathbf{1}, \overline{\mathbf{4}}, \mathbf{2}, \mathbf{1}, \mathbf{1}, \mathbf{1})$, $(0, 0, 0, 0, 0, 1, 1, 0, 0, 0) \mapsto (L, Q)$
$(\mathbf{4}, \mathbf{1}, \mathbf{1}, \mathbf{2}, \mathbf{1}, \mathbf{1})$, $(1, 0, 0, 0, 0, 0, 0, 1, 0, 0) \mapsto (D, E, N, U)$
$(\mathbf{4}, \mathbf{1}, \mathbf{1}, \mathbf{1}, \mathbf{2}, \mathbf{1})$, $(1, 0, 0, 0, 0, 0, 0, 0, 1, 0) \mapsto (D, E, N, U)$
$(\mathbf{1}, \mathbf{4}, \mathbf{1}, \mathbf{1}, \mathbf{1}, \mathbf{2})$, $(0, 0, 0, 1, 0, 0, 0, 0, 0, 1) \mapsto (D, E, N, U)$
Projection matrix for $\alpha$:

$$\begin{pmatrix} 0 & 1 & 0 & 0 & 1 & 0 & 0 & 0 & 0 & 0 \\ 1 & 0 & 0 & 1 & 0 & 0 & 0 & 0 & 0 & 0 \\ 0 & 0 & 0 & 0 & 0 & 0 & 1 & 0 & 0 & 0 \\ -1 & -2 & -3 & -1 & -2 & -3 & 0 & 3 & 3 & 3 \end{pmatrix}$$

**3 generation subalgebra** 298
Algebra: $\mathfrak{su}(4) \oplus \mathfrak{su}(4) \oplus \mathfrak{su}(2) \oplus \mathfrak{su}(2) \oplus \mathfrak{su}(2) \oplus \mathfrak{su}(2)$

$(\overline{\mathbf{4}}, \mathbf{1}, \mathbf{2}, \mathbf{1}, \mathbf{1}, \mathbf{1})$, $(0,0,1,0,0,0,1,0,0,0) \mapsto (D, E, N, U)$
$(\overline{\mathbf{4}}, \mathbf{1}, \mathbf{2}, \mathbf{1}, \mathbf{1}, \mathbf{1})$, $(0,0,1,0,0,0,1,0,0,0) \mapsto (D, E, N, U)$
$(\mathbf{1}, \overline{\mathbf{4}}, \mathbf{2}, \mathbf{1}, \mathbf{1}, \mathbf{1})$, $(0,0,0,0,0,1,1,0,0,0) \mapsto (D, E, N, U)$
$(\mathbf{4}, \mathbf{1}, \mathbf{1}, \mathbf{2}, \mathbf{1}, \mathbf{1})$, $(1,0,0,0,0,0,0,1,0,0) \mapsto (L, Q)$
$(\mathbf{4}, \mathbf{1}, \mathbf{1}, \mathbf{1}, \mathbf{2}, \mathbf{1})$, $(1,0,0,0,0,0,0,0,1,0) \mapsto (L, Q)$
$(\mathbf{1}, \mathbf{4}, \mathbf{1}, \mathbf{1}, \mathbf{1}, \mathbf{2})$, $(0,0,0,1,0,0,0,0,0,1) \mapsto (L, Q)$
Projection matrix for $\alpha$:

$$\begin{pmatrix} 1 & 0 & 0 & 1 & 0 & 0 & 0 & 0 & 0 & 0 \\ 0 & 1 & 0 & 0 & 1 & 0 & 0 & 0 & 0 & 0 \\ 0 & 0 & 0 & 0 & 0 & 0 & 0 & 1 & 1 & 1 \\ 1 & 2 & 3 & 1 & 2 & 3 & 3 & 0 & 0 & 0 \end{pmatrix}$$

**3 generation subalgebra** 299
Algebra: $\mathfrak{su}(4) \oplus \mathfrak{su}(4) \oplus \mathfrak{su}(2) \oplus \mathfrak{su}(2) \oplus \mathfrak{su}(2) \oplus \mathfrak{su}(2)$
$(\overline{\mathbf{4}}, \mathbf{1}, \mathbf{2}, \mathbf{1}, \mathbf{1}, \mathbf{1})$, $(0,0,1,0,0,0,1,0,0,0) \mapsto (L, Q)$
$(\overline{\mathbf{4}}, \mathbf{1}, \mathbf{2}, \mathbf{1}, \mathbf{1}, \mathbf{1})$, $(0,0,1,0,0,0,1,0,0,0) \mapsto (L, Q)$
$(\mathbf{4}, \mathbf{1}, \mathbf{1}, \mathbf{2}, \mathbf{1}, \mathbf{1})$, $(1,0,0,0,0,0,0,1,0,0) \mapsto (D, E, N, U)$
$(\mathbf{1}, \overline{\mathbf{4}}, \mathbf{1}, \mathbf{2}, \mathbf{1}, \mathbf{1})$, $(0,0,0,0,0,1,0,1,0,0) \mapsto (D, E, N, U)$
$(\mathbf{4}, \mathbf{1}, \mathbf{1}, \mathbf{1}, \mathbf{2}, \mathbf{1})$, $(1,0,0,0,0,0,0,0,1,0) \mapsto (D, E, N, U)$
$(\mathbf{1}, \mathbf{4}, \mathbf{1}, \mathbf{1}, \mathbf{1}, \mathbf{2})$, $(0,0,0,1,0,0,0,0,0,1) \mapsto (L, Q)$
Projection matrix for $\alpha$:

$$\begin{pmatrix} 0 & 1 & 0 & 1 & 0 & 0 & 0 & 0 & 0 & 0 \\ 1 & 0 & 0 & 0 & 1 & 0 & 0 & 0 & 0 & 0 \\ 0 & 0 & 0 & 0 & 0 & 1 & 0 & 0 & 1 \\ -1 & -2 & -3 & 1 & 2 & 3 & 0 & 3 & 3 & 0 \end{pmatrix}$$

**3 generation subalgebra** 300
Algebra: $\mathfrak{su}(4) \oplus \mathfrak{su}(4) \oplus \mathfrak{su}(2) \oplus \mathfrak{su}(2) \oplus \mathfrak{su}(2) \oplus \mathfrak{su}(2)$
$(\overline{\mathbf{4}}, \mathbf{1}, \mathbf{2}, \mathbf{1}, \mathbf{1}, \mathbf{1})$, $(0,0,1,0,0,0,1,0,0,0) \mapsto (D, E, N, U)$
$(\overline{\mathbf{4}}, \mathbf{1}, \mathbf{2}, \mathbf{1}, \mathbf{1}, \mathbf{1})$, $(0,0,1,0,0,0,1,0,0,0) \mapsto (D, E, N, U)$
$(\mathbf{4}, \mathbf{1}, \mathbf{1}, \mathbf{2}, \mathbf{1}, \mathbf{1})$, $(1,0,0,0,0,0,0,1,0,0) \mapsto (L, Q)$
$(\mathbf{1}, \overline{\mathbf{4}}, \mathbf{1}, \mathbf{2}, \mathbf{1}, \mathbf{1})$, $(0,0,0,0,0,1,0,1,0,0) \mapsto (L, Q)$
$(\mathbf{4}, \mathbf{1}, \mathbf{1}, \mathbf{1}, \mathbf{2}, \mathbf{1})$, $(1,0,0,0,0,0,0,0,1,0) \mapsto (L, Q)$
$(\mathbf{1}, \mathbf{4}, \mathbf{1}, \mathbf{1}, \mathbf{1}, \mathbf{2})$, $(0,0,0,1,0,0,0,0,0,1) \mapsto (D, E, N, U)$
Projection matrix for $\alpha$:

$$\begin{pmatrix} 1 & 0 & 0 & 0 & 1 & 0 & 0 & 0 & 0 & 0 \\ 0 & 1 & 0 & 1 & 0 & 0 & 0 & 0 & 0 & 0 \\ 0 & 0 & 0 & 0 & 0 & 0 & 0 & 1 & 1 & 0 \\ 1 & 2 & 3 & -1 & -2 & -3 & 3 & 0 & 0 & 3 \end{pmatrix}$$

**3 generation subalgebra** 301
Algebra: $\mathfrak{su}(4) \oplus \mathfrak{su}(4) \oplus \mathfrak{su}(2) \oplus \mathfrak{su}(2) \oplus \mathfrak{su}(2) \oplus \mathfrak{su}(2)$
$(\overline{\mathbf{4}}, \mathbf{1}, \mathbf{2}, \mathbf{1}, \mathbf{1}, \mathbf{1})$, $(0,0,1,0,0,0,1,0,0,0) \mapsto (L, Q)$
$(\overline{\mathbf{4}}, \mathbf{1}, \mathbf{2}, \mathbf{1}, \mathbf{1}, \mathbf{1})$, $(0,0,1,0,0,0,1,0,0,0) \mapsto (L, Q)$
$(\mathbf{4}, \mathbf{1}, \mathbf{1}, \mathbf{2}, \mathbf{1}, \mathbf{1})$, $(1,0,0,0,0,0,0,1,0,0) \mapsto (D, E, N, U)$
$(\mathbf{4}, \mathbf{1}, \mathbf{1}, \mathbf{2}, \mathbf{1}, \mathbf{1})$, $(1,0,0,0,0,0,0,1,0,0) \mapsto (D, E, N, U)$
$(\mathbf{1}, \overline{\mathbf{4}}, \mathbf{1}, \mathbf{1}, \mathbf{2}, \mathbf{1})$, $(0,0,0,0,0,1,0,0,1,0) \mapsto (L, Q)$
$(\mathbf{1}, \mathbf{4}, \mathbf{1}, \mathbf{1}, \mathbf{1}, \mathbf{2})$, $(0,0,0,1,0,0,0,0,0,1) \mapsto (D, E, N, U)$
Projection matrix for $\alpha$:

$$\begin{pmatrix} 0 & 1 & 0 & 0 & 1 & 0 & 0 & 0 & 0 & 0 \\ 1 & 0 & 0 & 1 & 0 & 0 & 0 & 0 & 0 & 0 \\ 0 & 0 & 0 & 0 & 0 & 0 & 1 & 0 & 1 & 0 \\ -1 & -2 & -3 & -1 & -2 & -3 & 0 & 3 & 0 & 3 \end{pmatrix}$$

**3 generation subalgebra** 302
Algebra: $\mathfrak{su}(4) \oplus \mathfrak{su}(4) \oplus \mathfrak{su}(4) \oplus \mathfrak{su}(2) \oplus \mathfrak{su}(2) \oplus \mathfrak{su}(2)$

$(\bar{\mathbf{4}}, \mathbf{1}, \mathbf{1}, \mathbf{2}, \mathbf{1}, \mathbf{1})$, $(0, 0, 1, 0, 0, 0, 0, 0, 0, 1, 0, 0) \mapsto (L, Q)$
$(\mathbf{1}, \bar{\mathbf{4}}, \mathbf{1}, \mathbf{2}, \mathbf{1}, \mathbf{1})$, $(0, 0, 0, 0, 0, 1, 0, 0, 0, 1, 0, 0) \mapsto (L, Q)$
$(\mathbf{1}, \mathbf{1}, \bar{\mathbf{4}}, \mathbf{2}, \mathbf{1}, \mathbf{1})$, $(0, 0, 0, 0, 0, 0, 0, 0, 1, 1, 0, 0) \mapsto (L, Q)$
$(\mathbf{4}, \mathbf{1}, \mathbf{1}, \mathbf{1}, \mathbf{2}, \mathbf{1})$, $(1, 0, 0, 0, 0, 0, 0, 0, 0, 0, 1, 0) \mapsto (D, E, N, U)$
$(\mathbf{1}, \mathbf{4}, \mathbf{1}, \mathbf{1}, \mathbf{2}, \mathbf{1})$, $(0, 0, 0, 1, 0, 0, 0, 0, 0, 0, 1, 0) \mapsto (D, E, N, U)$
$(\mathbf{1}, \mathbf{1}, \mathbf{4}, \mathbf{1}, \mathbf{1}, \mathbf{2})$, $(0, 0, 0, 0, 0, 0, 1, 0, 0, 0, 0, 1) \mapsto (D, E, N, U)$
Projection matrix for $\alpha$:

$$\begin{pmatrix} 0 & 1 & 0 & 0 & 1 & 0 & 0 & 1 & 0 & 0 & 0 & 0 \\ 1 & 0 & 0 & 1 & 0 & 0 & 1 & 0 & 0 & 0 & 0 & 0 \\ 0 & 0 & 0 & 0 & 0 & 0 & 0 & 0 & 0 & 1 & 0 & 0 \\ -1 & -2 & -3 & -1 & -2 & -3 & -1 & -2 & -3 & 0 & 3 & 3 \end{pmatrix}$$

**3 generation subalgebra** 303
Algebra: $\mathfrak{su}(4) \oplus \mathfrak{su}(4) \oplus \mathfrak{su}(4) \oplus \mathfrak{su}(2) \oplus \mathfrak{su}(2) \oplus \mathfrak{su}(2)$
$(\bar{\mathbf{4}}, \mathbf{1}, \mathbf{1}, \mathbf{2}, \mathbf{1}, \mathbf{1})$, $(0, 0, 1, 0, 0, 0, 0, 0, 0, 1, 0, 0) \mapsto (D, E, N, U)$
$(\mathbf{1}, \bar{\mathbf{4}}, \mathbf{1}, \mathbf{2}, \mathbf{1}, \mathbf{1})$, $(0, 0, 0, 0, 0, 1, 0, 0, 0, 1, 0, 0) \mapsto (D, E, N, U)$
$(\mathbf{1}, \mathbf{1}, \bar{\mathbf{4}}, \mathbf{2}, \mathbf{1}, \mathbf{1})$, $(0, 0, 0, 0, 0, 0, 0, 0, 1, 1, 0, 0) \mapsto (D, E, N, U)$
$(\mathbf{4}, \mathbf{1}, \mathbf{1}, \mathbf{1}, \mathbf{2}, \mathbf{1})$, $(1, 0, 0, 0, 0, 0, 0, 0, 0, 0, 1, 0) \mapsto (L, Q)$
$(\mathbf{1}, \mathbf{4}, \mathbf{1}, \mathbf{1}, \mathbf{2}, \mathbf{1})$, $(0, 0, 0, 1, 0, 0, 0, 0, 0, 0, 1, 0) \mapsto (L, Q)$
$(\mathbf{1}, \mathbf{1}, \mathbf{4}, \mathbf{1}, \mathbf{1}, \mathbf{2})$, $(0, 0, 0, 0, 0, 0, 1, 0, 0, 0, 0, 1) \mapsto (L, Q)$
Projection matrix for $\alpha$:

$$\begin{pmatrix} 1 & 0 & 0 & 1 & 0 & 0 & 1 & 0 & 0 & 0 & 0 & 0 \\ 0 & 1 & 0 & 0 & 1 & 0 & 0 & 1 & 0 & 0 & 0 & 0 \\ 0 & 0 & 0 & 0 & 0 & 0 & 0 & 0 & 0 & 0 & 1 & 1 \\ 1 & 2 & 3 & 1 & 2 & 3 & 1 & 2 & 3 & 3 & 0 & 0 \end{pmatrix}$$

**3 generation subalgebra** 304
Algebra: $\mathfrak{su}(4) \oplus \mathfrak{su}(4) \oplus \mathfrak{su}(5) \oplus \mathfrak{su}(2) \oplus \mathfrak{su}(2) \oplus \mathfrak{su}(2)$
$(\mathbf{1}, \mathbf{1}, \bar{\mathbf{5}}, \mathbf{1}, \mathbf{1}, \mathbf{1})$, $(0, 0, 0, 0, 0, 0, 0, 0, 0, 1, 0, 0, 0) \mapsto (D, L)$
$(\mathbf{1}, \mathbf{1}, \mathbf{10}, \mathbf{1}, \mathbf{1}, \mathbf{1})$, $(0, 0, 0, 0, 0, 0, 0, 1, 0, 0, 0, 0, 0) \mapsto (E, Q, U)$
$(\bar{\mathbf{4}}, \mathbf{1}, \mathbf{1}, \mathbf{2}, \mathbf{1}, \mathbf{1})$, $(0, 0, 1, 0, 0, 0, 0, 0, 0, 0, 1, 0, 0) \mapsto (L, Q)$
$(\mathbf{1}, \bar{\mathbf{4}}, \mathbf{1}, \mathbf{2}, \mathbf{1}, \mathbf{1})$, $(0, 0, 0, 0, 0, 1, 0, 0, 0, 0, 1, 0, 0) \mapsto (L, Q)$
$(\mathbf{4}, \mathbf{1}, \mathbf{1}, \mathbf{1}, \mathbf{2}, \mathbf{1})$, $(1, 0, 0, 0, 0, 0, 0, 0, 0, 0, 0, 1, 0) \mapsto (D, E, N, U)$
$(\mathbf{1}, \mathbf{4}, \mathbf{1}, \mathbf{1}, \mathbf{1}, \mathbf{2})$, $(0, 0, 0, 1, 0, 0, 0, 0, 0, 0, 0, 0, 1) \mapsto (D, E, N, U)$
$(\mathbf{1}, \mathbf{1}, \mathbf{1}, \mathbf{1}, \mathbf{1}, \mathbf{1})$, $(0, 0, 0, 0, 0, 0, 0, 0, 0, 0, 0, 0, 0) \mapsto (N)$
Projection matrix for $\alpha$:

$$\begin{pmatrix} 0 & 1 & 0 & 0 & 1 & 0 & 0 & 0 & 1 & 0 & 0 & 0 & 0 \\ 1 & 0 & 0 & 1 & 0 & 0 & 0 & 0 & 0 & 1 & 0 & 0 & 0 \\ 0 & 0 & 0 & 0 & 0 & 0 & 1 & 0 & 0 & 0 & 1 & 0 & 0 \\ -1 & -2 & -3 & -1 & -2 & -3 & 3 & 6 & 4 & 2 & 0 & 3 & 3 \end{pmatrix}$$

**3 generation subalgebra** 305
Algebra: $\mathfrak{su}(4) \oplus \mathfrak{su}(4) \oplus \mathfrak{su}(5) \oplus \mathfrak{su}(2) \oplus \mathfrak{su}(2) \oplus \mathfrak{su}(2)$
$(\mathbf{1}, \mathbf{1}, \bar{\mathbf{5}}, \mathbf{1}, \mathbf{1}, \mathbf{1})$, $(0, 0, 0, 0, 0, 0, 0, 0, 0, 1, 0, 0, 0) \mapsto (D, L)$
$(\mathbf{1}, \mathbf{1}, \mathbf{10}, \mathbf{1}, \mathbf{1}, \mathbf{1})$, $(0, 0, 0, 0, 0, 0, 0, 1, 0, 0, 0, 0, 0) \mapsto (E, Q, U)$
$(\bar{\mathbf{4}}, \mathbf{1}, \mathbf{1}, \mathbf{2}, \mathbf{1}, \mathbf{1})$, $(0, 0, 1, 0, 0, 0, 0, 0, 0, 0, 1, 0, 0) \mapsto (D, E, N, U)$
$(\mathbf{1}, \bar{\mathbf{4}}, \mathbf{1}, \mathbf{2}, \mathbf{1}, \mathbf{1})$, $(0, 0, 0, 0, 0, 1, 0, 0, 0, 0, 1, 0, 0) \mapsto (D, E, N, U)$
$(\mathbf{4}, \mathbf{1}, \mathbf{1}, \mathbf{1}, \mathbf{2}, \mathbf{1})$, $(1, 0, 0, 0, 0, 0, 0, 0, 0, 0, 0, 1, 0) \mapsto (L, Q)$
$(\mathbf{1}, \mathbf{4}, \mathbf{1}, \mathbf{1}, \mathbf{1}, \mathbf{2})$, $(0, 0, 0, 1, 0, 0, 0, 0, 0, 0, 0, 0, 1) \mapsto (L, Q)$
$(\mathbf{1}, \mathbf{1}, \mathbf{1}, \mathbf{1}, \mathbf{1}, \mathbf{1})$, $(0, 0, 0, 0, 0, 0, 0, 0, 0, 0, 0, 0, 0) \mapsto (N)$
Projection matrix for $\alpha$:

$$\begin{pmatrix} 1 & 0 & 0 & 1 & 0 & 0 & 0 & 0 & 1 & 0 & 0 & 0 & 0 \\ 0 & 1 & 0 & 0 & 1 & 0 & 0 & 0 & 0 & 1 & 0 & 0 & 0 \\ 0 & 0 & 0 & 0 & 0 & 0 & 1 & 0 & 0 & 0 & 0 & 1 & 1 \\ 1 & 2 & 3 & 1 & 2 & 3 & 3 & 6 & 4 & 2 & 3 & 0 & 0 \end{pmatrix}$$

**3 generation subalgebra** 306
Algebra: $\mathfrak{su}(4) \oplus \mathfrak{su}(5) \oplus \mathfrak{su}(2) \oplus \mathfrak{su}(2) \oplus \mathfrak{su}(2) \oplus \mathfrak{su}(2)$
$(\mathbf{1}, \overline{\mathbf{5}}, \mathbf{1}, \mathbf{1}, \mathbf{1}, \mathbf{1})$, $(0,0,0,0,0,0,1,0,0,0,0) \mapsto (D, L)$
$(\mathbf{1}, \mathbf{10}, \mathbf{1}, \mathbf{1}, \mathbf{1}, \mathbf{1})$, $(0,0,0,0,1,0,0,0,0,0,0) \mapsto (E, Q, U)$
$(\mathbf{4}, \mathbf{1}, \mathbf{2}, \mathbf{2}, \mathbf{1}, \mathbf{1})$, $(1,0,0,0,0,0,0,1,1,0,0) \mapsto (L, L, Q, Q)$
$(\overline{\mathbf{4}}, \mathbf{1}, \mathbf{1}, \mathbf{1}, \mathbf{2}, \mathbf{2})$, $(0,0,1,0,0,0,0,0,0,1,1) \mapsto (D, D, E, E, N, N, U, U)$
$(\mathbf{1}, \mathbf{1}, \mathbf{1}, \mathbf{1}, \mathbf{1}, \mathbf{1})$, $(0,0,0,0,0,0,0,0,0,0,0) \mapsto (N)$
Projection matrix for $\alpha$:

$$\begin{pmatrix} 1 & 0 & 0 & 0 & 0 & 1 & 0 & 0 & 0 & 0 & 0 \\ 0 & 1 & 0 & 0 & 0 & 0 & 1 & 0 & 0 & 0 & 0 \\ 0 & 0 & 0 & 1 & 0 & 0 & 0 & 1 & 0 & 0 & 0 \\ 1 & 2 & 3 & 3 & 6 & 4 & 2 & 0 & 0 & 3 & 0 \end{pmatrix}$$

**3 generation subalgebra** 307
Algebra: $\mathfrak{su}(4) \oplus \mathfrak{su}(5) \oplus \mathfrak{su}(2) \oplus \mathfrak{su}(2) \oplus \mathfrak{su}(2) \oplus \mathfrak{su}(2)$
$(\overline{\mathbf{4}}, \mathbf{1}, \mathbf{2}, \mathbf{1}, \mathbf{1}, \mathbf{1})$, $(0,0,1,0,0,0,0,1,0,0,0) \mapsto (L, Q)$
$(\mathbf{4}, \mathbf{1}, \mathbf{1}, \mathbf{2}, \mathbf{1}, \mathbf{1})$, $(1,0,0,0,0,0,0,0,1,0,0) \mapsto (D, E, N, U)$
$(\mathbf{1}, \overline{\mathbf{5}}, \mathbf{1}, \mathbf{1}, \mathbf{2}, \mathbf{1})$, $(0,0,0,0,0,0,1,0,0,1,0) \mapsto (D, D, L, L)$
$(\mathbf{1}, \mathbf{10}, \mathbf{1}, \mathbf{1}, \mathbf{1}, \mathbf{2})$, $(0,0,0,0,1,0,0,0,0,0,1) \mapsto (E, E, Q, Q, U, U)$
$(\mathbf{1}, \mathbf{1}, \mathbf{1}, \mathbf{1}, \mathbf{1}, \mathbf{1})$, $(0,0,0,0,0,0,0,0,0,0,0) \mapsto (N)$
$(\mathbf{1}, \mathbf{1}, \mathbf{1}, \mathbf{1}, \mathbf{1}, \mathbf{1})$, $(0,0,0,0,0,0,0,0,0,0,0) \mapsto (N)$
Projection matrix for $\alpha$:

$$\begin{pmatrix} 0 & 1 & 0 & 0 & 0 & 1 & 0 & 0 & 0 & 0 & 0 \\ 1 & 0 & 0 & 0 & 0 & 0 & 1 & 0 & 0 & 0 & 0 \\ 0 & 0 & 0 & 1 & 0 & 0 & 0 & 1 & 0 & 0 & 0 \\ -1 & -2 & -3 & 3 & 6 & 4 & 2 & 0 & 3 & 0 & 0 \end{pmatrix}$$

**3 generation subalgebra** 308
Algebra: $\mathfrak{su}(4) \oplus \mathfrak{su}(5) \oplus \mathfrak{su}(2) \oplus \mathfrak{su}(2) \oplus \mathfrak{su}(2) \oplus \mathfrak{su}(2)$
$(\mathbf{1}, \overline{\mathbf{5}}, \mathbf{1}, \mathbf{1}, \mathbf{1}, \mathbf{1})$, $(0,0,0,0,0,0,1,0,0,0,0) \mapsto (D, L)$
$(\mathbf{1}, \mathbf{10}, \mathbf{1}, \mathbf{1}, \mathbf{1}, \mathbf{1})$, $(0,0,0,0,1,0,0,0,0,0,0) \mapsto (E, Q, U)$
$(\mathbf{4}, \mathbf{1}, \mathbf{2}, \mathbf{2}, \mathbf{1}, \mathbf{1})$, $(1,0,0,0,0,0,0,1,1,0,0) \mapsto (D, D, E, E, N, N, U, U)$
$(\overline{\mathbf{4}}, \mathbf{1}, \mathbf{1}, \mathbf{1}, \mathbf{2}, \mathbf{1})$, $(0,0,1,0,0,0,0,0,0,1,0) \mapsto (L, Q)$
$(\overline{\mathbf{4}}, \mathbf{1}, \mathbf{1}, \mathbf{1}, \mathbf{1}, \mathbf{2})$, $(0,0,1,0,0,0,0,0,0,0,1) \mapsto (L, Q)$
$(\mathbf{1}, \mathbf{1}, \mathbf{1}, \mathbf{1}, \mathbf{1}, \mathbf{1})$, $(0,0,0,0,0,0,0,0,0,0,0) \mapsto (N)$
Projection matrix for $\alpha$:

$$\begin{pmatrix} 0 & 1 & 0 & 0 & 0 & 1 & 0 & 0 & 0 & 0 & 0 \\ 1 & 0 & 0 & 0 & 0 & 0 & 1 & 0 & 0 & 0 & 0 \\ 0 & 0 & 0 & 1 & 0 & 0 & 0 & 0 & 0 & 1 & 1 \\ -1 & -2 & -3 & 3 & 6 & 4 & 2 & 3 & 0 & 0 & 0 \end{pmatrix}$$

**3 generation subalgebra** 309
Algebra: $\mathfrak{su}(4) \oplus \mathfrak{su}(5) \oplus \mathfrak{su}(2) \oplus \mathfrak{su}(2) \oplus \mathfrak{su}(2) \oplus \mathfrak{su}(2)$
$(\mathbf{1}, \overline{\mathbf{5}}, \mathbf{1}, \mathbf{1}, \mathbf{1}, \mathbf{1})$, $(0,0,0,0,0,0,1,0,0,0,0) \mapsto (D, L)$
$(\mathbf{1}, \mathbf{10}, \mathbf{1}, \mathbf{1}, \mathbf{1}, \mathbf{1})$, $(0,0,0,0,1,0,0,0,0,0,0) \mapsto (E, Q, U)$
$(\mathbf{4}, \mathbf{1}, \mathbf{2}, \mathbf{2}, \mathbf{1}, \mathbf{1})$, $(1,0,0,0,0,0,0,1,1,0,0) \mapsto (L, L, Q, Q)$
$(\overline{\mathbf{4}}, \mathbf{1}, \mathbf{1}, \mathbf{1}, \mathbf{2}, \mathbf{1})$, $(0,0,1,0,0,0,0,0,0,1,0) \mapsto (D, E, N, U)$
$(\overline{\mathbf{4}}, \mathbf{1}, \mathbf{1}, \mathbf{1}, \mathbf{1}, \mathbf{2})$, $(0,0,1,0,0,0,0,0,0,0,1) \mapsto (D, E, N, U)$
$(\mathbf{1}, \mathbf{1}, \mathbf{1}, \mathbf{1}, \mathbf{1}, \mathbf{1})$, $(0,0,0,0,0,0,0,0,0,0,0) \mapsto (N)$
Projection matrix for $\alpha$:

$$\begin{pmatrix} 1 & 0 & 0 & 0 & 0 & 1 & 0 & 0 & 0 & 0 & 0 \\ 0 & 1 & 0 & 0 & 0 & 0 & 1 & 0 & 0 & 0 & 0 \\ 0 & 0 & 0 & 1 & 0 & 0 & 0 & 1 & 0 & 0 & 0 \\ 1 & 2 & 3 & 3 & 6 & 4 & 2 & 0 & 0 & 3 & 3 \end{pmatrix}$$

**3 generation subalgebra** 310
Algebra: $\mathfrak{su}(4) \oplus \mathfrak{su}(5) \oplus \mathfrak{su}(2) \oplus \mathfrak{su}(2) \oplus \mathfrak{su}(2) \oplus \mathfrak{su}(2)$

$(\bar{\mathbf{4}},\mathbf{1},\mathbf{2},\mathbf{1},\mathbf{1},\mathbf{1})$, $(0,0,1,0,0,0,0,1,0,0,0) \mapsto (L,Q)$
$(\mathbf{4},\mathbf{1},\mathbf{1},\mathbf{2},\mathbf{1},\mathbf{1})$, $(1,0,0,0,0,0,0,0,1,0,0) \mapsto (D,E,N,U)$
$(\mathbf{1},\bar{\mathbf{5}},\mathbf{1},\mathbf{1},\mathbf{2},\mathbf{1})$, $(0,0,0,0,0,0,1,0,0,1,0) \mapsto (D,D,L,L)$
$(\mathbf{1},\mathbf{10},\mathbf{1},\mathbf{1},\mathbf{1},\mathbf{2})$, $(0,0,0,0,1,0,0,0,0,0,1) \mapsto (E,E,Q,Q,U,U)$
$(\mathbf{1},\mathbf{1},\mathbf{1},\mathbf{1},\mathbf{1},\mathbf{2})$, $(0,0,0,0,0,0,0,0,0,0,1) \mapsto (N,N)$
Projection matrix for $\alpha$:

$$\begin{pmatrix} 0 & 1 & 0 & 0 & 0 & 1 & 0 & 0 & 0 & 0 & 0 \\ 1 & 0 & 0 & 0 & 0 & 0 & 1 & 0 & 0 & 0 & 0 \\ 0 & 0 & 0 & 1 & 0 & 0 & 0 & 1 & 0 & 0 & 0 \\ -1 & -2 & -3 & 3 & 6 & 4 & 2 & 0 & 3 & 0 & 0 \end{pmatrix}$$

**3 generation subalgebra** 311
Algebra: $\mathfrak{su}(4) \oplus \mathfrak{su}(5) \oplus \mathfrak{su}(2) \oplus \mathfrak{su}(2) \oplus \mathfrak{su}(2) \oplus \mathfrak{su}(2)$
$(\bar{\mathbf{4}},\mathbf{1},\mathbf{2},\mathbf{1},\mathbf{1},\mathbf{1})$, $(0,0,1,0,0,0,0,1,0,0,0) \mapsto (L,Q)$
$(\mathbf{4},\mathbf{1},\mathbf{1},\mathbf{2},\mathbf{1},\mathbf{1})$, $(1,0,0,0,0,0,0,0,1,0,0) \mapsto (D,E,N,U)$
$(\mathbf{1},\bar{\mathbf{5}},\mathbf{1},\mathbf{1},\mathbf{2},\mathbf{1})$, $(0,0,0,0,0,0,1,0,0,1,0) \mapsto (D,D,L,L)$
$(\mathbf{1},\mathbf{10},\mathbf{1},\mathbf{1},\mathbf{1},\mathbf{2})$, $(0,0,0,0,1,0,0,0,0,0,1) \mapsto (E,E,Q,Q,U,U)$
$(\mathbf{1},\mathbf{1},\mathbf{1},\mathbf{1},\mathbf{2},\mathbf{1})$, $(0,0,0,0,0,0,0,0,0,1,0) \mapsto (N,N)$
Projection matrix for $\alpha$:

$$\begin{pmatrix} 0 & 1 & 0 & 0 & 0 & 1 & 0 & 0 & 0 & 0 & 0 \\ 1 & 0 & 0 & 0 & 0 & 0 & 1 & 0 & 0 & 0 & 0 \\ 0 & 0 & 0 & 1 & 0 & 0 & 0 & 1 & 0 & 0 & 0 \\ -1 & -2 & -3 & 3 & 6 & 4 & 2 & 0 & 3 & 0 & 0 \end{pmatrix}$$

**3 generation subalgebra** 312
Algebra: $\mathfrak{su}(4) \oplus \mathfrak{su}(5) \oplus \mathfrak{su}(2) \oplus \mathfrak{su}(2) \oplus \mathfrak{su}(2) \oplus \mathfrak{su}(2)$
$(\bar{\mathbf{4}},\mathbf{1},\mathbf{2},\mathbf{1},\mathbf{1},\mathbf{1})$, $(0,0,1,0,0,0,0,1,0,0,0) \mapsto (L,Q)$
$(\mathbf{4},\mathbf{1},\mathbf{1},\mathbf{2},\mathbf{1},\mathbf{1})$, $(1,0,0,0,0,0,0,0,1,0,0) \mapsto (D,E,N,U)$
$(\mathbf{1},\bar{\mathbf{5}},\mathbf{1},\mathbf{1},\mathbf{2},\mathbf{1})$, $(0,0,0,0,0,0,1,0,0,1,0) \mapsto (D,D,L,L)$
$(\mathbf{1},\mathbf{10},\mathbf{1},\mathbf{1},\mathbf{2},\mathbf{1})$, $(0,0,0,0,1,0,0,0,0,1,0) \mapsto (E,E,Q,Q,U,U)$
$(\mathbf{1},\mathbf{1},\mathbf{1},\mathbf{1},\mathbf{1},\mathbf{2})$, $(0,0,0,0,0,0,0,0,0,0,1) \mapsto (N,N)$
Projection matrix for $\alpha$:

$$\begin{pmatrix} 0 & 1 & 0 & 0 & 0 & 1 & 0 & 0 & 0 & 0 & 0 \\ 1 & 0 & 0 & 0 & 0 & 0 & 1 & 0 & 0 & 0 & 0 \\ 0 & 0 & 0 & 1 & 0 & 0 & 0 & 1 & 0 & 0 & 0 \\ -1 & -2 & -3 & 3 & 6 & 4 & 2 & 0 & 3 & 0 & 0 \end{pmatrix}$$

**3 generation subalgebra** 313
Algebra: $\mathfrak{su}(4) \oplus \mathfrak{su}(5) \oplus \mathfrak{su}(2) \oplus \mathfrak{su}(2) \oplus \mathfrak{su}(2) \oplus \mathfrak{su}(2)$
$(\mathbf{1},\bar{\mathbf{5}},\mathbf{1},\mathbf{1},\mathbf{1},\mathbf{1})$, $(0,0,0,0,0,0,1,0,0,0,0) \mapsto (D,L)$
$(\mathbf{1},\bar{\mathbf{5}},\mathbf{1},\mathbf{1},\mathbf{1},\mathbf{1})$, $(0,0,0,0,0,0,1,0,0,0,0) \mapsto (D,L)$
$(\bar{\mathbf{4}},\mathbf{1},\mathbf{2},\mathbf{1},\mathbf{1},\mathbf{1})$, $(0,0,1,0,0,0,0,1,0,0,0) \mapsto (L,Q)$
$(\mathbf{4},\mathbf{1},\mathbf{1},\mathbf{2},\mathbf{1},\mathbf{1})$, $(1,0,0,0,0,0,0,0,1,0,0) \mapsto (D,E,N,U)$
$(\mathbf{1},\mathbf{10},\mathbf{1},\mathbf{1},\mathbf{2},\mathbf{1})$, $(0,0,0,0,1,0,0,0,0,1,0) \mapsto (E,E,Q,Q,U,U)$
$(\mathbf{1},\mathbf{1},\mathbf{1},\mathbf{1},\mathbf{1},\mathbf{2})$, $(0,0,0,0,0,0,0,0,0,0,1) \mapsto (N,N)$
Projection matrix for $\alpha$:

$$\begin{pmatrix} 0 & 1 & 0 & 0 & 0 & 1 & 0 & 0 & 0 & 0 & 0 \\ 1 & 0 & 0 & 0 & 0 & 0 & 1 & 0 & 0 & 0 & 0 \\ 0 & 0 & 0 & 1 & 0 & 0 & 0 & 1 & 0 & 0 & 0 \\ -1 & -2 & -3 & 3 & 6 & 4 & 2 & 0 & 3 & 0 & 0 \end{pmatrix}$$

**3 generation subalgebra** 314
Algebra: $\mathfrak{su}(4) \oplus \mathfrak{su}(5) \oplus \mathfrak{su}(2) \oplus \mathfrak{su}(2) \oplus \mathfrak{su}(2) \oplus \mathfrak{su}(2)$
$(\mathbf{1},\bar{\mathbf{5}},\mathbf{1},\mathbf{1},\mathbf{1},\mathbf{1})$, $(0,0,0,0,0,0,1,0,0,0,0) \mapsto (D,L)$
$(\mathbf{1},\mathbf{10},\mathbf{1},\mathbf{1},\mathbf{1},\mathbf{1})$, $(0,0,0,0,1,0,0,0,0,0,0) \mapsto (E,Q,U)$
$(\bar{\mathbf{4}},\mathbf{1},\mathbf{2},\mathbf{1},\mathbf{1},\mathbf{1})$, $(0,0,1,0,0,0,0,1,0,0,0) \mapsto (L,Q)$

$(\overline{\mathbf{4}}, \mathbf{1}, \mathbf{1}, \mathbf{2}, \mathbf{1}, \mathbf{1})$, $(0,0,1,0,0,0,0,0,1,0,0) \mapsto (L, Q)$
$(\mathbf{4}, \mathbf{1}, \mathbf{1}, \mathbf{1}, \mathbf{2}, \mathbf{1})$, $(1,0,0,0,0,0,0,0,0,1,0) \mapsto (D, E, N, U)$
$(\mathbf{4}, \mathbf{1}, \mathbf{1}, \mathbf{1}, \mathbf{1}, \mathbf{2})$, $(1,0,0,0,0,0,0,0,0,0,1) \mapsto (D, E, N, U)$
$(\mathbf{1}, \mathbf{1}, \mathbf{1}, \mathbf{1}, \mathbf{1}, \mathbf{1})$, $(0,0,0,0,0,0,0,0,0,0,0) \mapsto (N)$
Projection matrix for $\alpha$:

$$\begin{pmatrix} 0 & 1 & 0 & 0 & 0 & 1 & 0 & 0 & 0 & 0 & 0 \\ 1 & 0 & 0 & 0 & 0 & 0 & 1 & 0 & 0 & 0 & 0 \\ 0 & 0 & 0 & 1 & 0 & 0 & 0 & 1 & 1 & 0 & 0 \\ -1 & -2 & -3 & 3 & 6 & 4 & 2 & 0 & 0 & 3 & 3 \end{pmatrix}$$

**3 generation subalgebra** 315
Algebra: $\mathfrak{su}(4) \oplus \mathfrak{su}(5) \oplus \mathfrak{su}(2) \oplus \mathfrak{su}(2) \oplus \mathfrak{su}(2) \oplus \mathfrak{su}(2)$
$(\mathbf{1}, \mathbf{10}, \mathbf{1}, \mathbf{1}, \mathbf{1}, \mathbf{1})$, $(0,0,0,0,1,0,0,0,0,0,0) \mapsto (E, Q, U)$
$(\mathbf{1}, \mathbf{10}, \mathbf{1}, \mathbf{1}, \mathbf{1}, \mathbf{1})$, $(0,0,0,0,1,0,0,0,0,0,0) \mapsto (E, Q, U)$
$(\overline{\mathbf{4}}, \mathbf{1}, \mathbf{2}, \mathbf{1}, \mathbf{1}, \mathbf{1})$, $(0,0,1,0,0,0,0,1,0,0,0) \mapsto (L, Q)$
$(\mathbf{4}, \mathbf{1}, \mathbf{1}, \mathbf{2}, \mathbf{1}, \mathbf{1})$, $(1,0,0,0,0,0,0,0,1,0,0) \mapsto (D, E, N, U)$
$(\mathbf{1}, \overline{\mathbf{5}}, \mathbf{1}, \mathbf{1}, \mathbf{2}, \mathbf{1})$, $(0,0,0,0,0,0,1,0,0,1,0) \mapsto (D, D, L, L)$
$(\mathbf{1}, \mathbf{1}, \mathbf{1}, \mathbf{1}, \mathbf{1}, \mathbf{2})$, $(0,0,0,0,0,0,0,0,0,0,1) \mapsto (N, N)$
Projection matrix for $\alpha$:

$$\begin{pmatrix} 0 & 1 & 0 & 0 & 0 & 1 & 0 & 0 & 0 & 0 & 0 \\ 1 & 0 & 0 & 0 & 0 & 0 & 1 & 0 & 0 & 0 & 0 \\ 0 & 0 & 0 & 1 & 0 & 0 & 0 & 1 & 0 & 0 & 0 \\ -1 & -2 & -3 & 3 & 6 & 4 & 2 & 0 & 3 & 0 & 0 \end{pmatrix}$$

**3 generation subalgebra** 316
Algebra: $\mathfrak{su}(4) \oplus \mathfrak{su}(5) \oplus \mathfrak{su}(5) \oplus \mathfrak{su}(2) \oplus \mathfrak{su}(2) \oplus \mathfrak{su}(2)$
$(\mathbf{1}, \overline{\mathbf{5}}, \mathbf{1}, \mathbf{1}, \mathbf{1}, \mathbf{1})$, $(0,0,0,0,0,0,1,0,0,0,0,0,0,0,0) \mapsto (D, L)$
$(\mathbf{1}, \mathbf{10}, \mathbf{1}, \mathbf{1}, \mathbf{1}, \mathbf{1})$, $(0,0,0,0,1,0,0,0,0,0,0,0,0,0,0) \mapsto (E, Q, U)$
$(\mathbf{1}, \mathbf{1}, \overline{\mathbf{5}}, \mathbf{1}, \mathbf{1}, \mathbf{1})$, $(0,0,0,0,0,0,0,0,0,0,1,0,0,0,0) \mapsto (D, L)$
$(\mathbf{1}, \mathbf{1}, \mathbf{10}, \mathbf{1}, \mathbf{1}, \mathbf{1})$, $(0,0,0,0,0,0,0,0,1,0,0,0,0,0,0) \mapsto (E, Q, U)$
$(\overline{\mathbf{4}}, \mathbf{1}, \mathbf{1}, \mathbf{2}, \mathbf{1}, \mathbf{1})$, $(0,0,1,0,0,0,0,0,0,0,0,0,1,0,0) \mapsto (L, Q)$
$(\mathbf{4}, \mathbf{1}, \mathbf{1}, \mathbf{1}, \mathbf{2}, \mathbf{1})$, $(1,0,0,0,0,0,0,0,0,0,0,0,0,1,0) \mapsto (D, E, N, U)$
$(\mathbf{1}, \mathbf{1}, \mathbf{1}, \mathbf{1}, \mathbf{1}, \mathbf{2})$, $(0,0,0,0,0,0,0,0,0,0,0,0,0,0,1) \mapsto (N, N)$
Projection matrix for $\alpha$:

$$\begin{pmatrix} 0 & 1 & 0 & 0 & 0 & 1 & 0 & 0 & 0 & 1 & 0 & 0 & 0 & 0 & 0 \\ 1 & 0 & 0 & 0 & 0 & 0 & 1 & 0 & 0 & 0 & 1 & 0 & 0 & 0 & 0 \\ 0 & 0 & 0 & 1 & 0 & 0 & 0 & 1 & 0 & 0 & 0 & 1 & 0 & 0 & 0 \\ -1 & -2 & -3 & 3 & 6 & 4 & 2 & 3 & 6 & 4 & 2 & 0 & 3 & 0 & 0 \end{pmatrix}$$

**3 generation subalgebra** 317
Algebra: $\mathfrak{su}(4) \oplus \mathfrak{su}(8) \oplus \mathfrak{su}(2) \oplus \mathfrak{su}(2) \oplus \mathfrak{su}(2) \oplus \mathfrak{su}(2)$
$(\overline{\mathbf{4}}, \mathbf{1}, \mathbf{2}, \mathbf{1}, \mathbf{1}, \mathbf{1})$, $(0,0,1,0,0,0,0,0,0,0,1,0,0,0) \mapsto (L, Q)$
$(\mathbf{4}, \mathbf{1}, \mathbf{1}, \mathbf{2}, \mathbf{1}, \mathbf{1})$, $(1,0,0,0,0,0,0,0,0,0,0,1,0,0) \mapsto (D, E, N, U)$
$(\mathbf{1}, \overline{\mathbf{8}}, \mathbf{1}, \mathbf{1}, \mathbf{2}, \mathbf{1})$, $(0,0,0,0,0,0,0,0,0,1,0,0,1,0) \mapsto (L, L, Q, Q)$
$(\mathbf{1}, \mathbf{8}, \mathbf{1}, \mathbf{1}, \mathbf{1}, \mathbf{2})$, $(0,0,0,1,0,0,0,0,0,0,0,0,0,1) \mapsto (D, D, E, E, N, N, U, U)$
Projection matrix for $\alpha$:

$$\begin{pmatrix} 0 & 1 & 0 & 0 & 1 & 0 & 0 & 1 & 0 & 0 & 0 & 0 & 0 & 0 \\ 1 & 0 & 0 & 1 & 0 & 0 & 1 & 0 & 0 & 0 & 0 & 0 & 0 & 0 \\ 0 & 0 & 0 & 0 & 0 & 0 & 0 & 0 & 0 & 0 & 1 & 0 & 1 & 0 \\ -1 & -2 & -3 & -1 & -2 & -3 & -4 & -5 & -6 & -3 & 0 & 3 & 0 & 3 \end{pmatrix}$$

**3 generation subalgebra** 318
Algebra: $\mathfrak{su}(4) \oplus \mathfrak{su}(2) \oplus \mathfrak{su}(2) \oplus \mathfrak{su}(2) \oplus \mathfrak{su}(2) \oplus \mathfrak{su}(2) \oplus \mathfrak{su}(2)$
$(\mathbf{4}, \mathbf{2}, \mathbf{2}, \mathbf{1}, \mathbf{1}, \mathbf{1}, \mathbf{1})$, $(1,0,0,1,1,0,0,0,0) \mapsto (D, D, E, E, N, N, U, U)$
$(\overline{\mathbf{4}}, \mathbf{1}, \mathbf{1}, \mathbf{2}, \mathbf{2}, \mathbf{1}, \mathbf{1})$, $(0,0,1,0,0,1,1,0,0) \mapsto (L, L, Q, Q)$
$(\overline{\mathbf{4}}, \mathbf{1}, \mathbf{1}, \mathbf{1}, \mathbf{1}, \mathbf{2}, \mathbf{1})$, $(0,0,1,0,0,0,0,1,0) \mapsto (L, Q)$

$(\mathbf{4},\mathbf{1},\mathbf{1},\mathbf{1},\mathbf{1},\mathbf{1},\mathbf{2})$, $(1,0,0,0,0,0,0,0,1) \mapsto (D,E,N,U)$
Projection matrix for $\alpha$:

$$\begin{pmatrix} 0 & 1 & 0 & 0 & 0 & 0 & 0 & 0 & 0 \\ 1 & 0 & 0 & 0 & 0 & 0 & 0 & 0 & 0 \\ 0 & 0 & 0 & 0 & 0 & 1 & 0 & 1 & 0 \\ -1 & -2 & -3 & 3 & 0 & 0 & 0 & 0 & 3 \end{pmatrix}$$

**3 generation subalgebra** 319
Algebra: $\mathfrak{su}(4) \oplus \mathfrak{su}(2) \oplus \mathfrak{su}(2) \oplus \mathfrak{su}(2) \oplus \mathfrak{su}(2) \oplus \mathfrak{su}(2) \oplus \mathfrak{su}(2)$
$(\mathbf{4},\mathbf{2},\mathbf{2},\mathbf{1},\mathbf{1},\mathbf{1},\mathbf{1})$, $(1,0,0,1,1,0,0,0,0) \mapsto (D,D,E,E,N,N,U,U)$
$(\overline{\mathbf{4}},\mathbf{1},\mathbf{1},\mathbf{2},\mathbf{1},\mathbf{1},\mathbf{1})$, $(0,0,1,0,0,1,0,0,0) \mapsto (L,Q)$
$(\overline{\mathbf{4}},\mathbf{1},\mathbf{1},\mathbf{1},\mathbf{2},\mathbf{1},\mathbf{1})$, $(0,0,1,0,0,0,1,0,0) \mapsto (L,Q)$
$(\overline{\mathbf{4}},\mathbf{1},\mathbf{1},\mathbf{1},\mathbf{1},\mathbf{2},\mathbf{1})$, $(0,0,1,0,0,0,0,1,0) \mapsto (L,Q)$
$(\mathbf{4},\mathbf{1},\mathbf{1},\mathbf{1},\mathbf{1},\mathbf{1},\mathbf{2})$, $(1,0,0,0,0,0,0,0,1) \mapsto (D,E,N,U)$
Projection matrix for $\alpha$:

$$\begin{pmatrix} 0 & 1 & 0 & 0 & 0 & 0 & 0 & 0 & 0 \\ 1 & 0 & 0 & 0 & 0 & 0 & 0 & 0 & 0 \\ 0 & 0 & 0 & 0 & 0 & 1 & 1 & 1 & 0 \\ -1 & -2 & -3 & 3 & 0 & 0 & 0 & 0 & 3 \end{pmatrix}$$

**3 generation subalgebra** 320
Algebra: $\mathfrak{su}(4) \oplus \mathfrak{su}(2) \oplus \mathfrak{su}(2) \oplus \mathfrak{su}(2) \oplus \mathfrak{su}(2) \oplus \mathfrak{su}(2) \oplus \mathfrak{su}(2)$
$(\mathbf{4},\mathbf{2},\mathbf{2},\mathbf{1},\mathbf{1},\mathbf{1},\mathbf{1})$, $(1,0,0,1,1,0,0,0,0) \mapsto (L,L,Q,Q)$
$(\overline{\mathbf{4}},\mathbf{1},\mathbf{1},\mathbf{2},\mathbf{1},\mathbf{1},\mathbf{1})$, $(0,0,1,0,0,1,0,0,0) \mapsto (D,E,N,U)$
$(\overline{\mathbf{4}},\mathbf{1},\mathbf{1},\mathbf{1},\mathbf{2},\mathbf{1},\mathbf{1})$, $(0,0,1,0,0,0,1,0,0) \mapsto (D,E,N,U)$
$(\overline{\mathbf{4}},\mathbf{1},\mathbf{1},\mathbf{1},\mathbf{1},\mathbf{2},\mathbf{1})$, $(0,0,1,0,0,0,0,1,0) \mapsto (D,E,N,U)$
$(\mathbf{4},\mathbf{1},\mathbf{1},\mathbf{1},\mathbf{1},\mathbf{1},\mathbf{2})$, $(1,0,0,0,0,0,0,0,1) \mapsto (L,Q)$
Projection matrix for $\alpha$:

$$\begin{pmatrix} 1 & 0 & 0 & 0 & 0 & 0 & 0 & 0 & 0 \\ 0 & 1 & 0 & 0 & 0 & 0 & 0 & 0 & 0 \\ 0 & 0 & 0 & 1 & 0 & 0 & 0 & 0 & 1 \\ 1 & 2 & 3 & 0 & 0 & 3 & 3 & 3 & 0 \end{pmatrix}$$

**3 generation subalgebra** 321
Algebra: $\mathfrak{su}(4) \oplus \mathfrak{su}(2) \oplus \mathfrak{su}(2) \oplus \mathfrak{su}(2) \oplus \mathfrak{su}(2) \oplus \mathfrak{su}(2) \oplus \mathfrak{su}(2)$
$(\overline{\mathbf{4}},\mathbf{2},\mathbf{1},\mathbf{1},\mathbf{1},\mathbf{1},\mathbf{1})$, $(0,0,1,1,0,0,0,0,0) \mapsto (L,Q)$
$(\overline{\mathbf{4}},\mathbf{1},\mathbf{2},\mathbf{1},\mathbf{1},\mathbf{1},\mathbf{1})$, $(0,0,1,0,1,0,0,0,0) \mapsto (L,Q)$
$(\overline{\mathbf{4}},\mathbf{1},\mathbf{1},\mathbf{2},\mathbf{1},\mathbf{1},\mathbf{1})$, $(0,0,1,0,0,1,0,0,0) \mapsto (L,Q)$
$(\mathbf{4},\mathbf{1},\mathbf{1},\mathbf{1},\mathbf{2},\mathbf{1},\mathbf{1})$, $(1,0,0,0,0,0,1,0,0) \mapsto (D,E,N,U)$
$(\mathbf{4},\mathbf{1},\mathbf{1},\mathbf{1},\mathbf{1},\mathbf{2},\mathbf{1})$, $(1,0,0,0,0,0,0,1,0) \mapsto (D,E,N,U)$
$(\mathbf{4},\mathbf{1},\mathbf{1},\mathbf{1},\mathbf{1},\mathbf{1},\mathbf{2})$, $(1,0,0,0,0,0,0,0,1) \mapsto (D,E,N,U)$
Projection matrix for $\alpha$:

$$\begin{pmatrix} 0 & 1 & 0 & 0 & 0 & 0 & 0 & 0 & 0 \\ 1 & 0 & 0 & 0 & 0 & 0 & 0 & 0 & 0 \\ 0 & 0 & 0 & 1 & 1 & 1 & 0 & 0 & 0 \\ -1 & -2 & -3 & 0 & 0 & 0 & 3 & 3 & 3 \end{pmatrix}$$

**3 generation subalgebra** 322
Algebra: $\mathfrak{su}(4) \oplus \mathfrak{su}(4) \oplus \mathfrak{so}(10) \oplus \mathfrak{su}(2) \oplus \mathfrak{su}(2) \oplus \mathfrak{su}(2) \oplus \mathfrak{su}(2)$
$(\mathbf{1},\mathbf{1},\mathbf{16},\mathbf{1},\mathbf{1},\mathbf{1},\mathbf{1})$, $(0,0,0,0,0,0,0,0,0,0,1,0,0,0,0) \mapsto (D,E,L,N,Q,U)$
$(\overline{\mathbf{4}},\mathbf{1},\mathbf{1},\mathbf{2},\mathbf{1},\mathbf{1},\mathbf{1})$, $(0,0,1,0,0,0,0,0,0,0,0,1,0,0,0) \mapsto (L,Q)$
$(\mathbf{4},\mathbf{1},\mathbf{1},\mathbf{1},\mathbf{2},\mathbf{1},\mathbf{1})$, $(1,0,0,0,0,0,0,0,0,0,0,0,1,0,0) \mapsto (D,E,N,U)$
$(\mathbf{1},\overline{\mathbf{4}},\mathbf{1},\mathbf{1},\mathbf{1},\mathbf{2},\mathbf{1})$, $(0,0,0,0,0,1,0,0,0,0,0,0,0,1,0) \mapsto (L,Q)$
$(\mathbf{1},\mathbf{4},\mathbf{1},\mathbf{1},\mathbf{1},\mathbf{1},\mathbf{2})$, $(0,0,0,1,0,0,0,0,0,0,0,0,0,0,1) \mapsto (D,E,N,U)$

Projection matrix for $\alpha$:

$$\begin{pmatrix} 0 & 1 & 0 & 0 & 1 & 0 & 0 & 0 & 1 & 0 & 0 & 0 & 0 & 0 & 0 \\ 1 & 0 & 0 & 1 & 0 & 0 & 0 & 0 & 0 & 0 & 1 & 0 & 0 & 0 & 0 \\ 0 & 0 & 0 & 0 & 0 & 0 & 1 & 0 & 0 & 0 & 0 & 1 & 0 & 1 & 0 \\ -1 & -2 & -3 & -1 & -2 & -3 & 3 & 6 & 4 & 0 & 2 & 0 & 3 & 0 & 3 \end{pmatrix}$$

**3 generation subalgebra** 323
Algebra: $\mathfrak{su}(4) \oplus \mathfrak{su}(4) \oplus \mathfrak{sp}(4) \oplus \mathfrak{su}(2) \oplus \mathfrak{su}(2) \oplus \mathfrak{su}(2) \oplus \mathfrak{su}(2)$
$(\bar{\mathbf{4}}, \mathbf{1}, \mathbf{4}, \mathbf{1}, \mathbf{1}, \mathbf{1}, \mathbf{1})$, $(0,0,1,0,0,0,1,0,0,0,0,0) \mapsto (L, L, Q, Q)$
$(\mathbf{4}, \mathbf{1}, \mathbf{1}, \mathbf{2}, \mathbf{2}, \mathbf{1}, \mathbf{1})$, $(1,0,0,0,0,0,0,0,1,1,0,0) \mapsto (D, D, E, E, N, N, U, U)$
$(\mathbf{1}, \bar{\mathbf{4}}, \mathbf{1}, \mathbf{1}, \mathbf{1}, \mathbf{2}, \mathbf{1})$, $(0,0,0,0,0,1,0,0,0,0,1,0) \mapsto (L, Q)$
$(\mathbf{1}, \mathbf{4}, \mathbf{1}, \mathbf{1}, \mathbf{1}, \mathbf{1}, \mathbf{2})$, $(0,0,0,1,0,0,0,0,0,0,0,1) \mapsto (D, E, N, U)$
Projection matrix for $\alpha$:

$$\begin{pmatrix} 0 & 1 & 0 & 0 & 1 & 0 & 0 & 0 & 0 & 0 & 0 & 0 \\ 1 & 0 & 0 & 1 & 0 & 0 & 0 & 0 & 0 & 0 & 0 & 0 \\ 0 & 0 & 0 & 0 & 0 & 0 & 1 & 2 & 0 & 0 & 1 & 0 \\ -1 & -2 & -3 & -1 & -2 & -3 & 0 & 0 & 3 & 0 & 0 & 3 \end{pmatrix}$$

**3 generation subalgebra** 324
Algebra: $\mathfrak{su}(4) \oplus \mathfrak{su}(4) \oplus \mathfrak{sp}(4) \oplus \mathfrak{su}(2) \oplus \mathfrak{su}(2) \oplus \mathfrak{su}(2) \oplus \mathfrak{su}(2)$
$(\bar{\mathbf{4}}, \mathbf{1}, \mathbf{4}, \mathbf{1}, \mathbf{1}, \mathbf{1}, \mathbf{1})$, $(0,0,1,0,0,0,1,0,0,0,0,0) \mapsto (D, D, E, E, N, N, U, U)$
$(\mathbf{4}, \mathbf{1}, \mathbf{1}, \mathbf{2}, \mathbf{2}, \mathbf{1}, \mathbf{1})$, $(1,0,0,0,0,0,0,0,1,1,0,0) \mapsto (L, L, Q, Q)$
$(\mathbf{1}, \bar{\mathbf{4}}, \mathbf{1}, \mathbf{1}, \mathbf{1}, \mathbf{2}, \mathbf{1})$, $(0,0,0,0,0,1,0,0,0,0,1,0) \mapsto (L, Q)$
$(\mathbf{1}, \mathbf{4}, \mathbf{1}, \mathbf{1}, \mathbf{1}, \mathbf{1}, \mathbf{2})$, $(0,0,0,1,0,0,0,0,0,0,0,1) \mapsto (D, E, N, U)$
Projection matrix for $\alpha$:

$$\begin{pmatrix} 1 & 0 & 0 & 0 & 1 & 0 & 0 & 0 & 0 & 0 & 0 & 0 \\ 0 & 1 & 0 & 1 & 0 & 0 & 0 & 0 & 0 & 0 & 0 & 0 \\ 0 & 0 & 0 & 0 & 0 & 0 & 0 & 0 & 1 & 0 & 1 & 0 \\ 1 & 2 & 3 & -1 & -2 & -3 & 3 & 0 & 0 & 0 & 0 & 3 \end{pmatrix}$$

**3 generation subalgebra** 325
Algebra: $\mathfrak{su}(4) \oplus \mathfrak{su}(4) \oplus \mathfrak{sp}(4) \oplus \mathfrak{su}(2) \oplus \mathfrak{su}(2) \oplus \mathfrak{su}(2) \oplus \mathfrak{su}(2)$
$(\bar{\mathbf{4}}, \mathbf{1}, \mathbf{4}, \mathbf{1}, \mathbf{1}, \mathbf{1}, \mathbf{1})$, $(0,0,1,0,0,0,1,0,0,0,0,0) \mapsto (L, L, Q, Q)$
$(\mathbf{4}, \mathbf{1}, \mathbf{1}, \mathbf{2}, \mathbf{1}, \mathbf{1}, \mathbf{1})$, $(1,0,0,0,0,0,0,0,1,0,0,0) \mapsto (D, E, N, U)$
$(\mathbf{4}, \mathbf{1}, \mathbf{1}, \mathbf{1}, \mathbf{2}, \mathbf{1}, \mathbf{1})$, $(1,0,0,0,0,0,0,0,0,1,0,0) \mapsto (D, E, N, U)$
$(\mathbf{1}, \bar{\mathbf{4}}, \mathbf{1}, \mathbf{1}, \mathbf{1}, \mathbf{2}, \mathbf{1})$, $(0,0,0,0,0,1,0,0,0,0,1,0) \mapsto (L, Q)$
$(\mathbf{1}, \mathbf{4}, \mathbf{1}, \mathbf{1}, \mathbf{1}, \mathbf{1}, \mathbf{2})$, $(0,0,0,1,0,0,0,0,0,0,0,1) \mapsto (D, E, N, U)$
Projection matrix for $\alpha$:

$$\begin{pmatrix} 0 & 1 & 0 & 0 & 1 & 0 & 0 & 0 & 0 & 0 & 0 & 0 \\ 1 & 0 & 0 & 1 & 0 & 0 & 0 & 0 & 0 & 0 & 0 & 0 \\ 0 & 0 & 0 & 0 & 0 & 0 & 1 & 2 & 0 & 0 & 1 & 0 \\ -1 & -2 & -3 & -1 & -2 & -3 & 0 & 0 & 3 & 3 & 0 & 3 \end{pmatrix}$$

**3 generation subalgebra** 326
Algebra: $\mathfrak{su}(4) \oplus \mathfrak{su}(4) \oplus \mathfrak{sp}(4) \oplus \mathfrak{su}(2) \oplus \mathfrak{su}(2) \oplus \mathfrak{su}(2) \oplus \mathfrak{su}(2)$
$(\bar{\mathbf{4}}, \mathbf{1}, \mathbf{4}, \mathbf{1}, \mathbf{1}, \mathbf{1}, \mathbf{1})$, $(0,0,1,0,0,0,1,0,0,0,0,0) \mapsto (D, D, E, E, N, N, U, U)$
$(\mathbf{4}, \mathbf{1}, \mathbf{1}, \mathbf{2}, \mathbf{1}, \mathbf{1}, \mathbf{1})$, $(1,0,0,0,0,0,0,0,1,0,0,0) \mapsto (L, Q)$
$(\mathbf{4}, \mathbf{1}, \mathbf{1}, \mathbf{1}, \mathbf{2}, \mathbf{1}, \mathbf{1})$, $(1,0,0,0,0,0,0,0,0,1,0,0) \mapsto (L, Q)$
$(\mathbf{1}, \bar{\mathbf{4}}, \mathbf{1}, \mathbf{1}, \mathbf{1}, \mathbf{2}, \mathbf{1})$, $(0,0,0,0,0,1,0,0,0,0,1,0) \mapsto (L, Q)$
$(\mathbf{1}, \mathbf{4}, \mathbf{1}, \mathbf{1}, \mathbf{1}, \mathbf{1}, \mathbf{2})$, $(0,0,0,1,0,0,0,0,0,0,0,1) \mapsto (D, E, N, U)$
Projection matrix for $\alpha$:

$$\begin{pmatrix} 1 & 0 & 0 & 0 & 1 & 0 & 0 & 0 & 0 & 0 & 0 & 0 \\ 0 & 1 & 0 & 1 & 0 & 0 & 0 & 0 & 0 & 0 & 0 & 0 \\ 0 & 0 & 0 & 0 & 0 & 0 & 0 & 0 & 1 & 1 & 1 & 0 \\ 1 & 2 & 3 & -1 & -2 & -3 & 3 & 0 & 0 & 0 & 0 & 3 \end{pmatrix}$$

**3 generation subalgebra** 327
Algebra: $\mathfrak{su}(4) \oplus \mathfrak{su}(4) \oplus \mathfrak{su}(2) \oplus \mathfrak{su}(2) \oplus \mathfrak{su}(2) \oplus \mathfrak{su}(2) \oplus \mathfrak{su}(2)$
$(\mathbf{4}, \mathbf{1}, \mathbf{2}, \mathbf{2}, \mathbf{1}, \mathbf{1}, \mathbf{1}),\ (1,0,0,0,0,0,1,1,0,0,0) \mapsto (D, D, E, E, N, N, U, U)$
$(\mathbf{1}, \bar{\mathbf{4}}, \mathbf{2}, \mathbf{1}, \mathbf{1}, \mathbf{1}, \mathbf{1}),\ (0,0,0,0,0,1,1,0,0,0,0) \mapsto (D, E, N, U)$
$(\bar{\mathbf{4}}, \mathbf{1}, \mathbf{1}, \mathbf{1}, \mathbf{2}, \mathbf{2}, \mathbf{1}),\ (0,0,1,0,0,0,0,0,1,1,0) \mapsto (L, L, Q, Q)$
$(\mathbf{1}, \mathbf{4}, \mathbf{1}, \mathbf{1}, \mathbf{1}, \mathbf{1}, \mathbf{2}),\ (0,0,0,1,0,0,0,0,0,0,1) \mapsto (L, Q)$
Projection matrix for $\alpha$:

$$\begin{pmatrix} 0 & 1 & 0 & 1 & 0 & 0 & 0 & 0 & 0 & 0 & 0 \\ 1 & 0 & 0 & 0 & 1 & 0 & 0 & 0 & 0 & 0 & 0 \\ 0 & 0 & 0 & 0 & 0 & 0 & 0 & 1 & 0 & 1 \\ -1 & -2 & -3 & 1 & 2 & 3 & 3 & 0 & 0 & 0 & 0 \end{pmatrix}$$

**3 generation subalgebra** 328
Algebra: $\mathfrak{su}(4) \oplus \mathfrak{su}(4) \oplus \mathfrak{su}(2) \oplus \mathfrak{su}(2) \oplus \mathfrak{su}(2) \oplus \mathfrak{su}(2) \oplus \mathfrak{su}(2)$
$(\mathbf{4}, \mathbf{1}, \mathbf{2}, \mathbf{2}, \mathbf{1}, \mathbf{1}, \mathbf{1}),\ (1,0,0,0,0,0,1,1,0,0,0) \mapsto (L, L, Q, Q)$
$(\mathbf{1}, \bar{\mathbf{4}}, \mathbf{2}, \mathbf{1}, \mathbf{1}, \mathbf{1}, \mathbf{1}),\ (0,0,0,0,0,1,1,0,0,0,0) \mapsto (L, Q)$
$(\bar{\mathbf{4}}, \mathbf{1}, \mathbf{1}, \mathbf{1}, \mathbf{2}, \mathbf{2}, \mathbf{1}),\ (0,0,1,0,0,0,0,0,1,1,0) \mapsto (D, D, E, E, N, N, U, U)$
$(\mathbf{1}, \mathbf{4}, \mathbf{1}, \mathbf{1}, \mathbf{1}, \mathbf{1}, \mathbf{2}),\ (0,0,0,1,0,0,0,0,0,0,1) \mapsto (D, E, N, U)$
Projection matrix for $\alpha$:

$$\begin{pmatrix} 1 & 0 & 0 & 0 & 1 & 0 & 0 & 0 & 0 & 0 & 0 \\ 0 & 1 & 0 & 1 & 0 & 0 & 0 & 0 & 0 & 0 & 0 \\ 0 & 0 & 0 & 0 & 0 & 0 & 1 & 0 & 0 & 0 & 0 \\ 1 & 2 & 3 & -1 & -2 & -3 & 0 & 0 & 3 & 0 & 3 \end{pmatrix}$$

**3 generation subalgebra** 329
Algebra: $\mathfrak{su}(4) \oplus \mathfrak{su}(4) \oplus \mathfrak{su}(2) \oplus \mathfrak{su}(2) \oplus \mathfrak{su}(2) \oplus \mathfrak{su}(2) \oplus \mathfrak{su}(2)$
$(\mathbf{4}, \mathbf{1}, \mathbf{2}, \mathbf{2}, \mathbf{1}, \mathbf{1}, \mathbf{1}),\ (1,0,0,0,0,0,1,1,0,0,0) \mapsto (L, L, Q, Q)$
$(\bar{\mathbf{4}}, \mathbf{1}, \mathbf{2}, \mathbf{1}, \mathbf{2}, \mathbf{1}, \mathbf{1}),\ (0,0,1,0,0,0,1,0,1,0,0) \mapsto (D, D, E, E, N, N, U, U)$
$(\mathbf{1}, \bar{\mathbf{4}}, \mathbf{1}, \mathbf{1}, \mathbf{1}, \mathbf{2}, \mathbf{1}),\ (0,0,0,0,0,1,0,0,0,1,0) \mapsto (L, Q)$
$(\mathbf{1}, \mathbf{4}, \mathbf{1}, \mathbf{1}, \mathbf{1}, \mathbf{1}, \mathbf{2}),\ (0,0,0,1,0,0,0,0,0,0,1) \mapsto (D, E, N, U)$
Projection matrix for $\alpha$:

$$\begin{pmatrix} 1 & 0 & 0 & 0 & 1 & 0 & 0 & 0 & 0 & 0 & 0 \\ 0 & 1 & 0 & 1 & 0 & 0 & 0 & 0 & 0 & 0 & 0 \\ 0 & 0 & 0 & 0 & 0 & 0 & 0 & 1 & 0 & 1 & 0 \\ 1 & 2 & 3 & -1 & -2 & -3 & 0 & 0 & 3 & 0 & 3 \end{pmatrix}$$

**3 generation subalgebra** 330
Algebra: $\mathfrak{su}(4) \oplus \mathfrak{su}(4) \oplus \mathfrak{su}(2) \oplus \mathfrak{su}(2) \oplus \mathfrak{su}(2) \oplus \mathfrak{su}(2) \oplus \mathfrak{su}(2)$
$(\mathbf{4}, \mathbf{1}, \mathbf{2}, \mathbf{2}, \mathbf{1}, \mathbf{1}, \mathbf{1}),\ (1,0,0,0,0,0,1,1,0,0,0) \mapsto (D, D, E, E, N, N, U, U)$
$(\mathbf{1}, \bar{\mathbf{4}}, \mathbf{2}, \mathbf{1}, \mathbf{1}, \mathbf{1}, \mathbf{1}),\ (0,0,0,0,0,1,1,0,0,0,0) \mapsto (D, E, N, U)$
$(\bar{\mathbf{4}}, \mathbf{1}, \mathbf{1}, \mathbf{1}, \mathbf{2}, \mathbf{1}, \mathbf{1}),\ (0,0,1,0,0,0,0,0,1,0,0) \mapsto (L, Q)$
$(\bar{\mathbf{4}}, \mathbf{1}, \mathbf{1}, \mathbf{1}, \mathbf{1}, \mathbf{2}, \mathbf{1}),\ (0,0,1,0,0,0,0,0,0,1,0) \mapsto (L, Q)$
$(\mathbf{1}, \mathbf{4}, \mathbf{1}, \mathbf{1}, \mathbf{1}, \mathbf{1}, \mathbf{2}),\ (0,0,0,1,0,0,0,0,0,0,1) \mapsto (L, Q)$
Projection matrix for $\alpha$:

$$\begin{pmatrix} 0 & 1 & 0 & 1 & 0 & 0 & 0 & 0 & 0 & 0 & 0 \\ 1 & 0 & 0 & 0 & 1 & 0 & 0 & 0 & 0 & 0 & 0 \\ 0 & 0 & 0 & 0 & 0 & 0 & 0 & 0 & 1 & 1 & 1 \\ -1 & -2 & -3 & 1 & 2 & 3 & 3 & 0 & 0 & 0 & 0 \end{pmatrix}$$

**3 generation subalgebra** 331
Algebra: $\mathfrak{su}(4) \oplus \mathfrak{su}(4) \oplus \mathfrak{su}(2) \oplus \mathfrak{su}(2) \oplus \mathfrak{su}(2) \oplus \mathfrak{su}(2) \oplus \mathfrak{su}(2)$
$(\mathbf{4}, \mathbf{1}, \mathbf{2}, \mathbf{2}, \mathbf{1}, \mathbf{1}, \mathbf{1}),\ (1,0,0,0,0,0,1,1,0,0,0) \mapsto (L, L, Q, Q)$
$(\mathbf{1}, \bar{\mathbf{4}}, \mathbf{2}, \mathbf{1}, \mathbf{1}, \mathbf{1}, \mathbf{1}),\ (0,0,0,0,0,1,1,0,0,0,0) \mapsto (L, Q)$
$(\bar{\mathbf{4}}, \mathbf{1}, \mathbf{1}, \mathbf{1}, \mathbf{2}, \mathbf{1}, \mathbf{1}),\ (0,0,1,0,0,0,0,0,1,0,0) \mapsto (D, E, N, U)$
$(\bar{\mathbf{4}}, \mathbf{1}, \mathbf{1}, \mathbf{1}, \mathbf{1}, \mathbf{2}, \mathbf{1}),\ (0,0,1,0,0,0,0,0,0,1,0) \mapsto (D, E, N, U)$

$(\mathbf{1},\mathbf{4},\mathbf{1},\mathbf{1},\mathbf{1},\mathbf{1},\mathbf{2}),\ (0,0,0,1,0,0,0,0,0,0,1) \mapsto (D,E,N,U)$
Projection matrix for $\alpha$:

$$\begin{pmatrix} 1 & 0 & 0 & 0 & 1 & 0 & 0 & 0 & 0 & 0 & 0 \\ 0 & 1 & 0 & 1 & 0 & 0 & 0 & 0 & 0 & 0 & 0 \\ 0 & 0 & 0 & 0 & 0 & 0 & 1 & 0 & 0 & 0 & 0 \\ 1 & 2 & 3 & -1 & -2 & -3 & 0 & 0 & 3 & 3 & 3 \end{pmatrix}$$

**3 generation subalgebra** 332
Algebra: $\mathfrak{su}(4) \oplus \mathfrak{su}(4) \oplus \mathfrak{su}(2) \oplus \mathfrak{su}(2) \oplus \mathfrak{su}(2) \oplus \mathfrak{su}(2) \oplus \mathfrak{su}(2)$
$(\mathbf{4},\mathbf{1},\mathbf{2},\mathbf{2},\mathbf{1},\mathbf{1},\mathbf{1}),\ (1,0,0,0,0,0,1,1,0,0,0) \mapsto (D,D,E,E,N,N,U,U)$
$(\overline{\mathbf{4}},\mathbf{1},\mathbf{1},\mathbf{1},\mathbf{2},\mathbf{1},\mathbf{1}),\ (0,0,1,0,0,0,0,0,1,0,0) \mapsto (L,Q)$
$(\mathbf{1},\overline{\mathbf{4}},\mathbf{1},\mathbf{1},\mathbf{2},\mathbf{1},\mathbf{1}),\ (0,0,0,0,0,1,0,0,1,0,0) \mapsto (L,Q)$
$(\overline{\mathbf{4}},\mathbf{1},\mathbf{1},\mathbf{1},\mathbf{1},\mathbf{2},\mathbf{1}),\ (0,0,1,0,0,0,0,0,0,1,0) \mapsto (L,Q)$
$(\mathbf{1},\mathbf{4},\mathbf{1},\mathbf{1},\mathbf{1},\mathbf{1},\mathbf{2}),\ (0,0,0,1,0,0,0,0,0,0,1) \mapsto (D,E,N,U)$
Projection matrix for $\alpha$:

$$\begin{pmatrix} 0 & 1 & 0 & 0 & 1 & 0 & 0 & 0 & 0 & 0 & 0 \\ 1 & 0 & 0 & 1 & 0 & 0 & 0 & 0 & 0 & 0 & 0 \\ 0 & 0 & 0 & 0 & 0 & 0 & 0 & 0 & 1 & 1 & 0 \\ -1 & -2 & -3 & -1 & -2 & -3 & 3 & 0 & 0 & 0 & 3 \end{pmatrix}$$

**3 generation subalgebra** 333
Algebra: $\mathfrak{su}(4) \oplus \mathfrak{su}(4) \oplus \mathfrak{su}(2) \oplus \mathfrak{su}(2) \oplus \mathfrak{su}(2) \oplus \mathfrak{su}(2) \oplus \mathfrak{su}(2)$
$(\mathbf{4},\mathbf{1},\mathbf{2},\mathbf{2},\mathbf{1},\mathbf{1},\mathbf{1}),\ (1,0,0,0,0,0,1,1,0,0,0) \mapsto (L,L,Q,Q)$
$(\overline{\mathbf{4}},\mathbf{1},\mathbf{1},\mathbf{1},\mathbf{2},\mathbf{1},\mathbf{1}),\ (0,0,1,0,0,0,0,0,1,0,0) \mapsto (D,E,N,U)$
$(\mathbf{1},\overline{\mathbf{4}},\mathbf{1},\mathbf{1},\mathbf{2},\mathbf{1},\mathbf{1}),\ (0,0,0,0,0,1,0,0,1,0,0) \mapsto (D,E,N,U)$
$(\overline{\mathbf{4}},\mathbf{1},\mathbf{1},\mathbf{1},\mathbf{1},\mathbf{2},\mathbf{1}),\ (0,0,1,0,0,0,0,0,0,1,0) \mapsto (D,E,N,U)$
$(\mathbf{1},\mathbf{4},\mathbf{1},\mathbf{1},\mathbf{1},\mathbf{1},\mathbf{2}),\ (0,0,0,1,0,0,0,0,0,0,1) \mapsto (L,Q)$
Projection matrix for $\alpha$:

$$\begin{pmatrix} 1 & 0 & 0 & 1 & 0 & 0 & 0 & 0 & 0 & 0 & 0 \\ 0 & 1 & 0 & 0 & 1 & 0 & 0 & 0 & 0 & 0 & 0 \\ 0 & 0 & 0 & 0 & 0 & 0 & 1 & 0 & 0 & 0 & 1 \\ 1 & 2 & 3 & 1 & 2 & 3 & 0 & 0 & 3 & 3 & 0 \end{pmatrix}$$

**3 generation subalgebra** 334
Algebra: $\mathfrak{su}(4) \oplus \mathfrak{su}(4) \oplus \mathfrak{su}(2) \oplus \mathfrak{su}(2) \oplus \mathfrak{su}(2) \oplus \mathfrak{su}(2) \oplus \mathfrak{su}(2)$
$(\mathbf{4},\mathbf{1},\mathbf{2},\mathbf{2},\mathbf{1},\mathbf{1},\mathbf{1}),\ (1,0,0,0,0,0,1,1,0,0,0) \mapsto (D,D,E,E,N,N,U,U)$
$(\overline{\mathbf{4}},\mathbf{1},\mathbf{1},\mathbf{1},\mathbf{2},\mathbf{1},\mathbf{1}),\ (0,0,1,0,0,0,0,0,1,0,0) \mapsto (L,Q)$
$(\overline{\mathbf{4}},\mathbf{1},\mathbf{1},\mathbf{1},\mathbf{2},\mathbf{1},\mathbf{1}),\ (0,0,1,0,0,0,0,0,1,0,0) \mapsto (L,Q)$
$(\mathbf{1},\overline{\mathbf{4}},\mathbf{1},\mathbf{1},\mathbf{1},\mathbf{2},\mathbf{1}),\ (0,0,0,0,0,1,0,0,0,1,0) \mapsto (L,Q)$
$(\mathbf{1},\mathbf{4},\mathbf{1},\mathbf{1},\mathbf{1},\mathbf{1},\mathbf{2}),\ (0,0,0,1,0,0,0,0,0,0,1) \mapsto (D,E,N,U)$
Projection matrix for $\alpha$:

$$\begin{pmatrix} 0 & 1 & 0 & 0 & 1 & 0 & 0 & 0 & 0 & 0 & 0 \\ 1 & 0 & 0 & 1 & 0 & 0 & 0 & 0 & 0 & 0 & 0 \\ 0 & 0 & 0 & 0 & 0 & 0 & 0 & 0 & 1 & 1 & 0 \\ -1 & -2 & -3 & -1 & -2 & -3 & 3 & 0 & 0 & 0 & 3 \end{pmatrix}$$

**3 generation subalgebra** 335
Algebra: $\mathfrak{su}(4) \oplus \mathfrak{su}(4) \oplus \mathfrak{su}(2) \oplus \mathfrak{su}(2) \oplus \mathfrak{su}(2) \oplus \mathfrak{su}(2) \oplus \mathfrak{su}(2)$
$(\mathbf{4},\mathbf{1},\mathbf{2},\mathbf{2},\mathbf{1},\mathbf{1},\mathbf{1}),\ (1,0,0,0,0,0,1,1,0,0,0) \mapsto (L,L,Q,Q)$
$(\overline{\mathbf{4}},\mathbf{1},\mathbf{1},\mathbf{1},\mathbf{2},\mathbf{1},\mathbf{1}),\ (0,0,1,0,0,0,0,0,1,0,0) \mapsto (D,E,N,U)$
$(\overline{\mathbf{4}},\mathbf{1},\mathbf{1},\mathbf{1},\mathbf{2},\mathbf{1},\mathbf{1}),\ (0,0,1,0,0,0,0,0,1,0,0) \mapsto (D,E,N,U)$
$(\mathbf{1},\overline{\mathbf{4}},\mathbf{1},\mathbf{1},\mathbf{1},\mathbf{2},\mathbf{1}),\ (0,0,0,0,0,1,0,0,0,1,0) \mapsto (L,Q)$
$(\mathbf{1},\mathbf{4},\mathbf{1},\mathbf{1},\mathbf{1},\mathbf{1},\mathbf{2}),\ (0,0,0,1,0,0,0,0,0,0,1) \mapsto (D,E,N,U)$
Projection matrix for $\alpha$:

$$\begin{pmatrix} 1 & 0 & 0 & 0 & 1 & 0 & 0 & 0 & 0 & 0 & 0 \\ 0 & 1 & 0 & 1 & 0 & 0 & 0 & 0 & 0 & 0 & 0 \\ 0 & 0 & 0 & 0 & 0 & 0 & 1 & 0 & 0 & 1 & 0 \\ 1 & 2 & 3 & -1 & -2 & -3 & 0 & 0 & 3 & 0 & 3 \end{pmatrix}$$

**3 generation subalgebra** 336
Algebra: $\mathfrak{su}(4) \oplus \mathfrak{su}(4) \oplus \mathfrak{su}(2) \oplus \mathfrak{su}(2) \oplus \mathfrak{su}(2) \oplus \mathfrak{su}(2) \oplus \mathfrak{su}(2)$
$(\overline{\mathbf{4}}, \mathbf{1}, \mathbf{2}, \mathbf{1}, \mathbf{1}, \mathbf{1}, \mathbf{1})$, $(0,0,1,0,0,0,1,0,0,0,0) \mapsto (L, Q)$
$(\mathbf{1}, \overline{\mathbf{4}}, \mathbf{2}, \mathbf{1}, \mathbf{1}, \mathbf{1}, \mathbf{1})$, $(0,0,0,0,0,1,1,0,0,0,0) \mapsto (L, Q)$
$(\overline{\mathbf{4}}, \mathbf{1}, \mathbf{1}, \mathbf{2}, \mathbf{1}, \mathbf{1}, \mathbf{1})$, $(0,0,1,0,0,0,0,1,0,0,0) \mapsto (L, Q)$
$(\mathbf{4}, \mathbf{1}, \mathbf{1}, \mathbf{1}, \mathbf{2}, \mathbf{1}, \mathbf{1})$, $(1,0,0,0,0,0,0,0,1,0,0) \mapsto (D, E, N, U)$
$(\mathbf{4}, \mathbf{1}, \mathbf{1}, \mathbf{1}, \mathbf{1}, \mathbf{2}, \mathbf{1})$, $(1,0,0,0,0,0,0,0,0,1,0) \mapsto (D, E, N, U)$
$(\mathbf{1}, \mathbf{4}, \mathbf{1}, \mathbf{1}, \mathbf{1}, \mathbf{1}, \mathbf{2})$, $(0,0,0,1,0,0,0,0,0,0,1) \mapsto (D, E, N, U)$
Projection matrix for $\alpha$:

$$\begin{pmatrix} 0 & 1 & 0 & 0 & 1 & 0 & 0 & 0 & 0 & 0 & 0 \\ 1 & 0 & 0 & 1 & 0 & 0 & 0 & 0 & 0 & 0 & 0 \\ 0 & 0 & 0 & 0 & 0 & 0 & 1 & 1 & 0 & 0 & 0 \\ -1 & -2 & -3 & -1 & -2 & -3 & 0 & 0 & 3 & 3 & 3 \end{pmatrix}$$

**3 generation subalgebra** 337
Algebra: $\mathfrak{su}(4) \oplus \mathfrak{su}(4) \oplus \mathfrak{su}(2) \oplus \mathfrak{su}(2) \oplus \mathfrak{su}(2) \oplus \mathfrak{su}(2) \oplus \mathfrak{su}(2)$
$(\overline{\mathbf{4}}, \mathbf{1}, \mathbf{2}, \mathbf{1}, \mathbf{1}, \mathbf{1}, \mathbf{1})$, $(0,0,1,0,0,0,1,0,0,0,0) \mapsto (D, E, N, U)$
$(\mathbf{1}, \overline{\mathbf{4}}, \mathbf{2}, \mathbf{1}, \mathbf{1}, \mathbf{1}, \mathbf{1})$, $(0,0,0,0,0,1,1,0,0,0,0) \mapsto (D, E, N, U)$
$(\overline{\mathbf{4}}, \mathbf{1}, \mathbf{1}, \mathbf{2}, \mathbf{1}, \mathbf{1}, \mathbf{1})$, $(0,0,1,0,0,0,0,1,0,0,0) \mapsto (D, E, N, U)$
$(\mathbf{4}, \mathbf{1}, \mathbf{1}, \mathbf{1}, \mathbf{2}, \mathbf{1}, \mathbf{1})$, $(1,0,0,0,0,0,0,0,1,0,0) \mapsto (L, Q)$
$(\mathbf{4}, \mathbf{1}, \mathbf{1}, \mathbf{1}, \mathbf{1}, \mathbf{2}, \mathbf{1})$, $(1,0,0,0,0,0,0,0,0,1,0) \mapsto (L, Q)$
$(\mathbf{1}, \mathbf{4}, \mathbf{1}, \mathbf{1}, \mathbf{1}, \mathbf{1}, \mathbf{2})$, $(0,0,0,1,0,0,0,0,0,0,1) \mapsto (L, Q)$
Projection matrix for $\alpha$:

$$\begin{pmatrix} 1 & 0 & 0 & 1 & 0 & 0 & 0 & 0 & 0 & 0 & 0 \\ 0 & 1 & 0 & 0 & 1 & 0 & 0 & 0 & 0 & 0 & 0 \\ 0 & 0 & 0 & 0 & 0 & 0 & 0 & 0 & 1 & 1 & 1 \\ 1 & 2 & 3 & 1 & 2 & 3 & 3 & 3 & 0 & 0 & 0 \end{pmatrix}$$

**3 generation subalgebra** 338
Algebra: $\mathfrak{su}(4) \oplus \mathfrak{su}(4) \oplus \mathfrak{su}(2) \oplus \mathfrak{su}(2) \oplus \mathfrak{su}(2) \oplus \mathfrak{su}(2) \oplus \mathfrak{su}(2)$
$(\overline{\mathbf{4}}, \mathbf{1}, \mathbf{2}, \mathbf{1}, \mathbf{1}, \mathbf{1}, \mathbf{1})$, $(0,0,1,0,0,0,1,0,0,0,0) \mapsto (L, Q)$
$(\overline{\mathbf{4}}, \mathbf{1}, \mathbf{2}, \mathbf{1}, \mathbf{1}, \mathbf{1}, \mathbf{1})$, $(0,0,1,0,0,0,1,0,0,0,0) \mapsto (L, Q)$
$(\mathbf{4}, \mathbf{1}, \mathbf{1}, \mathbf{2}, \mathbf{1}, \mathbf{1}, \mathbf{1})$, $(1,0,0,0,0,0,0,1,0,0,0) \mapsto (D, E, N, U)$
$(\mathbf{4}, \mathbf{1}, \mathbf{1}, \mathbf{1}, \mathbf{2}, \mathbf{1}, \mathbf{1})$, $(1,0,0,0,0,0,0,0,1,0,0) \mapsto (D, E, N, U)$
$(\mathbf{1}, \overline{\mathbf{4}}, \mathbf{1}, \mathbf{1}, \mathbf{1}, \mathbf{2}, \mathbf{1})$, $(0,0,0,0,0,1,0,0,0,1,0) \mapsto (L, Q)$
$(\mathbf{1}, \mathbf{4}, \mathbf{1}, \mathbf{1}, \mathbf{1}, \mathbf{1}, \mathbf{2})$, $(0,0,0,1,0,0,0,0,0,0,1) \mapsto (D, E, N, U)$
Projection matrix for $\alpha$:

$$\begin{pmatrix} 0 & 1 & 0 & 0 & 1 & 0 & 0 & 0 & 0 & 0 & 0 \\ 1 & 0 & 0 & 1 & 0 & 0 & 0 & 0 & 0 & 0 & 0 \\ 0 & 0 & 0 & 0 & 0 & 0 & 1 & 0 & 0 & 1 & 0 \\ -1 & -2 & -3 & -1 & -2 & -3 & 0 & 3 & 3 & 0 & 3 \end{pmatrix}$$

**3 generation subalgebra** 339
Algebra: $\mathfrak{su}(4) \oplus \mathfrak{su}(4) \oplus \mathfrak{su}(2) \oplus \mathfrak{su}(2) \oplus \mathfrak{su}(2) \oplus \mathfrak{su}(2) \oplus \mathfrak{su}(2)$
$(\overline{\mathbf{4}}, \mathbf{1}, \mathbf{2}, \mathbf{1}, \mathbf{1}, \mathbf{1}, \mathbf{1})$, $(0,0,1,0,0,0,1,0,0,0,0) \mapsto (D, E, N, U)$
$(\overline{\mathbf{4}}, \mathbf{1}, \mathbf{2}, \mathbf{1}, \mathbf{1}, \mathbf{1}, \mathbf{1})$, $(0,0,1,0,0,0,1,0,0,0,0) \mapsto (D, E, N, U)$
$(\mathbf{4}, \mathbf{1}, \mathbf{1}, \mathbf{2}, \mathbf{1}, \mathbf{1}, \mathbf{1})$, $(1,0,0,0,0,0,0,1,0,0,0) \mapsto (L, Q)$
$(\mathbf{4}, \mathbf{1}, \mathbf{1}, \mathbf{1}, \mathbf{2}, \mathbf{1}, \mathbf{1})$, $(1,0,0,0,0,0,0,0,1,0,0) \mapsto (L, Q)$
$(\mathbf{1}, \overline{\mathbf{4}}, \mathbf{1}, \mathbf{1}, \mathbf{1}, \mathbf{2}, \mathbf{1})$, $(0,0,0,0,0,1,0,0,0,1,0) \mapsto (L, Q)$
$(\mathbf{1}, \mathbf{4}, \mathbf{1}, \mathbf{1}, \mathbf{1}, \mathbf{1}, \mathbf{2})$, $(0,0,0,1,0,0,0,0,0,0,1) \mapsto (D, E, N, U)$
Projection matrix for $\alpha$:

$$\begin{pmatrix} 1 & 0 & 0 & 0 & 1 & 0 & 0 & 0 & 0 & 0 & 0 \\ 0 & 1 & 0 & 1 & 0 & 0 & 0 & 0 & 0 & 0 & 0 \\ 0 & 0 & 0 & 0 & 0 & 0 & 0 & 1 & 1 & 1 & 0 \\ 1 & 2 & 3 & -1 & -2 & -3 & 3 & 0 & 0 & 0 & 3 \end{pmatrix}$$

**3 generation subalgebra** 340
Algebra: $\mathfrak{su}(4) \oplus \mathfrak{su}(4) \oplus \mathfrak{su}(4) \oplus \mathfrak{su}(2) \oplus \mathfrak{su}(2) \oplus \mathfrak{su}(2) \oplus \mathfrak{su}(2)$
$(\overline{\mathbf{4}}, \mathbf{1}, \mathbf{1}, \mathbf{2}, \mathbf{1}, \mathbf{1}, \mathbf{1})$, $(0,0,1,0,0,0,0,0,0,1,0,0,0) \mapsto (L, Q)$
$(\mathbf{1}, \overline{\mathbf{4}}, \mathbf{1}, \mathbf{2}, \mathbf{1}, \mathbf{1}, \mathbf{1})$, $(0,0,0,0,0,1,0,0,0,1,0,0,0) \mapsto (L, Q)$
$(\mathbf{1}, \mathbf{1}, \overline{\mathbf{4}}, \mathbf{2}, \mathbf{1}, \mathbf{1}, \mathbf{1})$, $(0,0,0,0,0,0,0,0,1,1,0,0,0) \mapsto (L, Q)$
$(\mathbf{4}, \mathbf{1}, \mathbf{1}, \mathbf{1}, \mathbf{2}, \mathbf{1}, \mathbf{1})$, $(1,0,0,0,0,0,0,0,0,0,1,0,0) \mapsto (D, E, N, U)$
$(\mathbf{1}, \mathbf{4}, \mathbf{1}, \mathbf{1}, \mathbf{1}, \mathbf{2}, \mathbf{1})$, $(0,0,0,1,0,0,0,0,0,0,0,1,0) \mapsto (D, E, N, U)$
$(\mathbf{1}, \mathbf{1}, \mathbf{4}, \mathbf{1}, \mathbf{1}, \mathbf{1}, \mathbf{2})$, $(0,0,0,0,0,0,1,0,0,0,0,0,1) \mapsto (D, E, N, U)$
Projection matrix for $\alpha$:

$$\begin{pmatrix} 0 & 1 & 0 & 0 & 1 & 0 & 0 & 1 & 0 & 0 & 0 & 0 & 0 \\ 1 & 0 & 0 & 1 & 0 & 0 & 1 & 0 & 0 & 0 & 0 & 0 & 0 \\ 0 & 0 & 0 & 0 & 0 & 0 & 0 & 0 & 0 & 1 & 0 & 0 & 0 \\ -1 & -2 & -3 & -1 & -2 & -3 & -1 & -2 & -3 & 0 & 3 & 3 & 3 \end{pmatrix}$$

**3 generation subalgebra** 341
Algebra: $\mathfrak{su}(4) \oplus \mathfrak{su}(4) \oplus \mathfrak{su}(4) \oplus \mathfrak{su}(2) \oplus \mathfrak{su}(2) \oplus \mathfrak{su}(2) \oplus \mathfrak{su}(2)$
$(\overline{\mathbf{4}}, \mathbf{1}, \mathbf{1}, \mathbf{2}, \mathbf{1}, \mathbf{1}, \mathbf{1})$, $(0,0,1,0,0,0,0,0,0,1,0,0,0) \mapsto (D, E, N, U)$
$(\mathbf{1}, \overline{\mathbf{4}}, \mathbf{1}, \mathbf{2}, \mathbf{1}, \mathbf{1}, \mathbf{1})$, $(0,0,0,0,0,1,0,0,0,1,0,0,0) \mapsto (D, E, N, U)$
$(\mathbf{1}, \mathbf{1}, \overline{\mathbf{4}}, \mathbf{2}, \mathbf{1}, \mathbf{1}, \mathbf{1})$, $(0,0,0,0,0,0,0,0,1,1,0,0,0) \mapsto (D, E, N, U)$
$(\mathbf{4}, \mathbf{1}, \mathbf{1}, \mathbf{1}, \mathbf{2}, \mathbf{1}, \mathbf{1})$, $(1,0,0,0,0,0,0,0,0,0,1,0,0) \mapsto (L, Q)$
$(\mathbf{1}, \mathbf{4}, \mathbf{1}, \mathbf{1}, \mathbf{1}, \mathbf{2}, \mathbf{1})$, $(0,0,0,1,0,0,0,0,0,0,0,1,0) \mapsto (L, Q)$
$(\mathbf{1}, \mathbf{1}, \mathbf{4}, \mathbf{1}, \mathbf{1}, \mathbf{1}, \mathbf{2})$, $(0,0,0,0,0,0,1,0,0,0,0,0,1) \mapsto (L, Q)$
Projection matrix for $\alpha$:

$$\begin{pmatrix} 1 & 0 & 0 & 1 & 0 & 0 & 1 & 0 & 0 & 0 & 0 & 0 & 0 \\ 0 & 1 & 0 & 0 & 1 & 0 & 0 & 1 & 0 & 0 & 0 & 0 & 0 \\ 0 & 0 & 0 & 0 & 0 & 0 & 0 & 0 & 0 & 0 & 1 & 1 & 1 \\ 1 & 2 & 3 & 1 & 2 & 3 & 1 & 2 & 3 & 3 & 0 & 0 & 0 \end{pmatrix}$$

**3 generation subalgebra** 342
Algebra: $\mathfrak{su}(4) \oplus \mathfrak{su}(4) \oplus \mathfrak{su}(4) \oplus \mathfrak{su}(2) \oplus \mathfrak{su}(2) \oplus \mathfrak{su}(2) \oplus \mathfrak{su}(2)$
$(\overline{\mathbf{4}}, \mathbf{1}, \mathbf{1}, \mathbf{2}, \mathbf{1}, \mathbf{1}, \mathbf{1})$, $(0,0,1,0,0,0,0,0,0,1,0,0,0) \mapsto (D, E, N, U)$
$(\mathbf{1}, \overline{\mathbf{4}}, \mathbf{1}, \mathbf{2}, \mathbf{1}, \mathbf{1}, \mathbf{1})$, $(0,0,0,0,0,1,0,0,0,1,0,0,0) \mapsto (D, E, N, U)$
$(\mathbf{4}, \mathbf{1}, \mathbf{1}, \mathbf{1}, \mathbf{2}, \mathbf{1}, \mathbf{1})$, $(1,0,0,0,0,0,0,0,0,0,1,0,0) \mapsto (L, Q)$
$(\mathbf{1}, \mathbf{1}, \overline{\mathbf{4}}, \mathbf{1}, \mathbf{2}, \mathbf{1}, \mathbf{1})$, $(0,0,0,0,0,0,0,0,1,0,1,0,0) \mapsto (L, Q)$
$(\mathbf{1}, \mathbf{4}, \mathbf{1}, \mathbf{1}, \mathbf{1}, \mathbf{2}, \mathbf{1})$, $(0,0,0,1,0,0,0,0,0,0,0,1,0) \mapsto (L, Q)$
$(\mathbf{1}, \mathbf{1}, \mathbf{4}, \mathbf{1}, \mathbf{1}, \mathbf{1}, \mathbf{2})$, $(0,0,0,0,0,0,1,0,0,0,0,0,1) \mapsto (D, E, N, U)$
Projection matrix for $\alpha$:

$$\begin{pmatrix} 1 & 0 & 0 & 1 & 0 & 0 & 0 & 1 & 0 & 0 & 0 & 0 & 0 \\ 0 & 1 & 0 & 0 & 1 & 0 & 1 & 0 & 0 & 0 & 0 & 0 & 0 \\ 0 & 0 & 0 & 0 & 0 & 0 & 0 & 0 & 0 & 0 & 1 & 1 & 0 \\ 1 & 2 & 3 & 1 & 2 & 3 & -1 & -2 & -3 & 3 & 0 & 0 & 3 \end{pmatrix}$$

**3 generation subalgebra** 343
Algebra: $\mathfrak{su}(4) \oplus \mathfrak{su}(4) \oplus \mathfrak{su}(4) \oplus \mathfrak{su}(2) \oplus \mathfrak{su}(2) \oplus \mathfrak{su}(2) \oplus \mathfrak{su}(2)$
$(\overline{\mathbf{4}}, \mathbf{1}, \mathbf{1}, \mathbf{2}, \mathbf{1}, \mathbf{1}, \mathbf{1})$, $(0,0,1,0,0,0,0,0,0,1,0,0,0) \mapsto (L, Q)$
$(\mathbf{1}, \overline{\mathbf{4}}, \mathbf{1}, \mathbf{2}, \mathbf{1}, \mathbf{1}, \mathbf{1})$, $(0,0,0,0,0,1,0,0,0,1,0,0,0) \mapsto (L, Q)$
$(\mathbf{4}, \mathbf{1}, \mathbf{1}, \mathbf{1}, \mathbf{2}, \mathbf{1}, \mathbf{1})$, $(1,0,0,0,0,0,0,0,0,0,1,0,0) \mapsto (D, E, N, U)$
$(\mathbf{1}, \mathbf{4}, \mathbf{1}, \mathbf{1}, \mathbf{2}, \mathbf{1}, \mathbf{1})$, $(0,0,0,1,0,0,0,0,0,0,1,0,0) \mapsto (D, E, N, U)$
$(\mathbf{1}, \mathbf{1}, \overline{\mathbf{4}}, \mathbf{1}, \mathbf{1}, \mathbf{2}, \mathbf{1})$, $(0,0,0,0,0,0,0,0,1,0,0,1,0) \mapsto (L, Q)$
$(\mathbf{1}, \mathbf{1}, \mathbf{4}, \mathbf{1}, \mathbf{1}, \mathbf{1}, \mathbf{2})$, $(0,0,0,0,0,0,1,0,0,0,0,0,1) \mapsto (D, E, N, U)$
Projection matrix for $\alpha$:

$$\begin{pmatrix} 0 & 1 & 0 & 0 & 1 & 0 & 0 & 1 & 0 & 0 & 0 & 0 & 0 \\ 1 & 0 & 0 & 1 & 0 & 0 & 1 & 0 & 0 & 0 & 0 & 0 & 0 \\ 0 & 0 & 0 & 0 & 0 & 0 & 0 & 0 & 0 & 1 & 0 & 1 & 0 \\ -1 & -2 & -3 & -1 & -2 & -3 & -1 & -2 & -3 & 0 & 3 & 0 & 3 \end{pmatrix}$$

**3 generation subalgebra** 344
Algebra: $\mathfrak{su}(4) \oplus \mathfrak{su}(4) \oplus \mathfrak{su}(5) \oplus \mathfrak{su}(2) \oplus \mathfrak{su}(2) \oplus \mathfrak{su}(2) \oplus \mathfrak{su}(2)$
$(\mathbf{1}, \mathbf{1}, \overline{\mathbf{5}}, \mathbf{1}, \mathbf{1}, \mathbf{1}, \mathbf{1})$, $(0, 0, 0, 0, 0, 0, 0, 0, 0, 1, 0, 0, 0, 0) \mapsto (D, L)$
$(\mathbf{1}, \mathbf{1}, \mathbf{10}, \mathbf{1}, \mathbf{1}, \mathbf{1}, \mathbf{1})$, $(0, 0, 0, 0, 0, 0, 0, 1, 0, 0, 0, 0, 0, 0) \mapsto (E, Q, U)$
$(\overline{\mathbf{4}}, \mathbf{1}, \mathbf{1}, \mathbf{2}, \mathbf{1}, \mathbf{1}, \mathbf{1})$, $(0, 0, 1, 0, 0, 0, 0, 0, 0, 0, 1, 0, 0, 0) \mapsto (L, Q)$
$(\mathbf{4}, \mathbf{1}, \mathbf{1}, \mathbf{1}, \mathbf{2}, \mathbf{1}, \mathbf{1})$, $(1, 0, 0, 0, 0, 0, 0, 0, 0, 0, 0, 1, 0, 0) \mapsto (D, E, N, U)$
$(\mathbf{1}, \overline{\mathbf{4}}, \mathbf{1}, \mathbf{1}, \mathbf{1}, \mathbf{2}, \mathbf{1})$, $(0, 0, 0, 0, 0, 1, 0, 0, 0, 0, 0, 0, 1, 0) \mapsto (L, Q)$
$(\mathbf{1}, \mathbf{4}, \mathbf{1}, \mathbf{1}, \mathbf{1}, \mathbf{1}, \mathbf{2})$, $(0, 0, 0, 1, 0, 0, 0, 0, 0, 0, 0, 0, 0, 1) \mapsto (D, E, N, U)$
$(\mathbf{1}, \mathbf{1}, \mathbf{1}, \mathbf{1}, \mathbf{1}, \mathbf{1}, \mathbf{1})$, $(0, 0, 0, 0, 0, 0, 0, 0, 0, 0, 0, 0, 0, 0) \mapsto (N)$
Projection matrix for $\alpha$:

$$\begin{pmatrix} 0 & 1 & 0 & 0 & 1 & 0 & 0 & 0 & 1 & 0 & 0 & 0 & 0 & 0 \\ 1 & 0 & 0 & 1 & 0 & 0 & 0 & 0 & 0 & 1 & 0 & 0 & 0 & 0 \\ 0 & 0 & 0 & 0 & 0 & 0 & 1 & 0 & 0 & 0 & 1 & 0 & 1 & 0 \\ -1 & -2 & -3 & -1 & -2 & -3 & 3 & 6 & 4 & 2 & 0 & 3 & 0 & 3 \end{pmatrix}$$

**3 generation subalgebra** 345
Algebra: $\mathfrak{su}(4) \oplus \mathfrak{su}(5) \oplus \mathfrak{su}(2) \oplus \mathfrak{su}(2) \oplus \mathfrak{su}(2) \oplus \mathfrak{su}(2) \oplus \mathfrak{su}(2)$
$(\overline{\mathbf{4}}, \mathbf{1}, \mathbf{2}, \mathbf{1}, \mathbf{1}, \mathbf{1}, \mathbf{1})$, $(0, 0, 1, 0, 0, 0, 0, 1, 0, 0, 0, 0) \mapsto (L, Q)$
$(\mathbf{4}, \mathbf{1}, \mathbf{1}, \mathbf{2}, \mathbf{1}, \mathbf{1}, \mathbf{1})$, $(1, 0, 0, 0, 0, 0, 0, 0, 1, 0, 0, 0) \mapsto (D, E, N, U)$
$(\mathbf{1}, \overline{\mathbf{5}}, \mathbf{1}, \mathbf{1}, \mathbf{2}, \mathbf{1}, \mathbf{1})$, $(0, 0, 0, 0, 0, 0, 1, 0, 0, 1, 0, 0) \mapsto (D, D, L, L)$
$(\mathbf{1}, \mathbf{10}, \mathbf{1}, \mathbf{1}, \mathbf{1}, \mathbf{2}, \mathbf{1})$, $(0, 0, 0, 0, 1, 0, 0, 0, 0, 0, 1, 0) \mapsto (E, E, Q, Q, U, U)$
$(\mathbf{1}, \mathbf{1}, \mathbf{1}, \mathbf{1}, \mathbf{1}, \mathbf{1}, \mathbf{2})$, $(0, 0, 0, 0, 0, 0, 0, 0, 0, 0, 0, 1) \mapsto (N, N)$
Projection matrix for $\alpha$:

$$\begin{pmatrix} 0 & 1 & 0 & 0 & 0 & 1 & 0 & 0 & 0 & 0 & 0 & 0 \\ 1 & 0 & 0 & 0 & 0 & 0 & 1 & 0 & 0 & 0 & 0 & 0 \\ 0 & 0 & 0 & 1 & 0 & 0 & 0 & 1 & 0 & 0 & 0 & 0 \\ -1 & -2 & -3 & 3 & 6 & 4 & 2 & 0 & 3 & 0 & 0 & 0 \end{pmatrix}$$

**3 generation subalgebra** 346
Algebra: $\mathfrak{su}(4) \oplus \mathfrak{su}(4) \oplus \mathfrak{su}(2) \oplus \mathfrak{su}(2) \oplus \mathfrak{su}(2) \oplus \mathfrak{su}(2) \oplus \mathfrak{su}(2) \oplus \mathfrak{su}(2)$
$(\mathbf{4}, \mathbf{1}, \mathbf{2}, \mathbf{2}, \mathbf{1}, \mathbf{1}, \mathbf{1}, \mathbf{1})$, $(1, 0, 0, 0, 0, 0, 1, 1, 0, 0, 0, 0) \mapsto (L, L, Q, Q)$
$(\overline{\mathbf{4}}, \mathbf{1}, \mathbf{1}, \mathbf{1}, \mathbf{2}, \mathbf{2}, \mathbf{1}, \mathbf{1})$, $(0, 0, 1, 0, 0, 0, 0, 0, 1, 1, 0, 0) \mapsto (D, D, E, E, N, N, U, U)$
$(\mathbf{1}, \overline{\mathbf{4}}, \mathbf{1}, \mathbf{1}, \mathbf{1}, \mathbf{1}, \mathbf{2}, \mathbf{1})$, $(0, 0, 0, 0, 0, 1, 0, 0, 0, 0, 1, 0) \mapsto (L, Q)$
$(\mathbf{1}, \mathbf{4}, \mathbf{1}, \mathbf{1}, \mathbf{1}, \mathbf{1}, \mathbf{1}, \mathbf{2})$, $(0, 0, 0, 1, 0, 0, 0, 0, 0, 0, 0, 1) \mapsto (D, E, N, U)$
Projection matrix for $\alpha$:

$$\begin{pmatrix} 1 & 0 & 0 & 0 & 1 & 0 & 0 & 0 & 0 & 0 & 0 & 0 \\ 0 & 1 & 0 & 1 & 0 & 0 & 0 & 0 & 0 & 0 & 0 & 0 \\ 0 & 0 & 0 & 0 & 0 & 0 & 1 & 0 & 0 & 0 & 1 & 0 \\ 1 & 2 & 3 & -1 & -2 & -3 & 0 & 0 & 3 & 0 & 0 & 3 \end{pmatrix}$$

**3 generation subalgebra** 347
Algebra: $\mathfrak{su}(4) \oplus \mathfrak{su}(4) \oplus \mathfrak{su}(2) \oplus \mathfrak{su}(2) \oplus \mathfrak{su}(2) \oplus \mathfrak{su}(2) \oplus \mathfrak{su}(2) \oplus \mathfrak{su}(2)$
$(\mathbf{4}, \mathbf{1}, \mathbf{2}, \mathbf{2}, \mathbf{1}, \mathbf{1}, \mathbf{1}, \mathbf{1})$, $(1, 0, 0, 0, 0, 0, 1, 1, 0, 0, 0, 0) \mapsto (D, D, E, E, N, N, U, U)$
$(\overline{\mathbf{4}}, \mathbf{1}, \mathbf{1}, \mathbf{1}, \mathbf{2}, \mathbf{1}, \mathbf{1}, \mathbf{1})$, $(0, 0, 1, 0, 0, 0, 0, 0, 1, 0, 0, 0) \mapsto (L, Q)$
$(\overline{\mathbf{4}}, \mathbf{1}, \mathbf{1}, \mathbf{1}, \mathbf{1}, \mathbf{2}, \mathbf{1}, \mathbf{1})$, $(0, 0, 1, 0, 0, 0, 0, 0, 0, 1, 0, 0) \mapsto (L, Q)$
$(\mathbf{1}, \overline{\mathbf{4}}, \mathbf{1}, \mathbf{1}, \mathbf{1}, \mathbf{1}, \mathbf{2}, \mathbf{1})$, $(0, 0, 0, 0, 0, 1, 0, 0, 0, 0, 1, 0) \mapsto (L, Q)$
$(\mathbf{1}, \mathbf{4}, \mathbf{1}, \mathbf{1}, \mathbf{1}, \mathbf{1}, \mathbf{1}, \mathbf{2})$, $(0, 0, 0, 1, 0, 0, 0, 0, 0, 0, 0, 1) \mapsto (D, E, N, U)$
Projection matrix for $\alpha$:

$$\begin{pmatrix} 0 & 1 & 0 & 0 & 1 & 0 & 0 & 0 & 0 & 0 & 0 & 0 \\ 1 & 0 & 0 & 1 & 0 & 0 & 0 & 0 & 0 & 0 & 0 & 0 \\ 0 & 0 & 0 & 0 & 0 & 0 & 0 & 0 & 1 & 1 & 1 & 0 \\ -1 & -2 & -3 & -1 & -2 & -3 & 3 & 0 & 0 & 0 & 0 & 3 \end{pmatrix}$$

**3 generation subalgebra** 348
Algebra: $\mathfrak{su}(4) \oplus \mathfrak{su}(4) \oplus \mathfrak{su}(2) \oplus \mathfrak{su}(2) \oplus \mathfrak{su}(2) \oplus \mathfrak{su}(2) \oplus \mathfrak{su}(2) \oplus \mathfrak{su}(2)$
$(\mathbf{4}, \mathbf{1}, \mathbf{2}, \mathbf{2}, \mathbf{1}, \mathbf{1}, \mathbf{1}, \mathbf{1})$, $(1, 0, 0, 0, 0, 0, 1, 1, 0, 0, 0, 0) \mapsto (L, L, Q, Q)$

$(\overline{\mathbf{4}}, \mathbf{1}, \mathbf{1}, \mathbf{1}, \mathbf{2}, \mathbf{1}, \mathbf{1}, \mathbf{1})$, $(0,0,1,0,0,0,0,0,1,0,0,0) \mapsto (D, E, N, U)$
$(\overline{\mathbf{4}}, \mathbf{1}, \mathbf{1}, \mathbf{1}, \mathbf{1}, \mathbf{2}, \mathbf{1}, \mathbf{1})$, $(0,0,1,0,0,0,0,0,0,1,0,0) \mapsto (D, E, N, U)$
$(\mathbf{1}, \overline{\mathbf{4}}, \mathbf{1}, \mathbf{1}, \mathbf{1}, \mathbf{1}, \mathbf{2}, \mathbf{1})$, $(0,0,0,0,0,1,0,0,0,0,1,0) \mapsto (L, Q)$
$(\mathbf{1}, \mathbf{4}, \mathbf{1}, \mathbf{1}, \mathbf{1}, \mathbf{1}, \mathbf{1}, \mathbf{2})$, $(0,0,0,1,0,0,0,0,0,0,0,1) \mapsto (D, E, N, U)$
Projection matrix for $\alpha$:

$$\begin{pmatrix} 1 & 0 & 0 & 0 & 1 & 0 & 0 & 0 & 0 & 0 & 0 & 0 \\ 0 & 1 & 0 & 1 & 0 & 0 & 0 & 0 & 0 & 0 & 0 & 0 \\ 0 & 0 & 0 & 0 & 0 & 0 & 1 & 0 & 0 & 0 & 1 & 0 \\ 1 & 2 & 3 & -1 & -2 & -3 & 0 & 0 & 3 & 3 & 0 & 3 \end{pmatrix}$$

**3 generation subalgebra** 349
Algebra: $\mathfrak{su}(4) \oplus \mathfrak{su}(4) \oplus \mathfrak{su}(2) \oplus \mathfrak{su}(2) \oplus \mathfrak{su}(2) \oplus \mathfrak{su}(2) \oplus \mathfrak{su}(2) \oplus \mathfrak{su}(2)$
$(\overline{\mathbf{4}}, \mathbf{1}, \mathbf{2}, \mathbf{1}, \mathbf{1}, \mathbf{1}, \mathbf{1}, \mathbf{1})$, $(0,0,1,0,0,0,1,0,0,0,0,0) \mapsto (L, Q)$
$(\overline{\mathbf{4}}, \mathbf{1}, \mathbf{1}, \mathbf{2}, \mathbf{1}, \mathbf{1}, \mathbf{1}, \mathbf{1})$, $(0,0,1,0,0,0,0,1,0,0,0,0) \mapsto (L, Q)$
$(\mathbf{4}, \mathbf{1}, \mathbf{1}, \mathbf{1}, \mathbf{2}, \mathbf{1}, \mathbf{1}, \mathbf{1})$, $(1,0,0,0,0,0,0,0,1,0,0,0) \mapsto (D, E, N, U)$
$(\mathbf{4}, \mathbf{1}, \mathbf{1}, \mathbf{1}, \mathbf{1}, \mathbf{2}, \mathbf{1}, \mathbf{1})$, $(1,0,0,0,0,0,0,0,0,1,0,0) \mapsto (D, E, N, U)$
$(\mathbf{1}, \overline{\mathbf{4}}, \mathbf{1}, \mathbf{1}, \mathbf{1}, \mathbf{1}, \mathbf{2}, \mathbf{1})$, $(0,0,0,0,0,1,0,0,0,0,1,0) \mapsto (L, Q)$
$(\mathbf{1}, \mathbf{4}, \mathbf{1}, \mathbf{1}, \mathbf{1}, \mathbf{1}, \mathbf{1}, \mathbf{2})$, $(0,0,0,1,0,0,0,0,0,0,0,1) \mapsto (D, E, N, U)$
Projection matrix for $\alpha$:

$$\begin{pmatrix} 0 & 1 & 0 & 0 & 1 & 0 & 0 & 0 & 0 & 0 & 0 & 0 \\ 1 & 0 & 0 & 1 & 0 & 0 & 0 & 0 & 0 & 0 & 0 & 0 \\ 0 & 0 & 0 & 0 & 0 & 0 & 1 & 1 & 0 & 0 & 1 & 0 \\ -1 & -2 & -3 & -1 & -2 & -3 & 0 & 0 & 3 & 3 & 0 & 3 \end{pmatrix}$$

**3 generation subalgebra** 350
Algebra: $\mathfrak{su}(4) \oplus \mathfrak{su}(4) \oplus \mathfrak{su}(4) \oplus \mathfrak{su}(2) \oplus \mathfrak{su}(2) \oplus \mathfrak{su}(2) \oplus \mathfrak{su}(2) \oplus \mathfrak{su}(2)$
$(\overline{\mathbf{4}}, \mathbf{1}, \mathbf{1}, \mathbf{2}, \mathbf{1}, \mathbf{1}, \mathbf{1}, \mathbf{1})$, $(0,0,1,0,0,0,0,0,0,1,0,0,0,0) \mapsto (L, Q)$
$(\mathbf{1}, \overline{\mathbf{4}}, \mathbf{1}, \mathbf{2}, \mathbf{1}, \mathbf{1}, \mathbf{1}, \mathbf{1})$, $(0,0,0,0,0,1,0,0,0,1,0,0,0,0) \mapsto (L, Q)$
$(\mathbf{4}, \mathbf{1}, \mathbf{1}, \mathbf{1}, \mathbf{2}, \mathbf{1}, \mathbf{1}, \mathbf{1})$, $(1,0,0,0,0,0,0,0,0,0,1,0,0,0) \mapsto (D, E, N, U)$
$(\mathbf{1}, \mathbf{4}, \mathbf{1}, \mathbf{1}, \mathbf{1}, \mathbf{2}, \mathbf{1}, \mathbf{1})$, $(0,0,0,1,0,0,0,0,0,0,0,1,0,0) \mapsto (D, E, N, U)$
$(\mathbf{1}, \mathbf{1}, \overline{\mathbf{4}}, \mathbf{1}, \mathbf{1}, \mathbf{1}, \mathbf{2}, \mathbf{1})$, $(0,0,0,0,0,0,0,0,1,0,0,0,1,0) \mapsto (L, Q)$
$(\mathbf{1}, \mathbf{1}, \mathbf{4}, \mathbf{1}, \mathbf{1}, \mathbf{1}, \mathbf{1}, \mathbf{2})$, $(0,0,0,0,0,0,1,0,0,0,0,0,0,1) \mapsto (D, E, N, U)$
Projection matrix for $\alpha$:

$$\begin{pmatrix} 0 & 1 & 0 & 0 & 1 & 0 & 0 & 1 & 0 & 0 & 0 & 0 & 0 & 0 \\ 1 & 0 & 0 & 1 & 0 & 0 & 1 & 0 & 0 & 0 & 0 & 0 & 0 & 0 \\ 0 & 0 & 0 & 0 & 0 & 0 & 0 & 0 & 0 & 1 & 0 & 0 & 1 & 0 \\ -1 & -2 & -3 & -1 & -2 & -3 & -1 & -2 & -3 & 0 & 3 & 3 & 0 & 3 \end{pmatrix}$$

**3 generation subalgebra** 351
Algebra: $\mathfrak{su}(4) \oplus \mathfrak{su}(4) \oplus \mathfrak{su}(4) \oplus \mathfrak{su}(2) \oplus \mathfrak{su}(2) \oplus \mathfrak{su}(2) \oplus \mathfrak{su}(2) \oplus \mathfrak{su}(2)$
$(\overline{\mathbf{4}}, \mathbf{1}, \mathbf{1}, \mathbf{2}, \mathbf{1}, \mathbf{1}, \mathbf{1}, \mathbf{1})$, $(0,0,1,0,0,0,0,0,0,1,0,0,0,0) \mapsto (D, E, N, U)$
$(\mathbf{1}, \overline{\mathbf{4}}, \mathbf{1}, \mathbf{2}, \mathbf{1}, \mathbf{1}, \mathbf{1}, \mathbf{1})$, $(0,0,0,0,0,1,0,0,0,1,0,0,0,0) \mapsto (D, E, N, U)$
$(\mathbf{4}, \mathbf{1}, \mathbf{1}, \mathbf{1}, \mathbf{2}, \mathbf{1}, \mathbf{1}, \mathbf{1})$, $(1,0,0,0,0,0,0,0,0,0,1,0,0,0) \mapsto (L, Q)$
$(\mathbf{1}, \mathbf{4}, \mathbf{1}, \mathbf{1}, \mathbf{1}, \mathbf{2}, \mathbf{1}, \mathbf{1})$, $(0,0,0,1,0,0,0,0,0,0,0,1,0,0) \mapsto (L, Q)$
$(\mathbf{1}, \mathbf{1}, \overline{\mathbf{4}}, \mathbf{1}, \mathbf{1}, \mathbf{1}, \mathbf{2}, \mathbf{1})$, $(0,0,0,0,0,0,0,0,1,0,0,0,1,0) \mapsto (L, Q)$
$(\mathbf{1}, \mathbf{1}, \mathbf{4}, \mathbf{1}, \mathbf{1}, \mathbf{1}, \mathbf{1}, \mathbf{2})$, $(0,0,0,0,0,0,1,0,0,0,0,0,0,1) \mapsto (D, E, N, U)$
Projection matrix for $\alpha$:

$$\begin{pmatrix} 1 & 0 & 0 & 1 & 0 & 0 & 0 & 1 & 0 & 0 & 0 & 0 & 0 & 0 \\ 0 & 1 & 0 & 0 & 1 & 0 & 1 & 0 & 0 & 0 & 0 & 0 & 0 & 0 \\ 0 & 0 & 0 & 0 & 0 & 0 & 0 & 0 & 0 & 0 & 1 & 1 & 1 & 0 \\ 1 & 2 & 3 & 1 & 2 & 3 & -1 & -2 & -3 & 3 & 0 & 0 & 0 & 3 \end{pmatrix}$$

**3 generation subalgebra** 352
Algebra: $\mathfrak{su}(4) \oplus \mathfrak{su}(4) \oplus \mathfrak{su}(4) \oplus \mathfrak{su}(2) \oplus \mathfrak{su}(2) \oplus \mathfrak{su}(2) \oplus \mathfrak{su}(2) \oplus \mathfrak{su}(2) \oplus \mathfrak{su}(2)$
$(\overline{\mathbf{4}}, \mathbf{1}, \mathbf{1}, \mathbf{2}, \mathbf{1}, \mathbf{1}, \mathbf{1}, \mathbf{1}, \mathbf{1})$, $(0,0,1,0,0,0,0,0,0,1,0,0,0,0,0) \mapsto (L, Q)$
$(\mathbf{4}, \mathbf{1}, \mathbf{1}, \mathbf{1}, \mathbf{2}, \mathbf{1}, \mathbf{1}, \mathbf{1}, \mathbf{1})$, $(1,0,0,0,0,0,0,0,0,0,1,0,0,0,0) \mapsto (D, E, N, U)$

$(\mathbf{1}, \overline{\mathbf{4}}, \mathbf{1}, \mathbf{1}, \mathbf{1}, \mathbf{2}, \mathbf{1}, \mathbf{1}, \mathbf{1}),\ (0, 0, 0, 0, 0, 1, 0, 0, 0, 0, 0, 1, 0, 0, 0) \mapsto (L, Q)$
$(\mathbf{1}, \mathbf{4}, \mathbf{1}, \mathbf{1}, \mathbf{1}, \mathbf{1}, \mathbf{2}, \mathbf{1}, \mathbf{1}),\ (0, 0, 0, 1, 0, 0, 0, 0, 0, 0, 0, 0, 1, 0, 0) \mapsto (D, E, N, U)$
$(\mathbf{1}, \mathbf{1}, \overline{\mathbf{4}}, \mathbf{1}, \mathbf{1}, \mathbf{1}, \mathbf{1}, \mathbf{2}, \mathbf{1}),\ (0, 0, 0, 0, 0, 0, 0, 0, 1, 0, 0, 0, 0, 1, 0) \mapsto (L, Q)$
$(\mathbf{1}, \mathbf{1}, \mathbf{4}, \mathbf{1}, \mathbf{1}, \mathbf{1}, \mathbf{1}, \mathbf{1}, \mathbf{2}),\ (0, 0, 0, 0, 0, 0, 1, 0, 0, 0, 0, 0, 0, 0, 1) \mapsto (D, E, N, U)$
Projection matrix for $\alpha$:

$$\begin{pmatrix} 0 & 1 & 0 & 0 & 1 & 0 & 0 & 1 & 0 & 0 & 0 & 0 & 0 & 0 & 0 \\ 1 & 0 & 0 & 1 & 0 & 0 & 1 & 0 & 0 & 0 & 0 & 0 & 0 & 0 & 0 \\ 0 & 0 & 0 & 0 & 0 & 0 & 0 & 0 & 0 & 1 & 0 & 1 & 0 & 1 & 0 \\ -1 & -2 & -3 & -1 & -2 & -3 & -1 & -2 & -3 & 0 & 3 & 0 & 3 & 0 & 3 \end{pmatrix}$$
